# Supplementary material for: Coherent turbulent structures in a rapid contraction
Source: arXiv:2401.05869 source file (2024-01-11)
Supplement: Supplementary file 1 [file StrRun1.pdf]

# Run 1

Iso-surface of  $|\omega| = 40 \text{ } ^1/s$

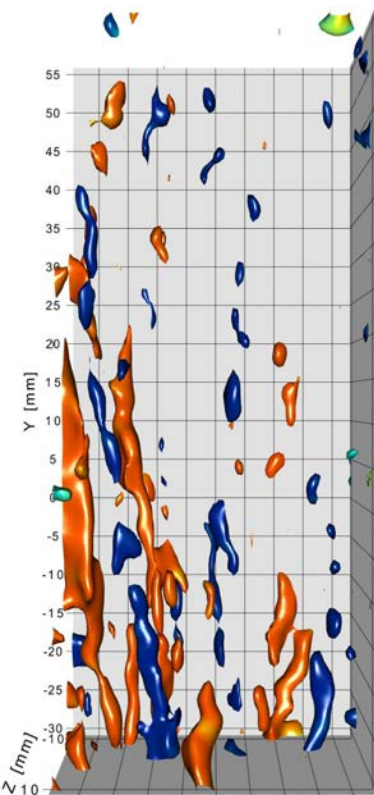

3136

1

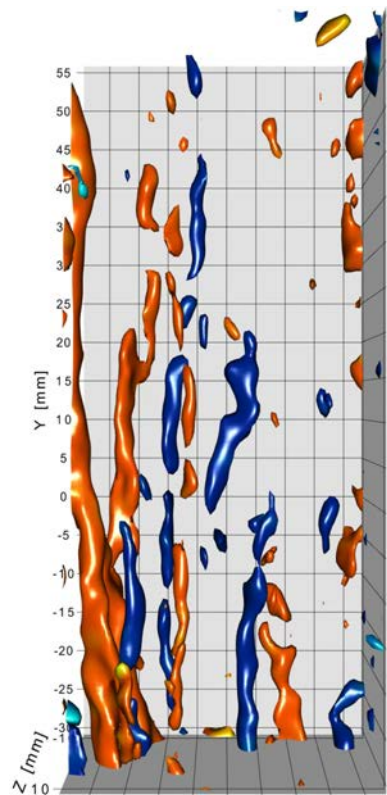

3253

2

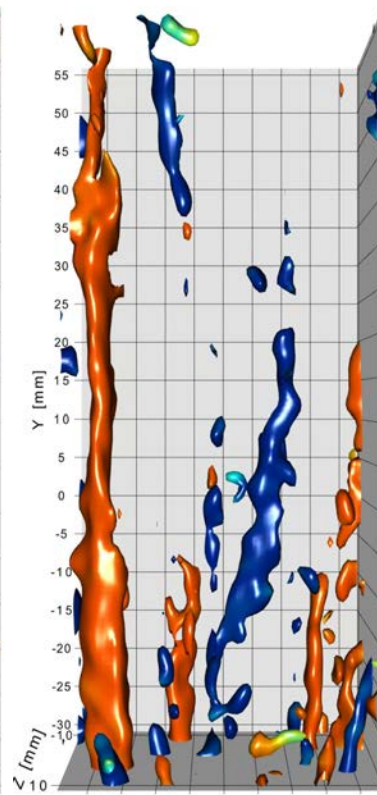

3497

3

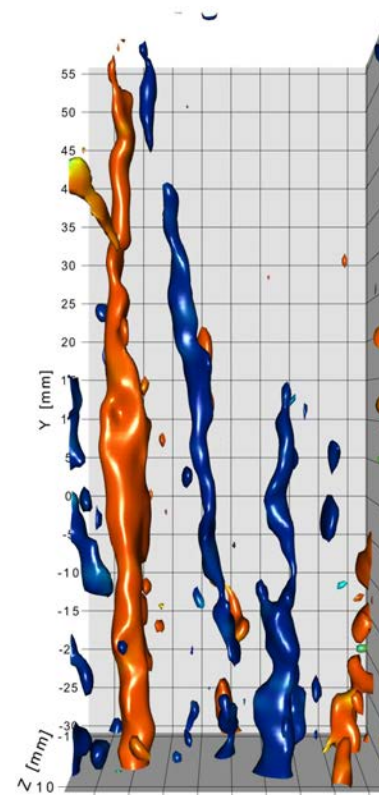

3583

4

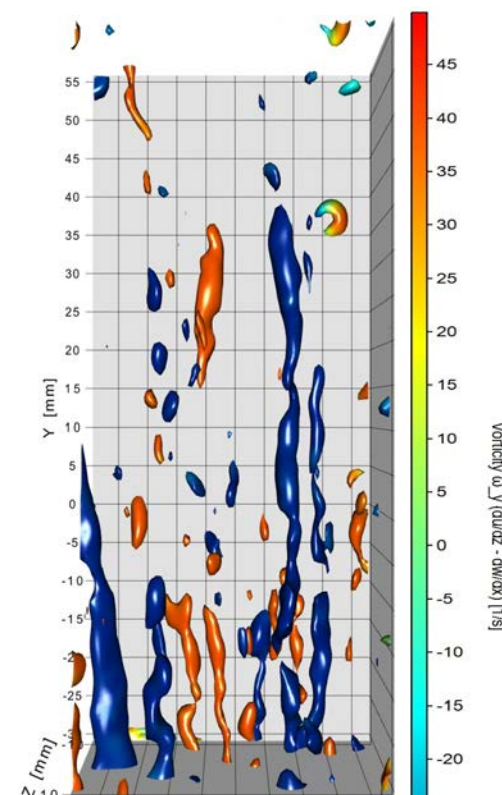

4055

5

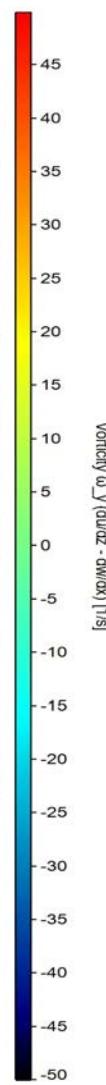

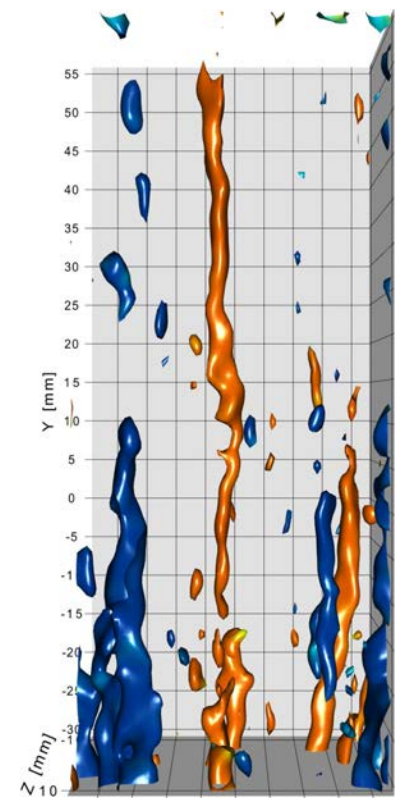

5651

6

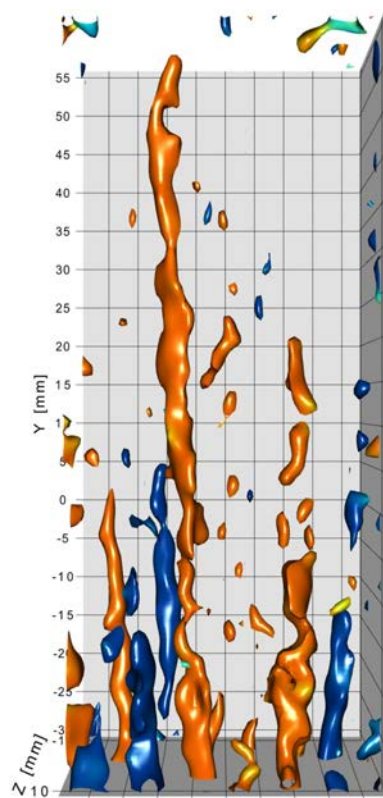

5987

7

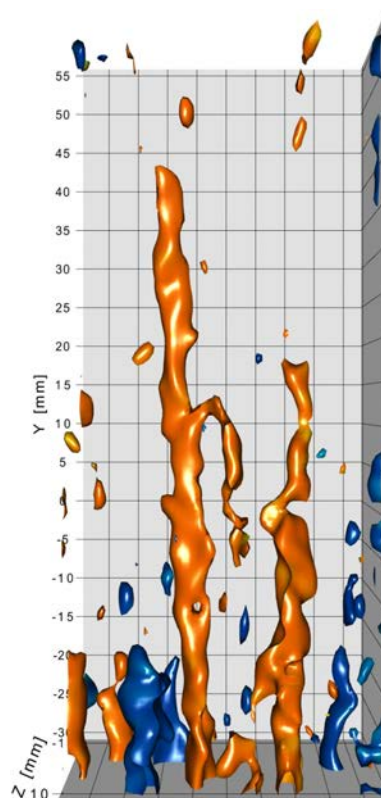

6036

8

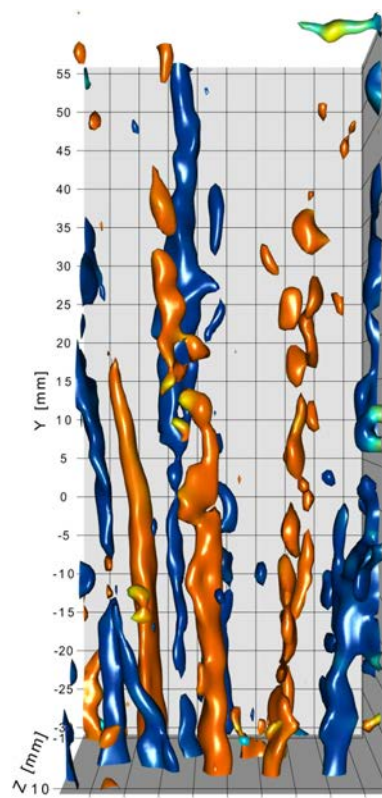

6466

9

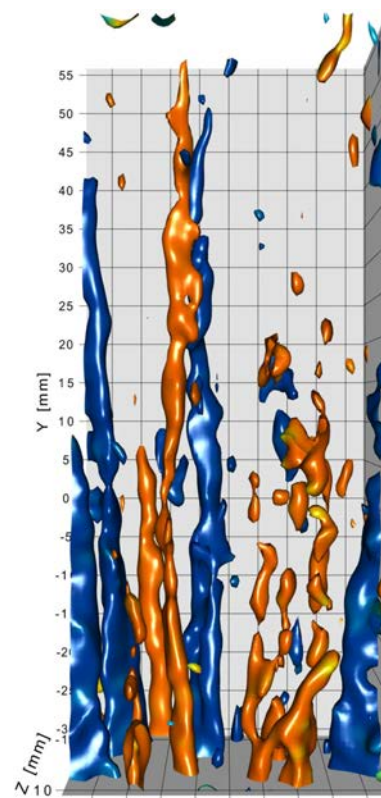

6614

10



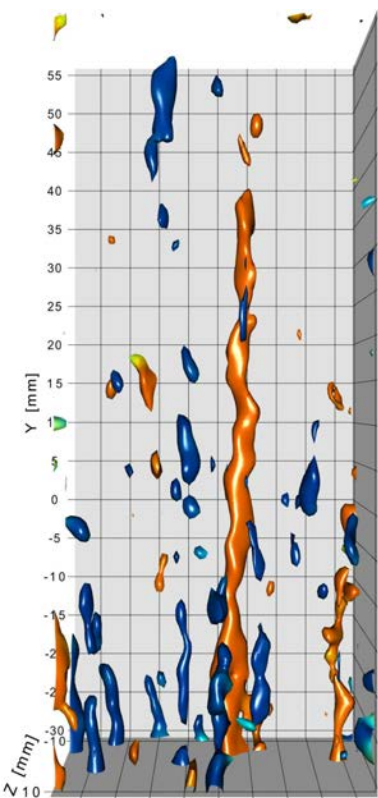

7314

11

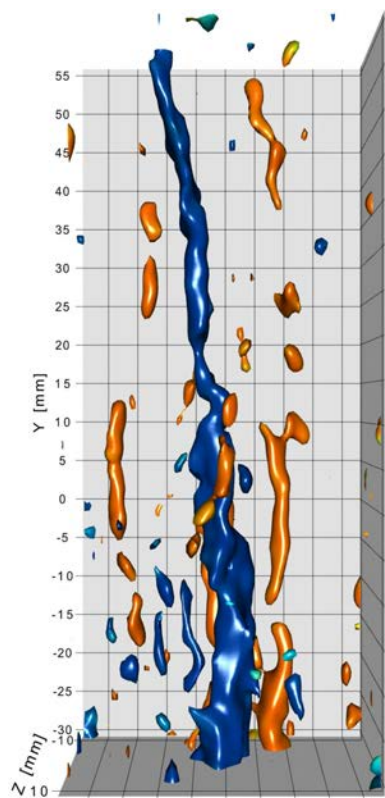

7606

12

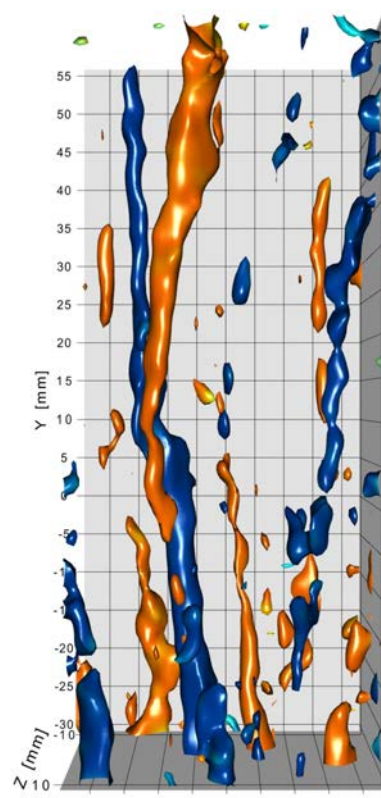

7825

13

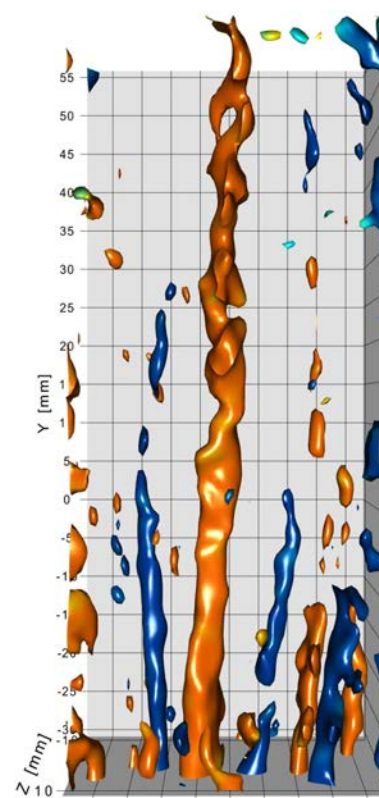

8002

14

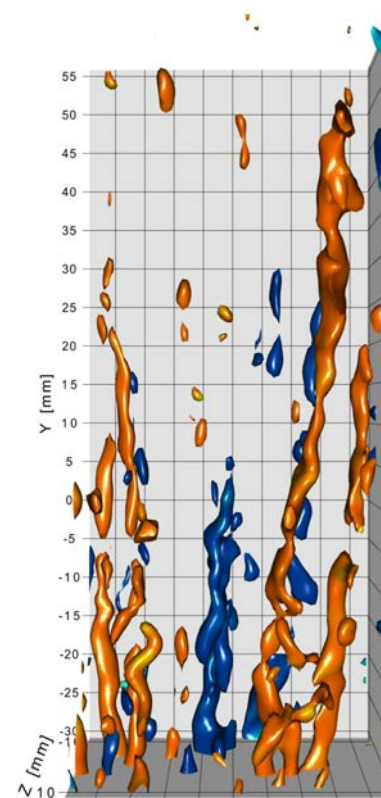

8519

15

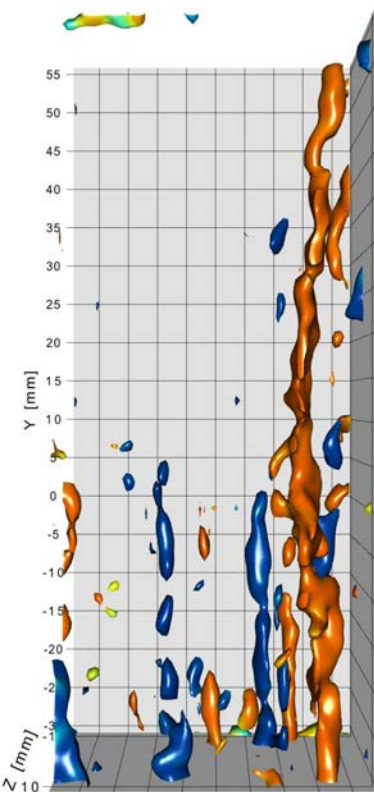

9779

16

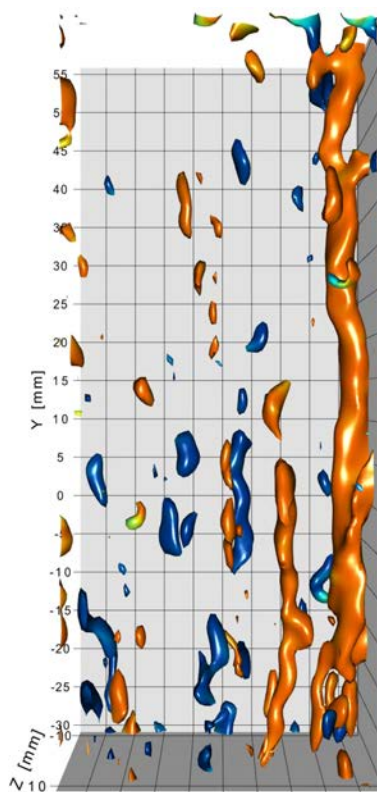

11668

17

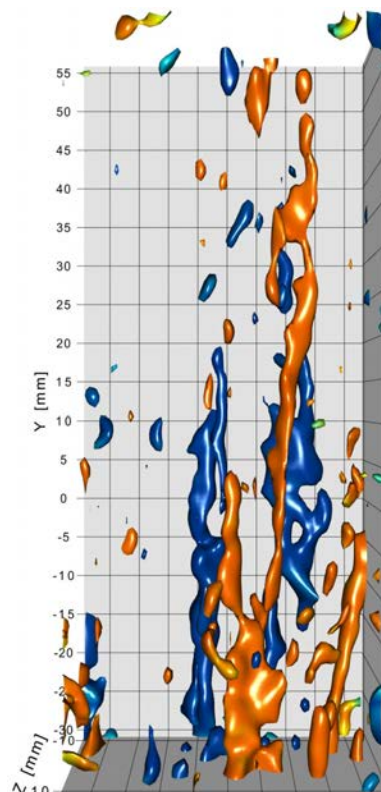

12120

18

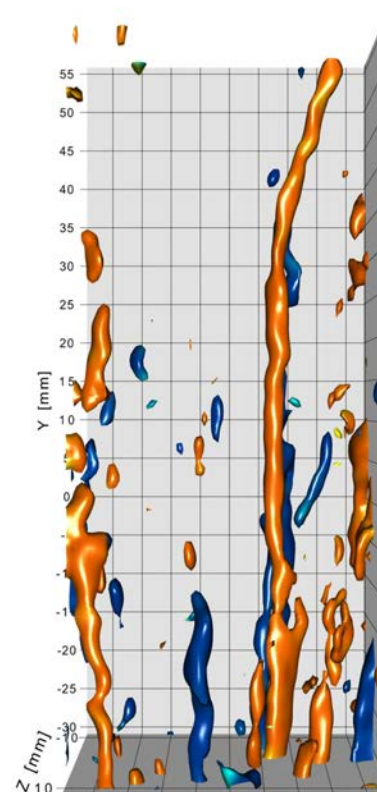

12514

19

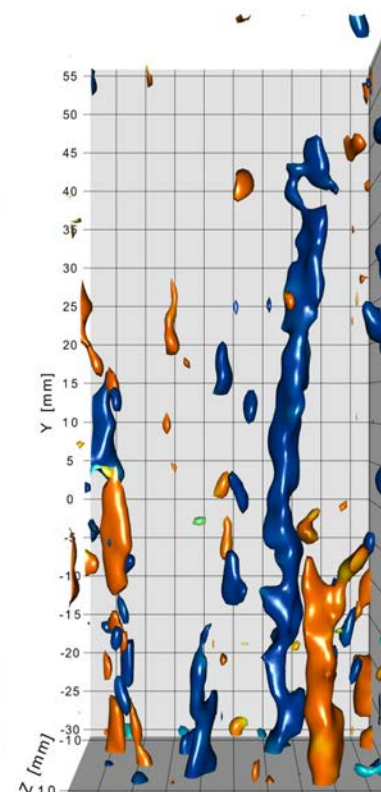

13061

20



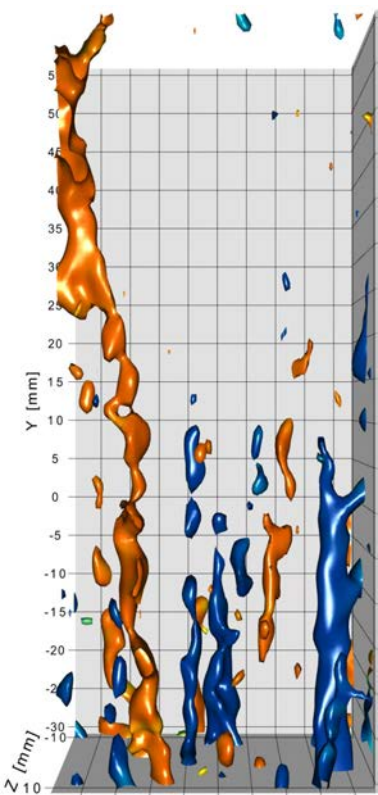

13628

21

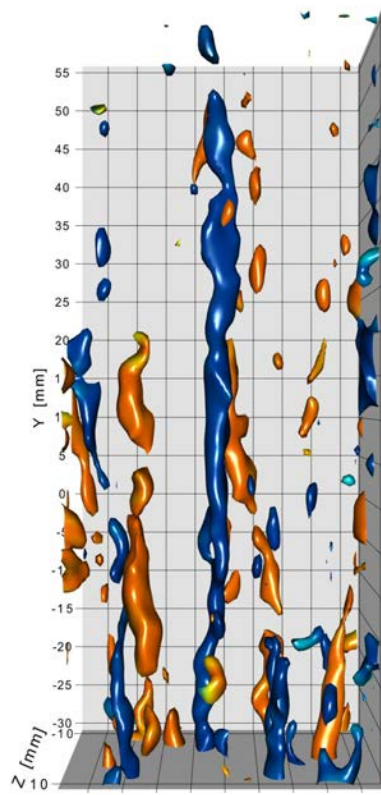

13966

22

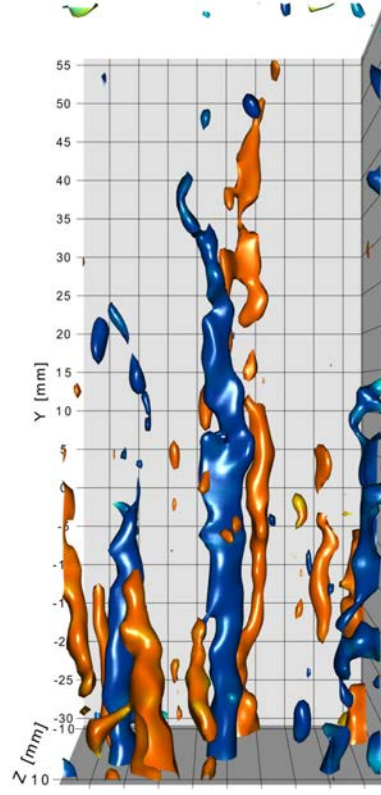

14065

23

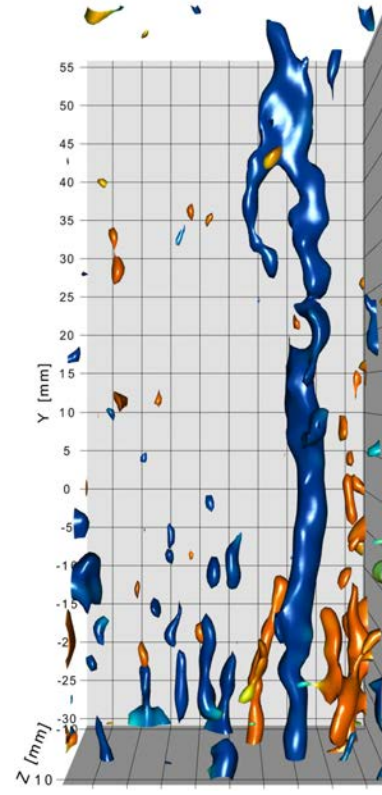

16680

24

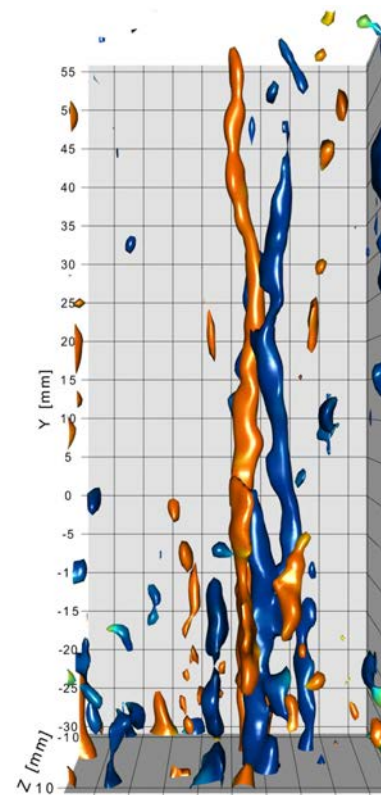

16943

25

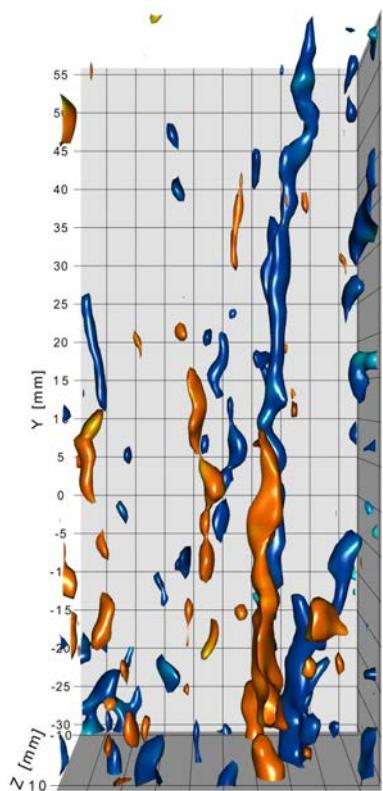

17370

26

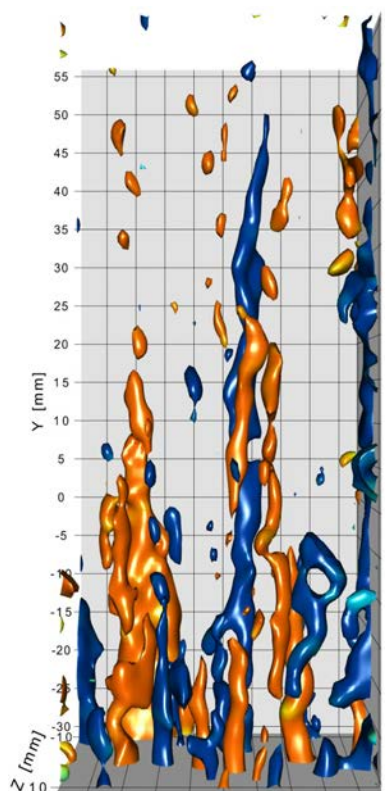

17798

27

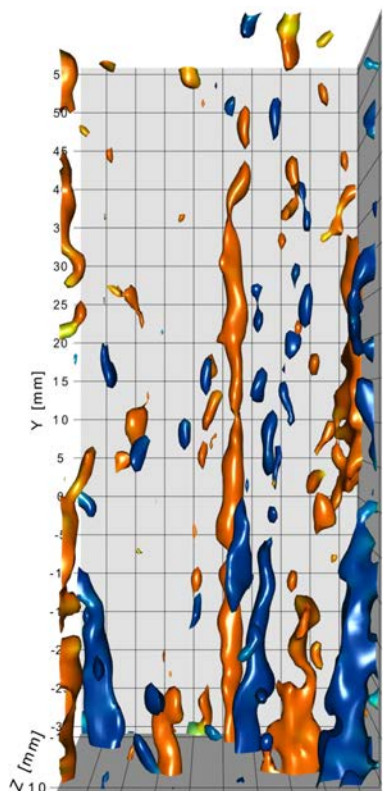

17978

28

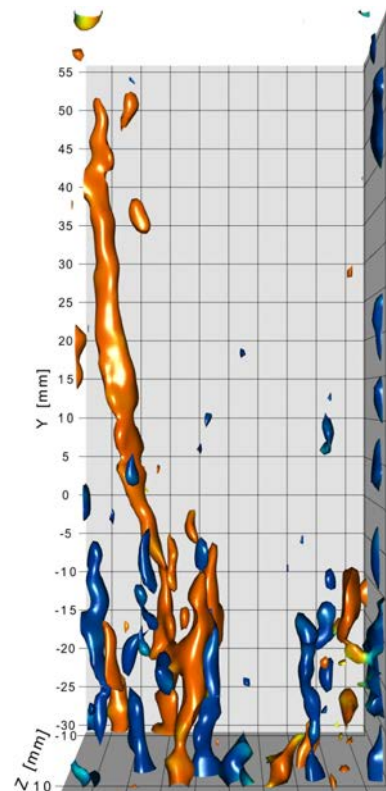

19416

29

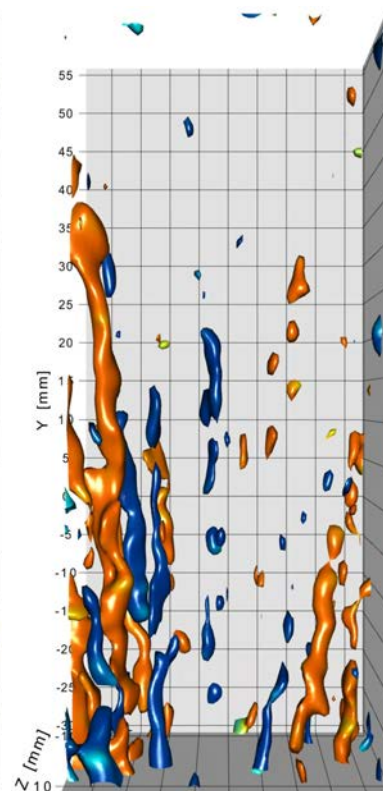

20998

30



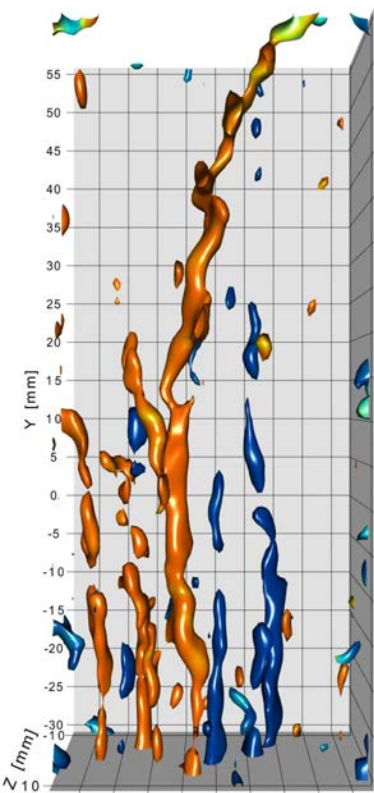

22547

31

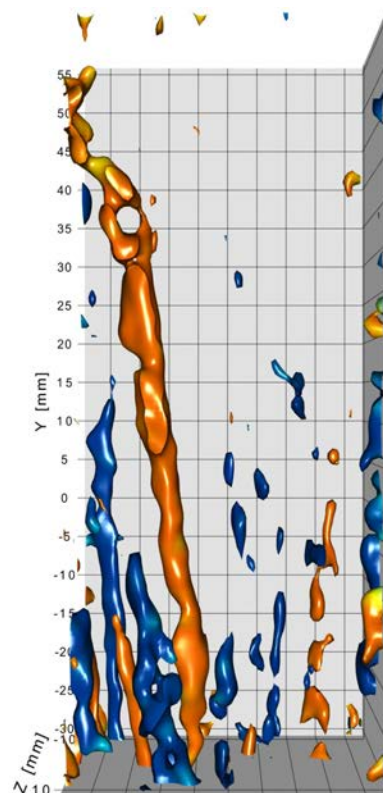

22974

32

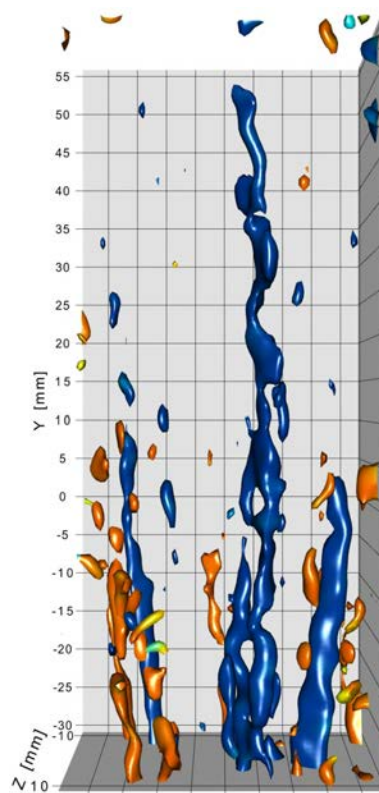

25992

33

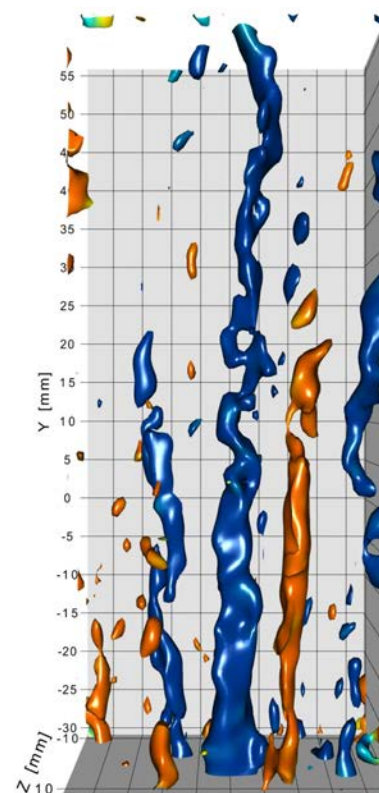

26195

34

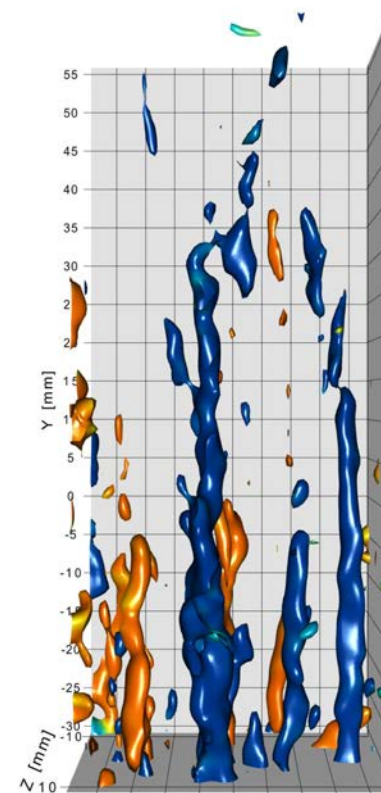

28300

35



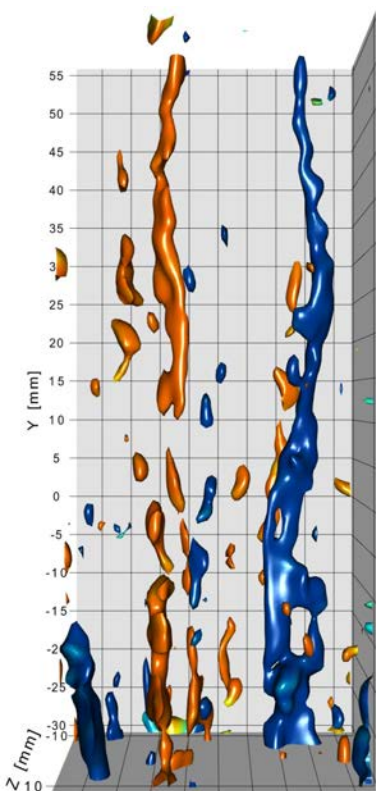

29176

36

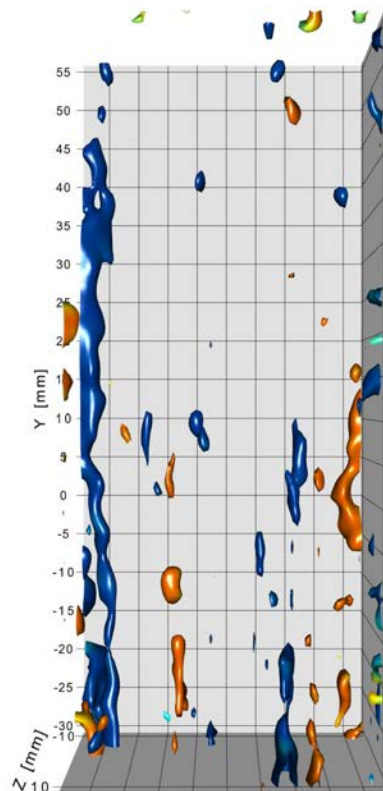

30838

37

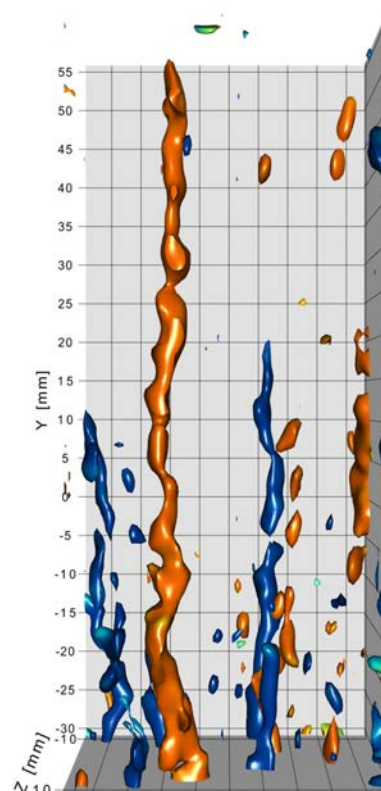

31072

38

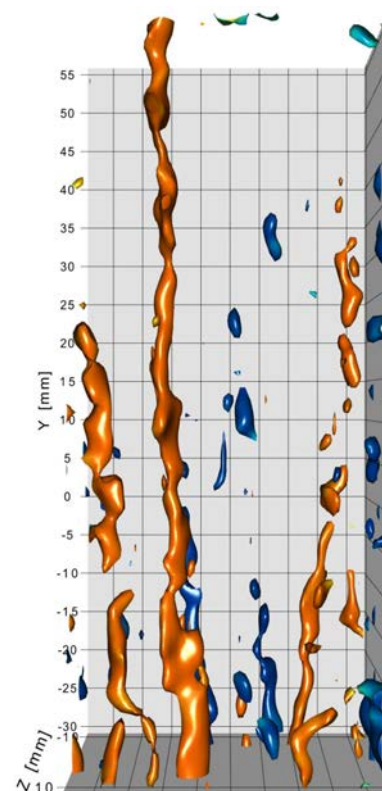

31263

39

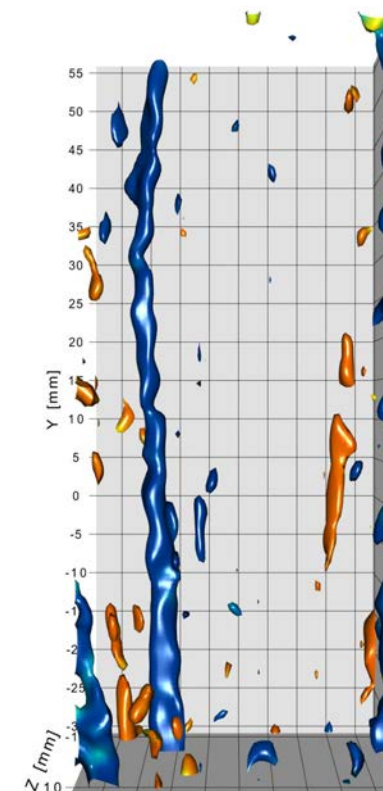

32229

40

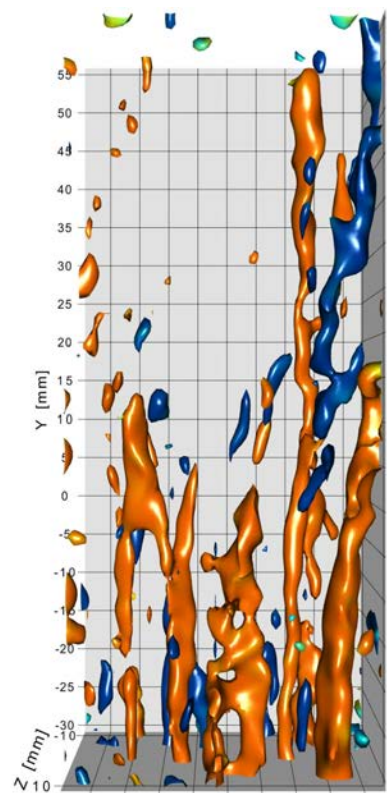

32684

41

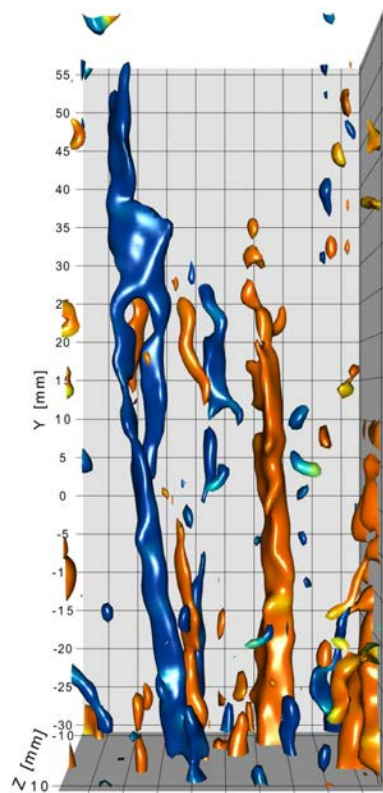

32994

42

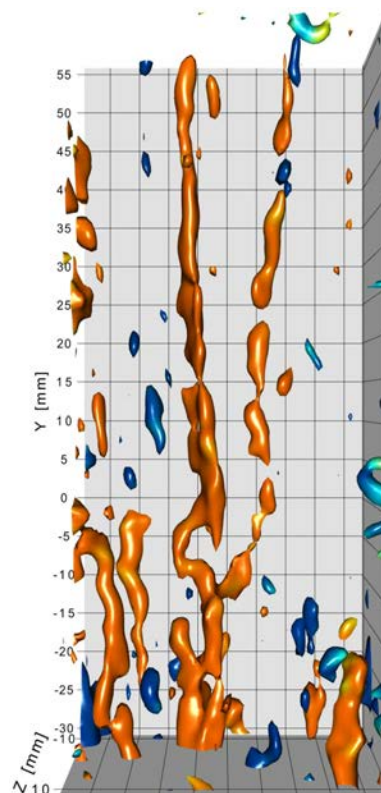

33986

43

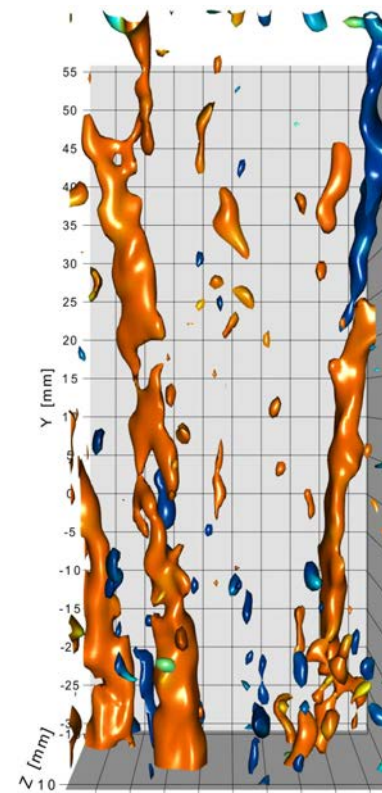

34415

44

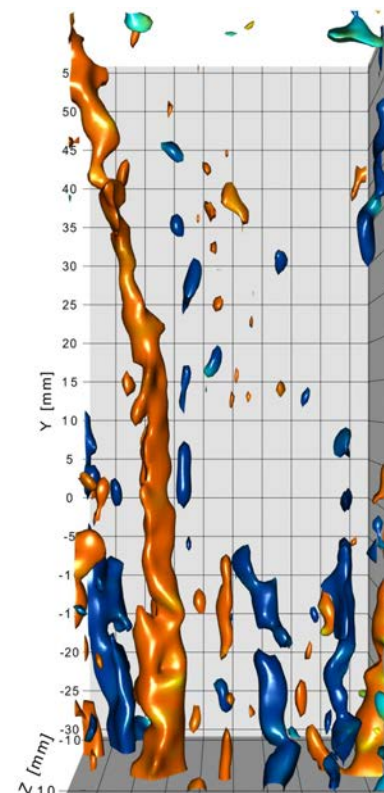

34643

45



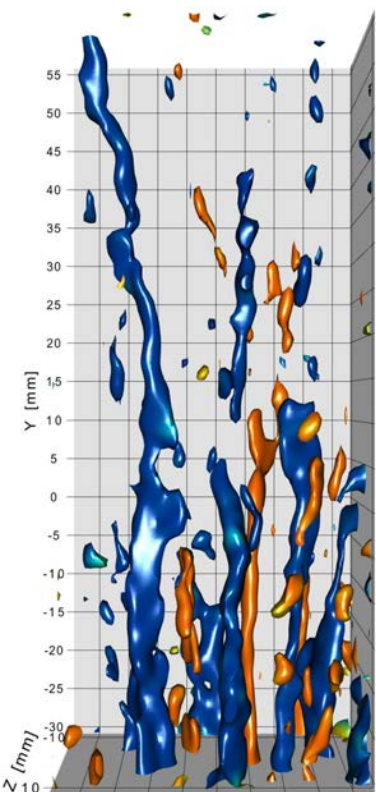

35430

46

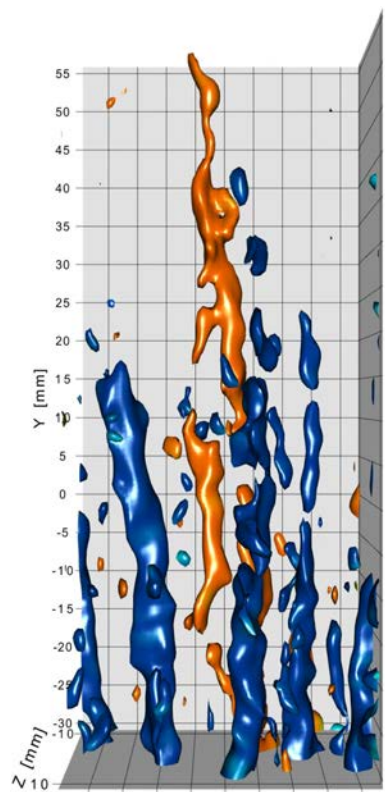

35578

47

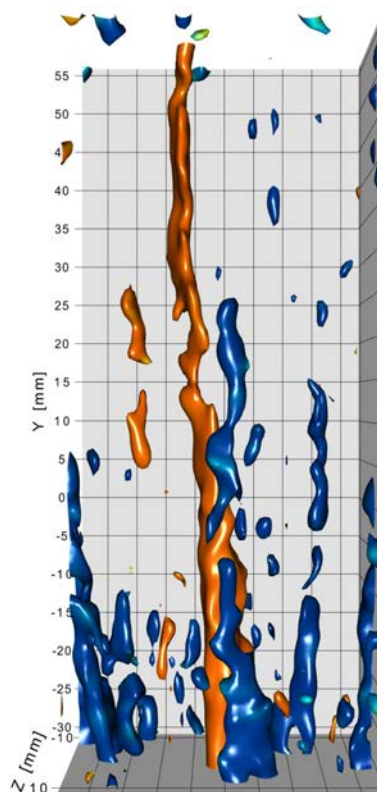

35724

48

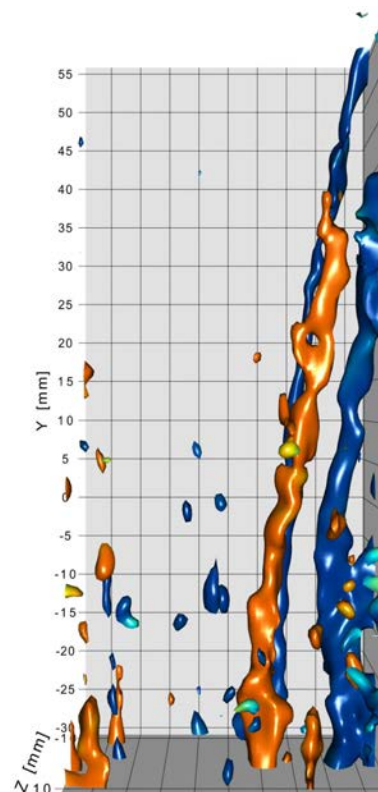

37171

49

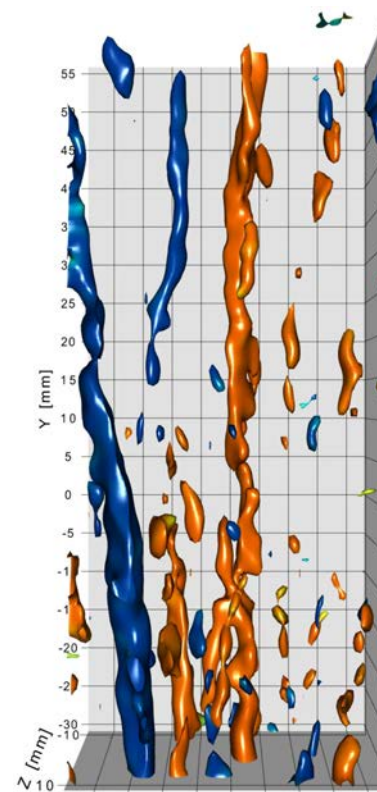

39430

50



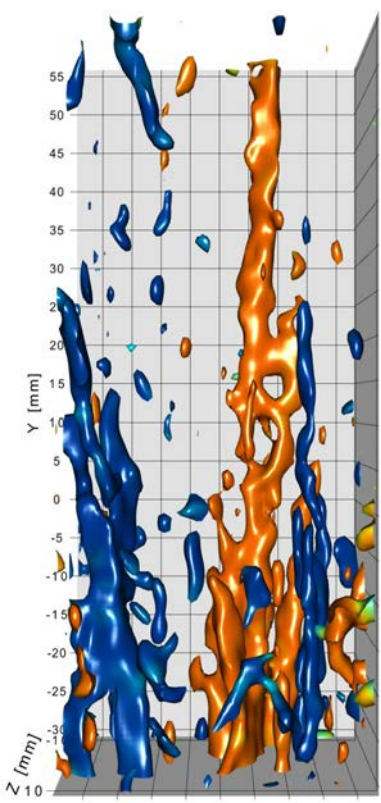

39761

51

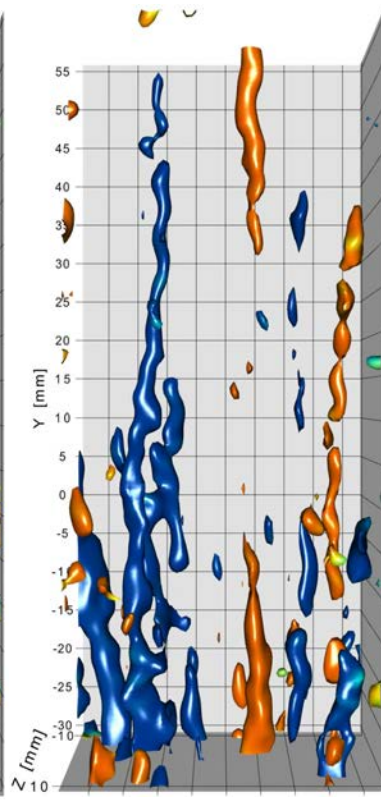

40643

52

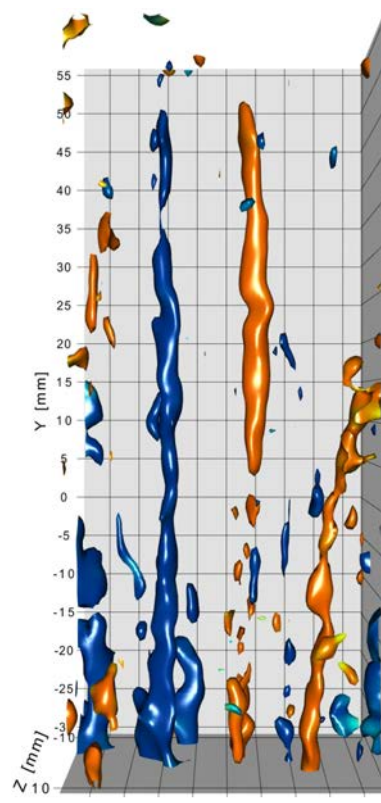

40719

53

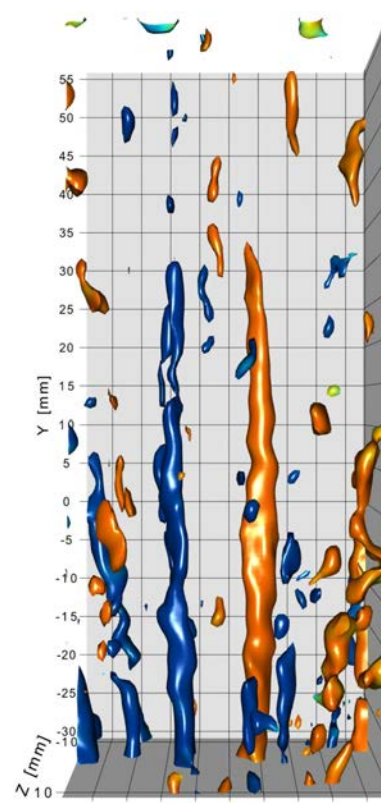

40786

54

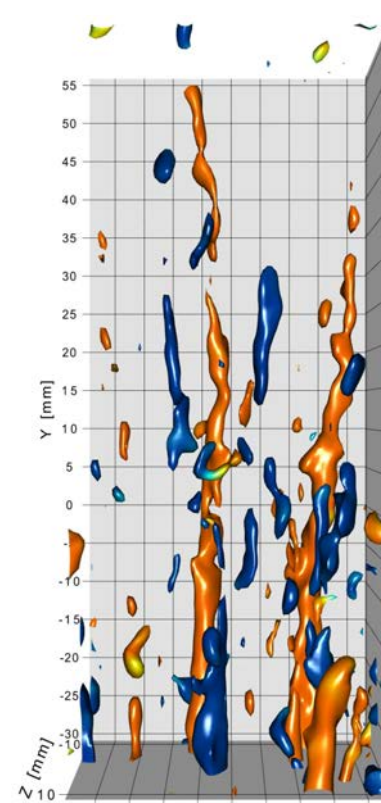

41830

55

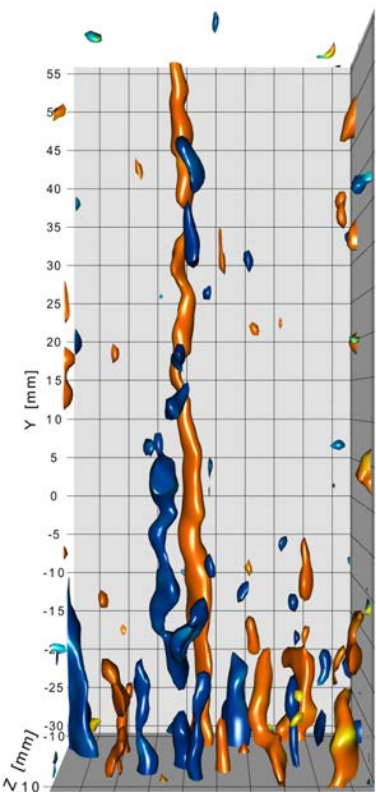

41979

56

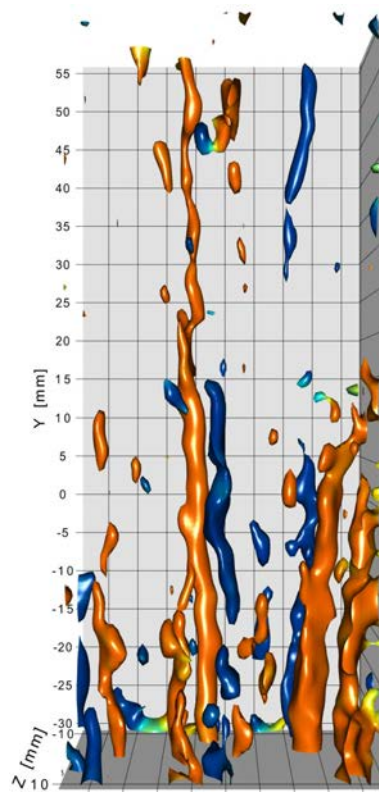

42172

57

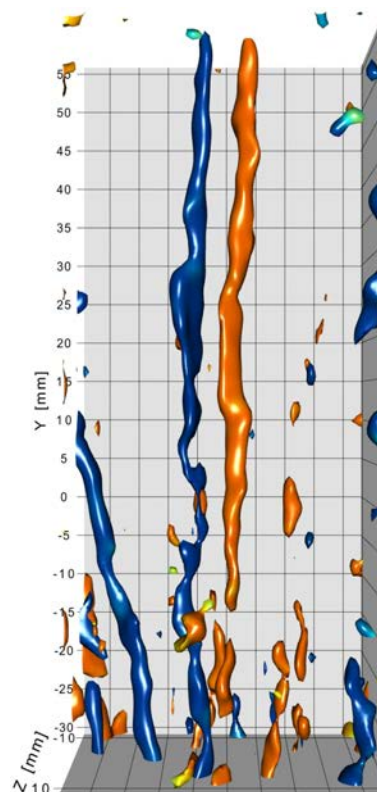

42620

58

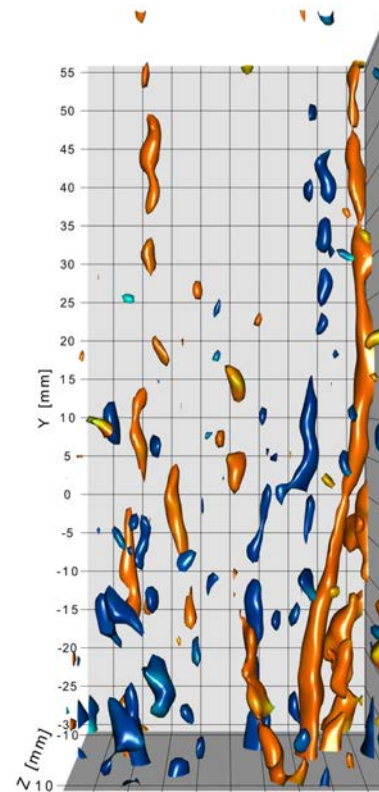

43246

59

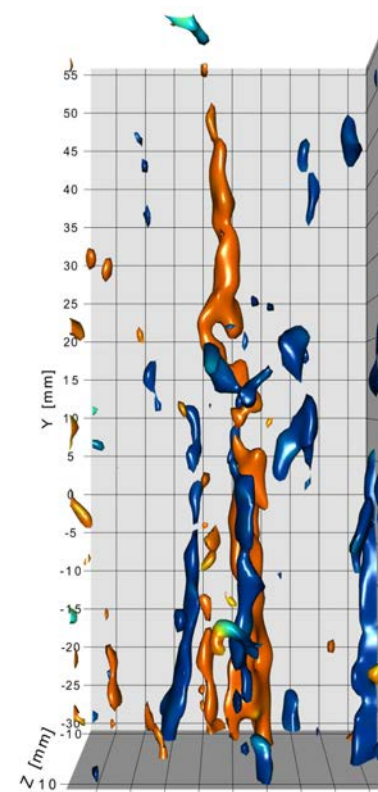

44425

60



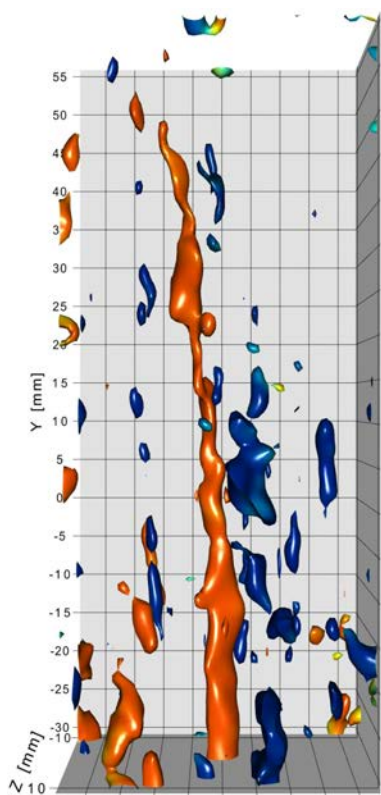

44549

61

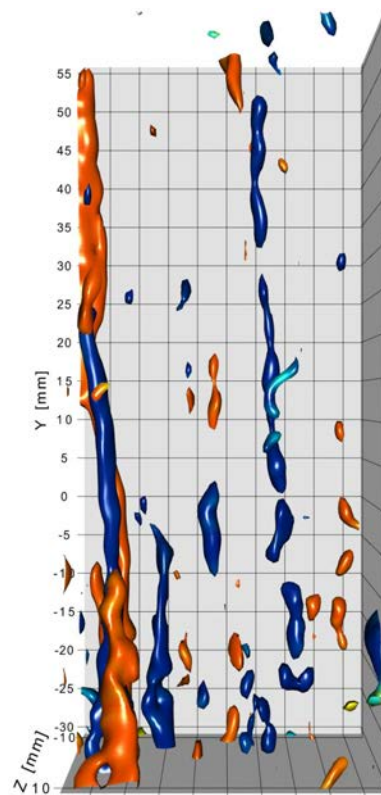

45000

62

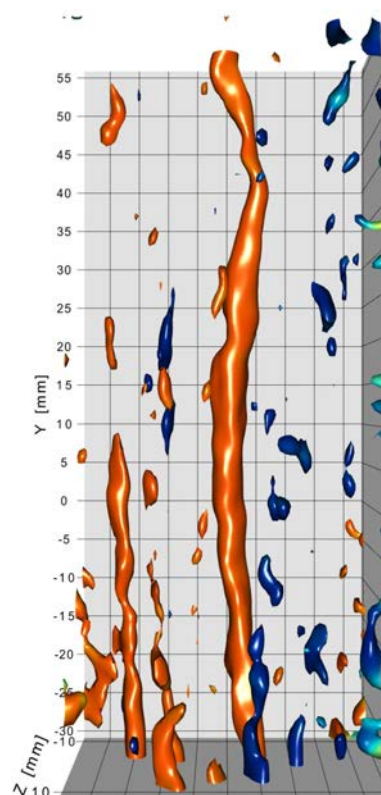

45214

63

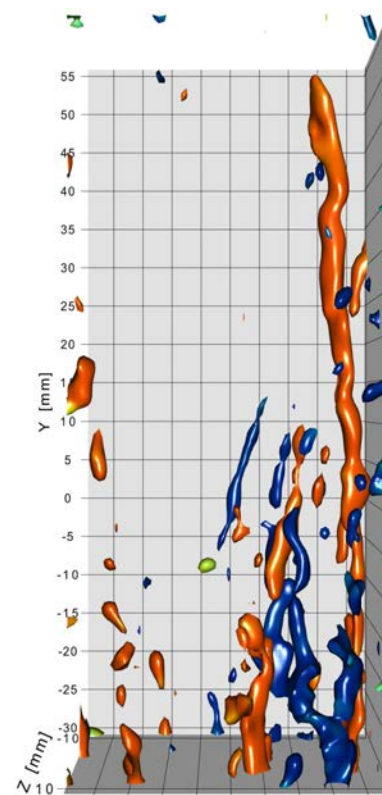

46382

64

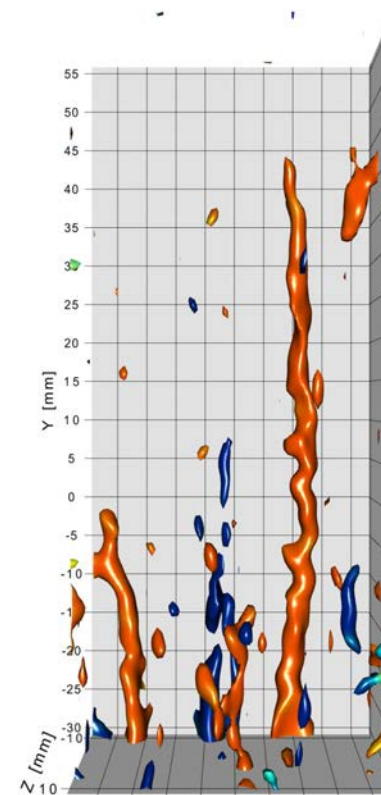

47360

65



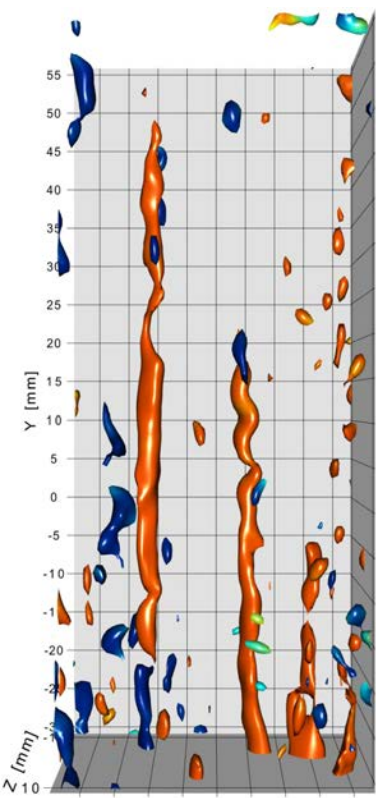

47562

66

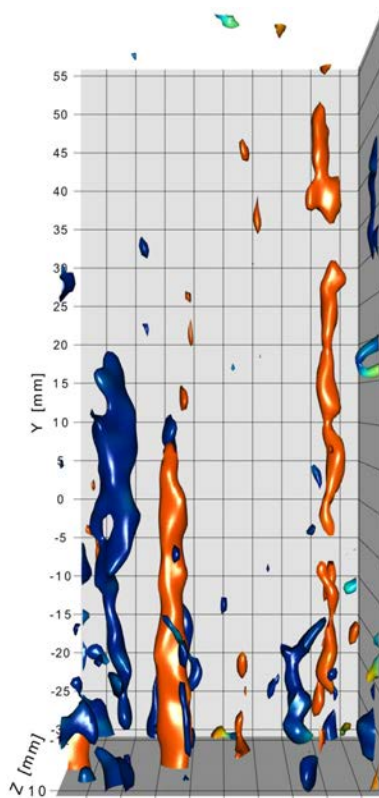

47702

67

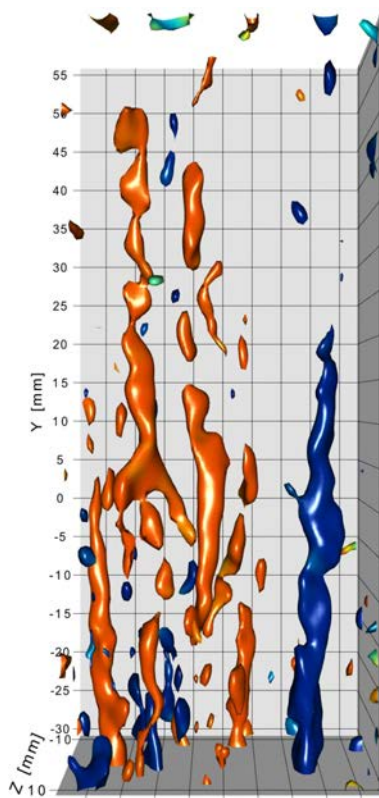

48841

68

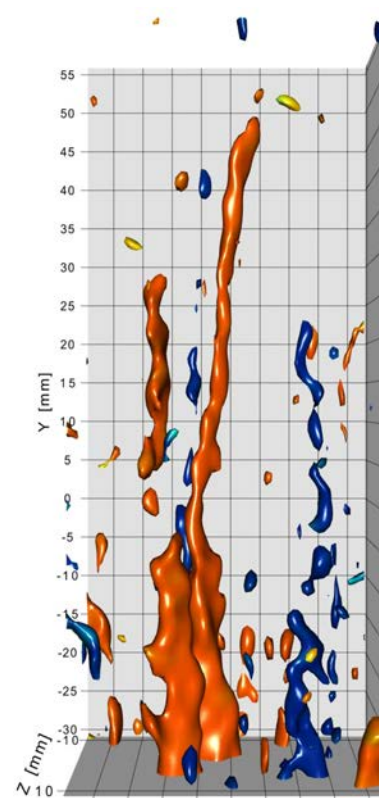

48999

69

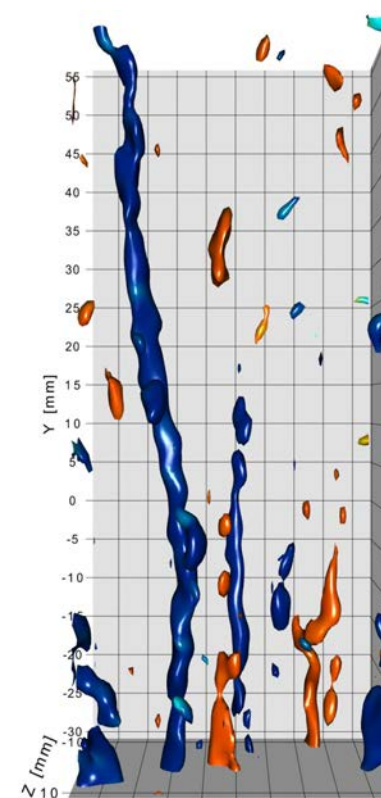

49571

70

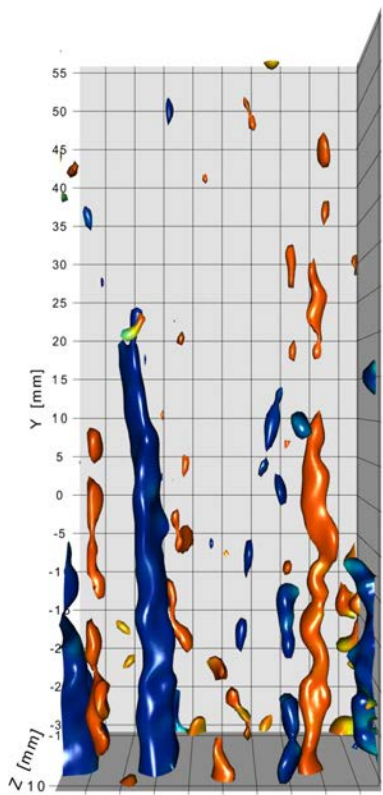

49727

71

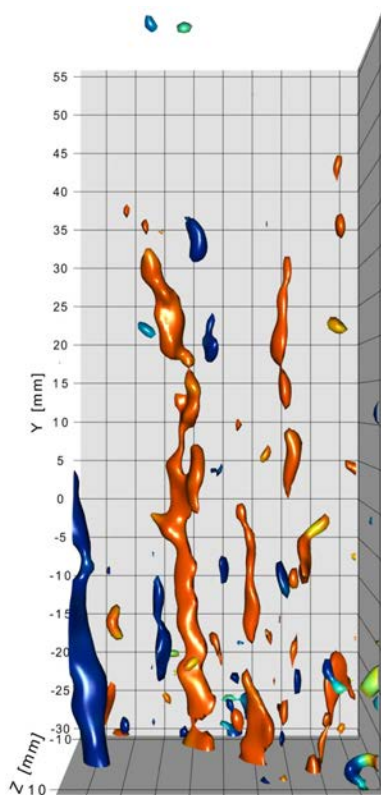

50148

72

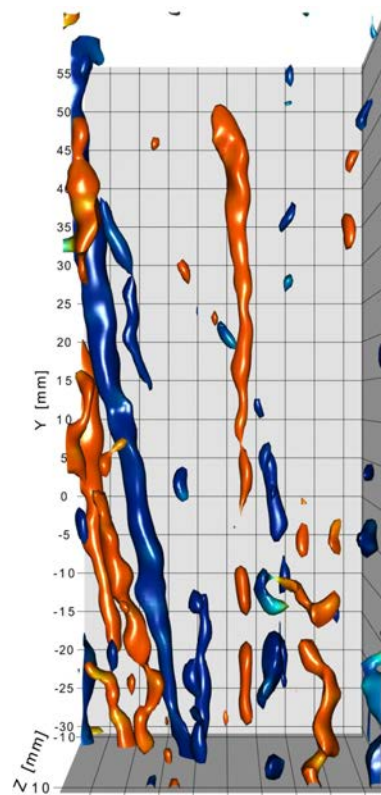

50727

73

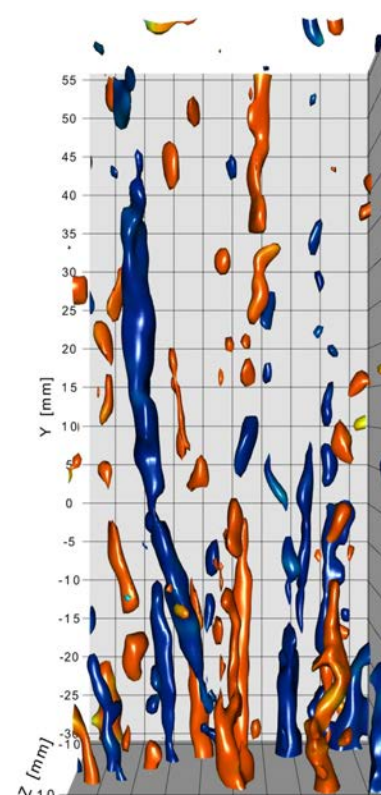

52282

74

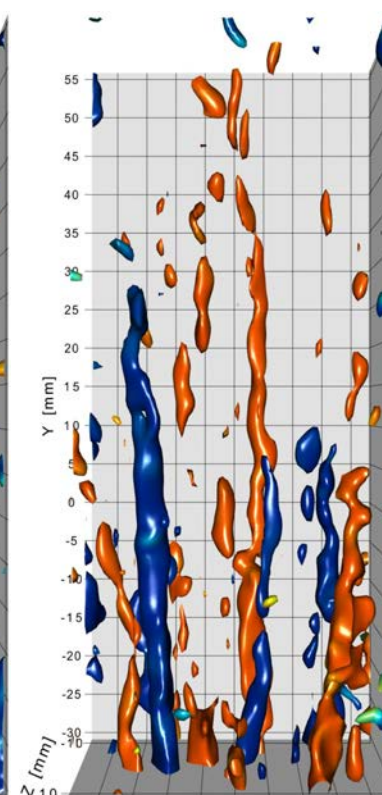

52364

75



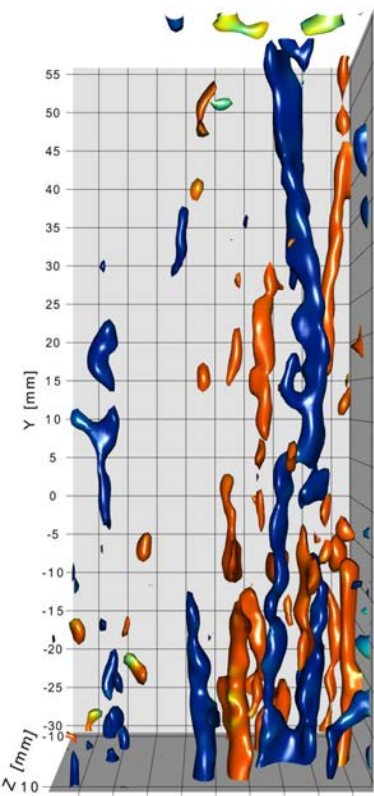

52719

76

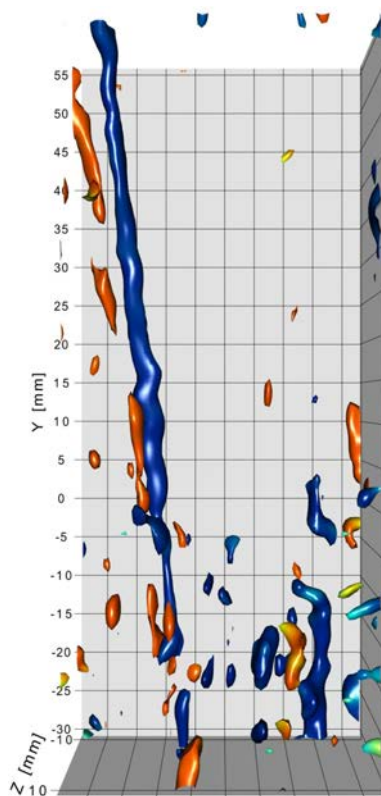

53412

77

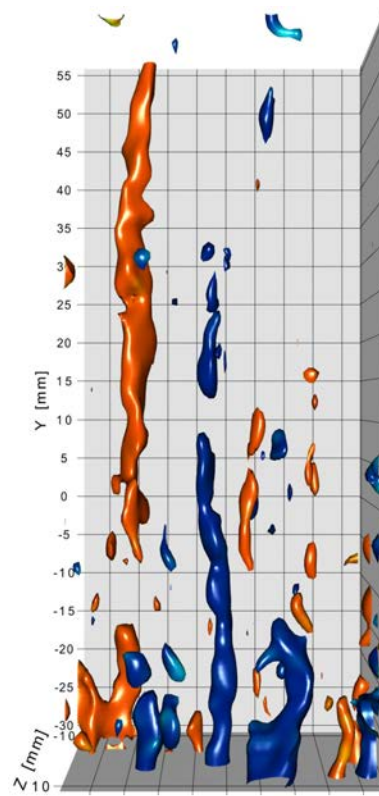

54477

78

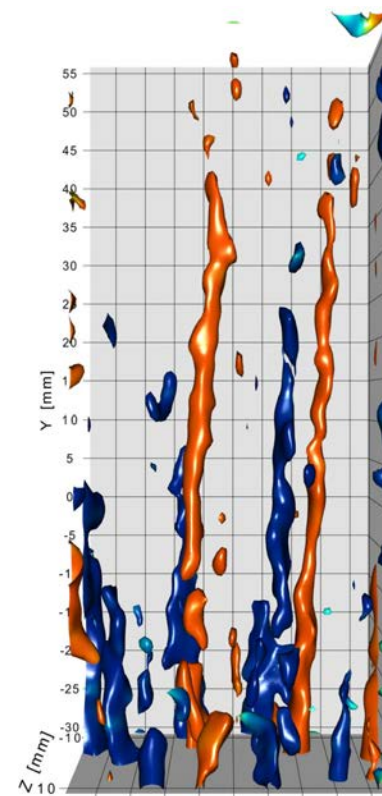

54914

79

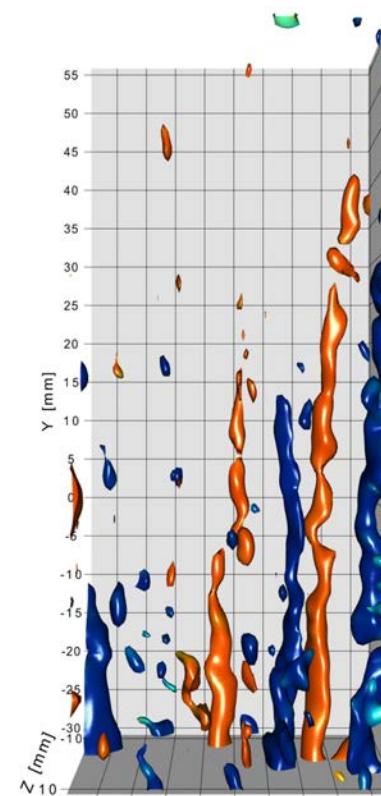

55081

80



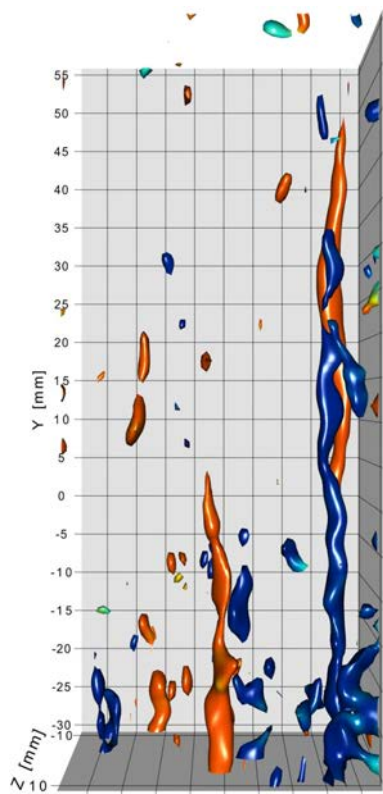

55378

81

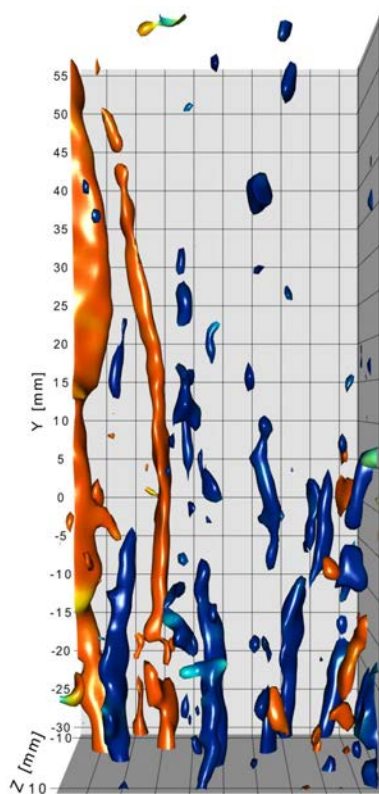

56884

82

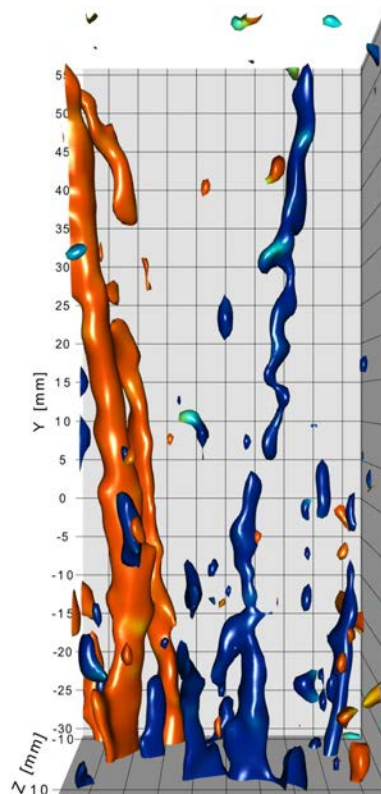

56994

83

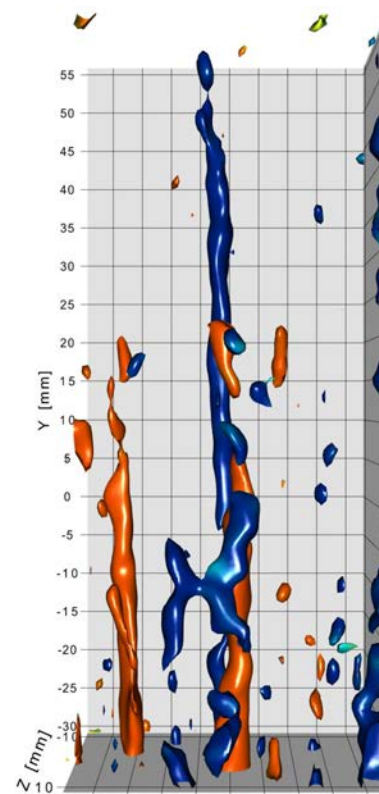

60250

84

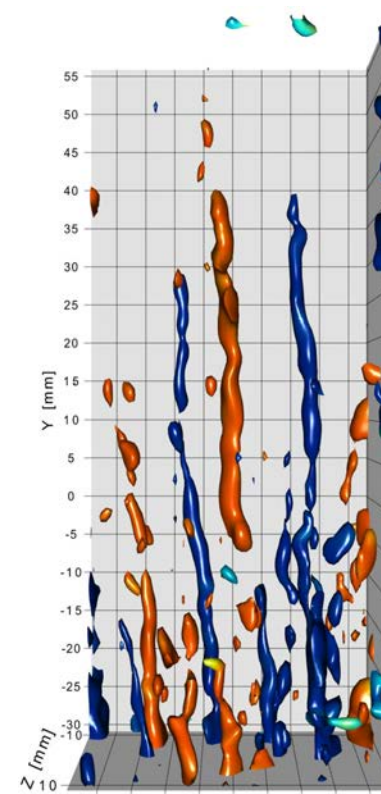

64276

85

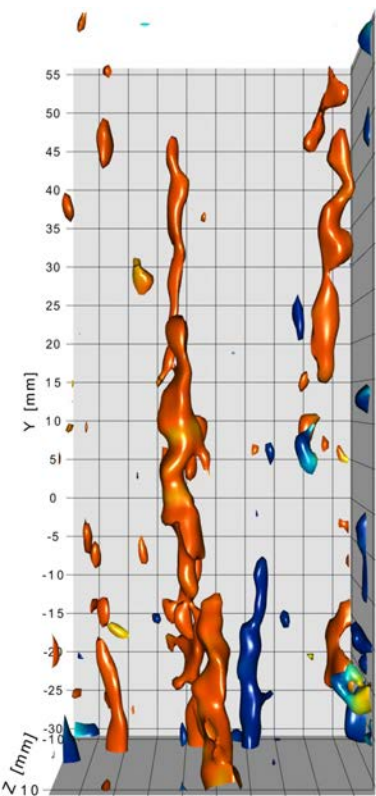

64478

86

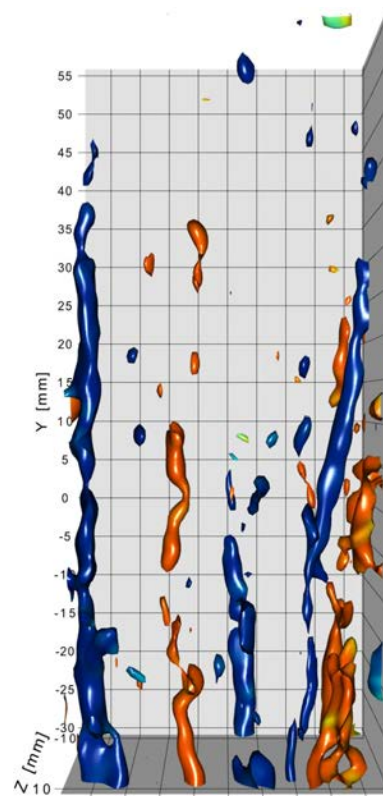

65499

87

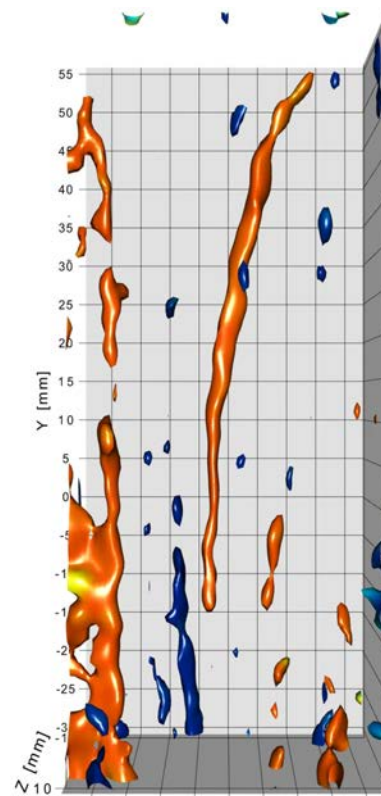

66684

88

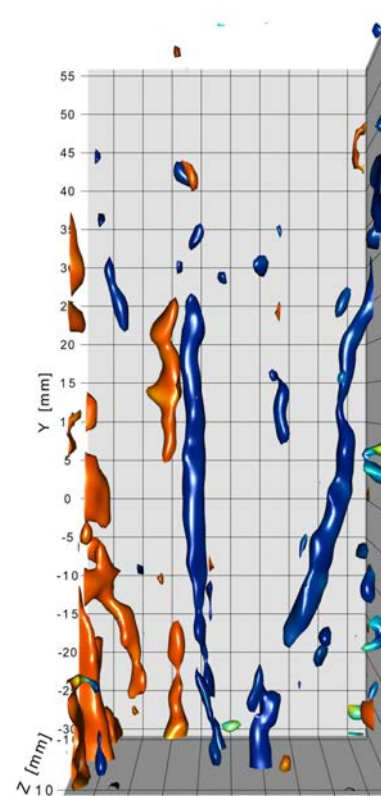

67153

89

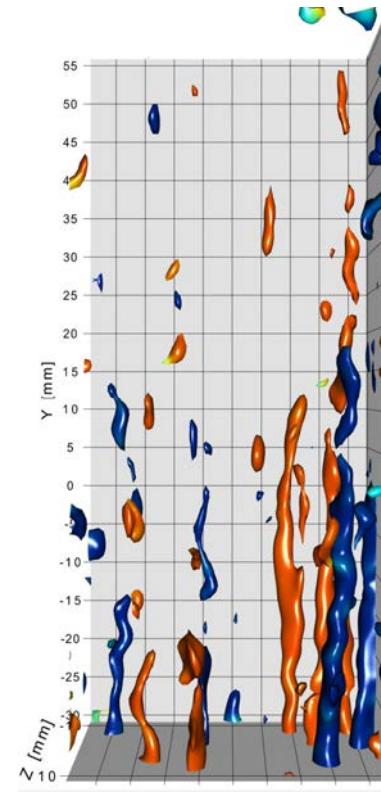

68272

90



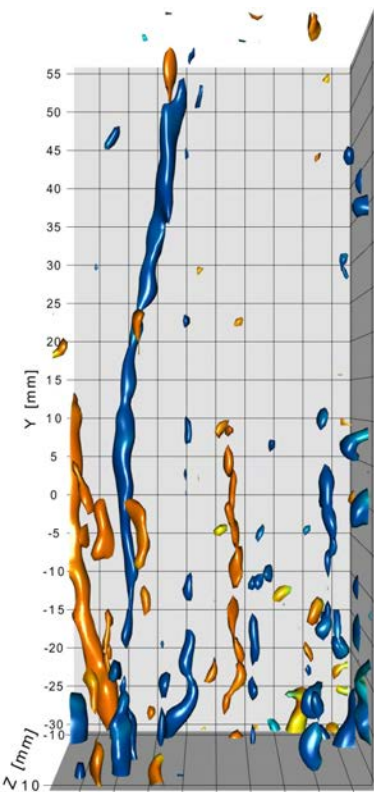

69257

91

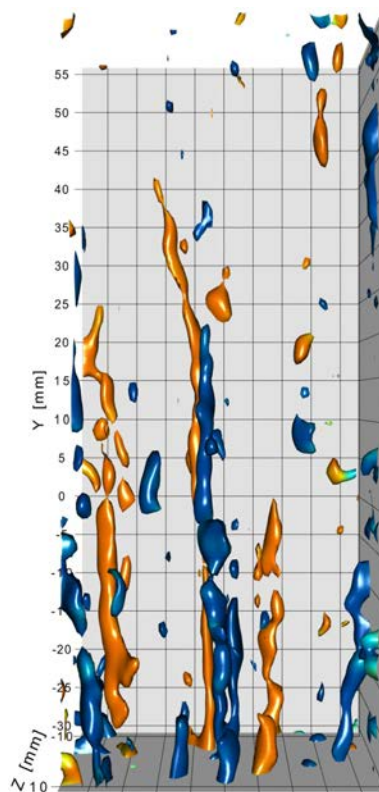

69489

92

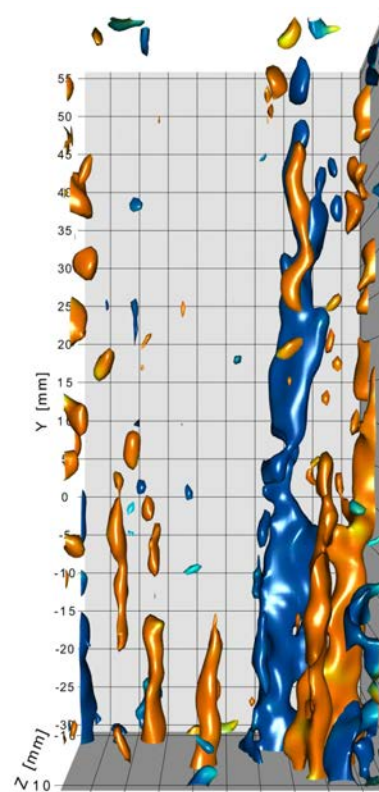

70450

93

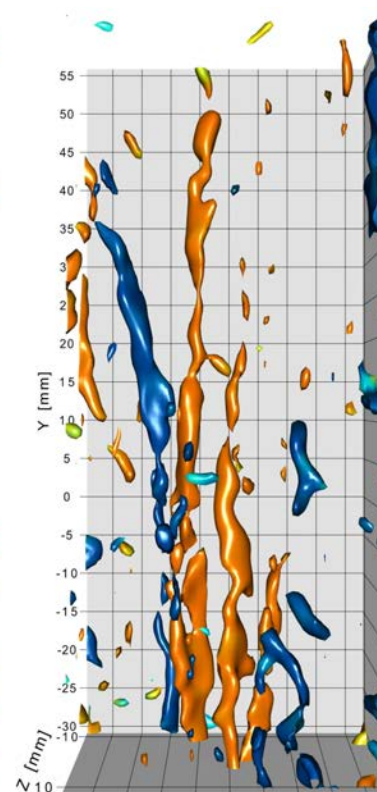

71198

94

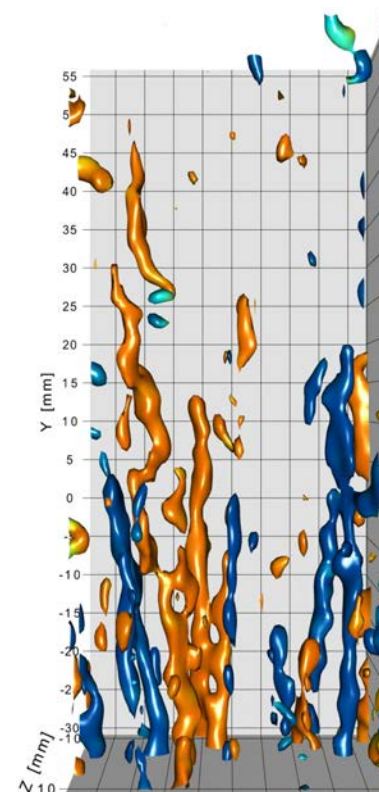

71579

95



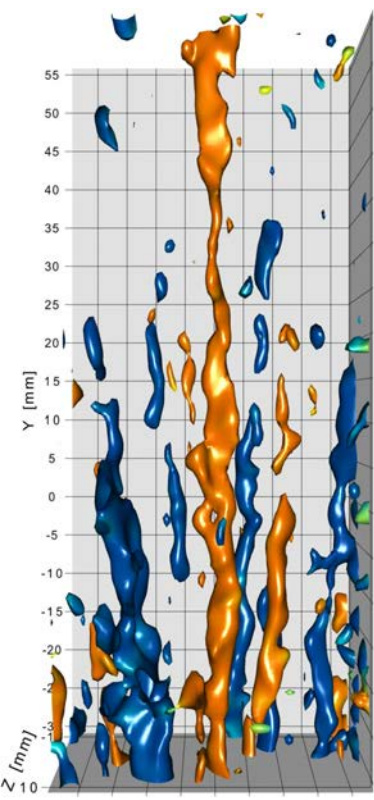

72484

96

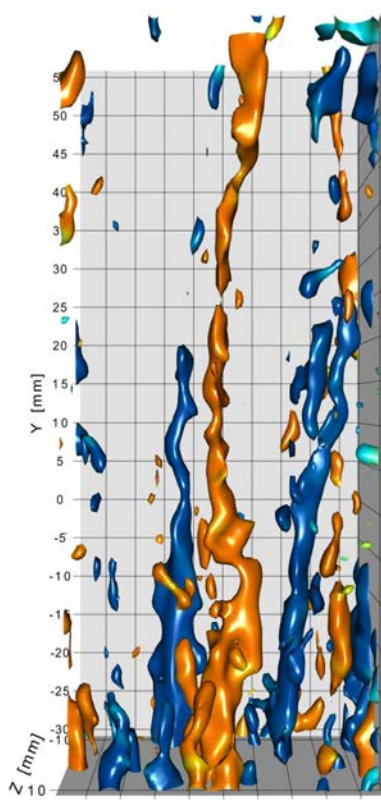

72739

97

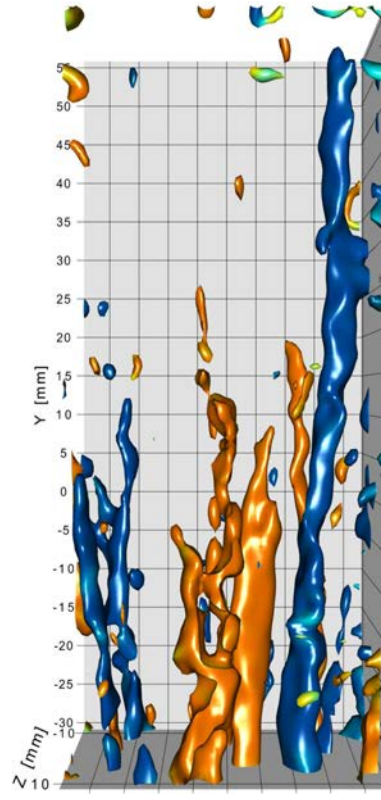

72945

98

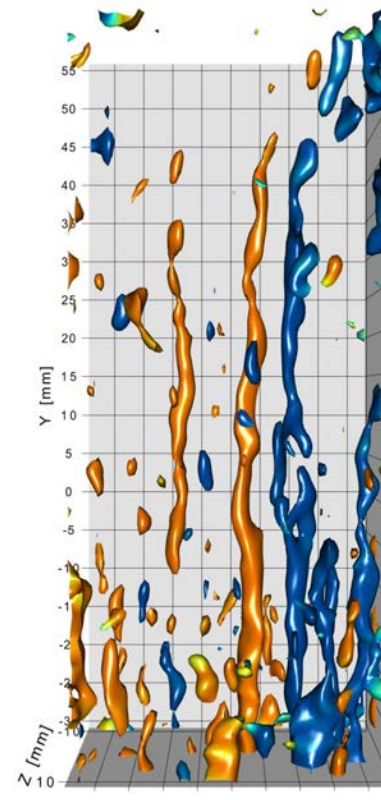

73271

99

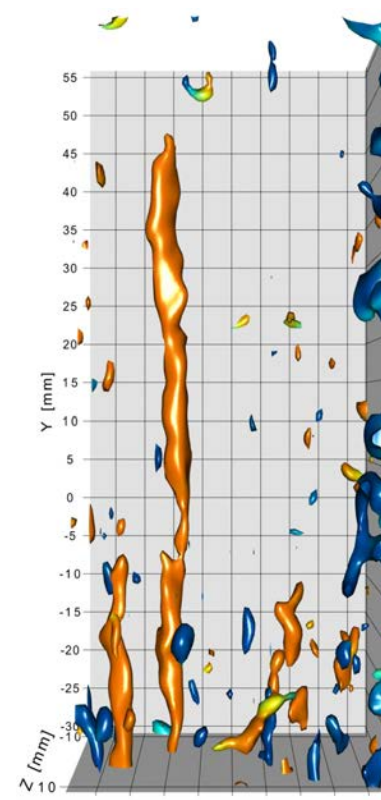

74314

100

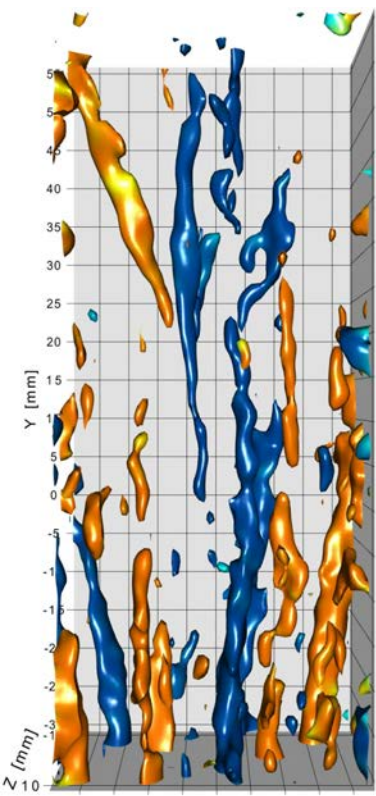

76515

101

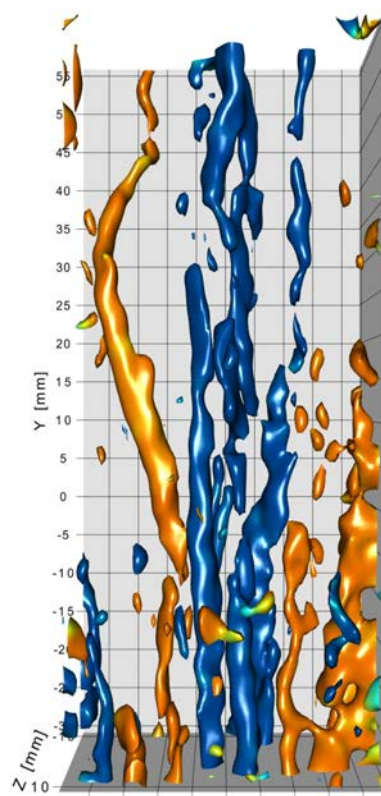

76612

102

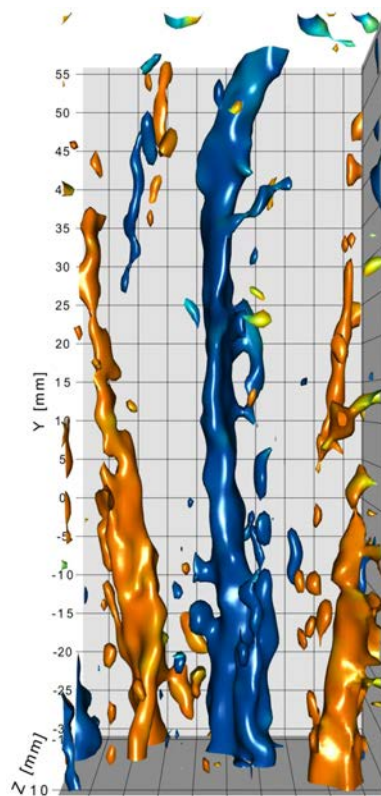

76943

103

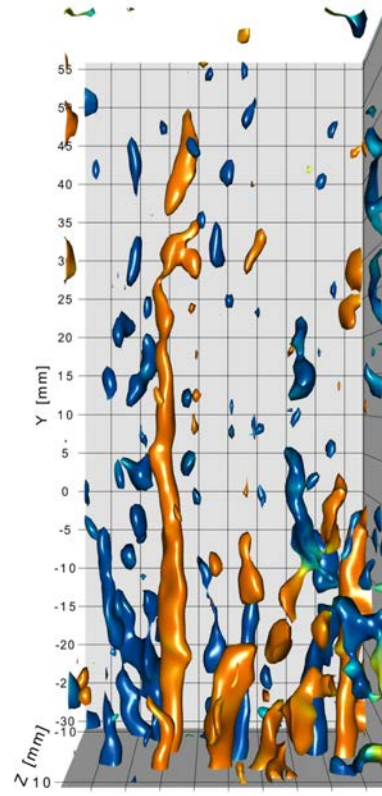

77746

104

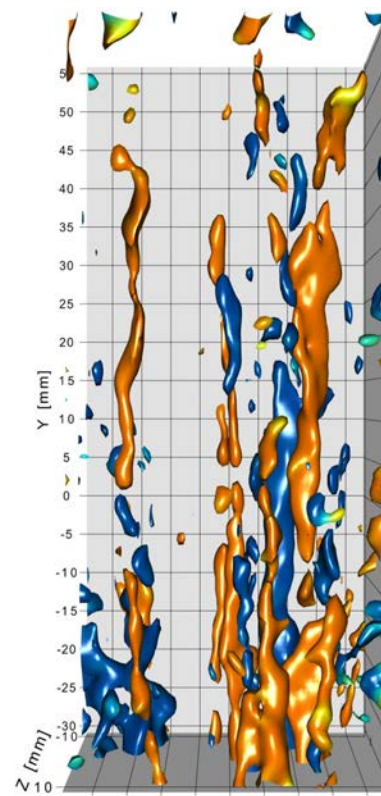

78028

105



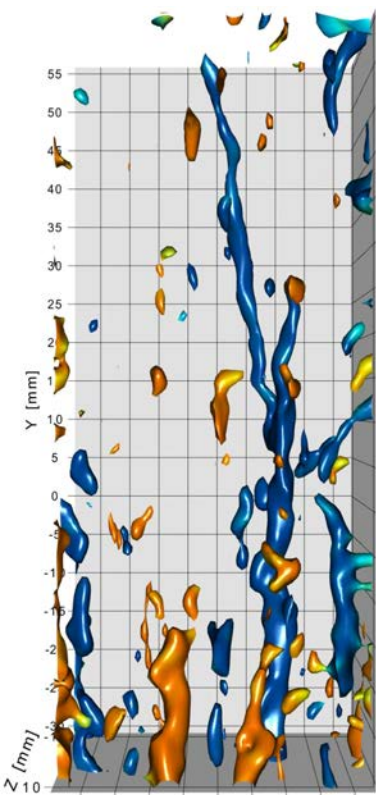

78629

106

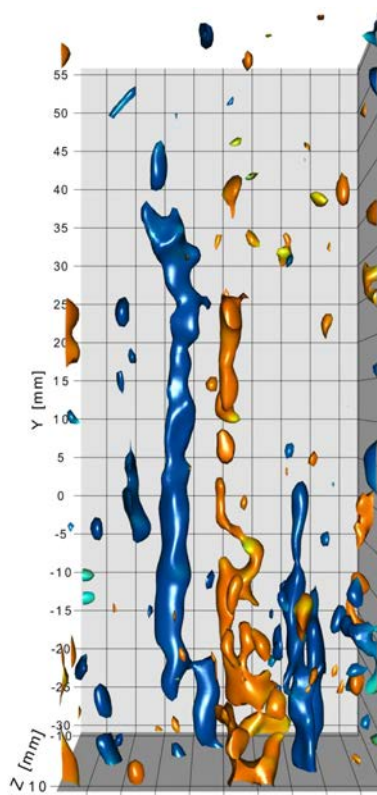

79025

107

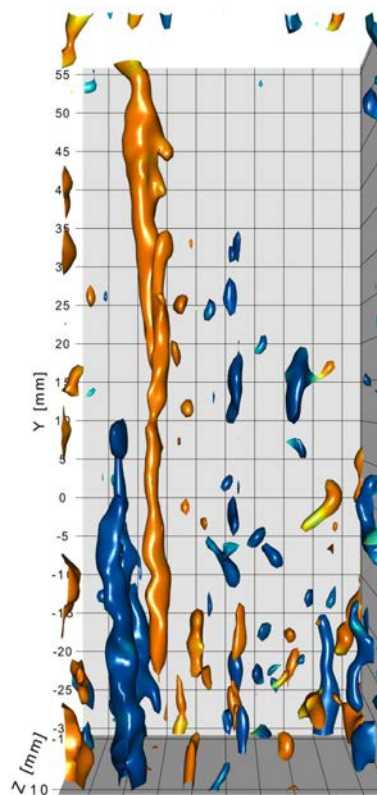

81725

108

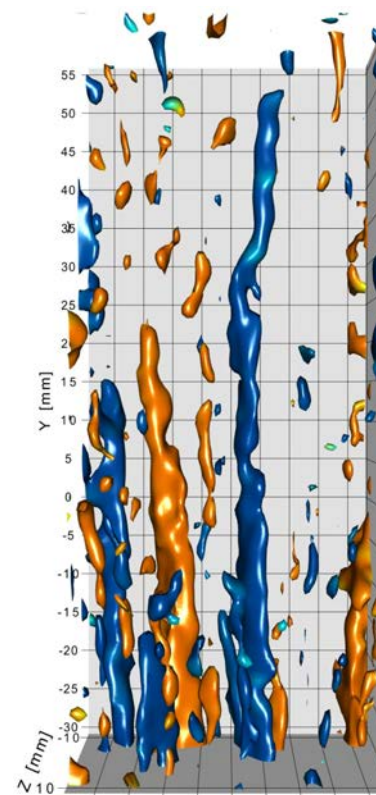

82000

109

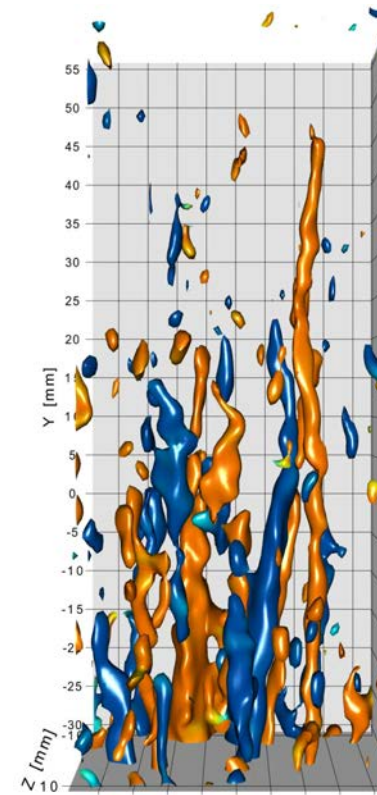

82186

110

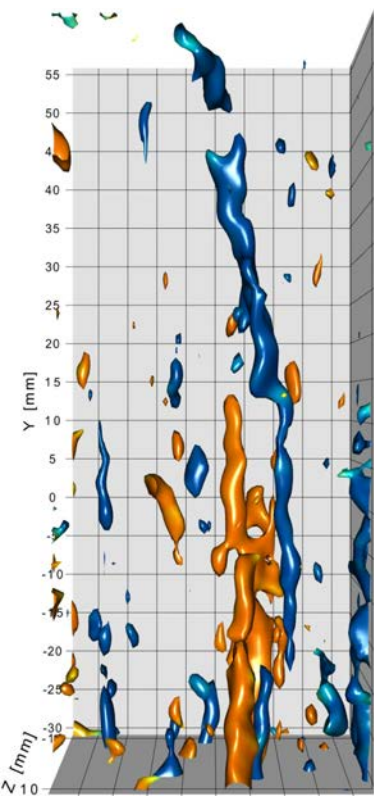

82618

111

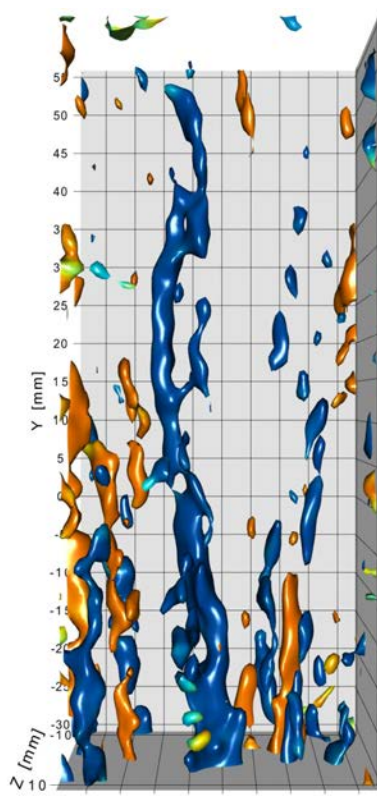

82934

112

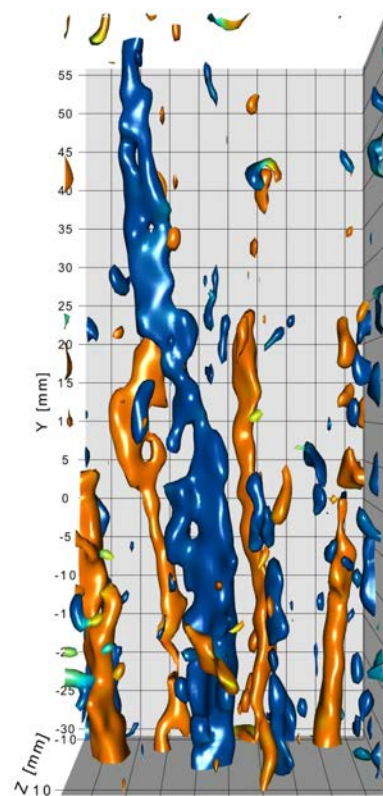

83096

113

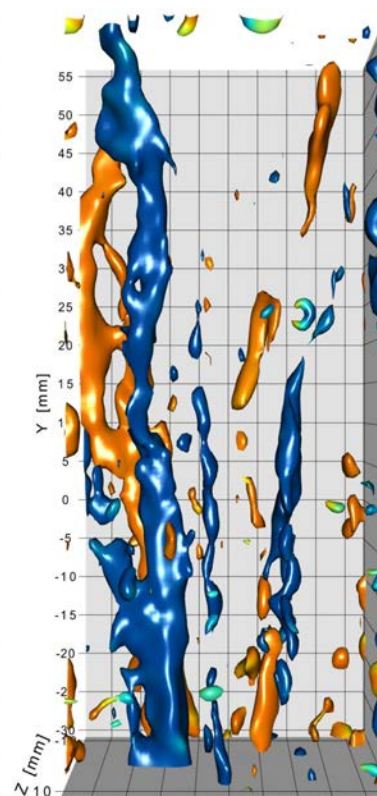

83280

114

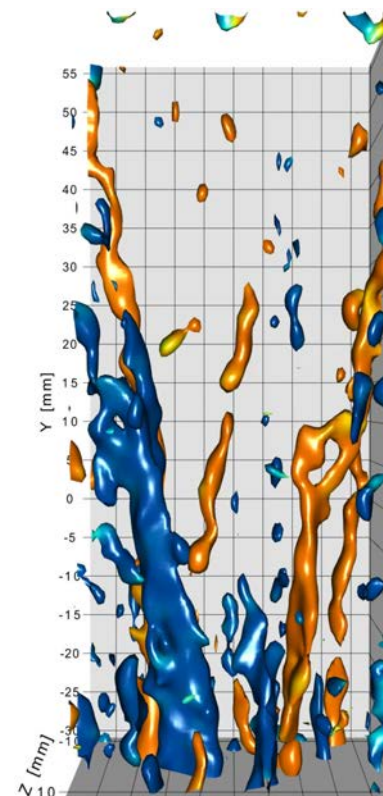

83450

115



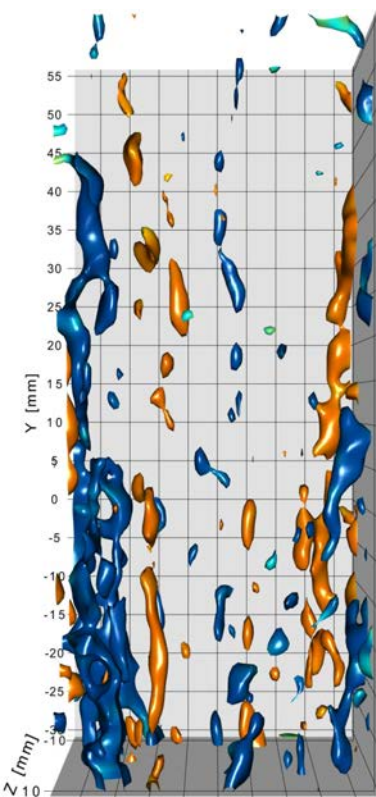

83741

116

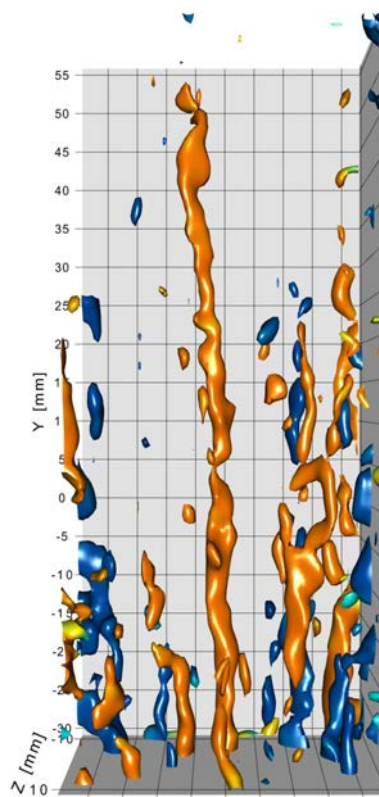

84776

117

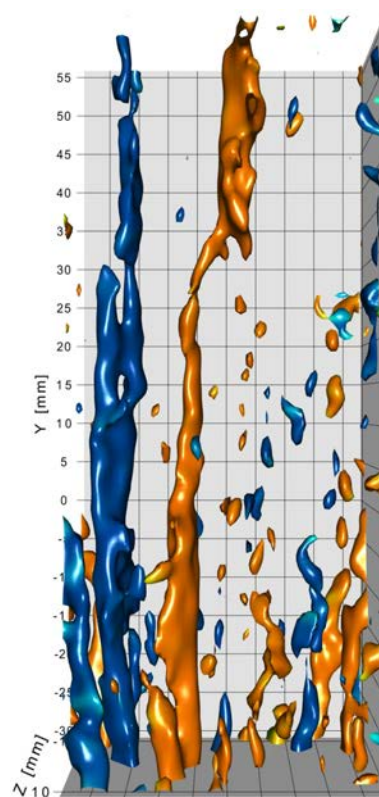

86341

118

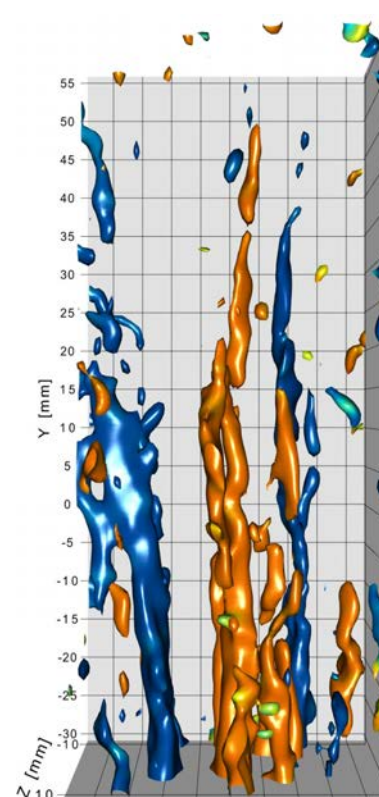

86639

119

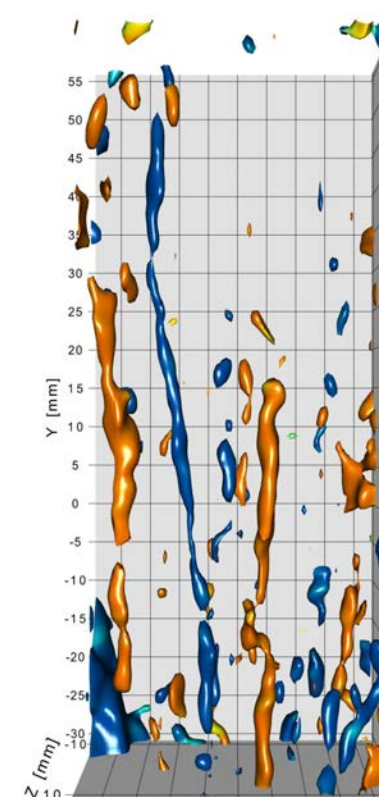

88067

120

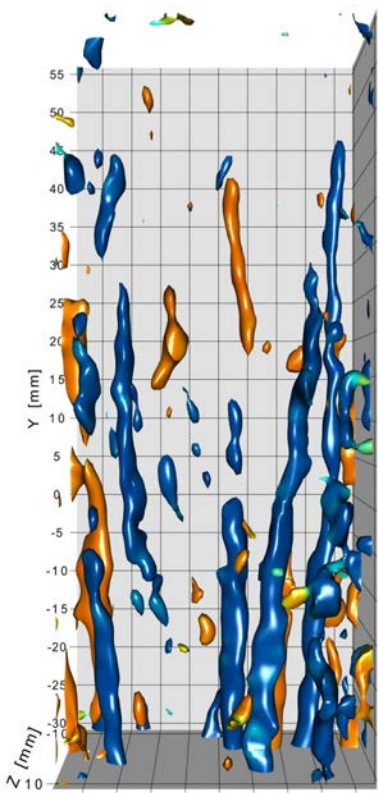

88607

121

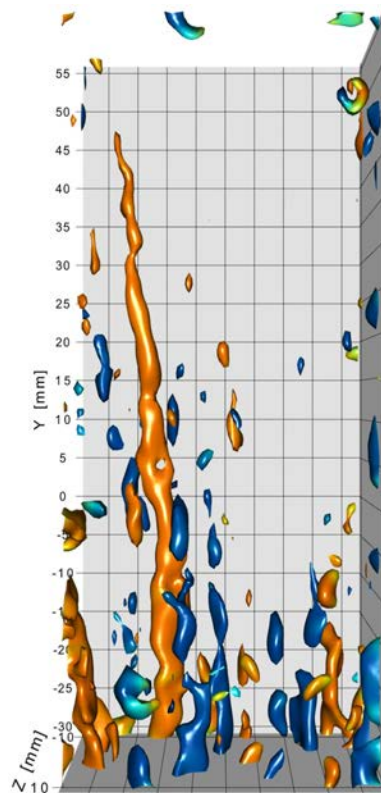

92881

122

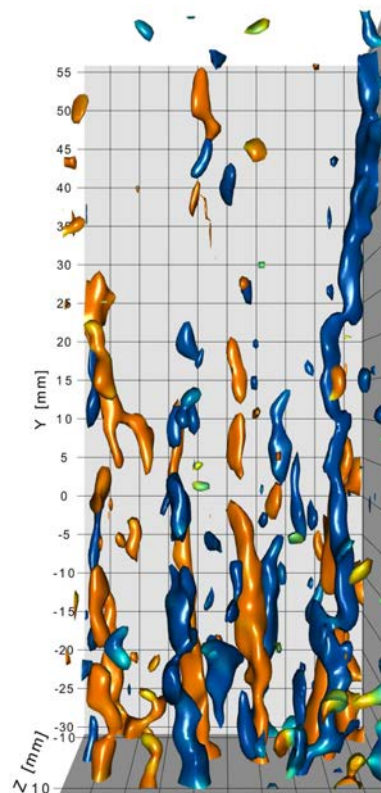

93479

123

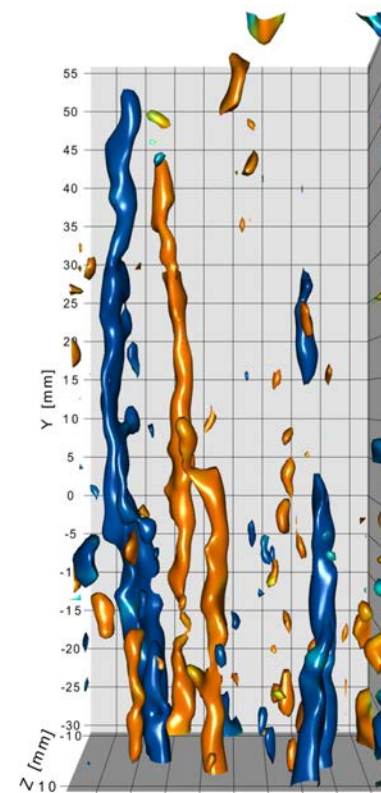

93912

124

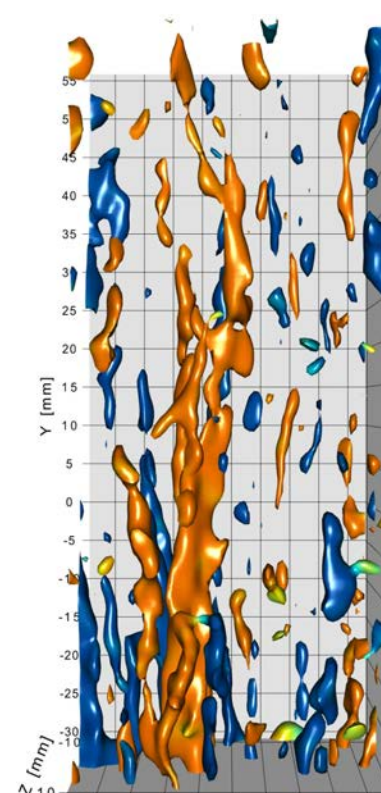

94294

125



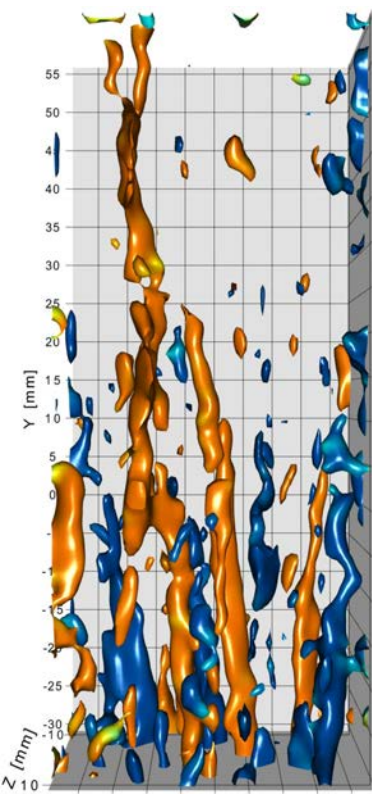

94521

126

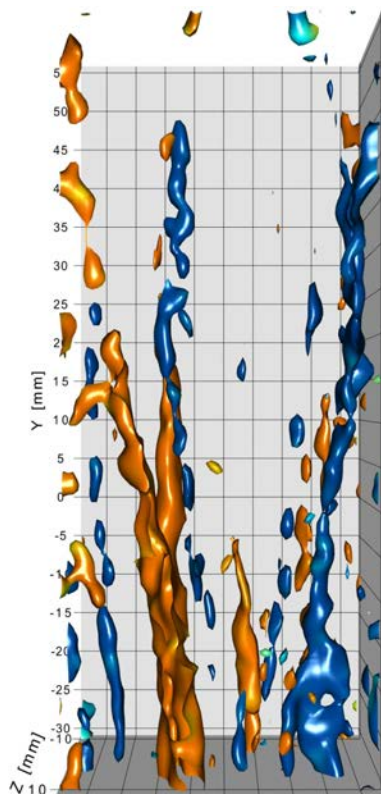

94681

127

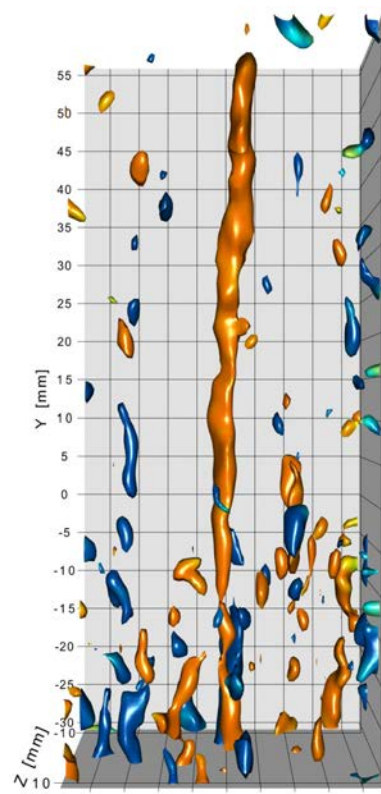

96565

128

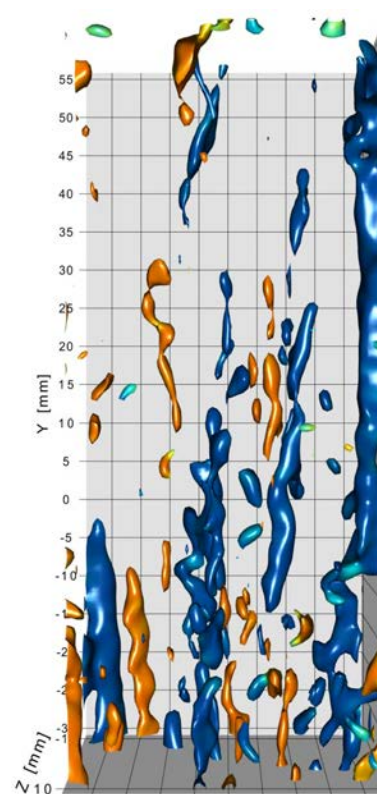

97589

129

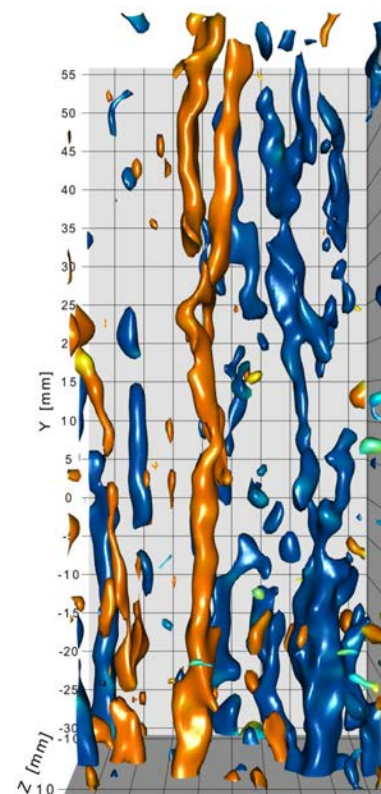

97772

130

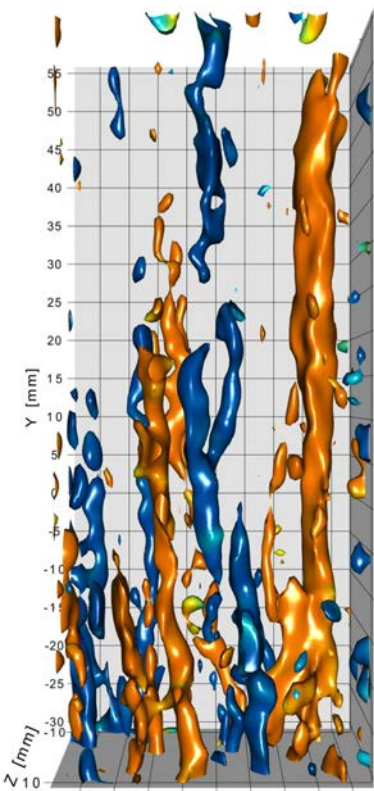

98302

131

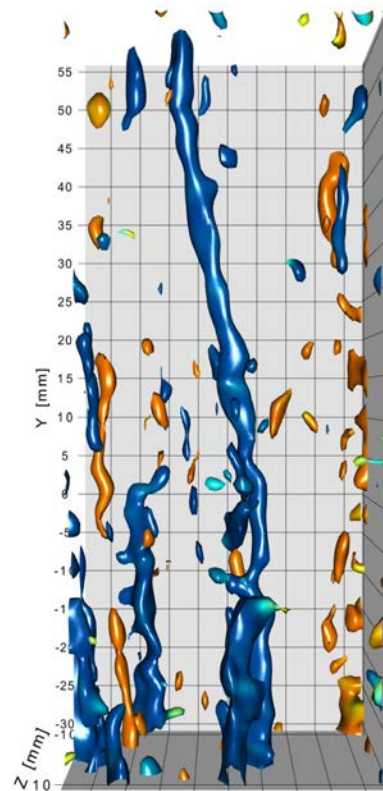

98981

132

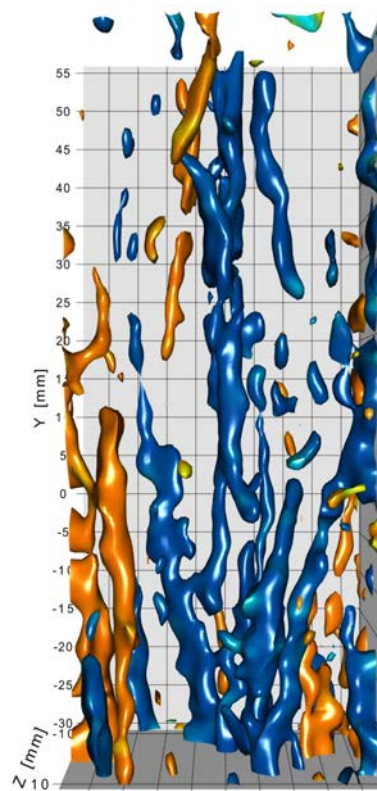

99400

133

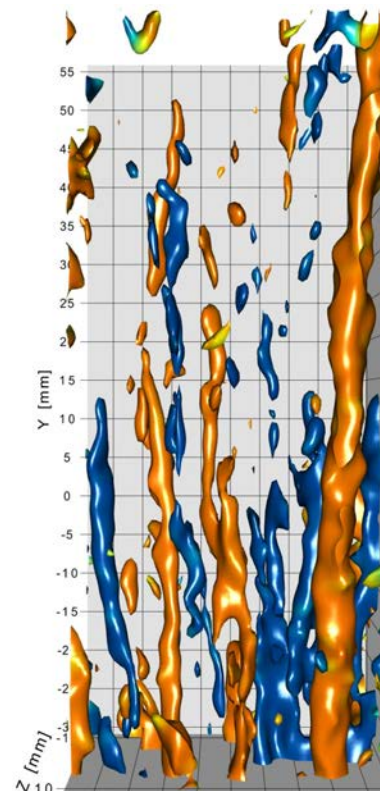

100125

134

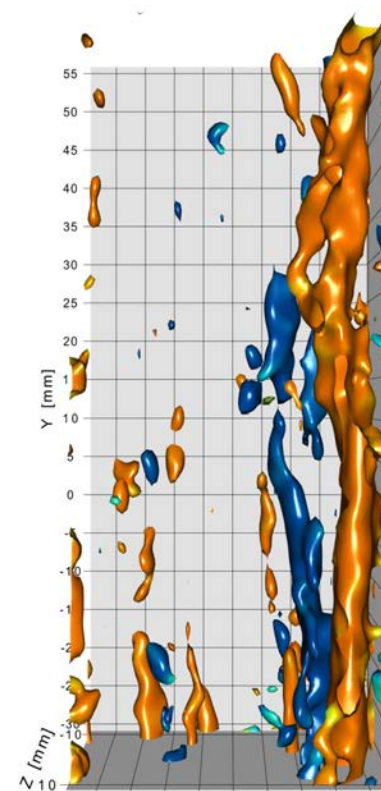

100473

135



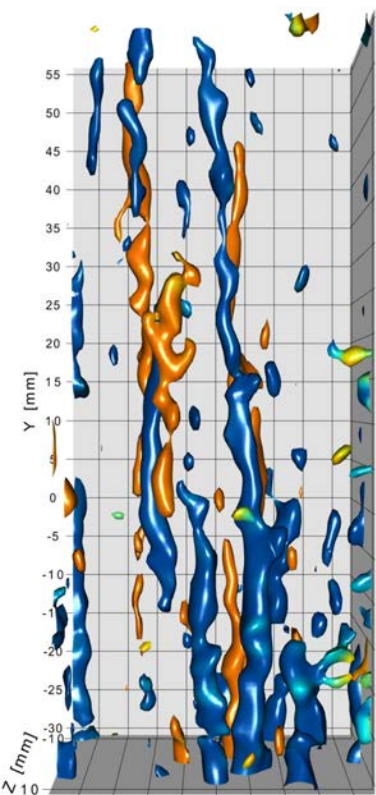

102237

136

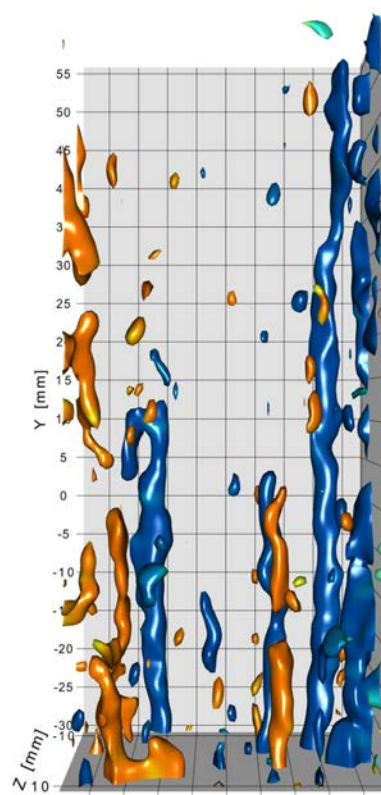

102680

137

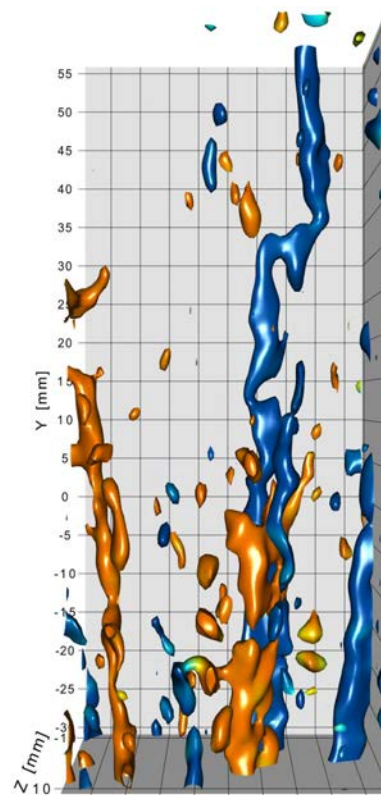

103225

138

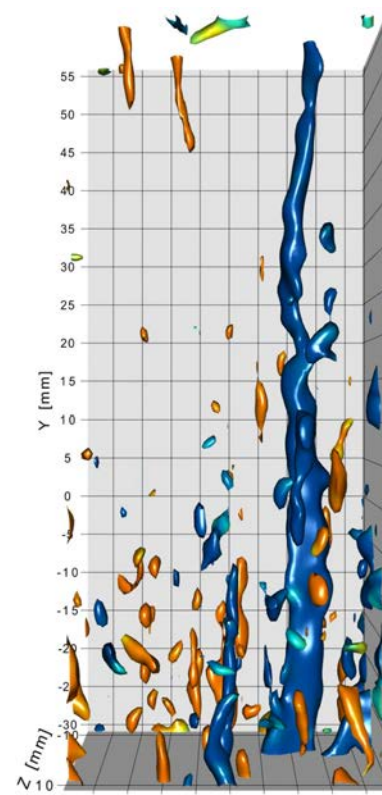

103396

139

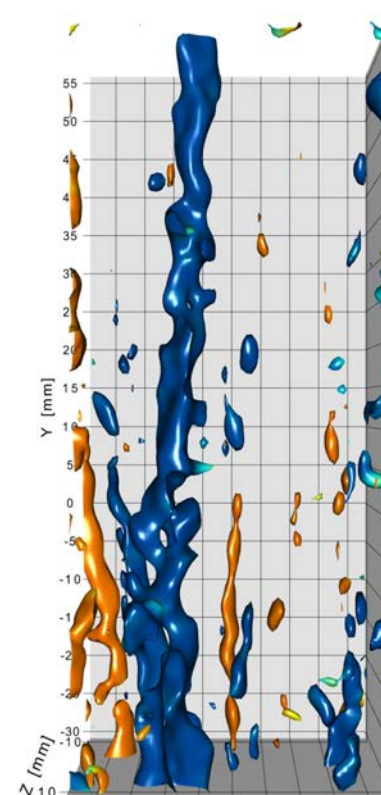

104094

140

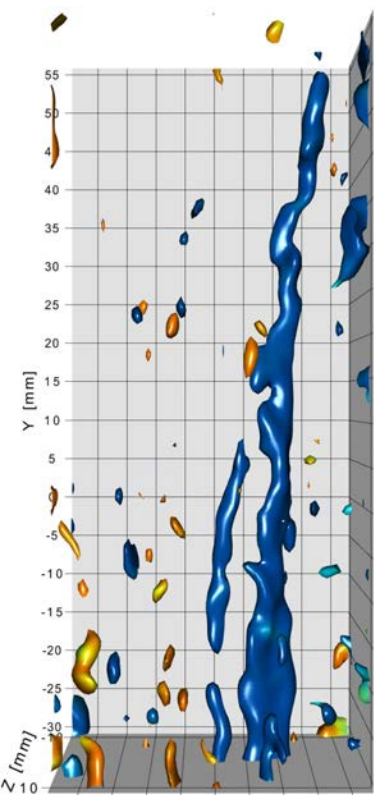

104750

141

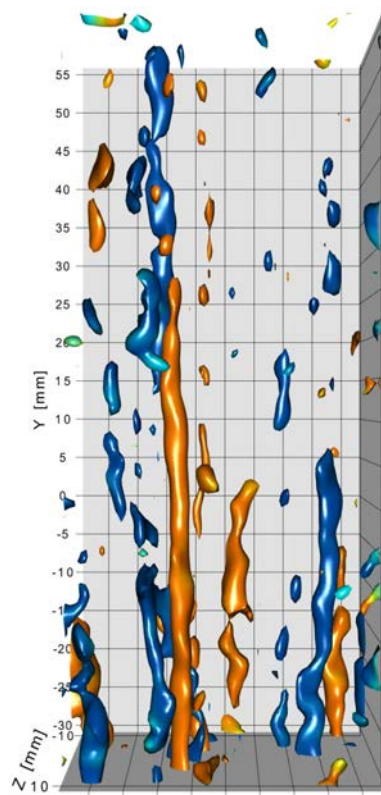

105381

142

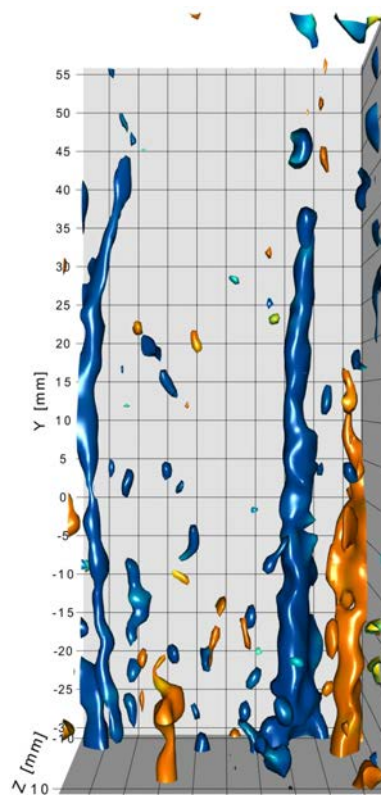

107131

143

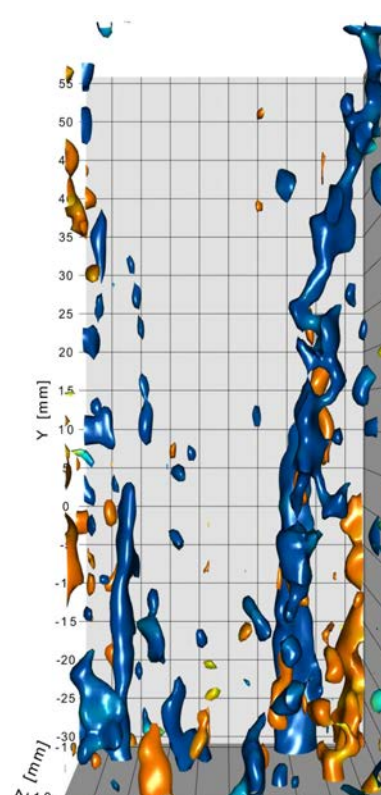

107229

144

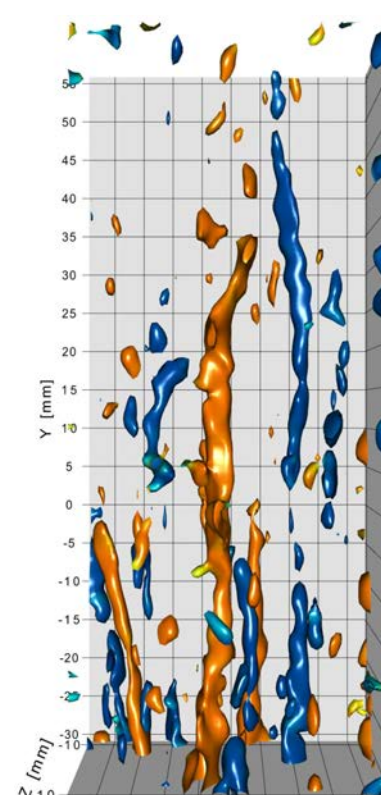

108459

145



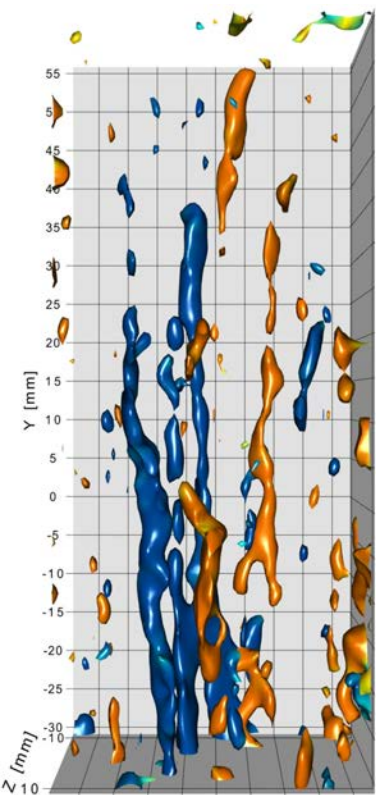

110406

146

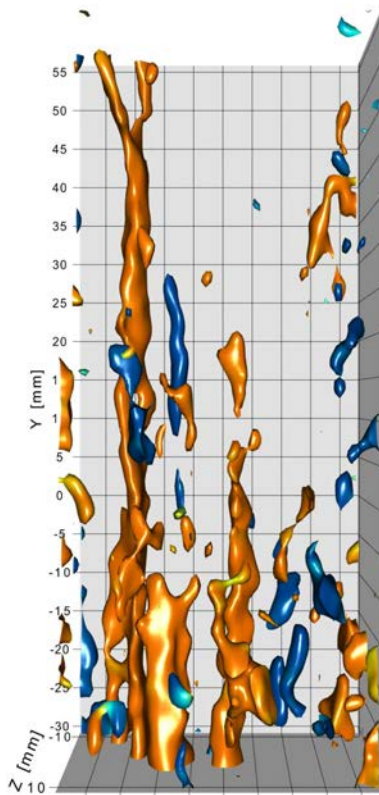

111310

147

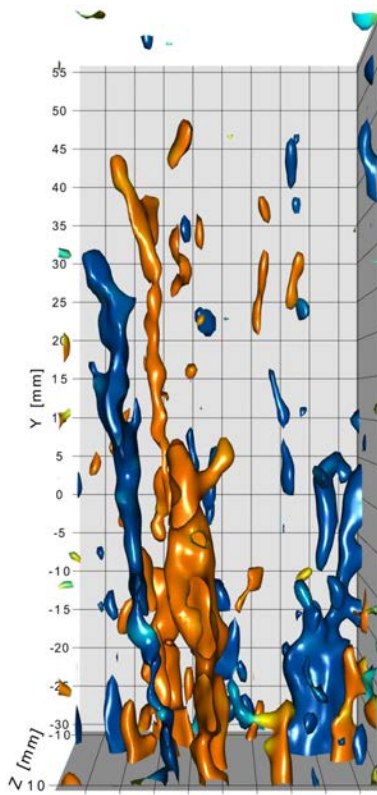

111585

148

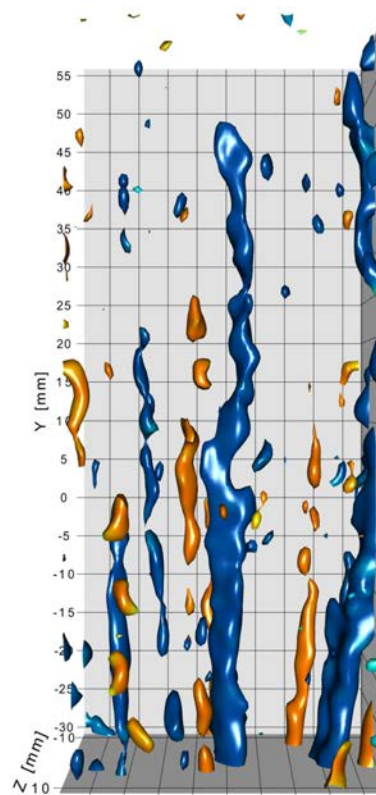

112051

149

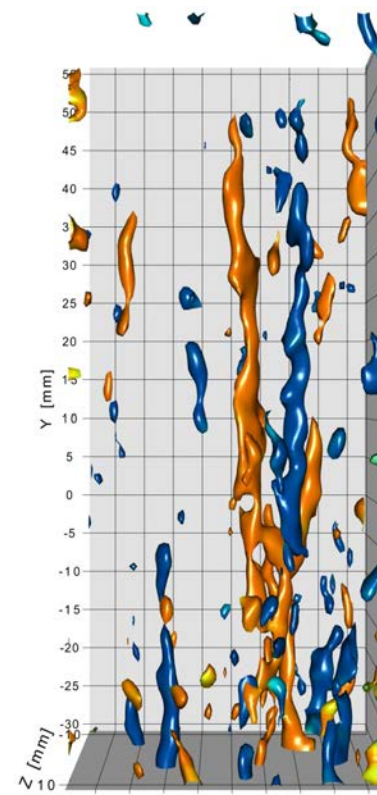

113333

150

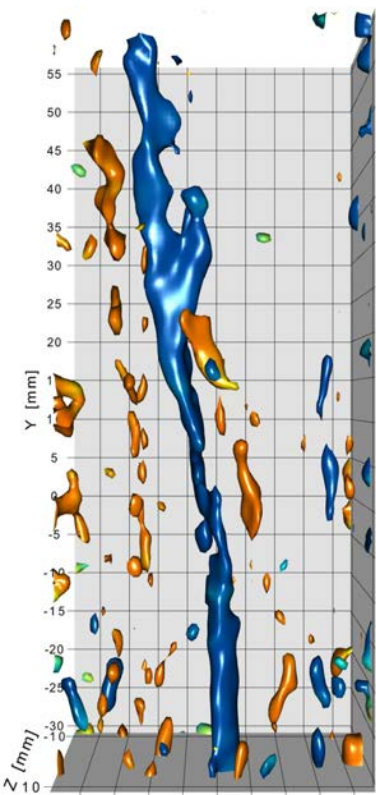

113746

151

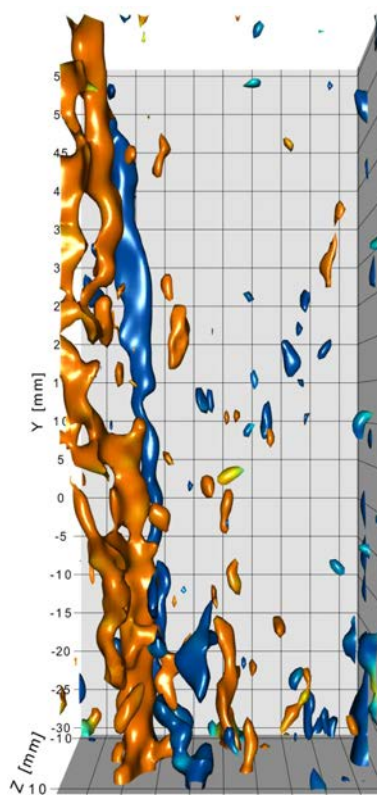

114158

152

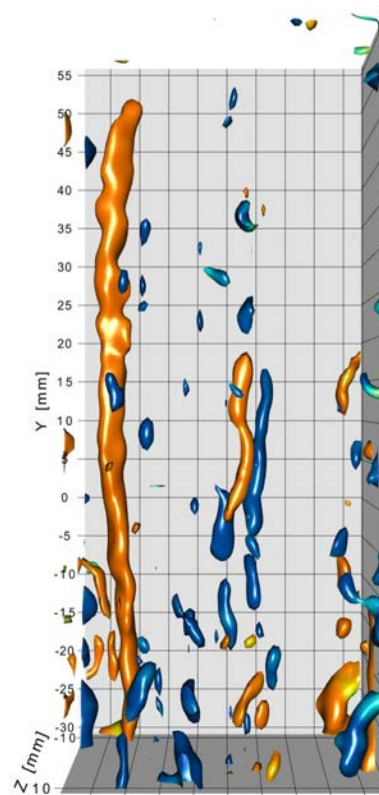

114881

153

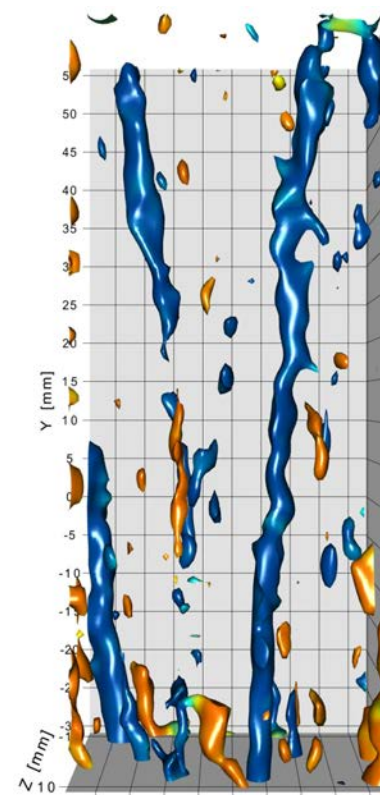

117083

154

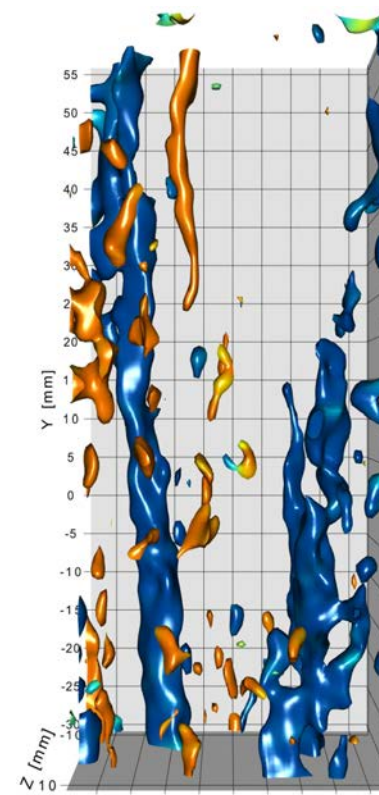

117289

155



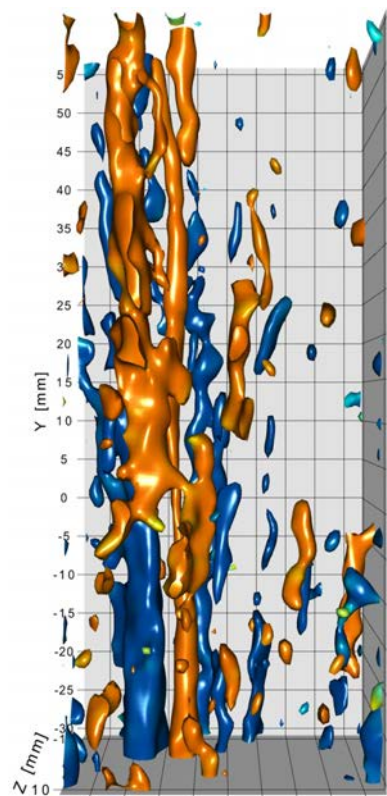

117524

156

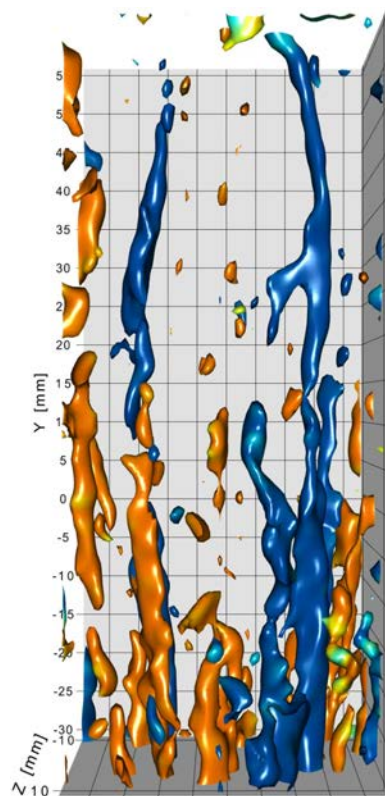

118005

157

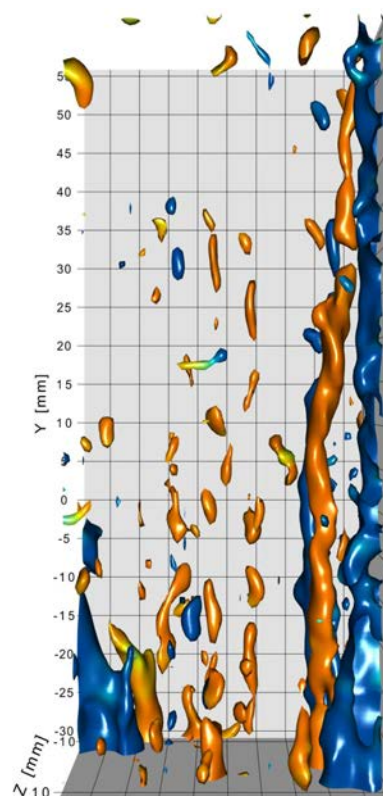

118321

158

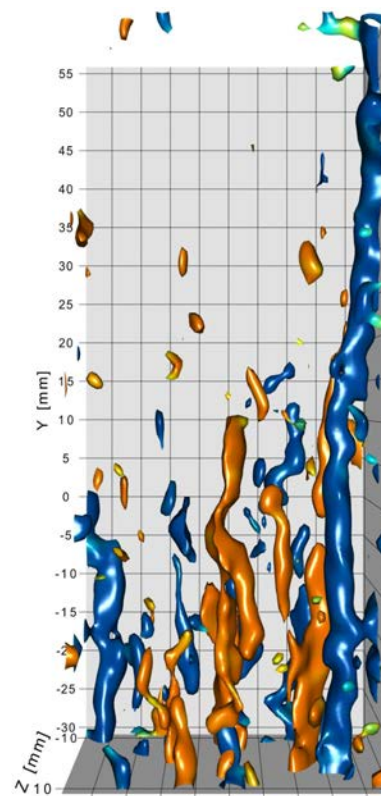

118463

159

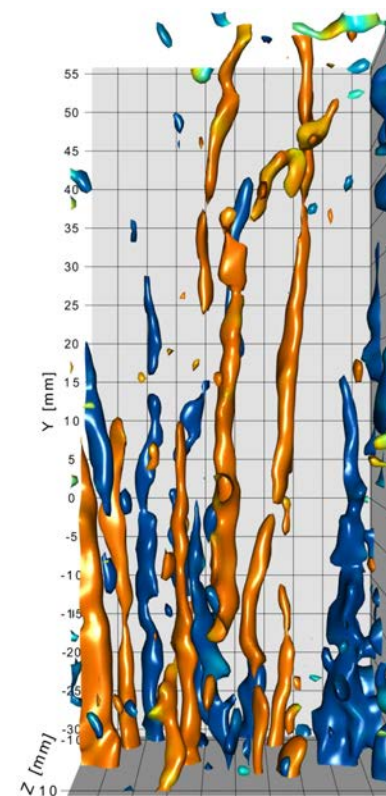

120129

160

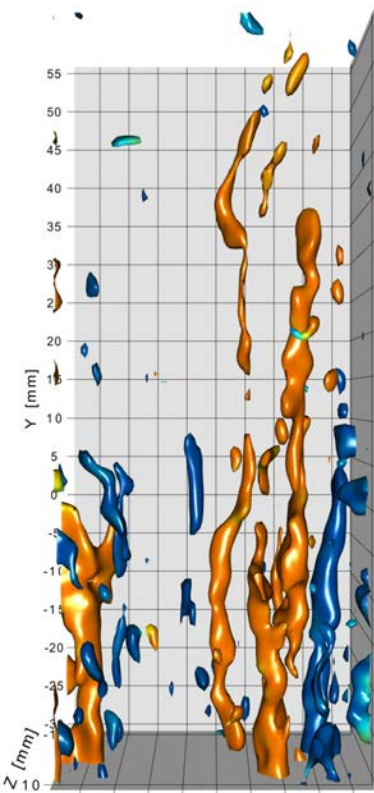

120429

161

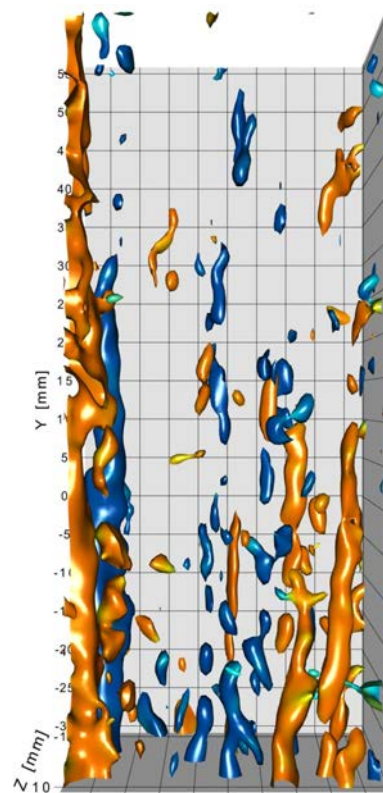

121323

162

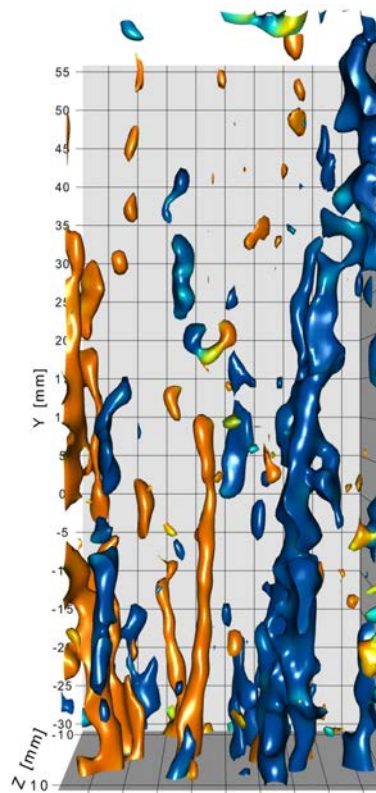

122988

163

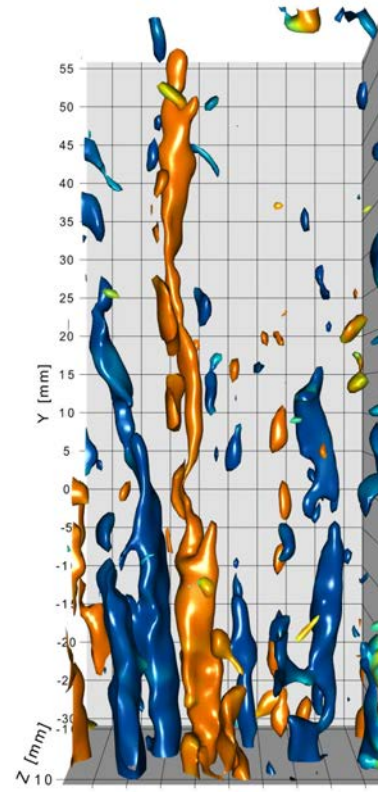

123921

164

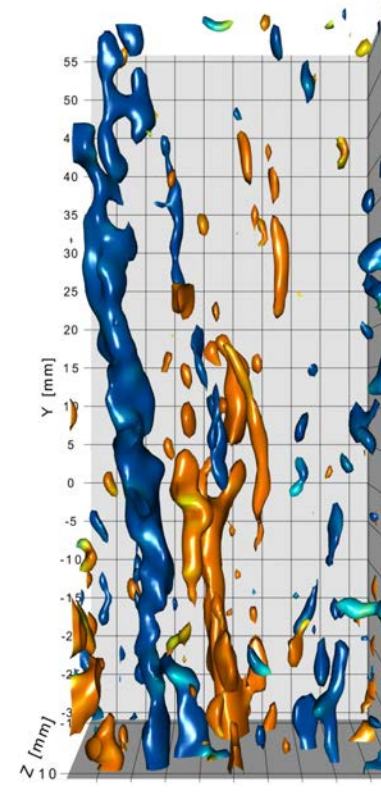

126285

165



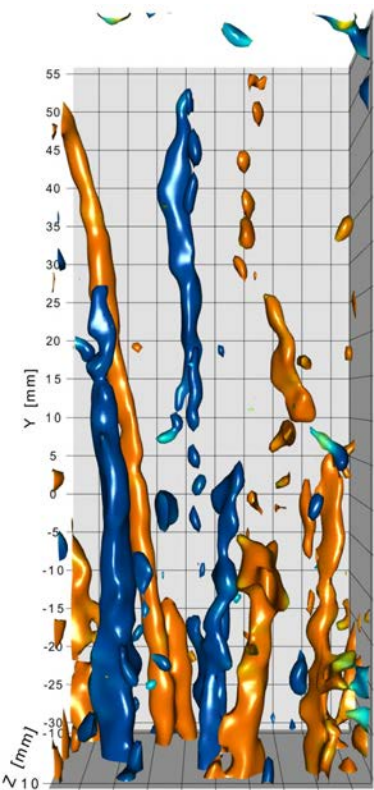

126701

166

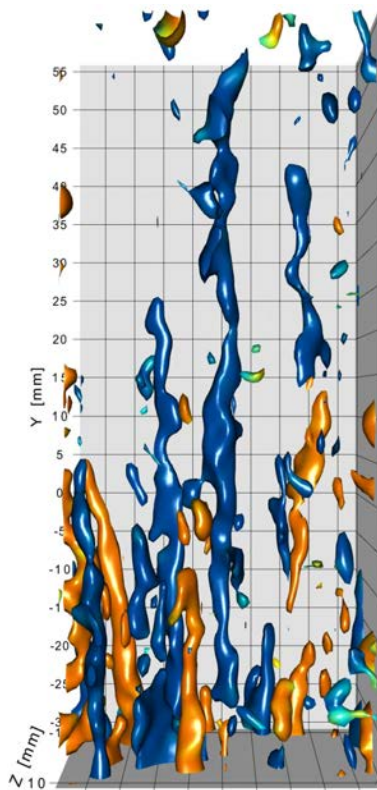

127575

167

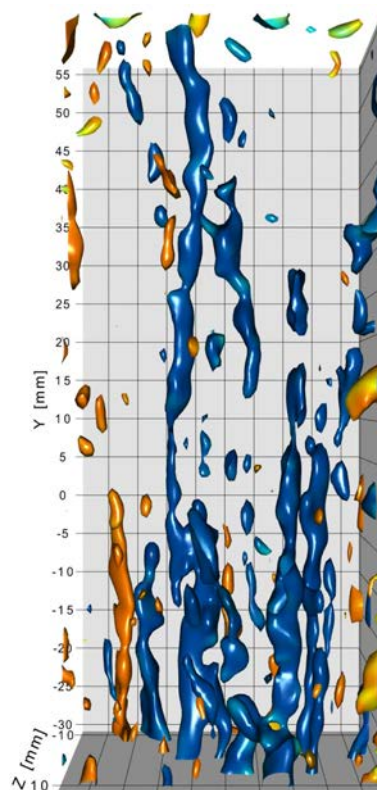

127818

168

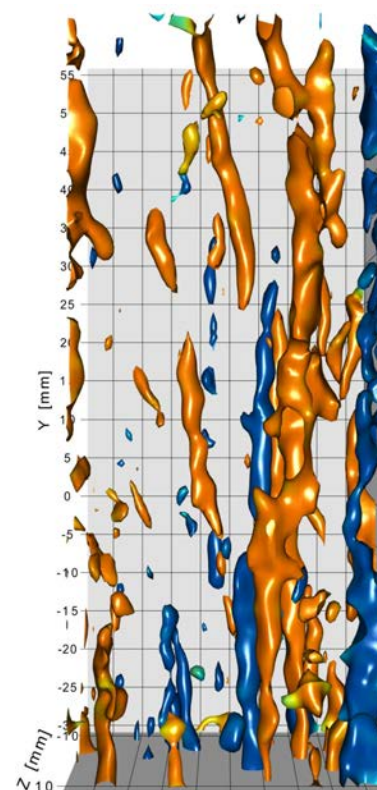

128842

169

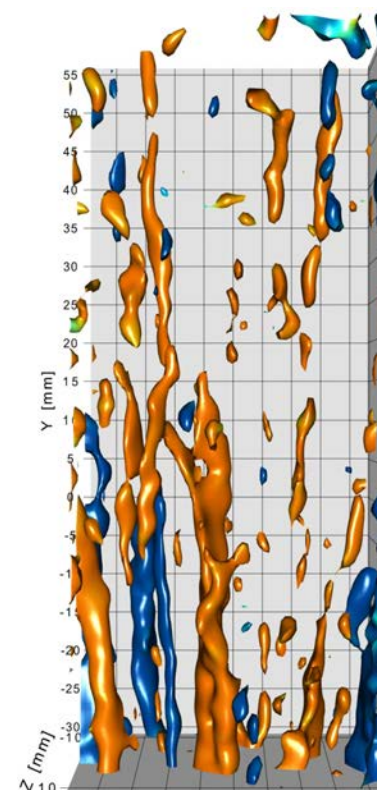

129136

170

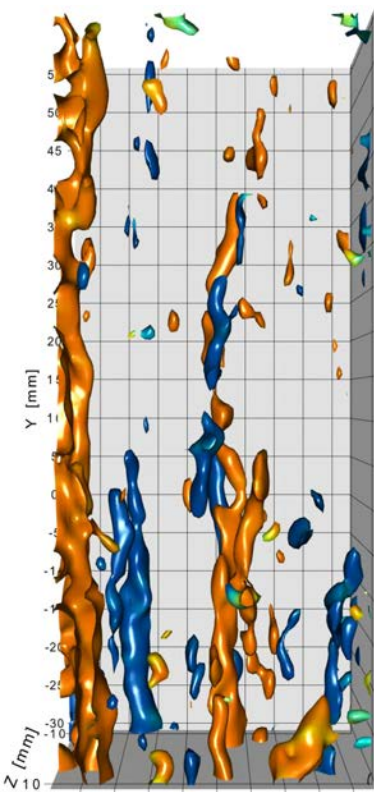

129757

171

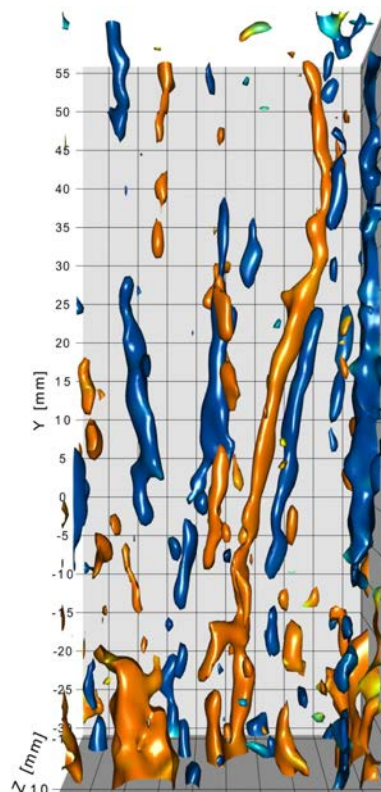

129963

172

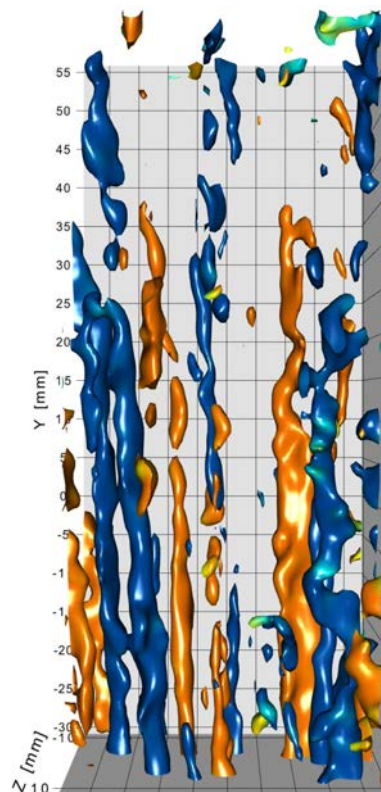

130122

173

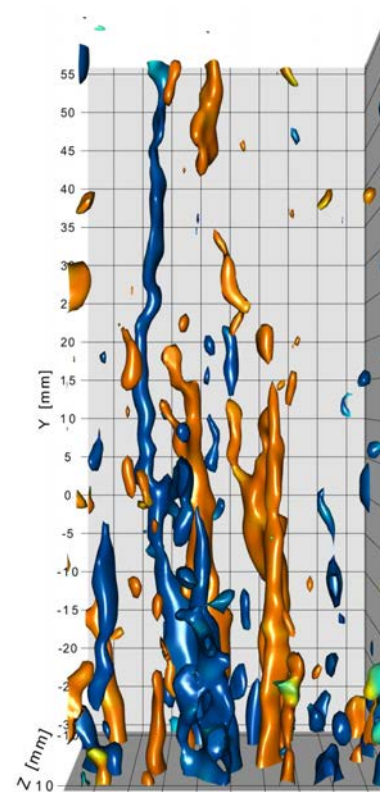

130455

174

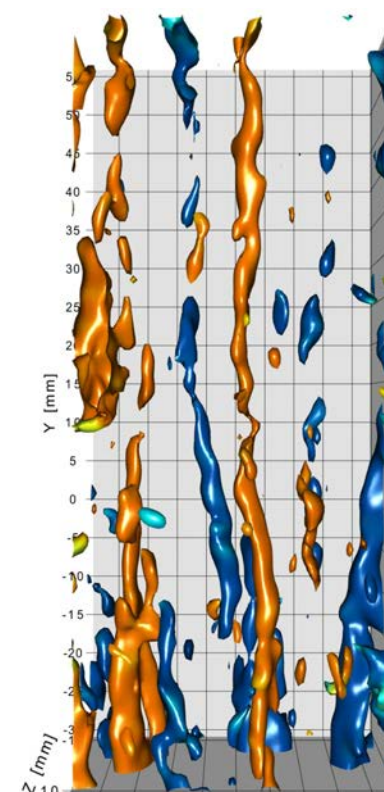

132132

175



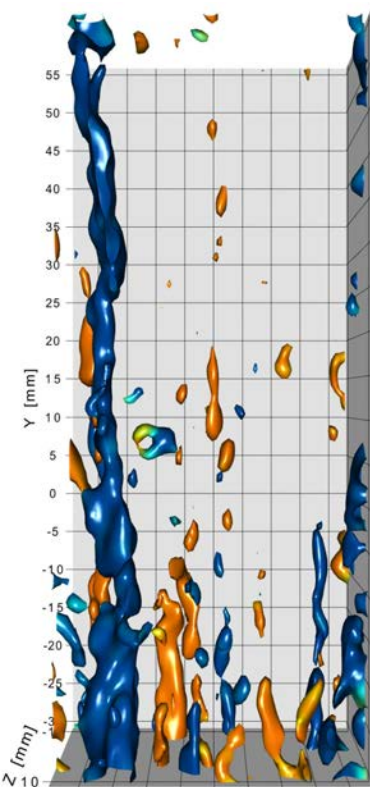

133235

176

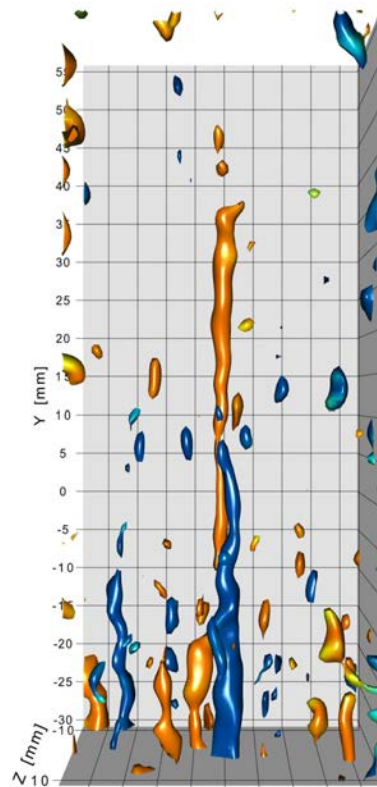

134244

177

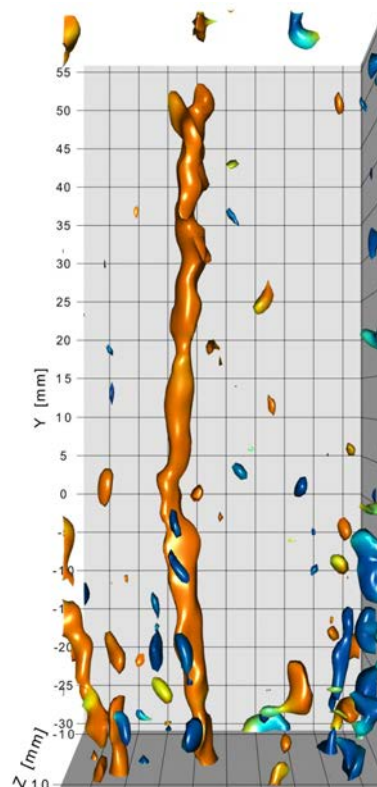

134487

178

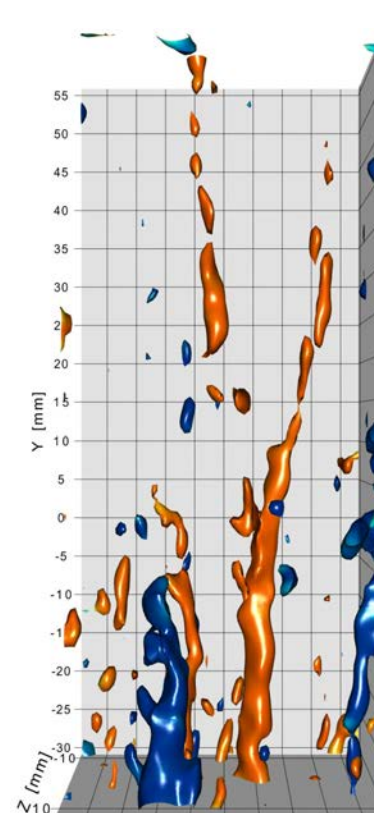

136268

179

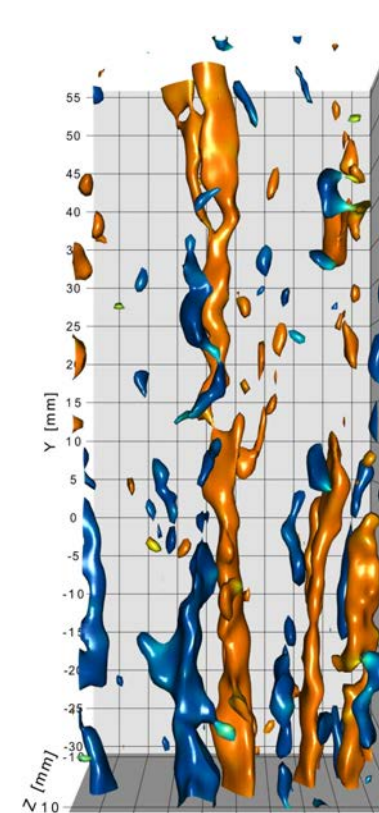

136375

180
