# Supplementary material for: Coherent turbulent structures in a rapid contraction
Source: arXiv:2401.05869 source file (2024-01-11)
Supplement: Supplementary file 2 [file StrRun2.pdf]

# Run2

Iso-surface of  $|\omega| = 40 \text{ } ^1/s$

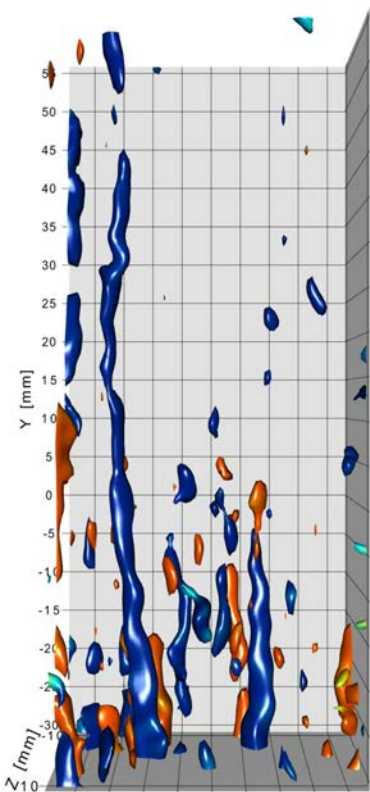

52

181

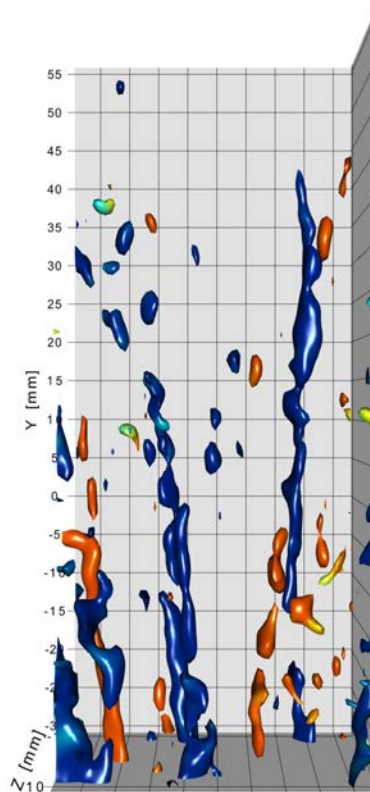

813

182

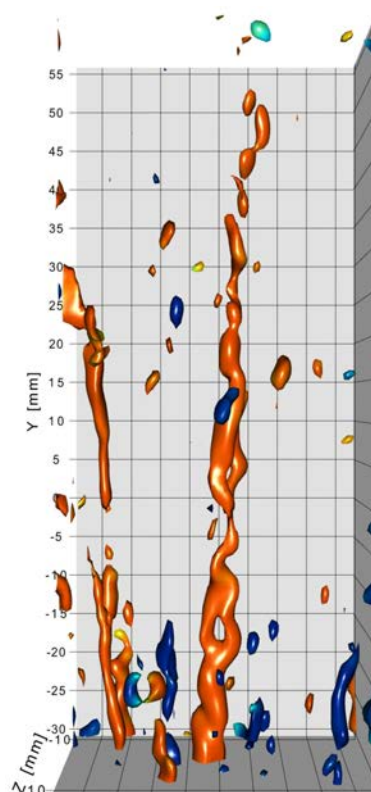

2657

183

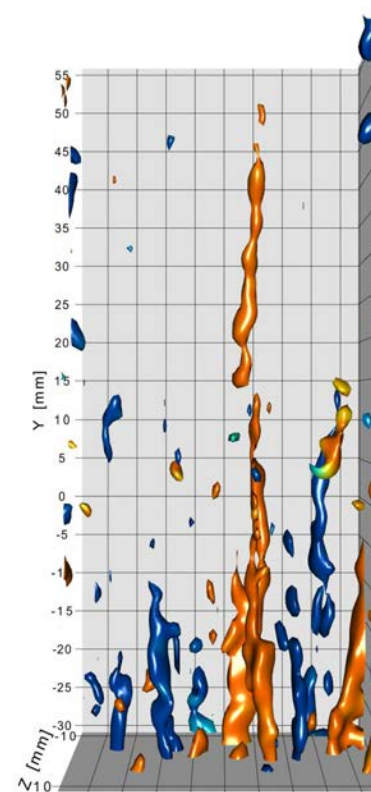

2945

184

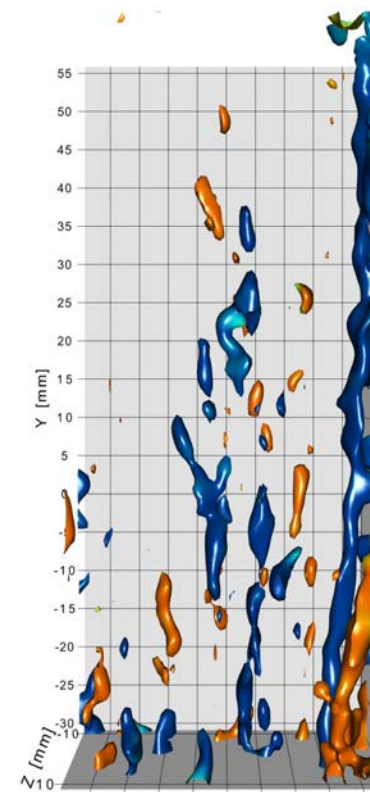

3566

185

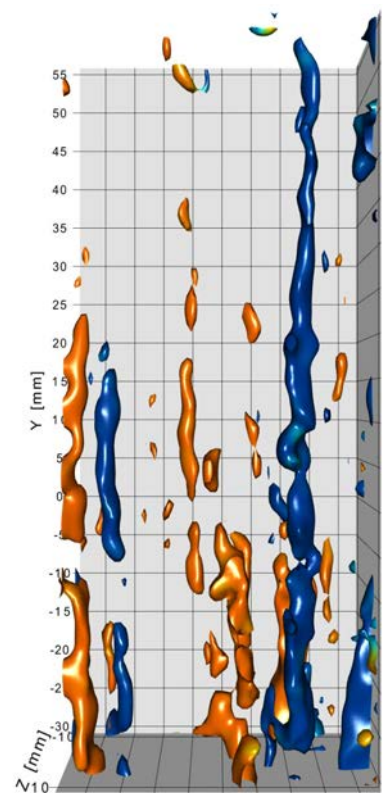

3999

186

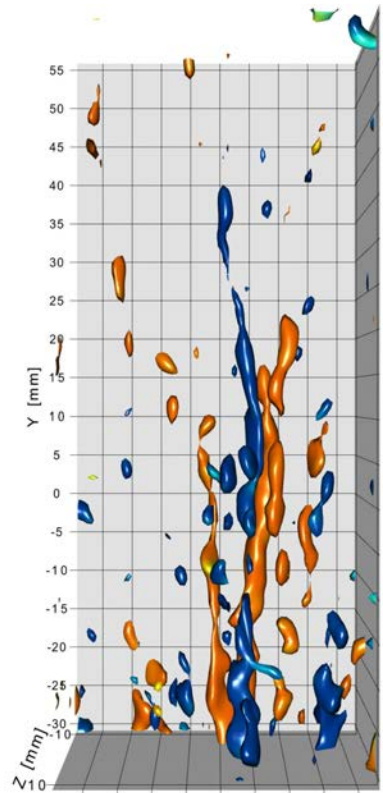

5247

187

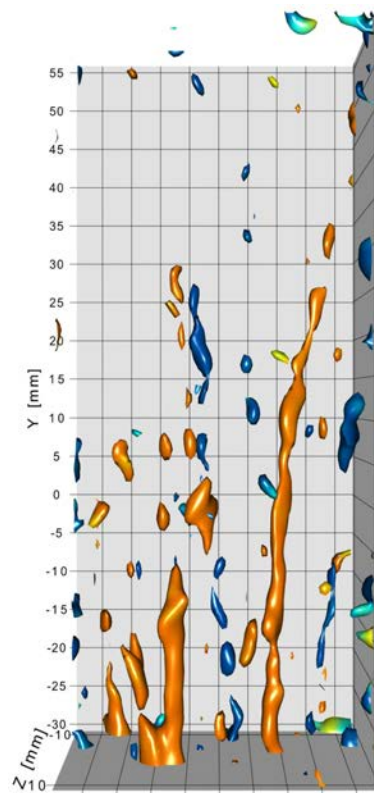

6720

188

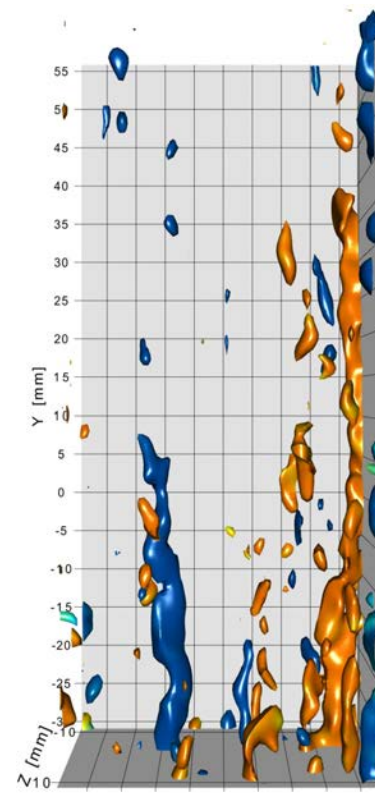

7206

189

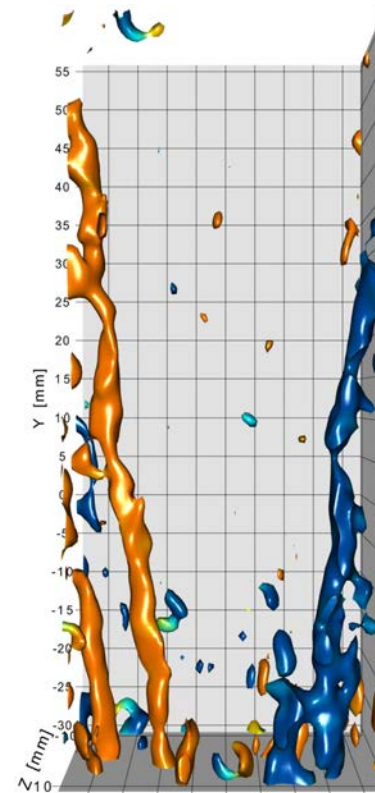

7615

190



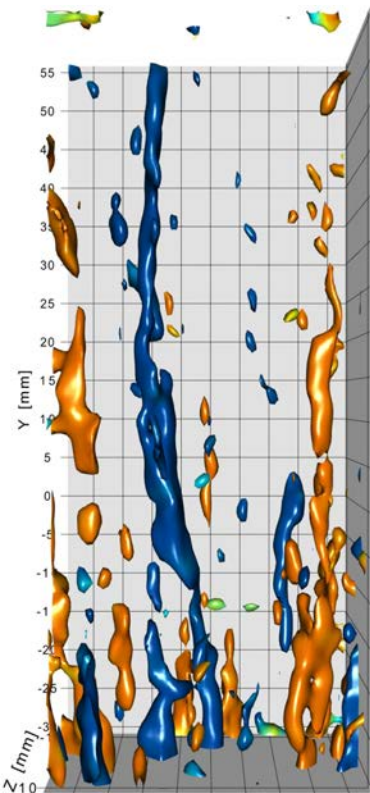

8901

191

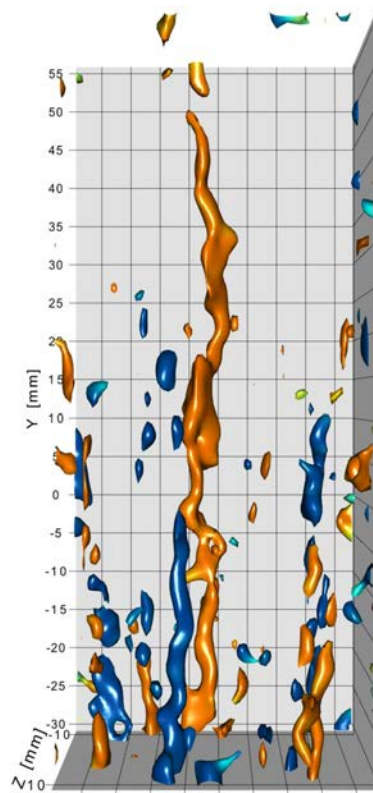

10887

192

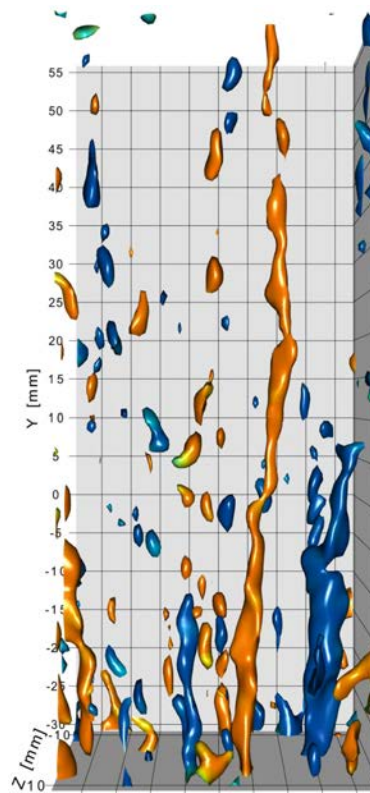

11390

193

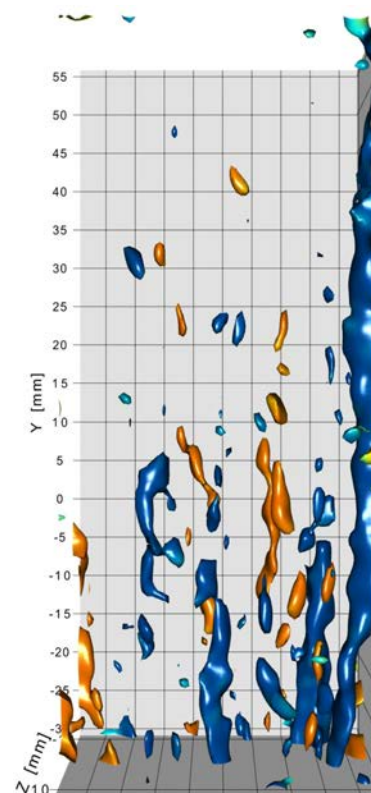

11777

194

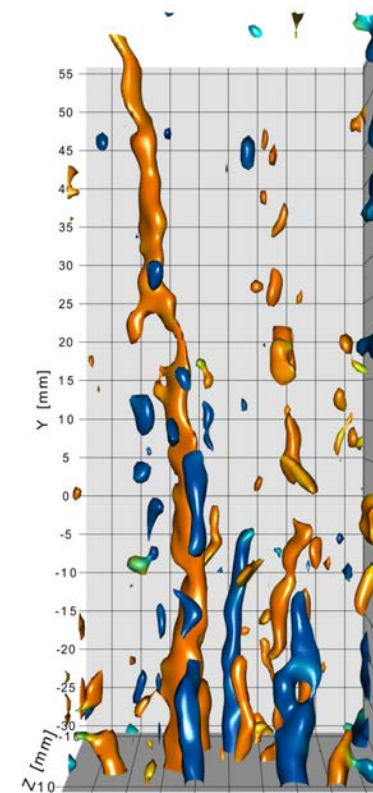

13857

195

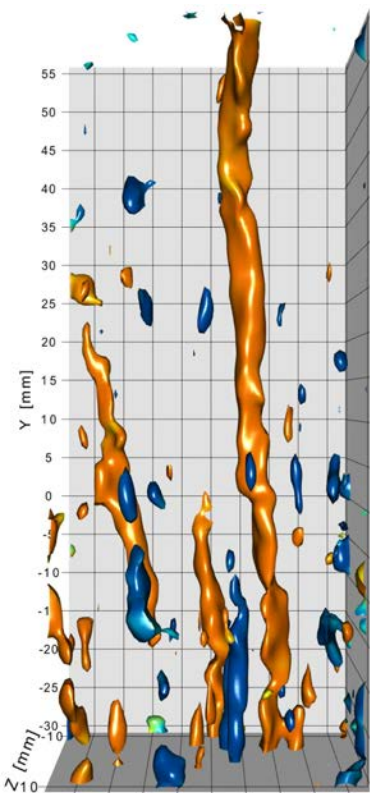

15150

196

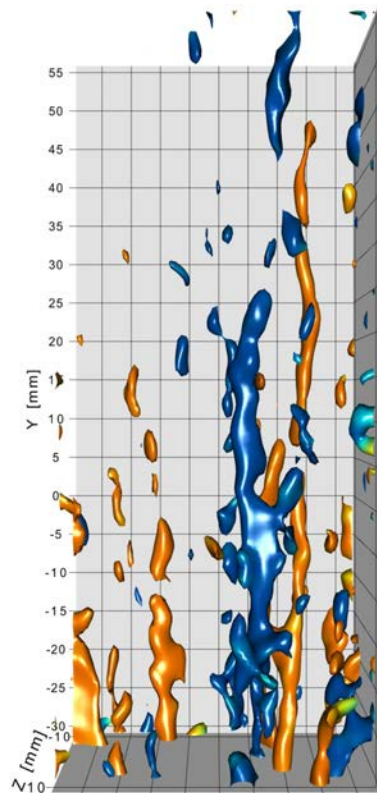

16508

197

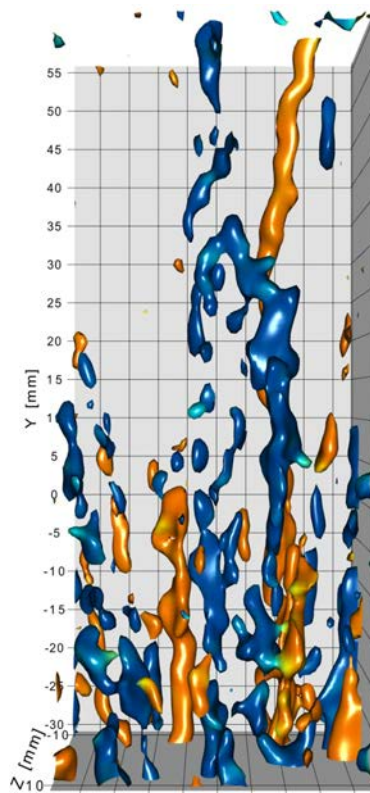

16789

198

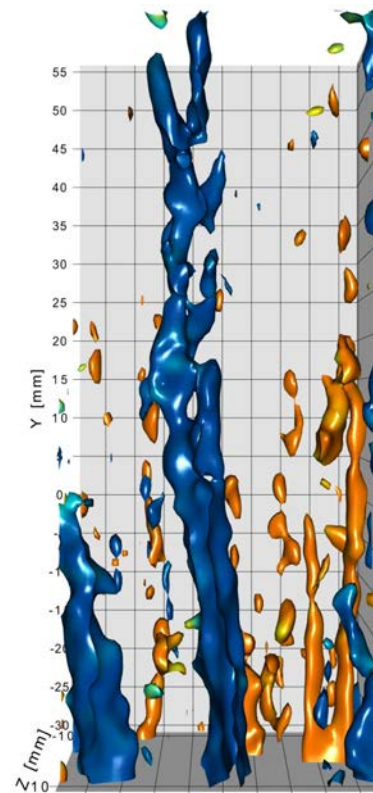

17088

199

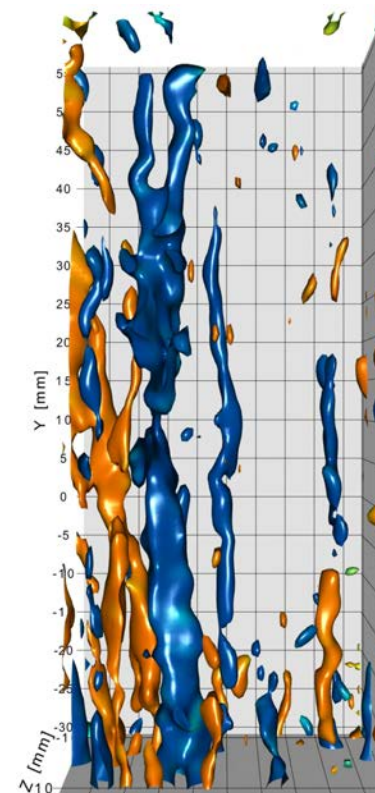

17625

200



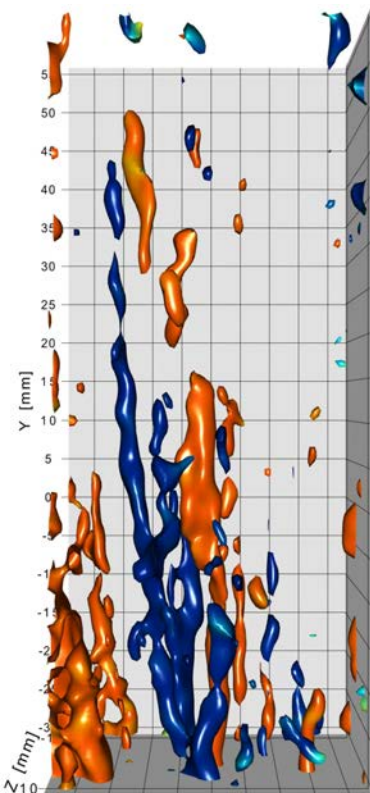

17904

201

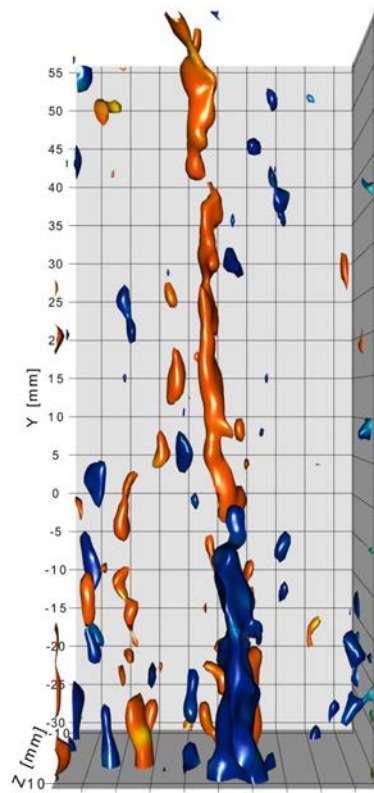

18269

202

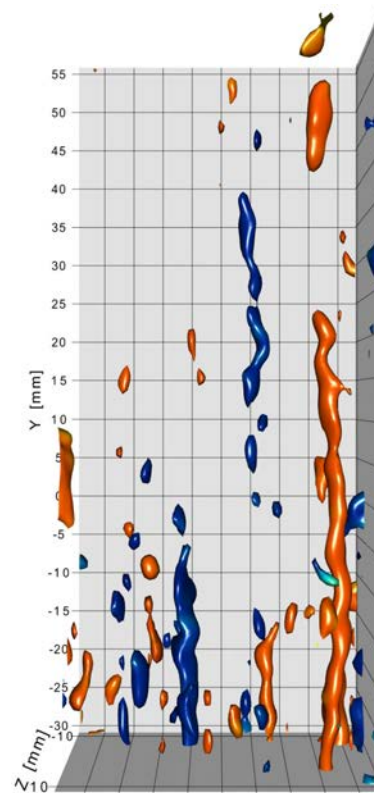

19961

203

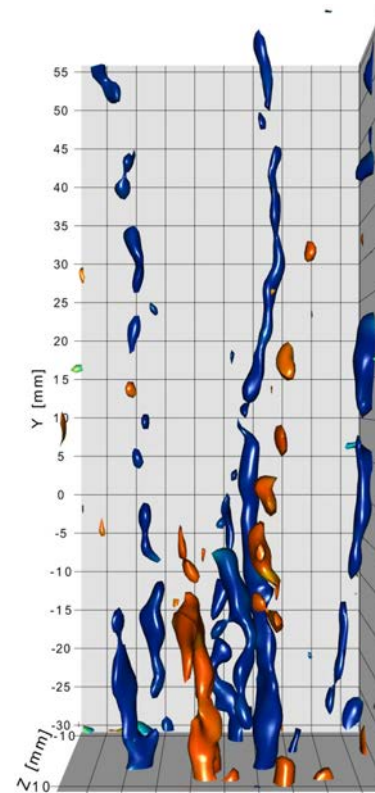

20357

204

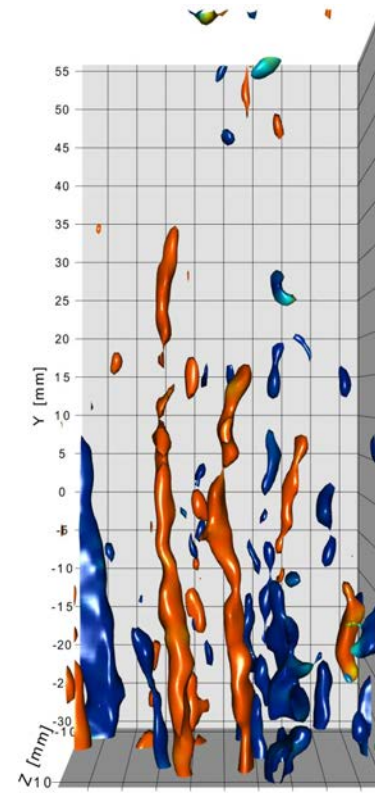

20765

205

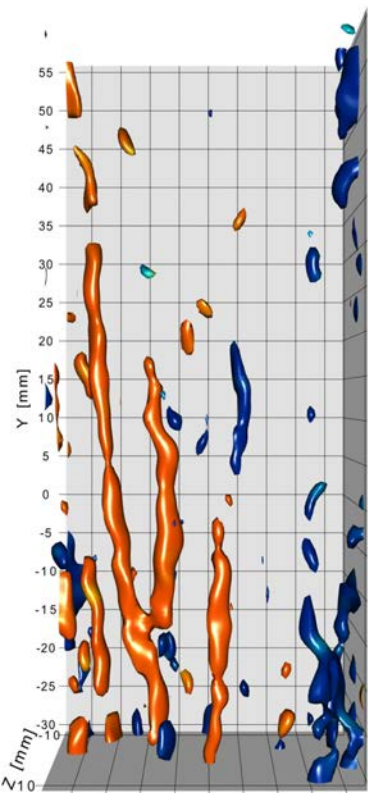

22323

206

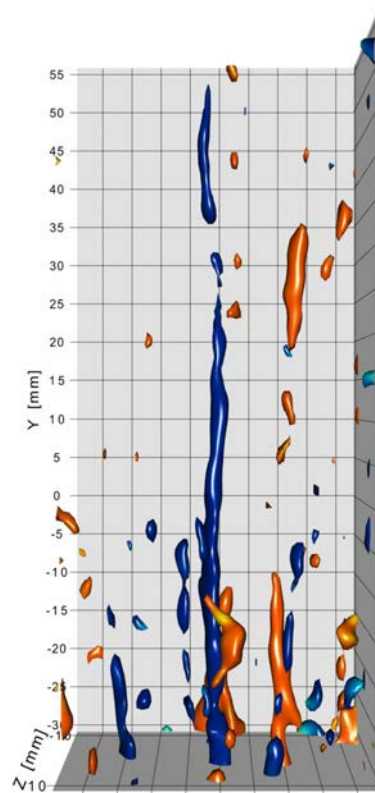

23359

207

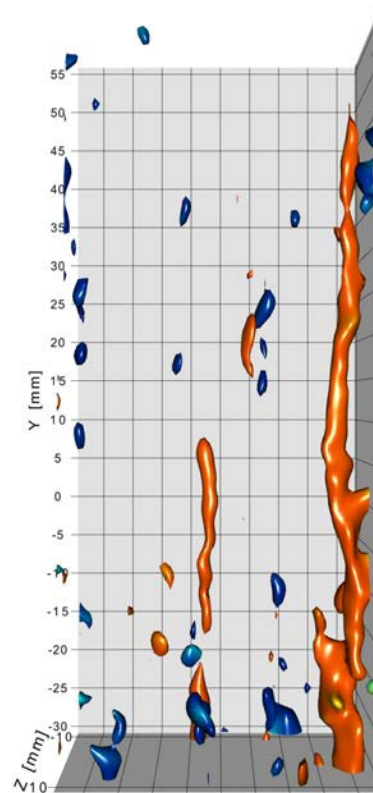

25087

208

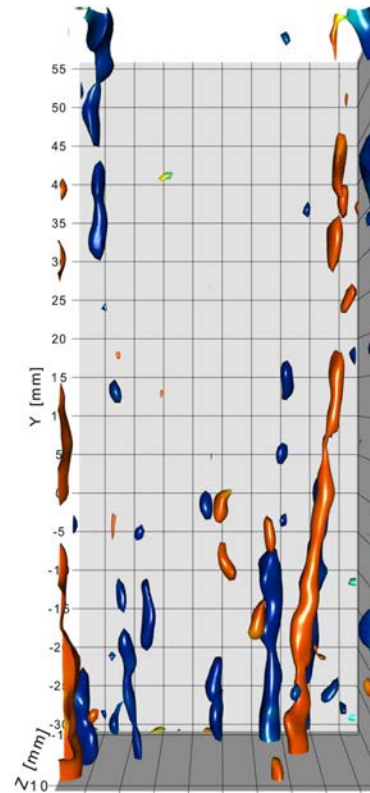

25419

209

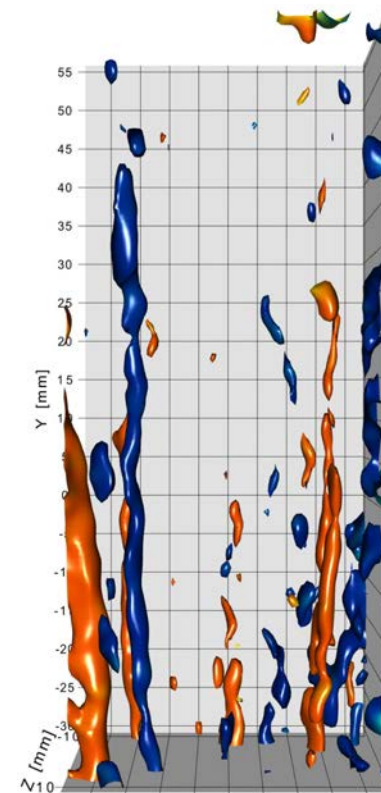

25540

210

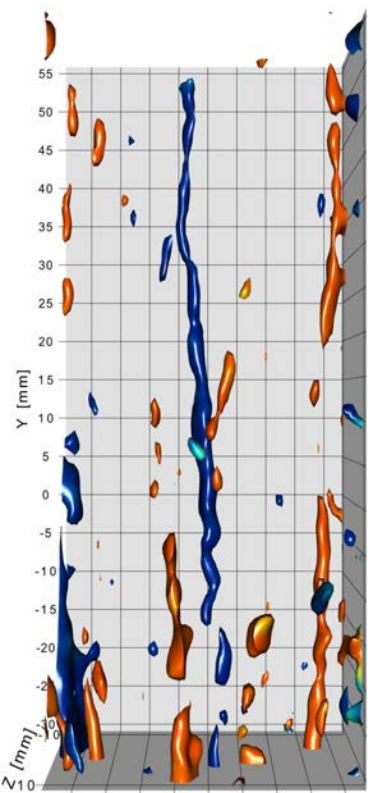

26241

211

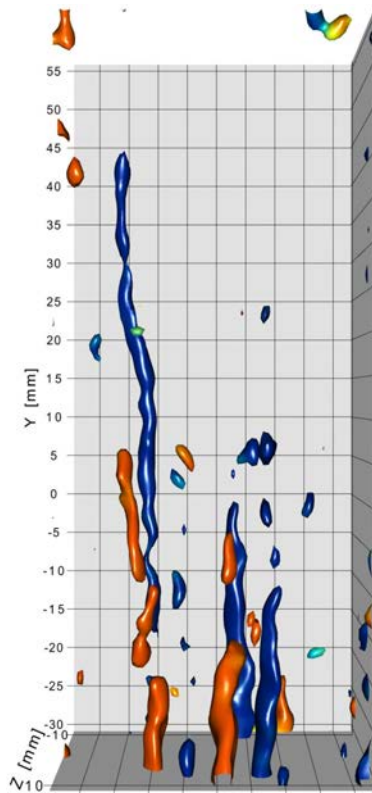

27779

212

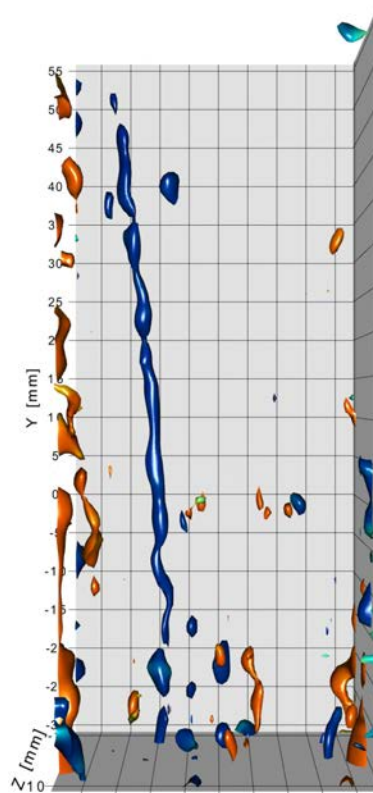

29261

213

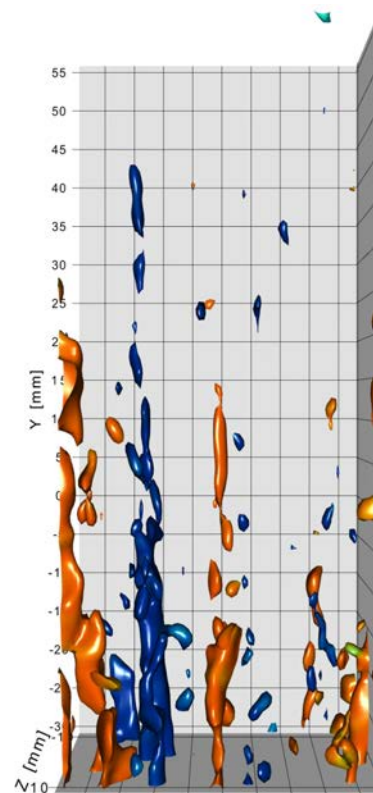

29471

214

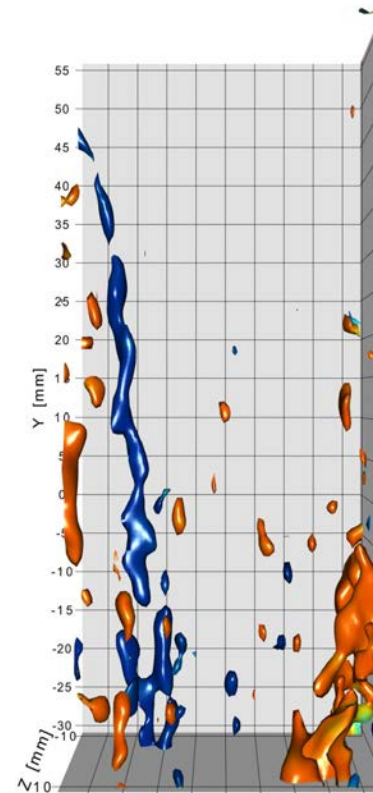

30251

215



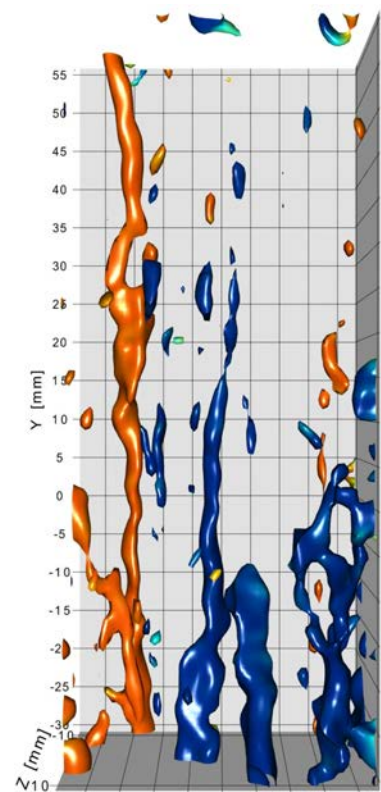

31247

216

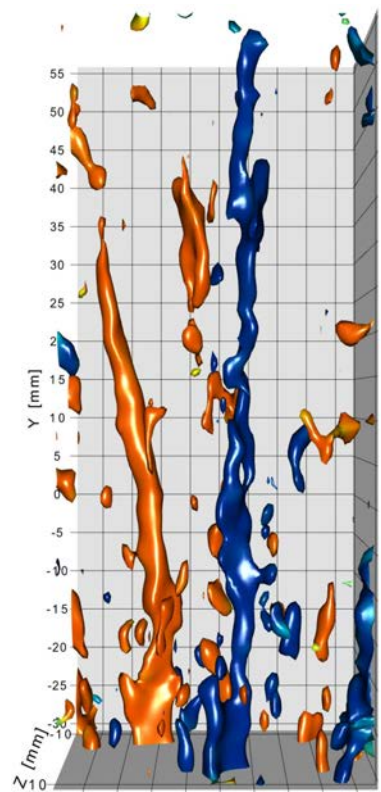

31389

217

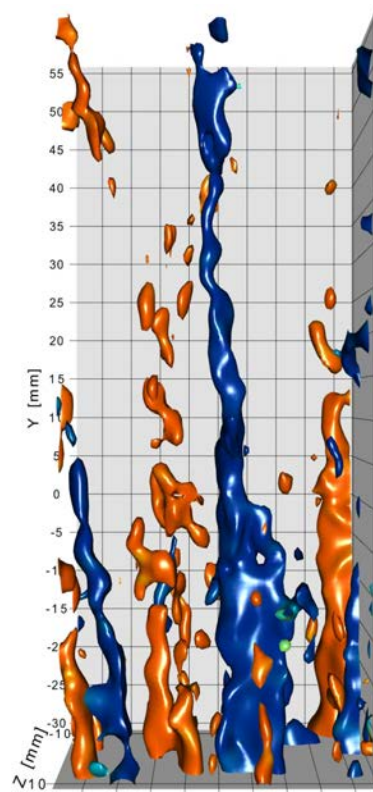

31777

218

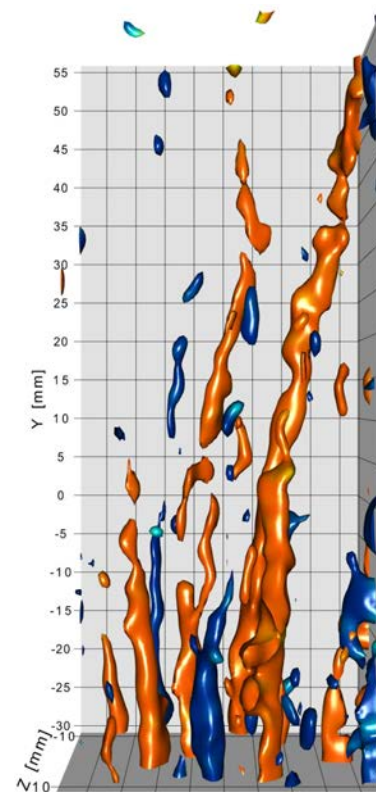

32979

219

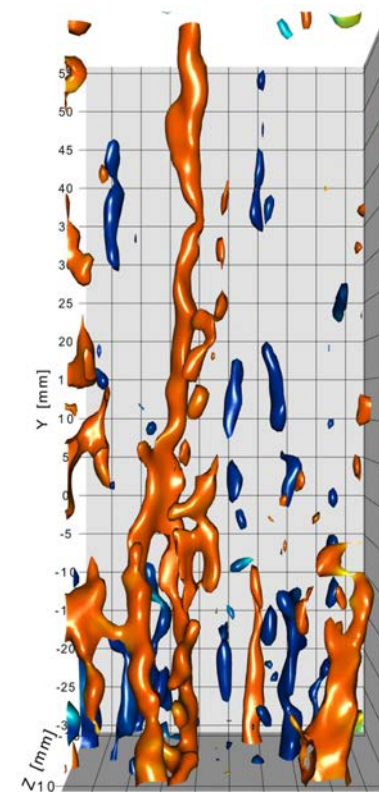

33436

220

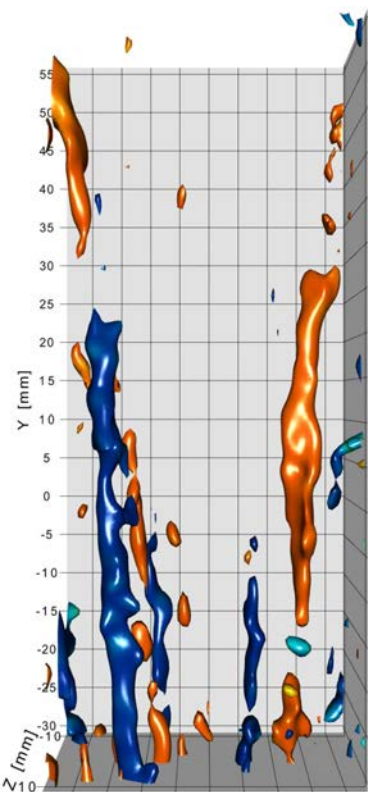

35196

221

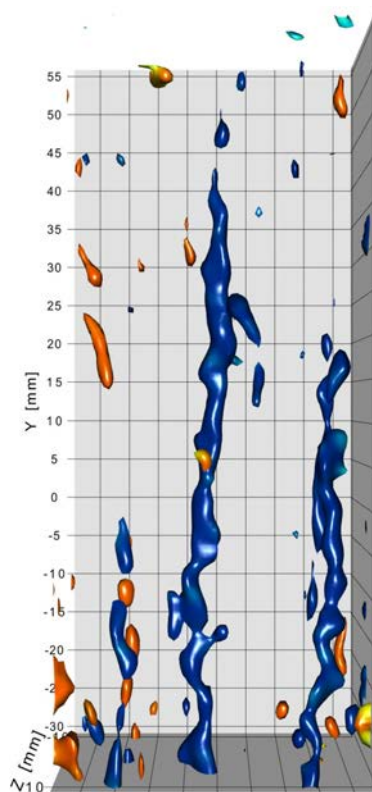

36105

222

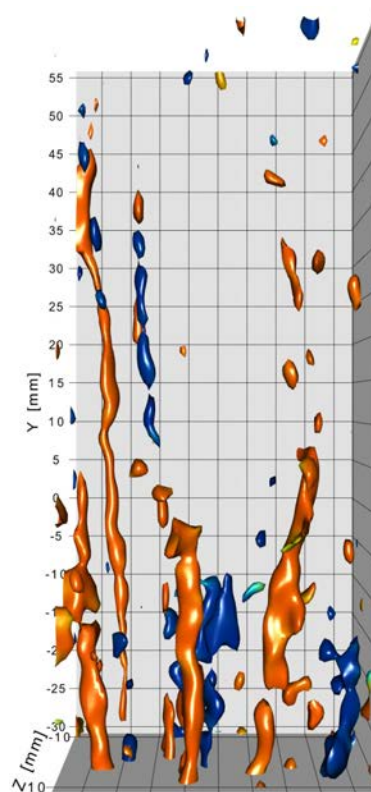

36987

223

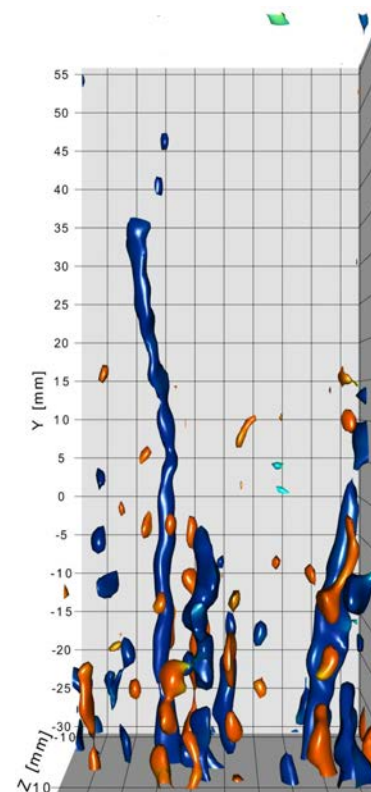

37323

224

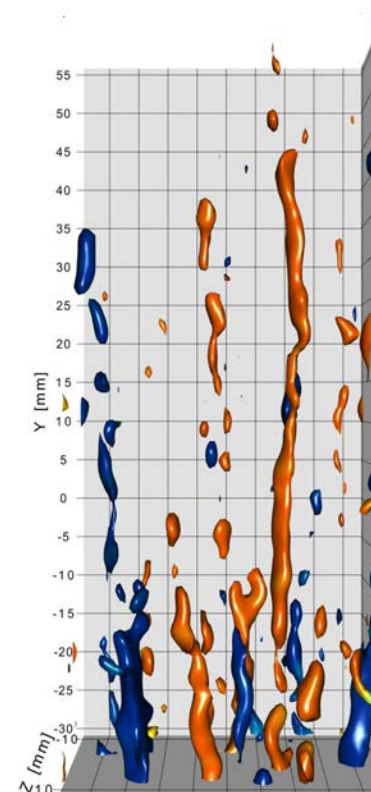

38830

225



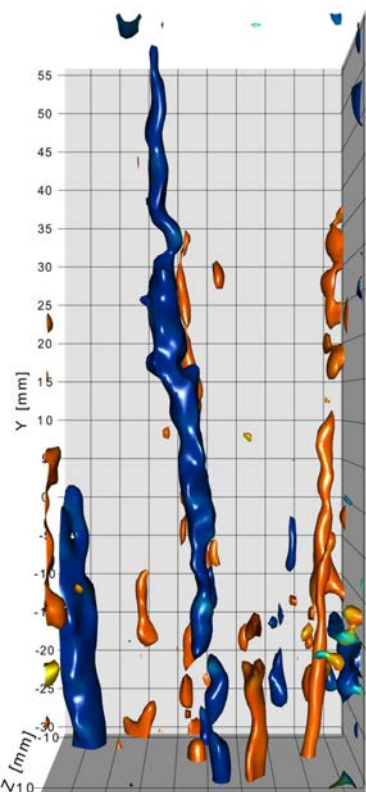

39032

226

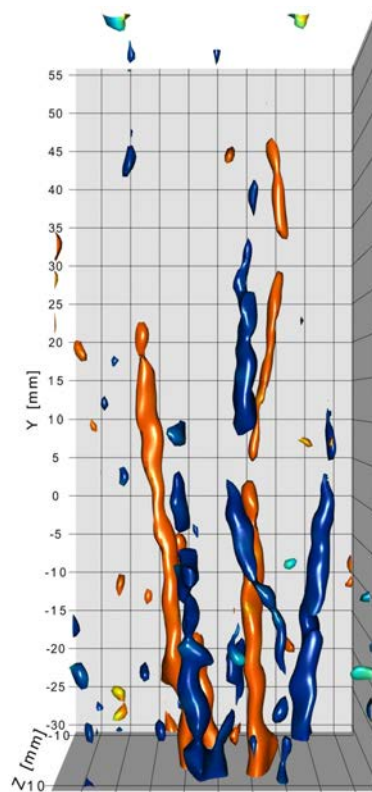

39533

227

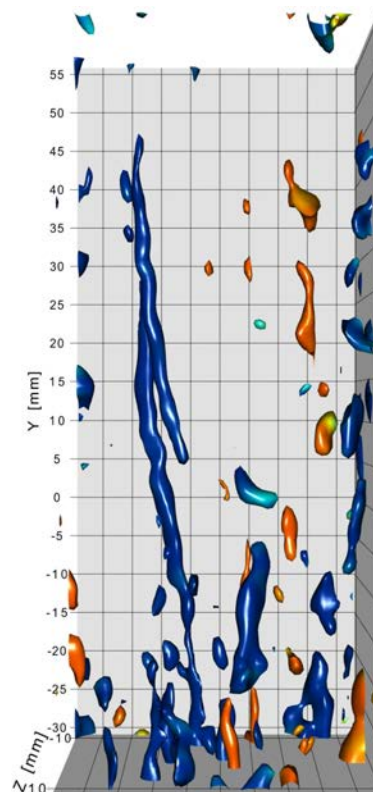

39778

228

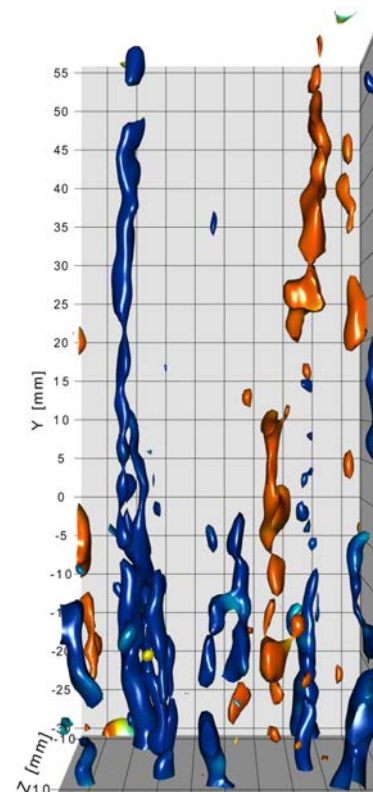

40018

229

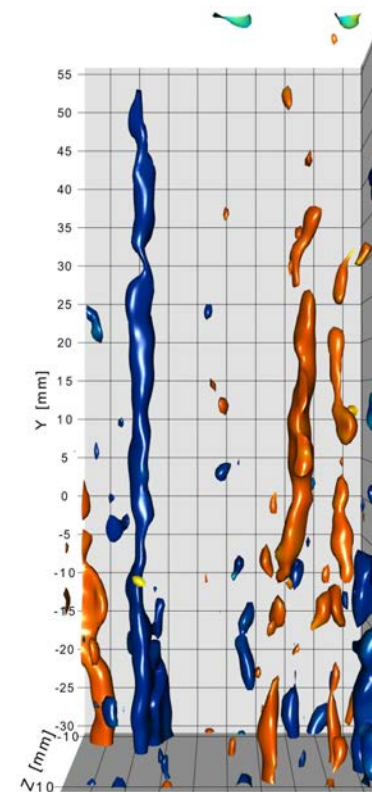

40088

230



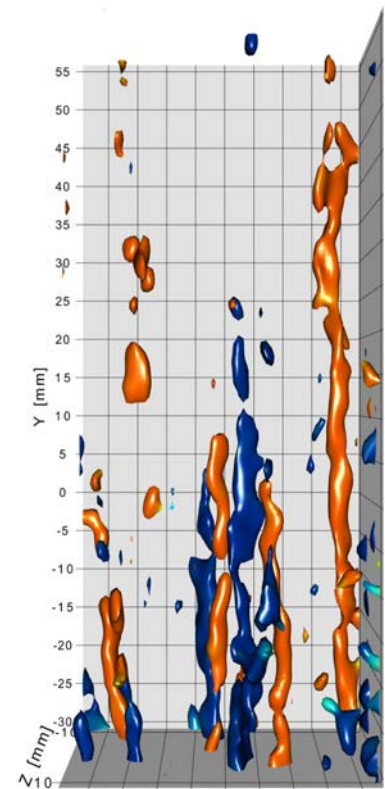

40992

231

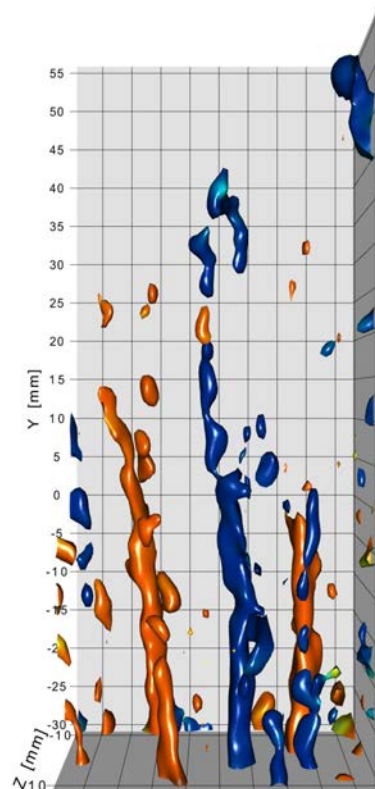

41208

232

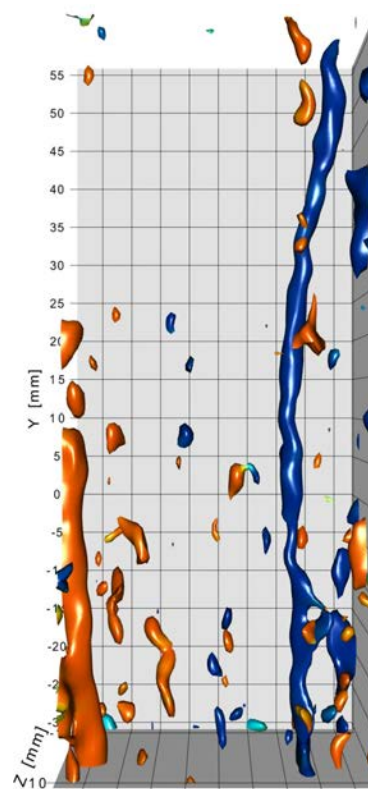

41427

233

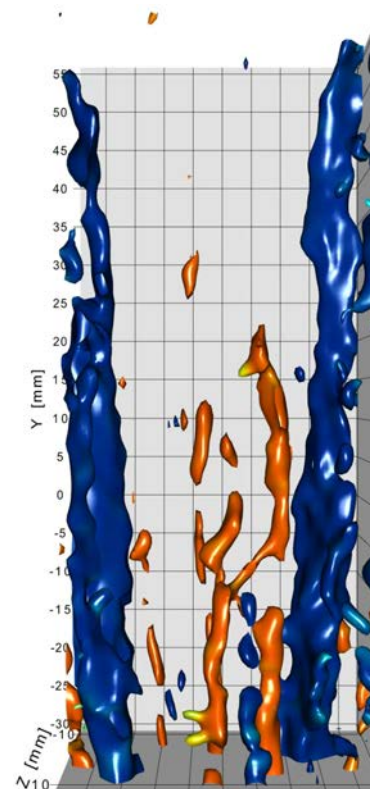

41930

234

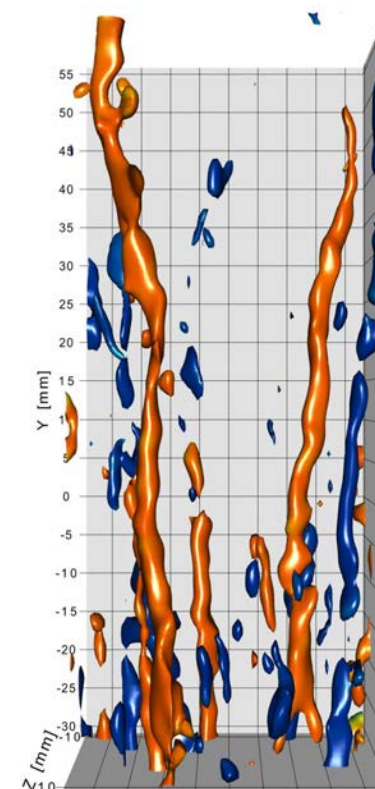

42588

235

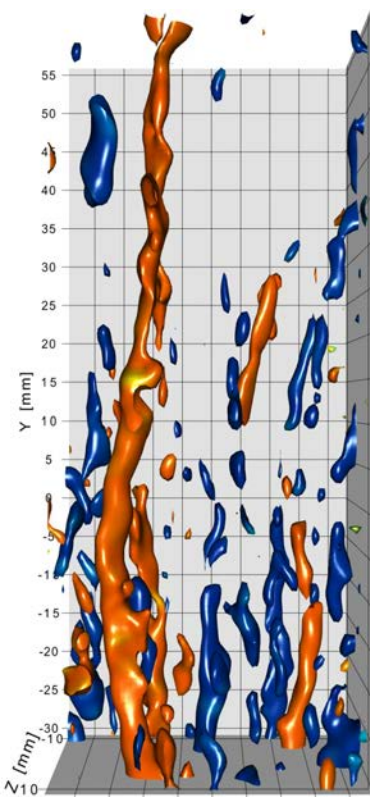

42768

236

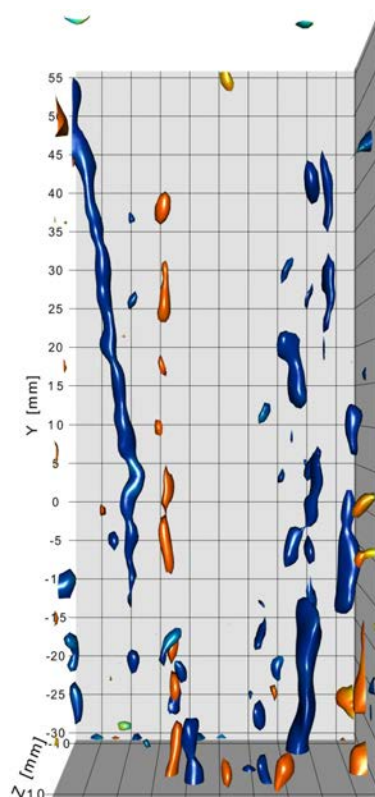

44358

237

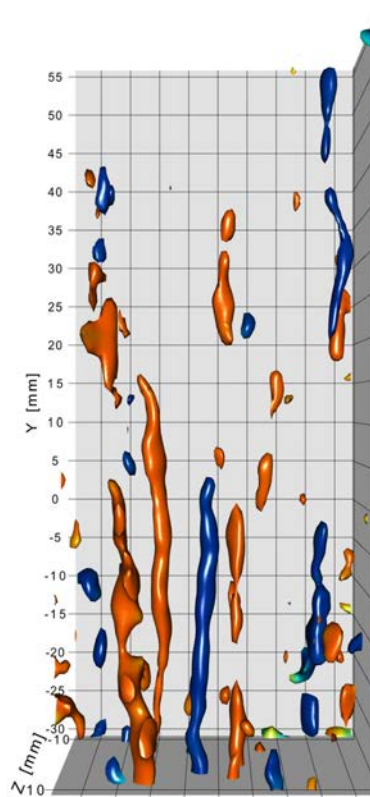

46177

238

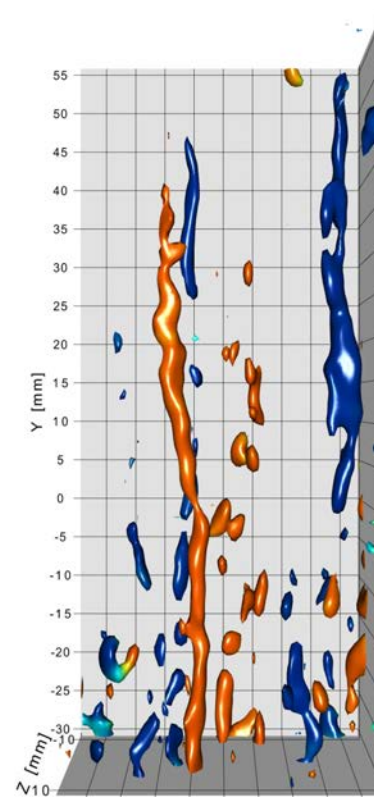

46706

239

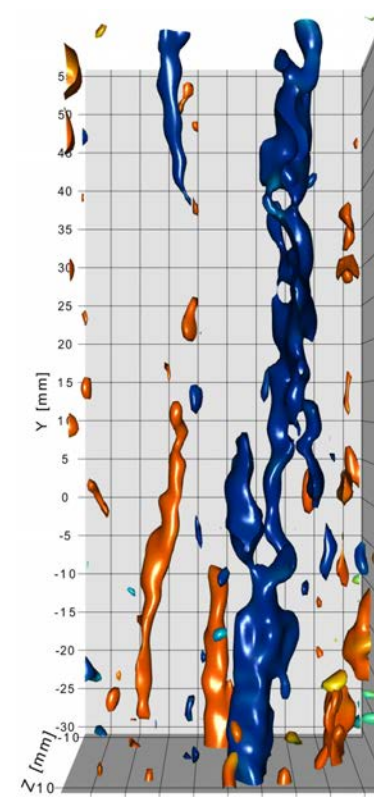

49327

240



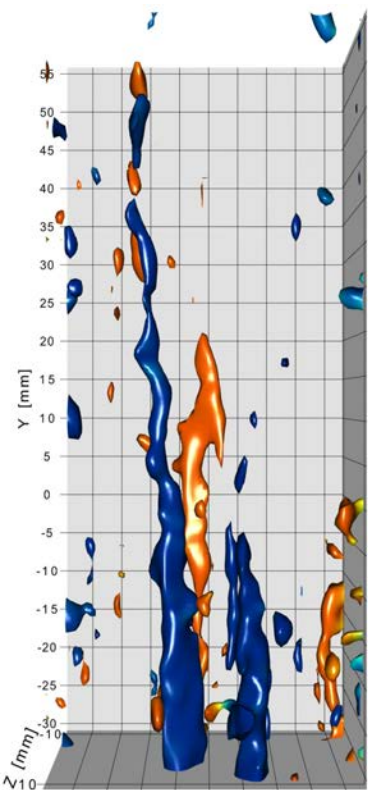

49629

241

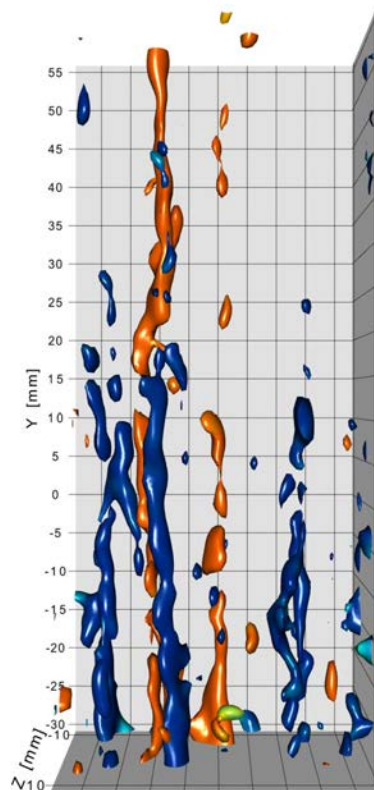

49738

242

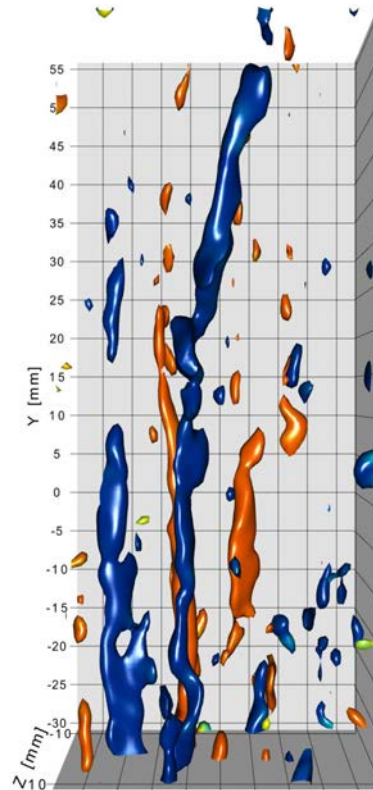

49950

243

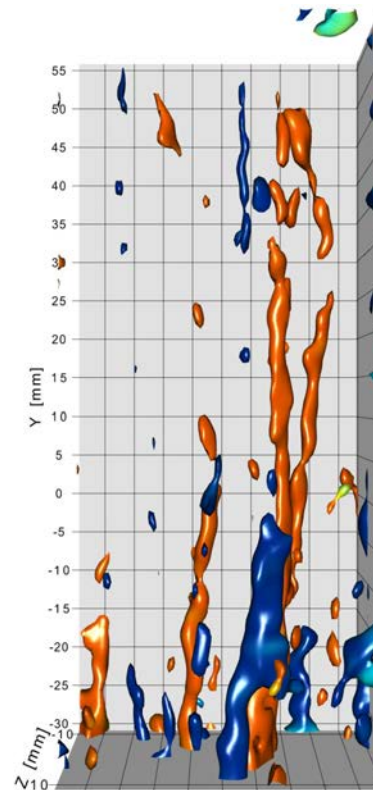

50130

244

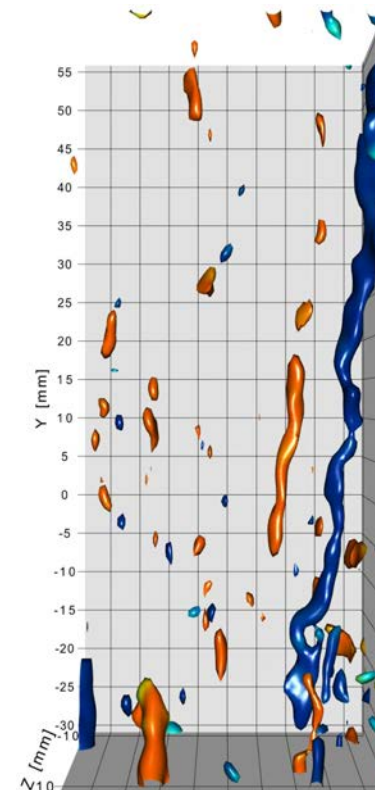

51336

245



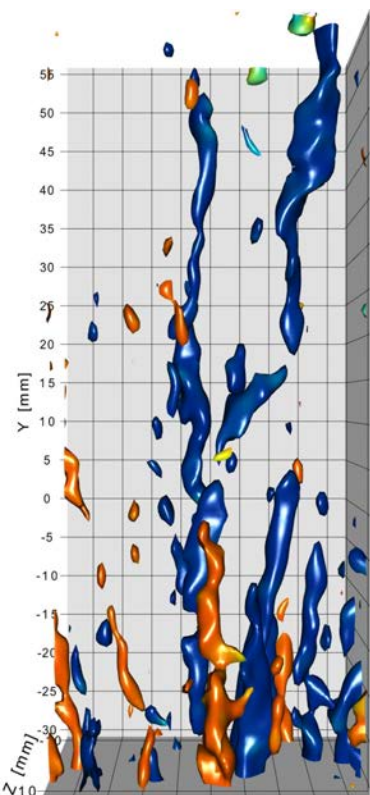

52849

246

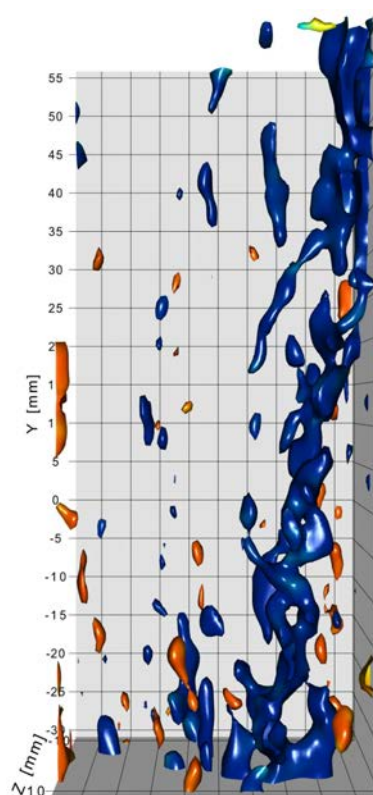

53191

247

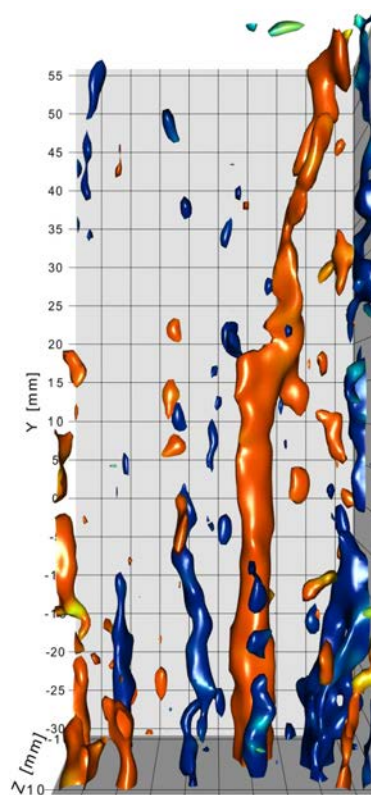

53694

248

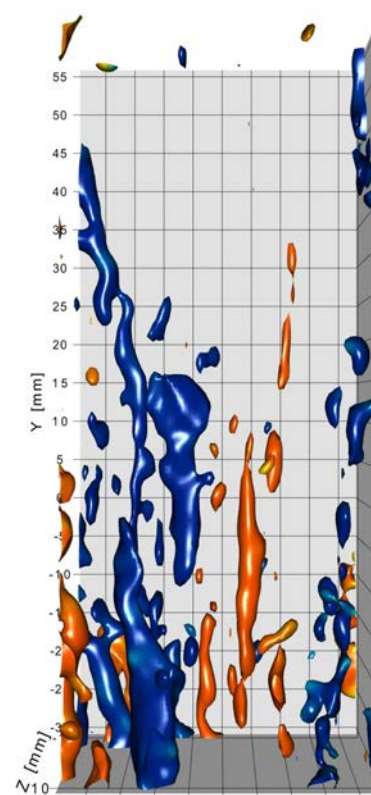

54744

249

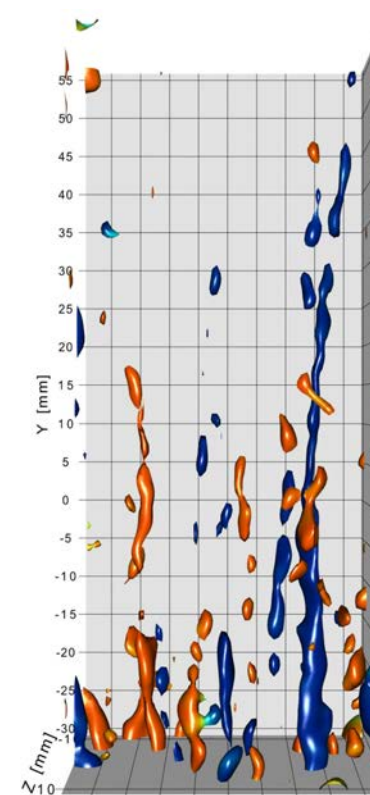

55640

250

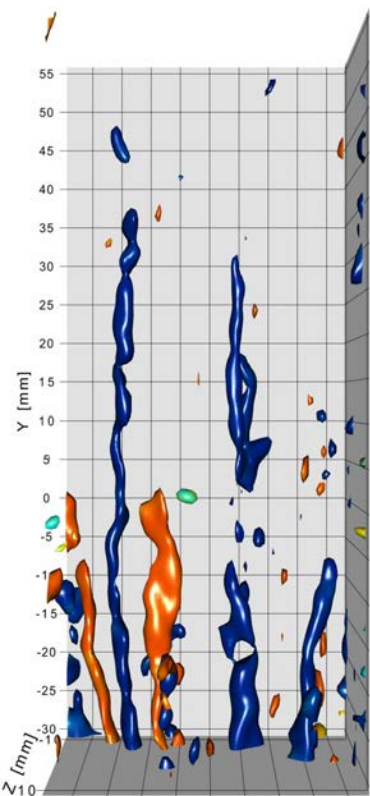

55998

251

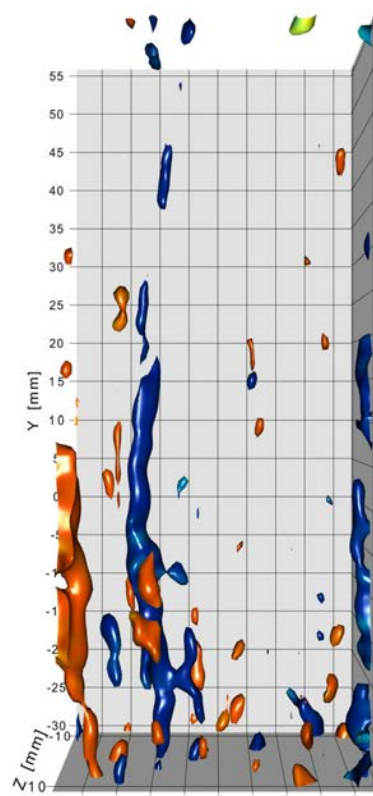

56783

252

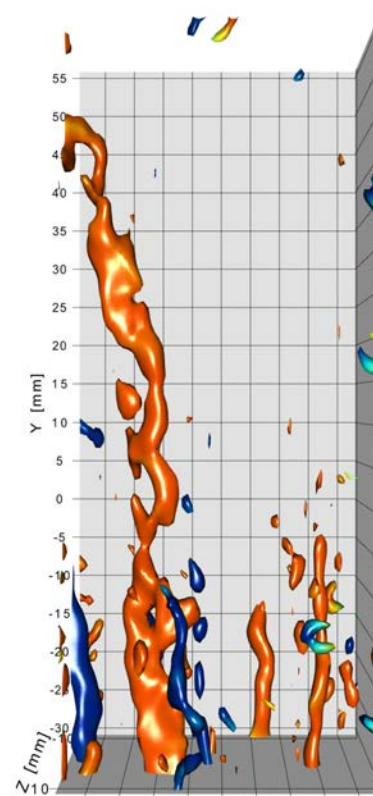

58242

253

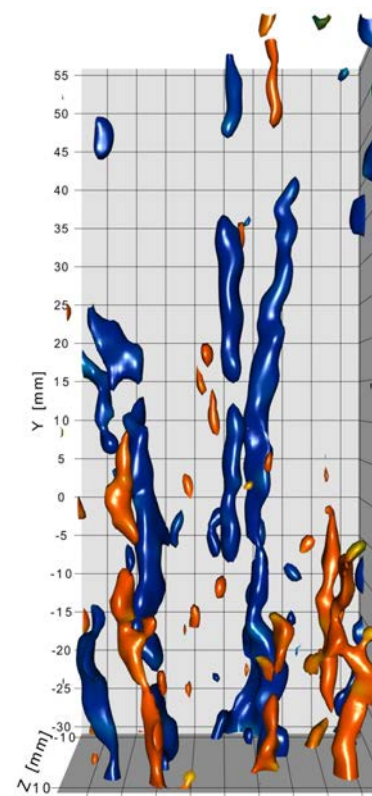

59797

254

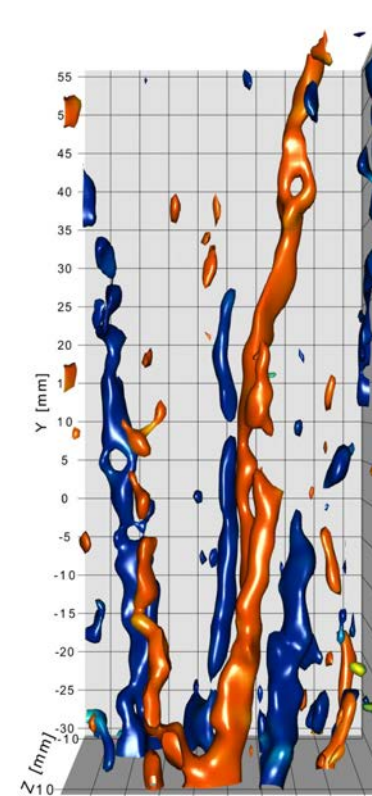

59982

255



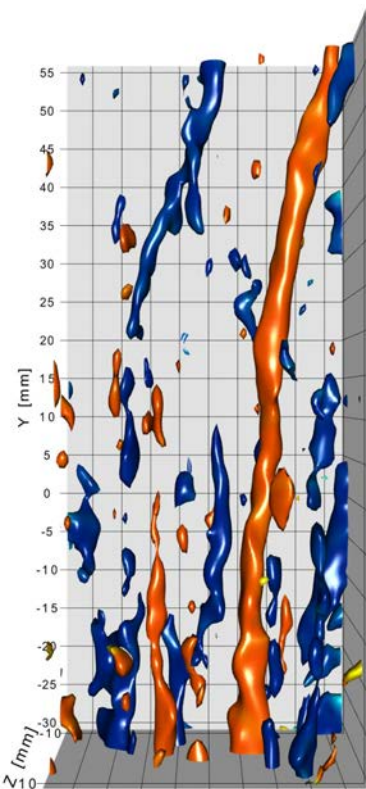

60155

256

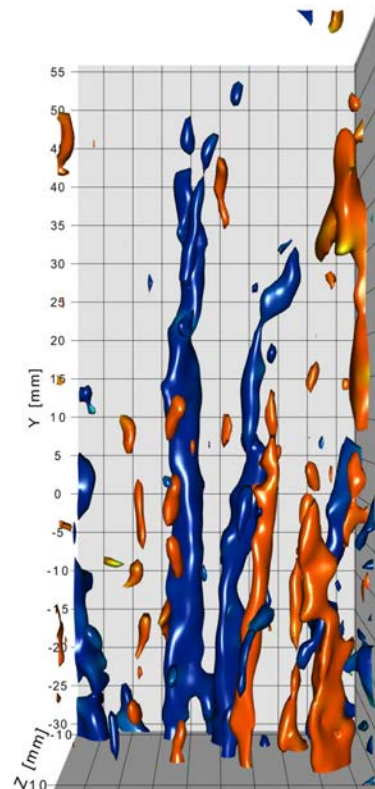

60420

257

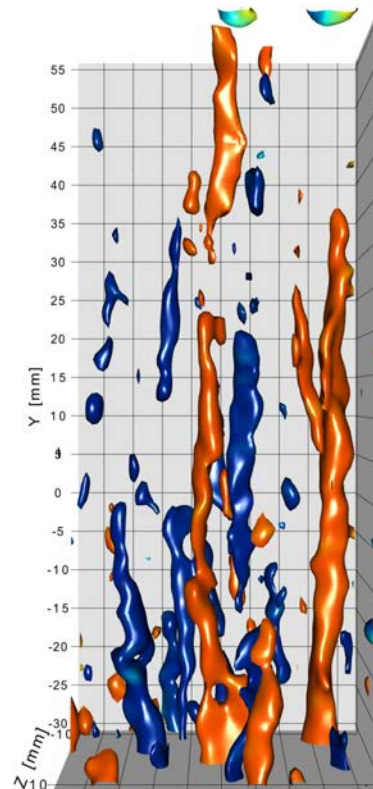

60886

258

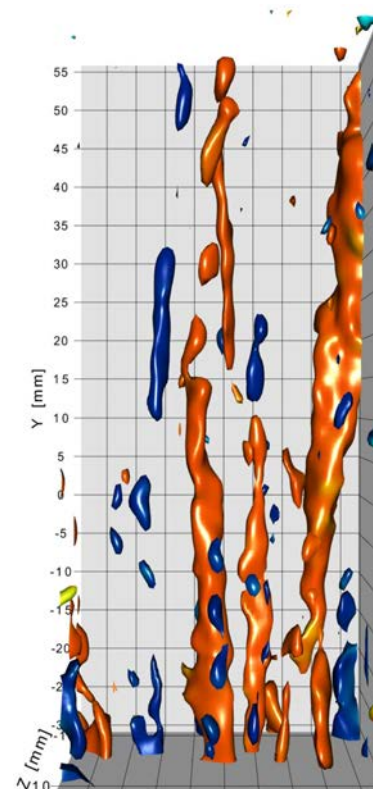

61102

259

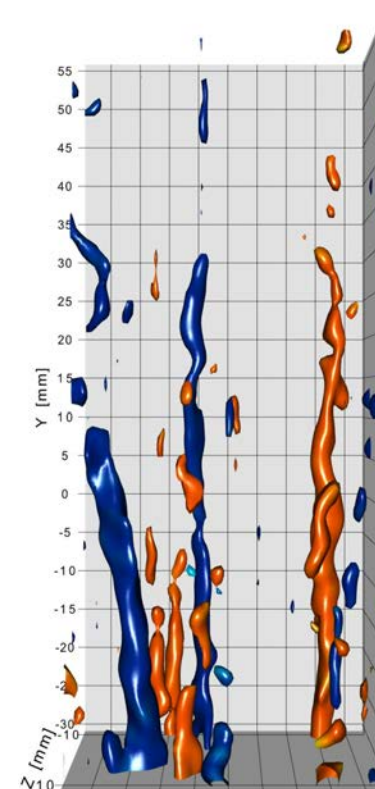

62450

260



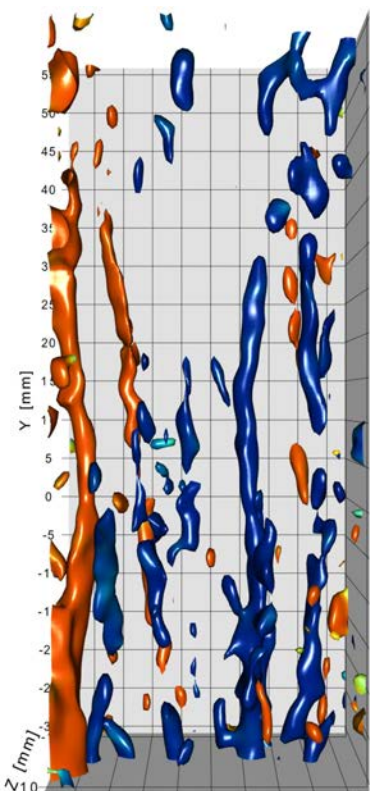

63383

261

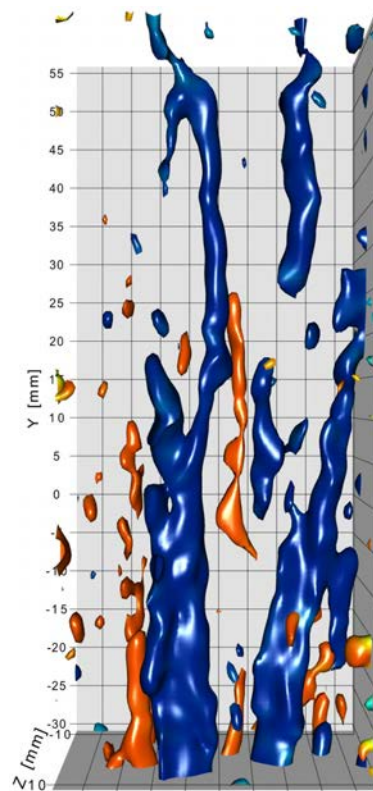

63596

262

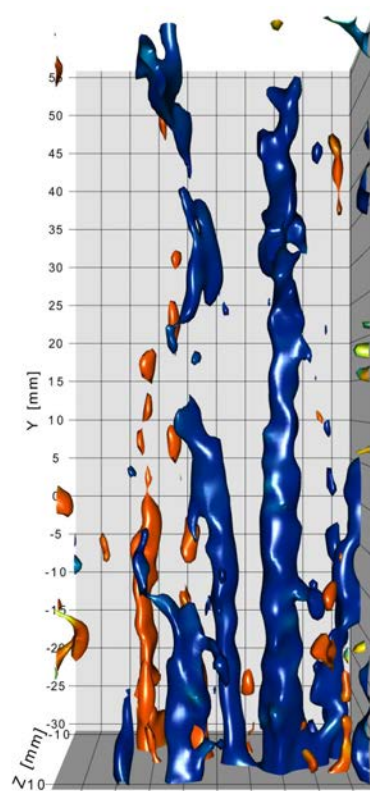

63743

263

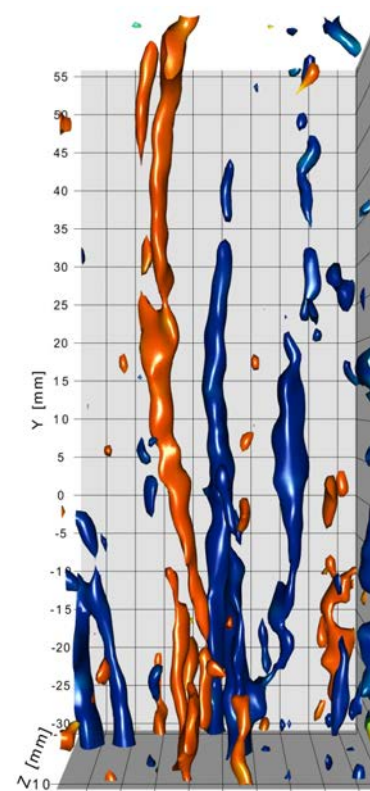

66154

264

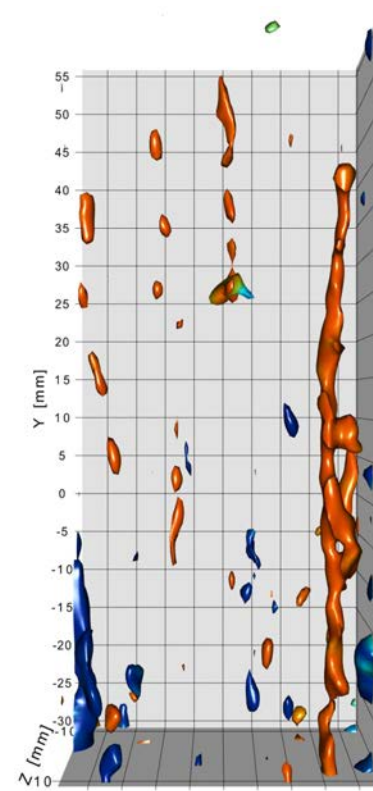

69736

265

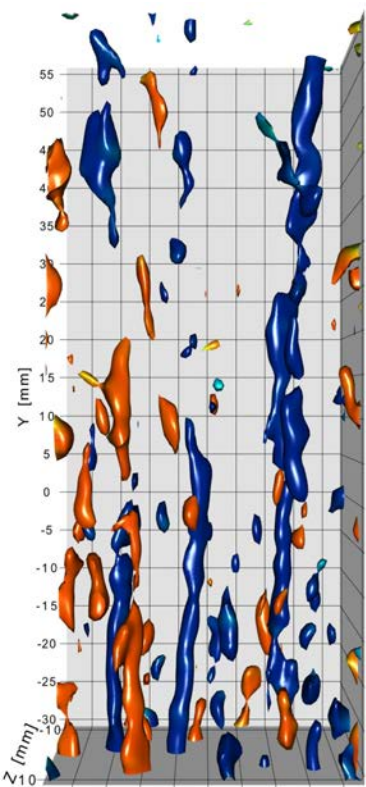

71363

266

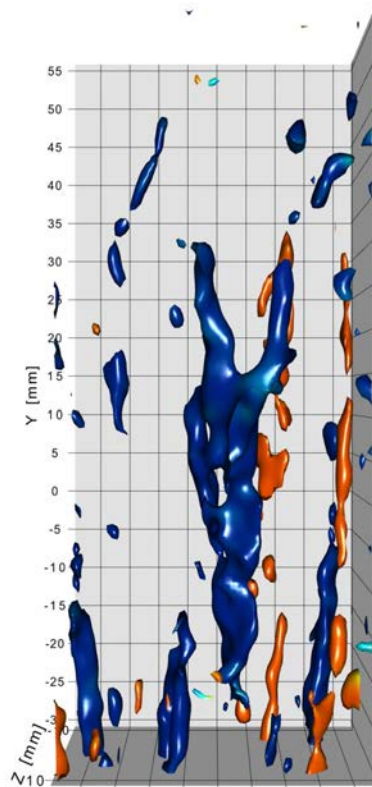

71901

267

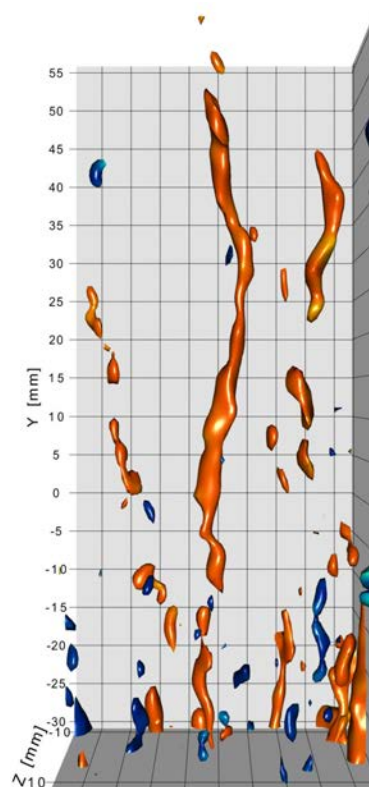

72693

268

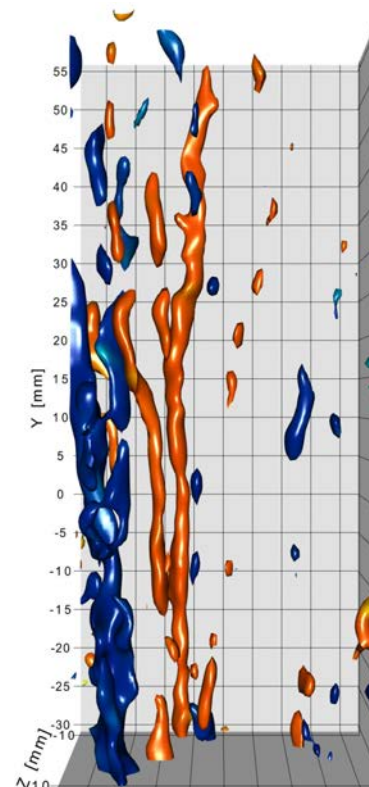

73190

269

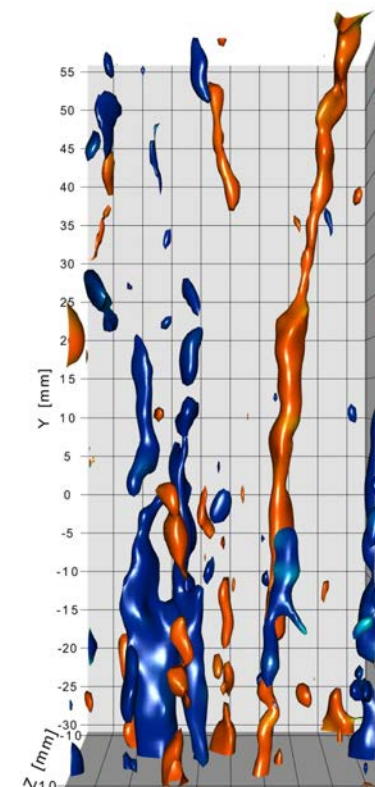

73413

270



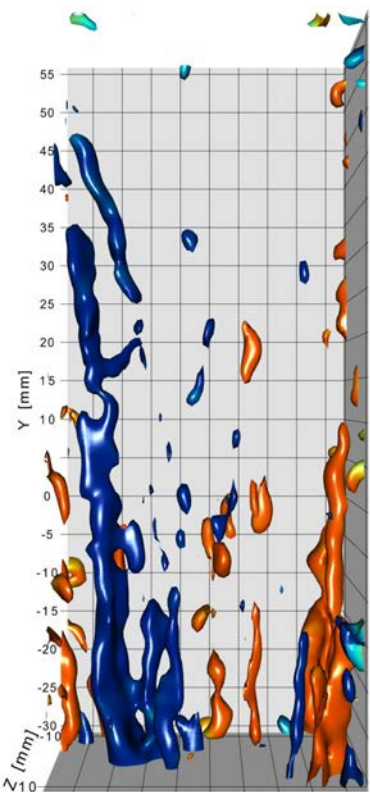

73722

271

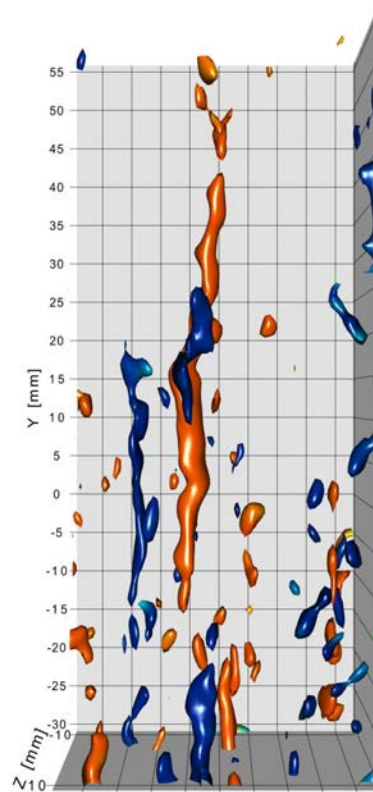

75045

272

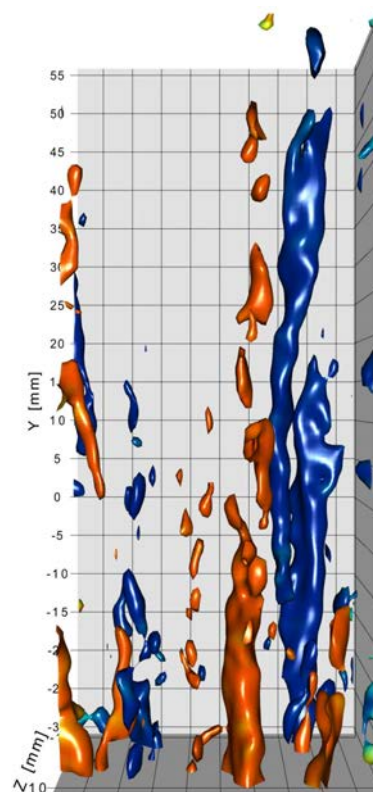

75677

273

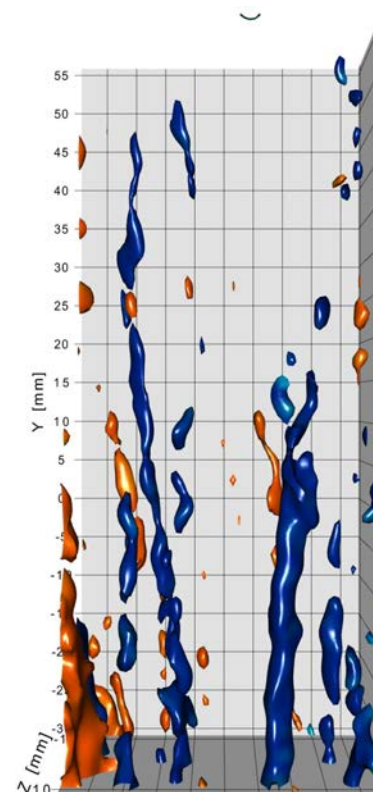

76019

274

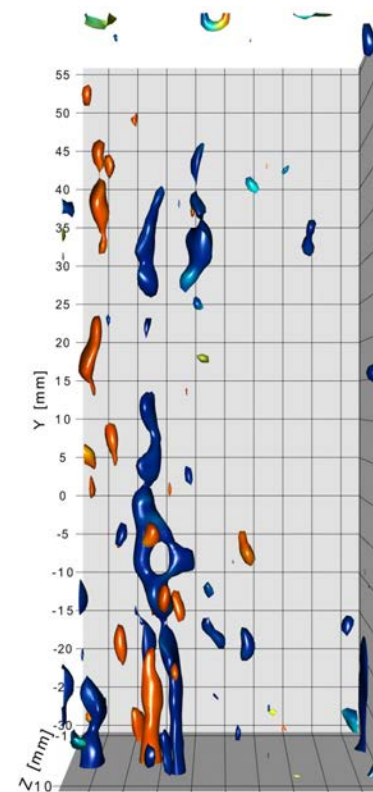

76775

275



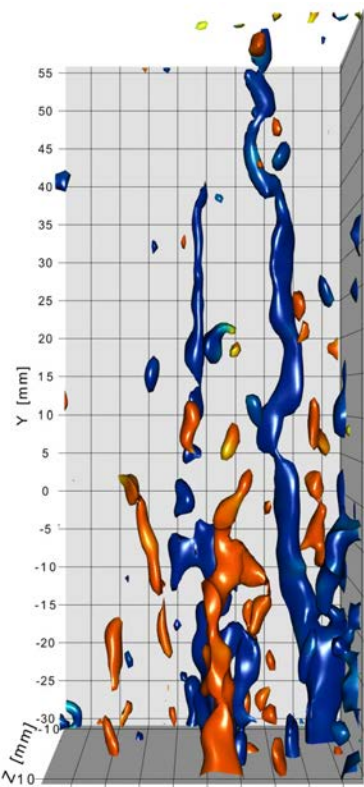

78286

276

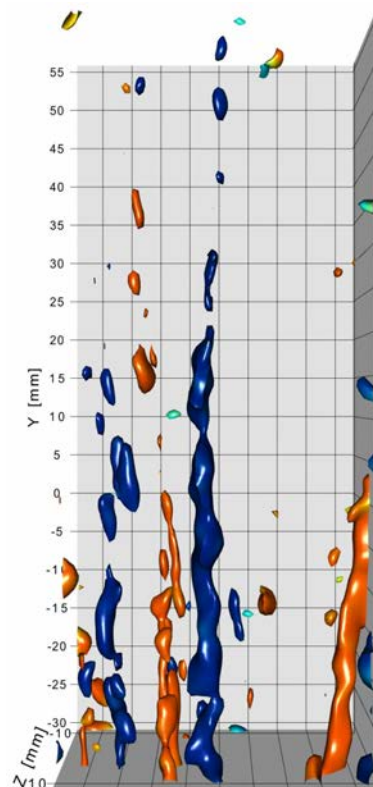

78679

277

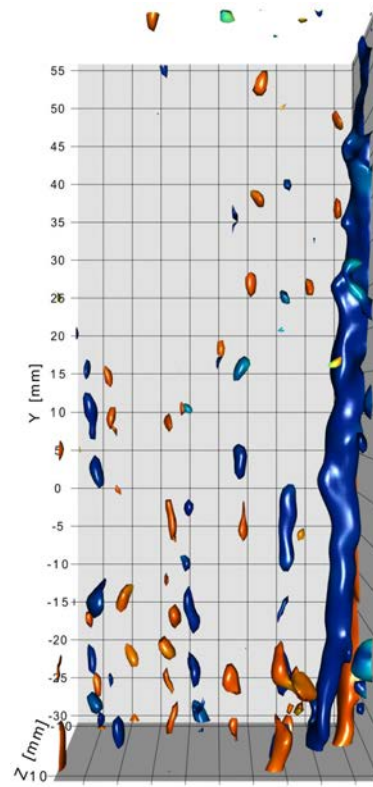

79648

278

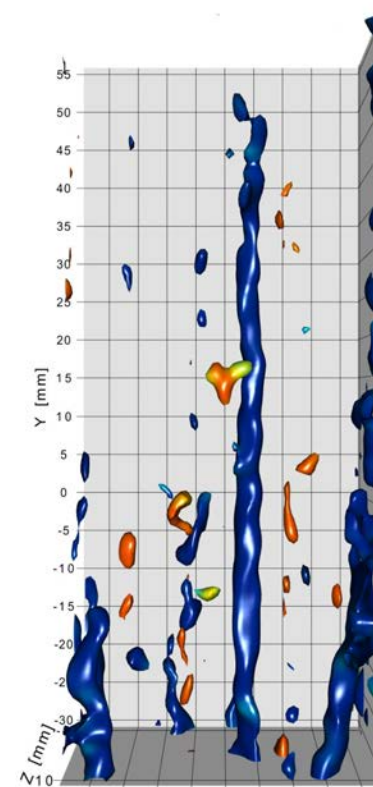

79903

279

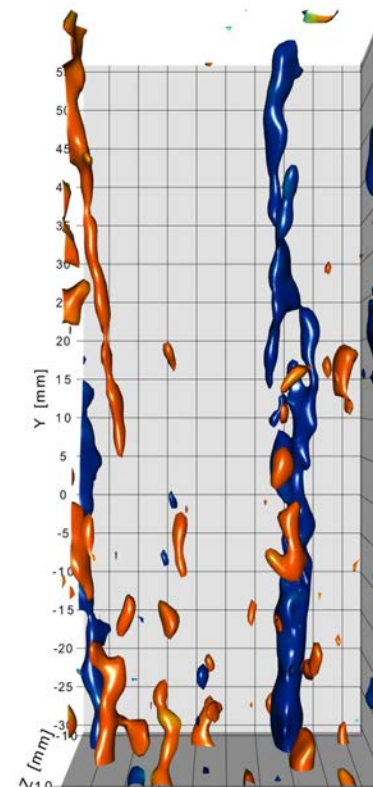

81225

280

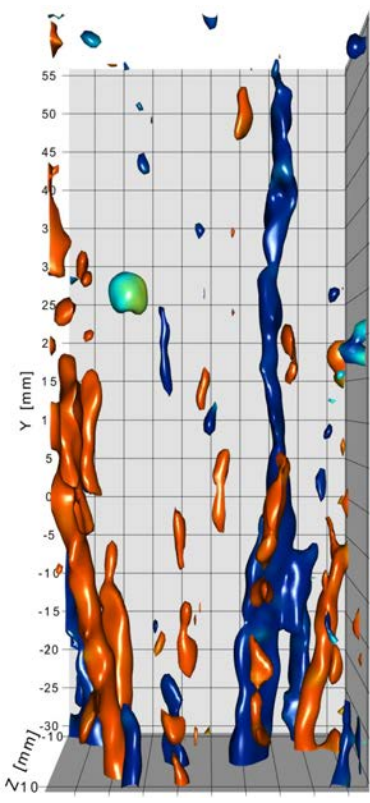

81489

281

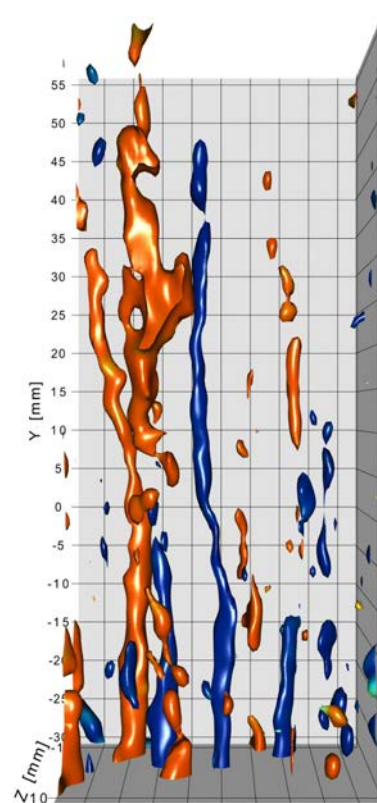

81783

282

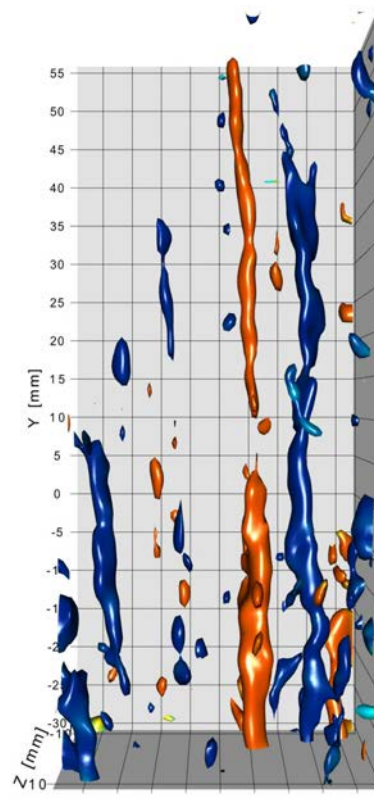

82725

283

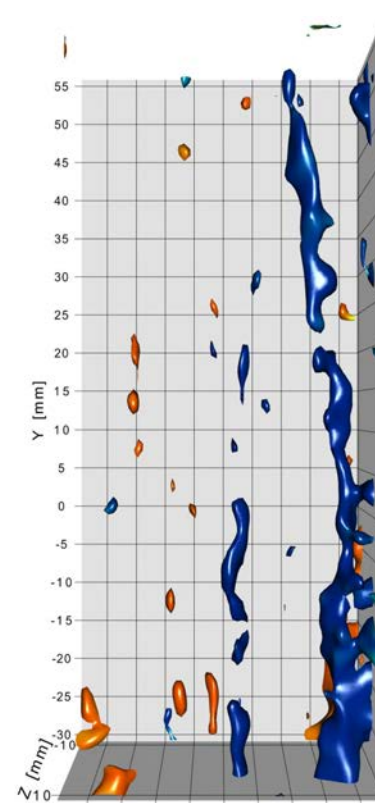

83897

284

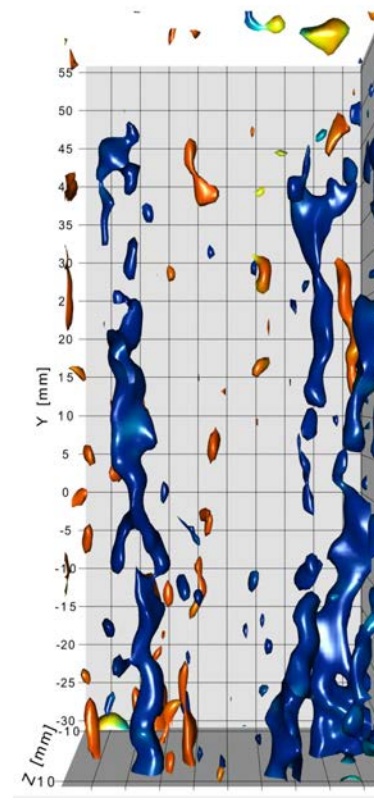

84219

285



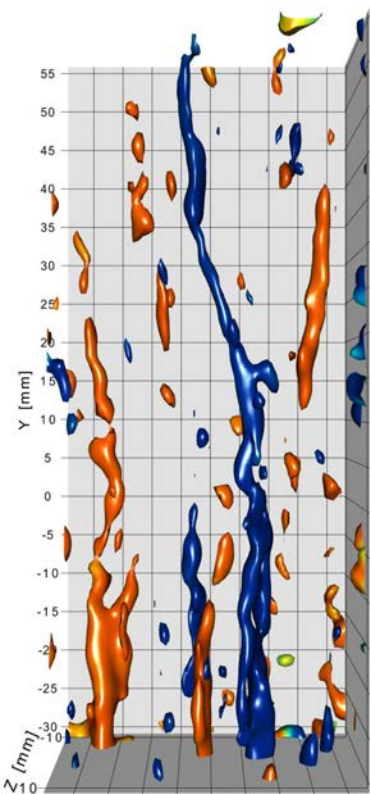

85007

286

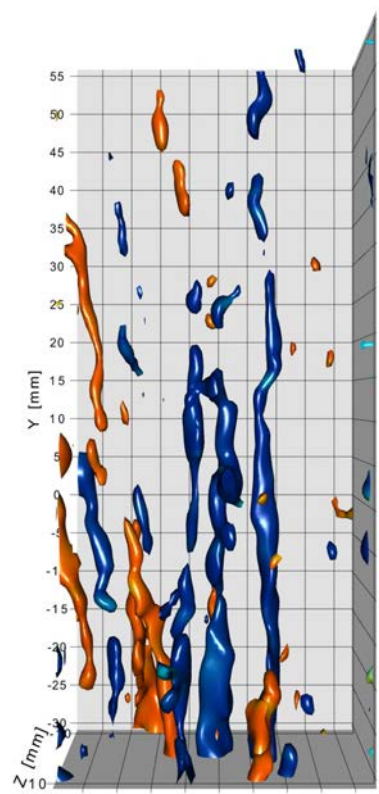

85251

287

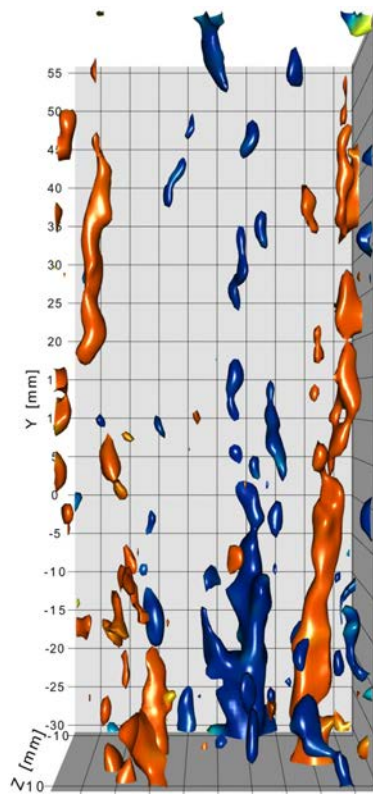

85719

288

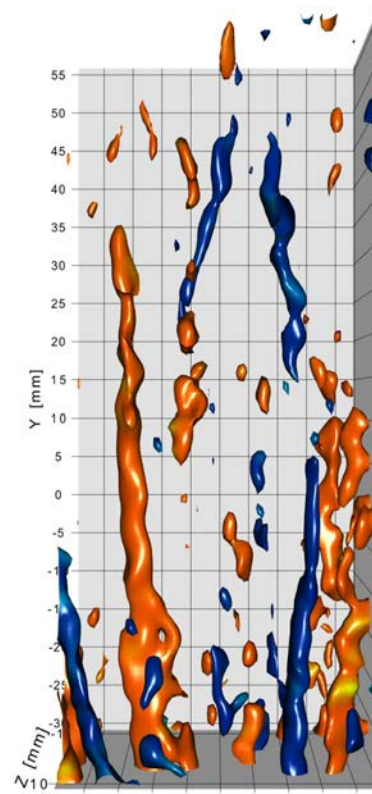

86195

289

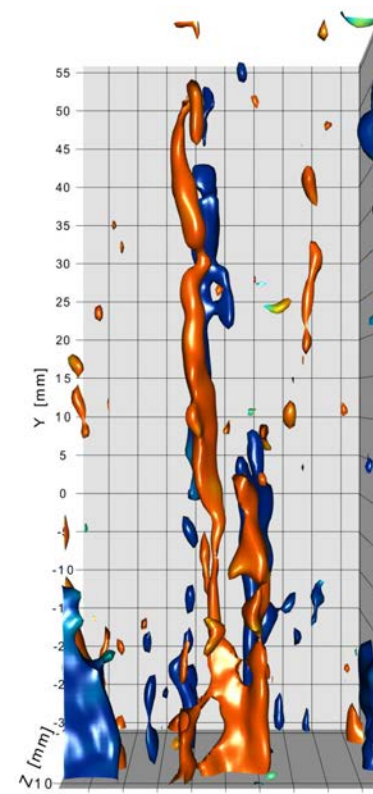

86712

290



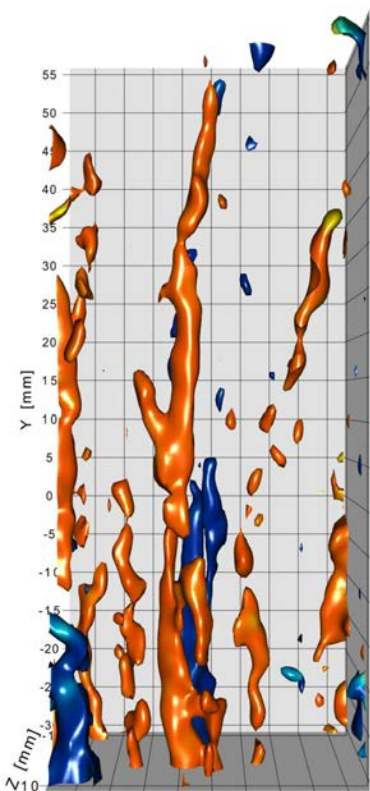

86884

291

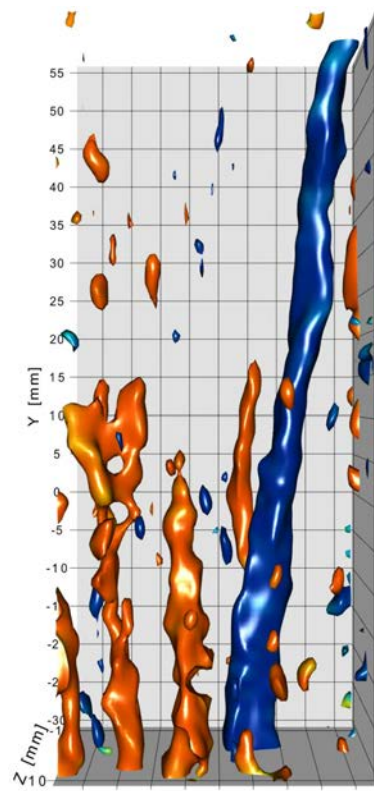

87172

292

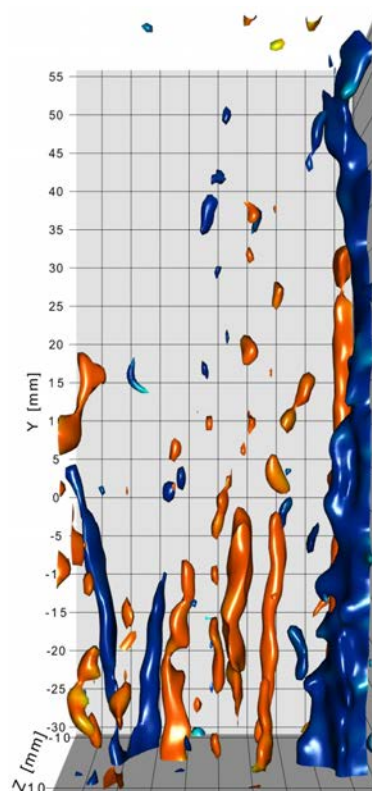

87716

293

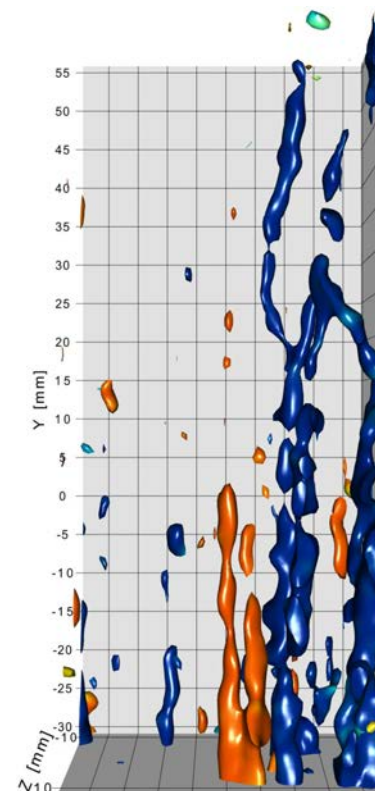

87993

294

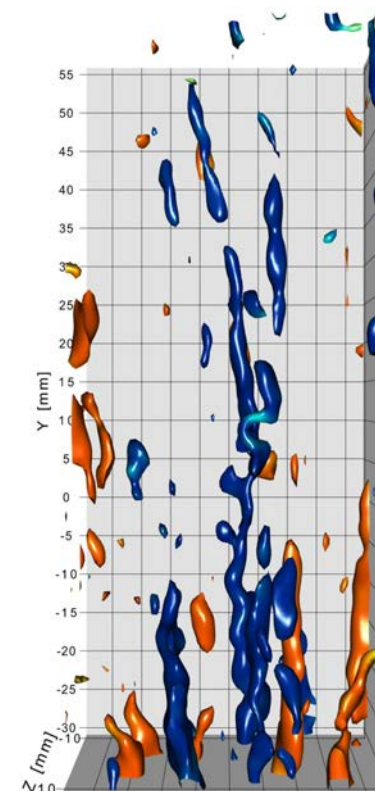

89664

295

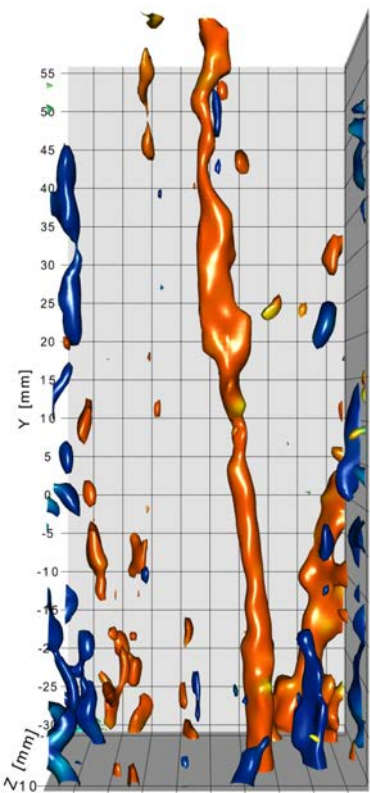

90246

296

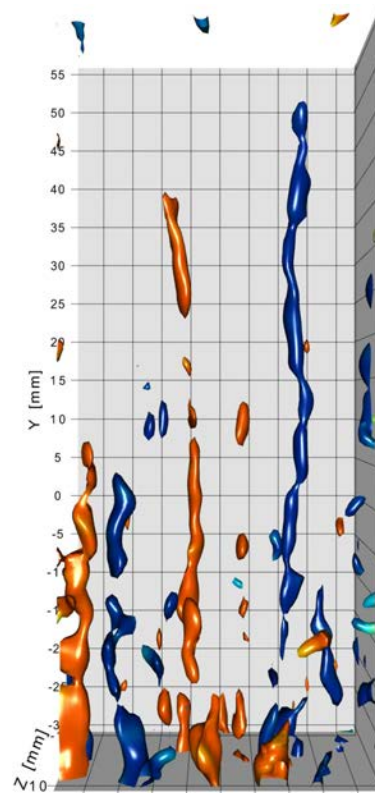

90688

297

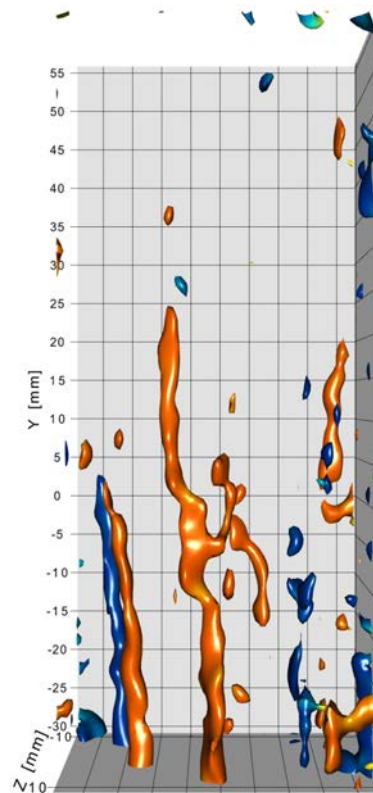

91455

298

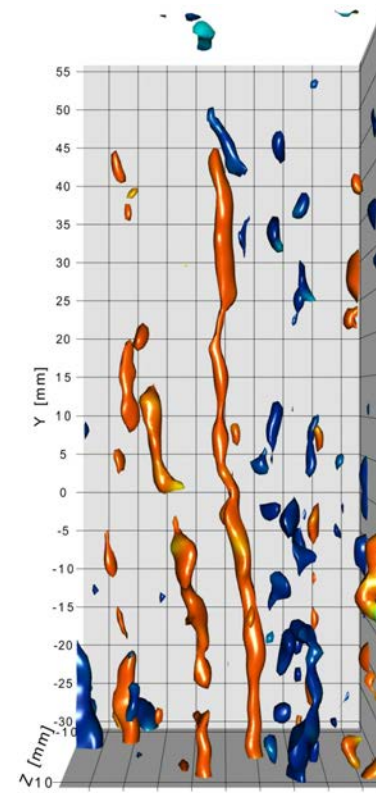

93530

299

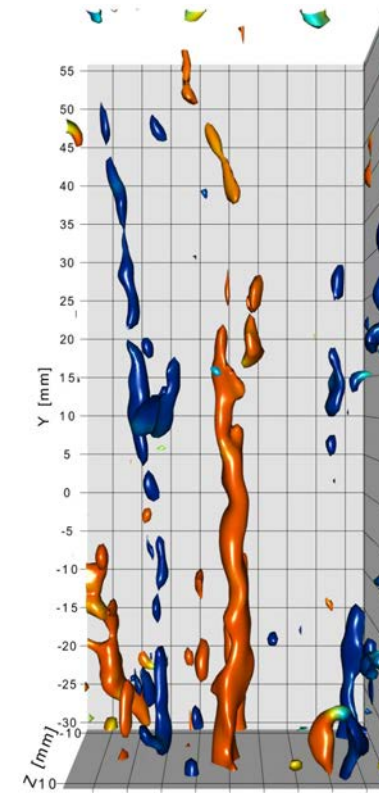

95397

300

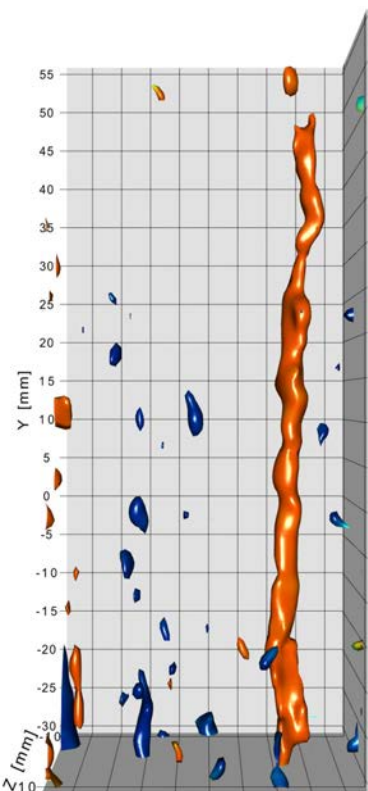

97277

301

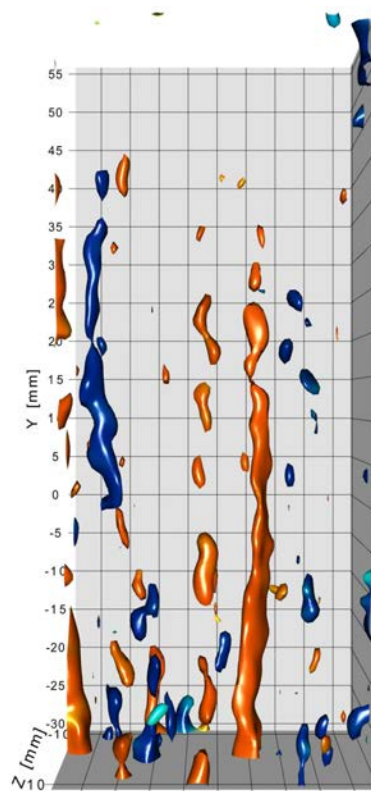

97822

302

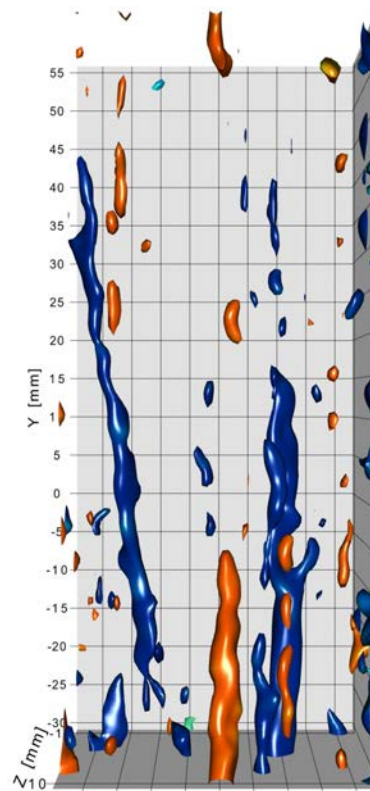

99764

303

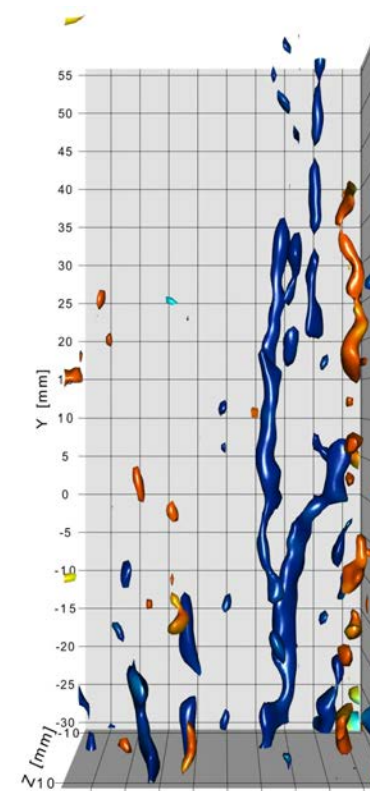

101151

304

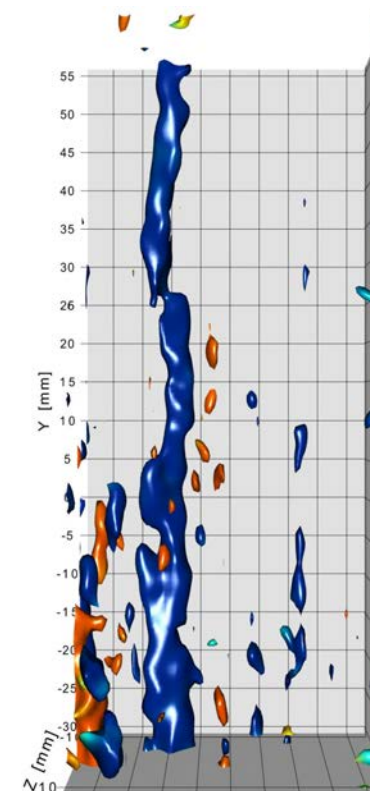

103207

305



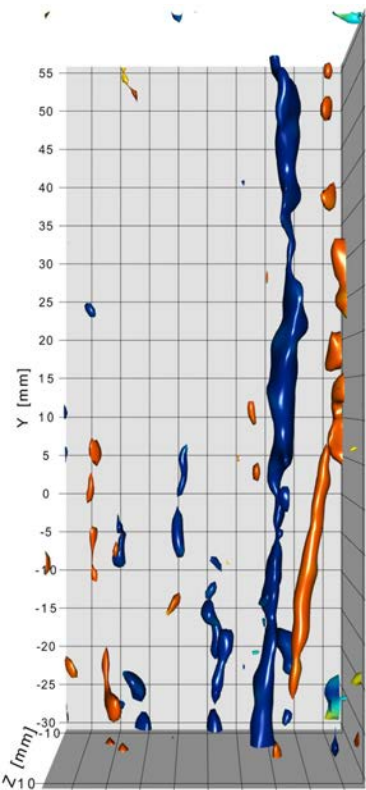

104022

306

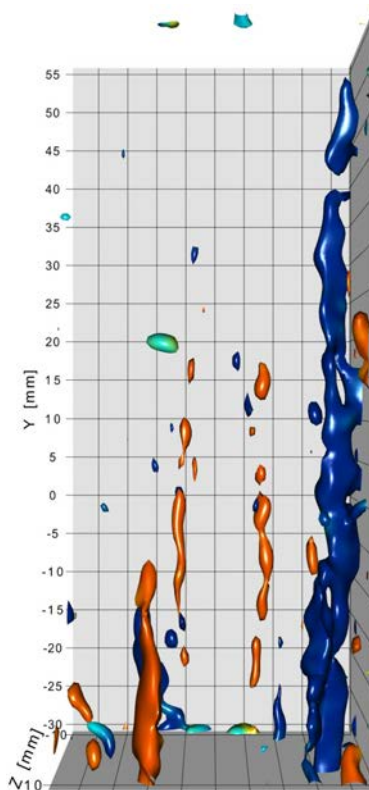

105307

307

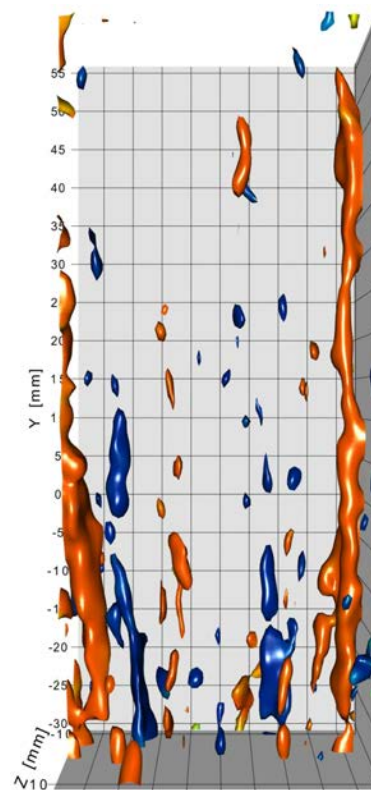

105815

308

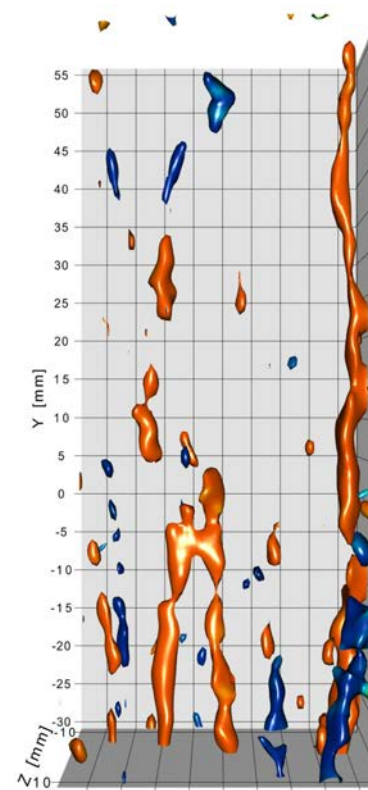

106859

309

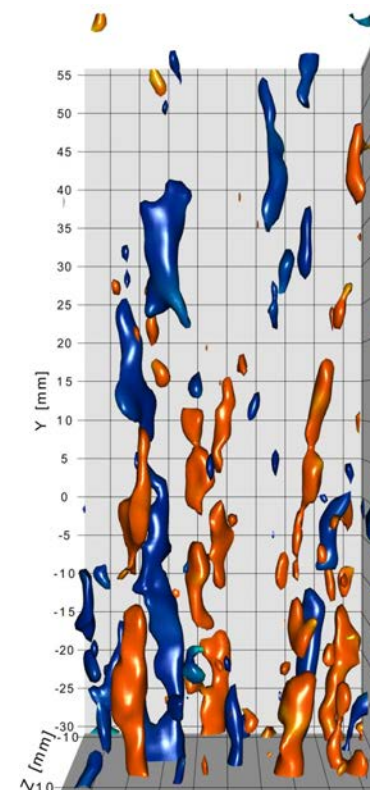

107157

310

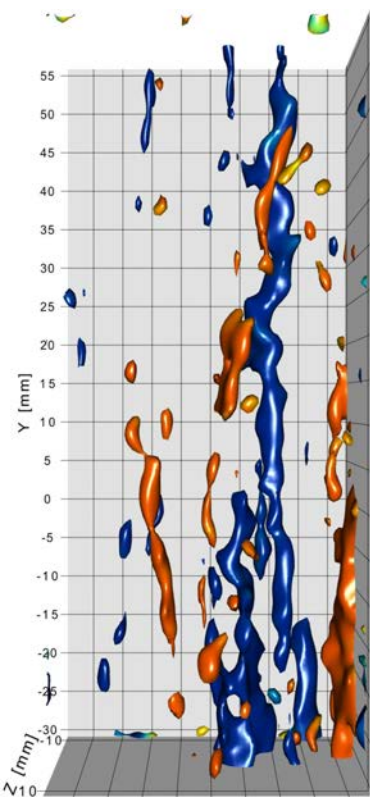

107693

311

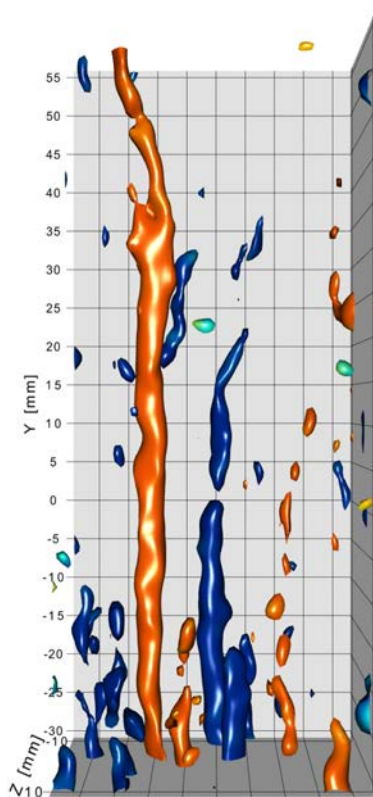

108238

312

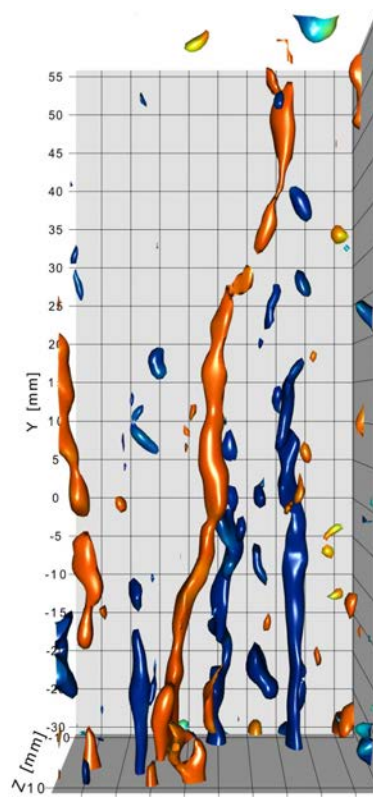

108706

313

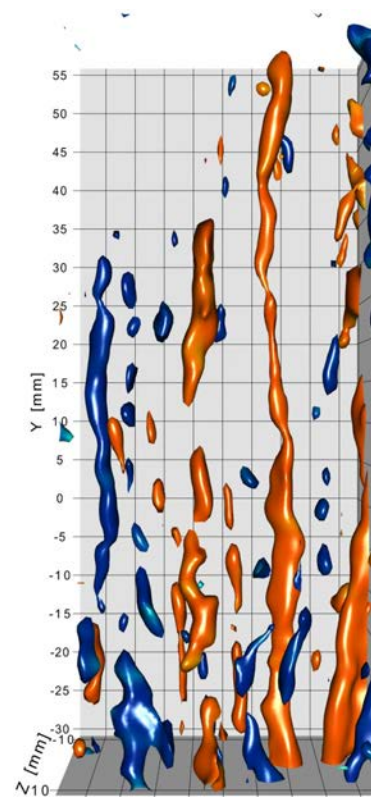

108933

314

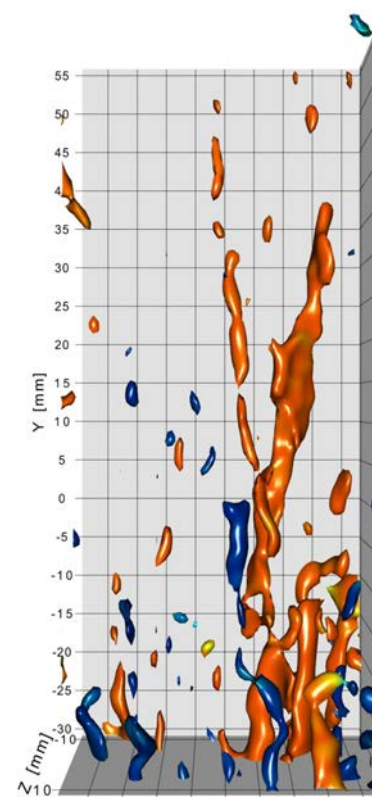

109446

315



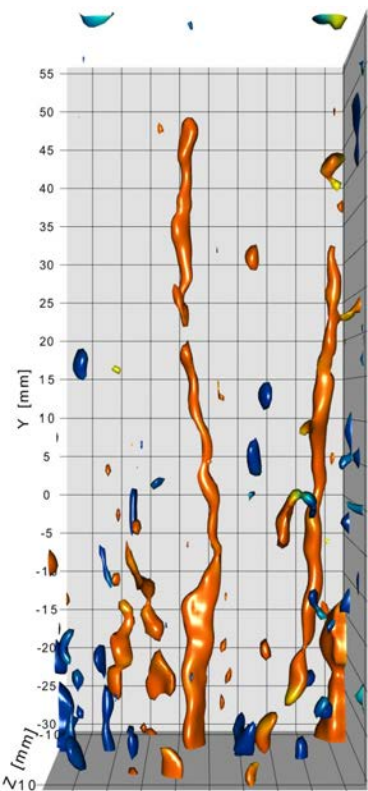

111023

316

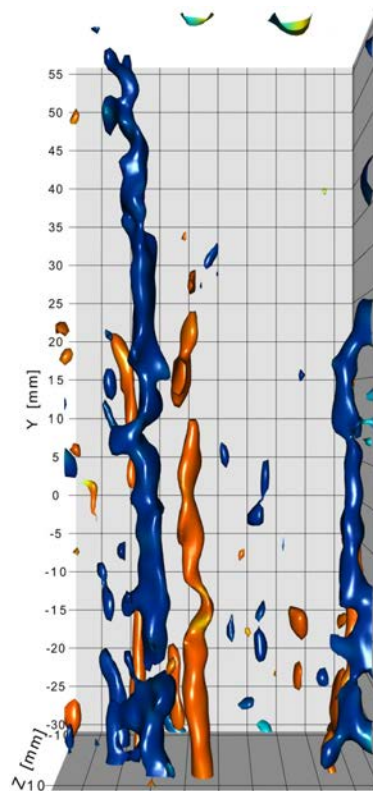

111333

317

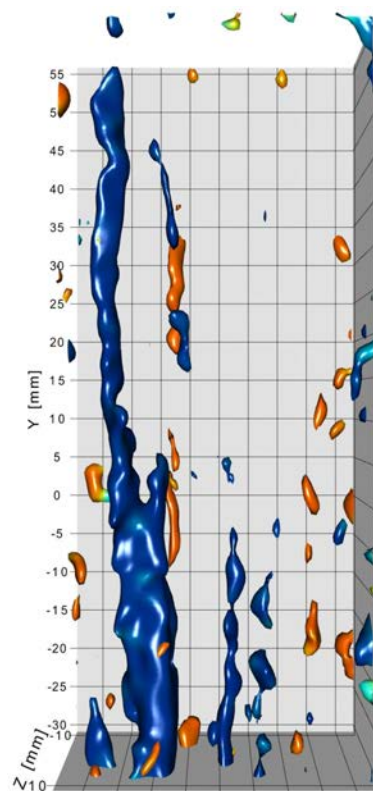

111504

318

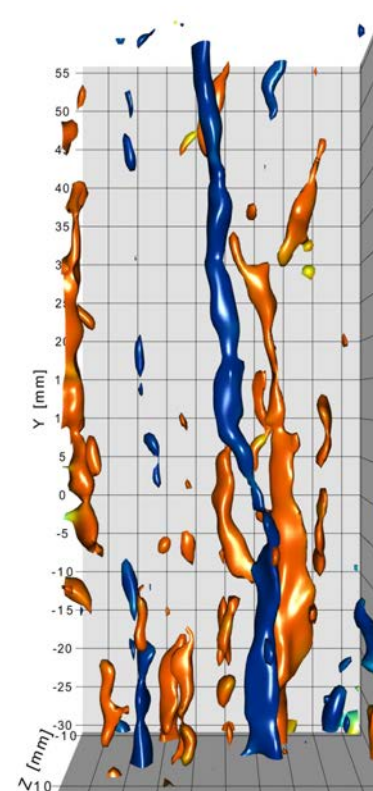

113128

319

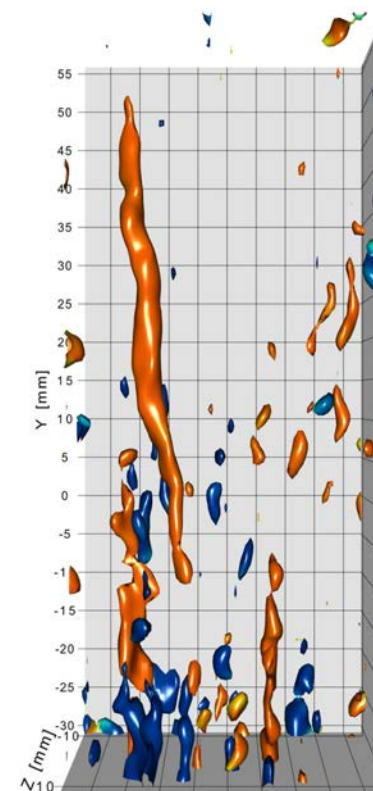

113717

320



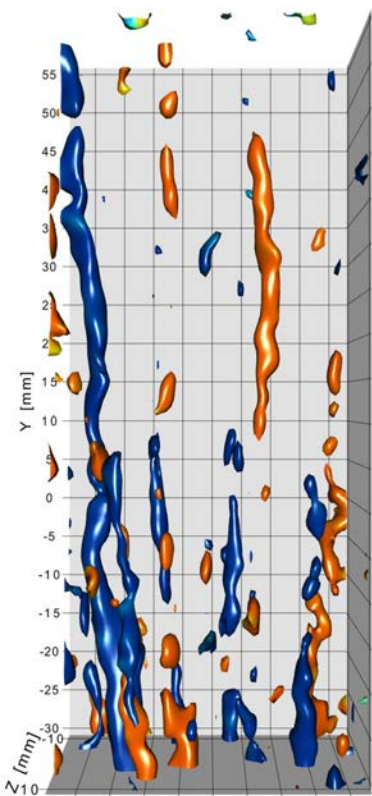

114788

321

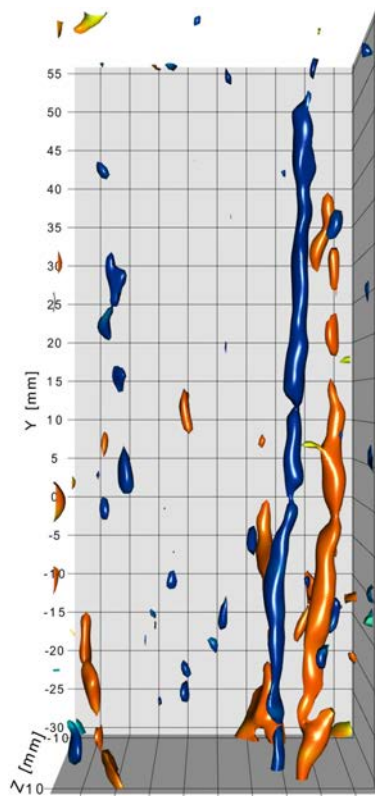

115789

322

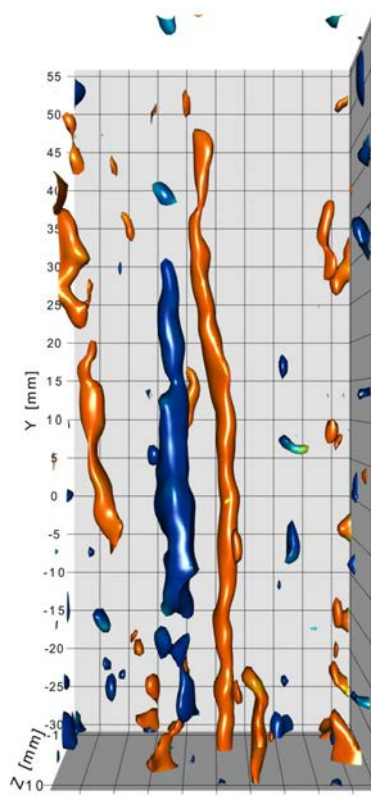

116353

323

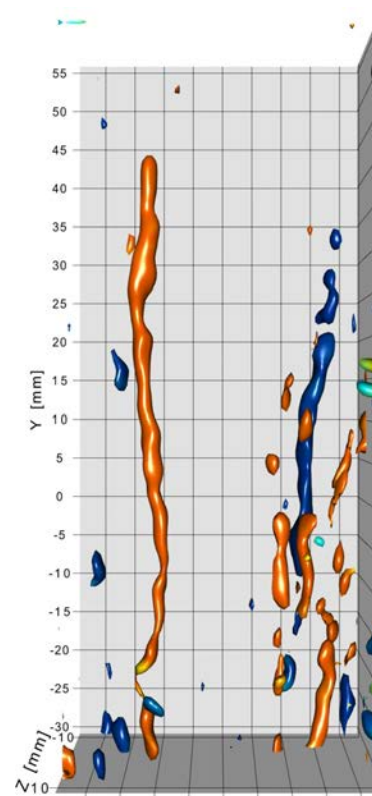

118981

324

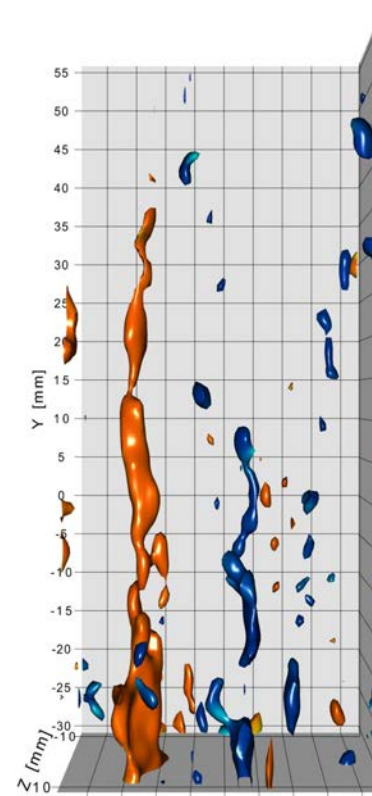

119837

325

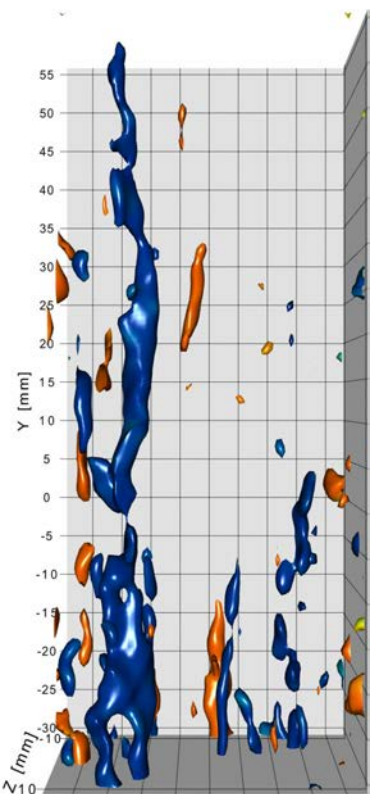

120502

326

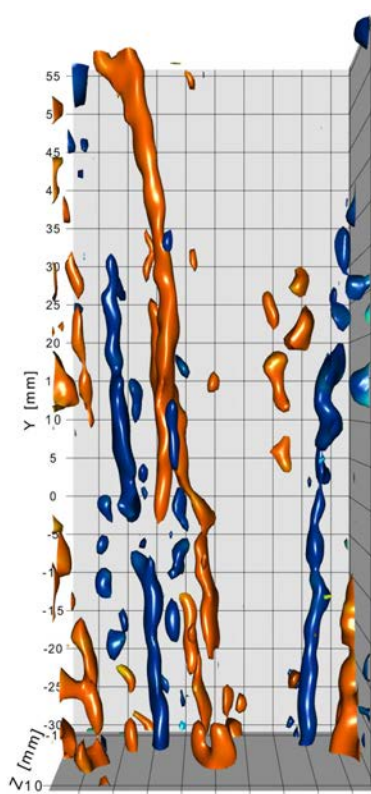

120833

327

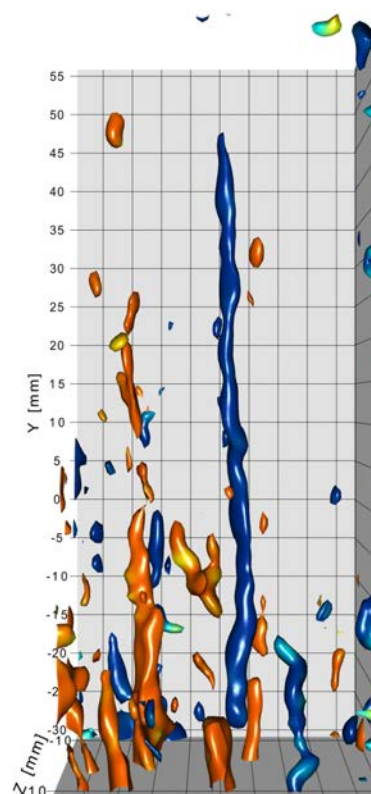

121243

328

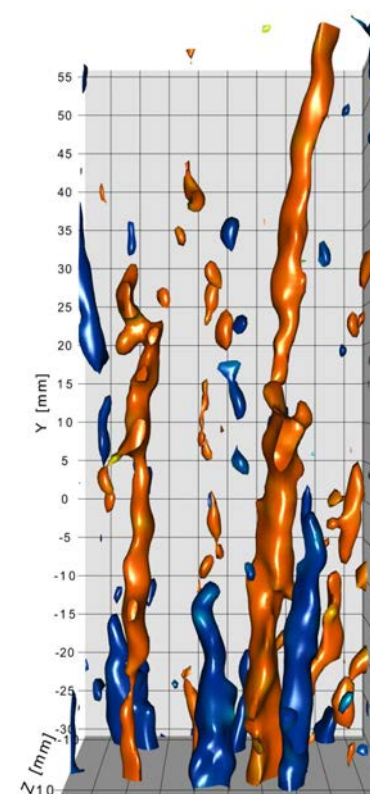

122233

329

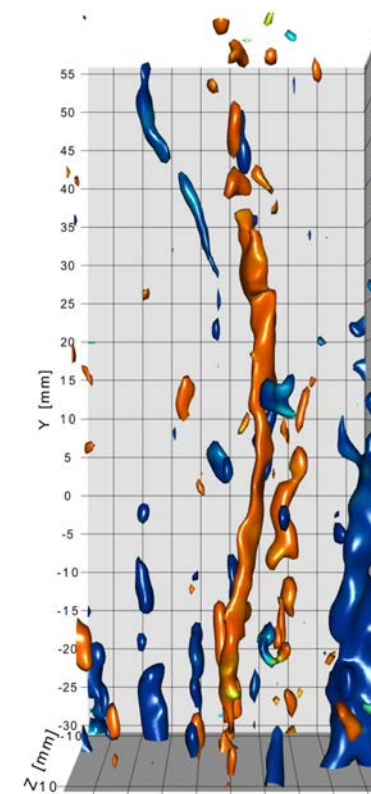

122692

330



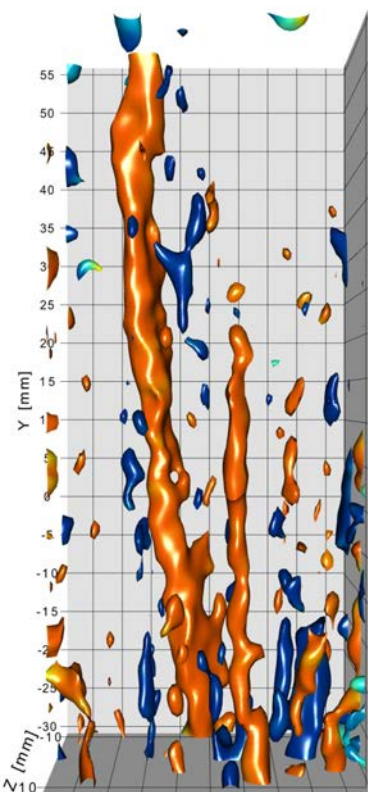

123286

331

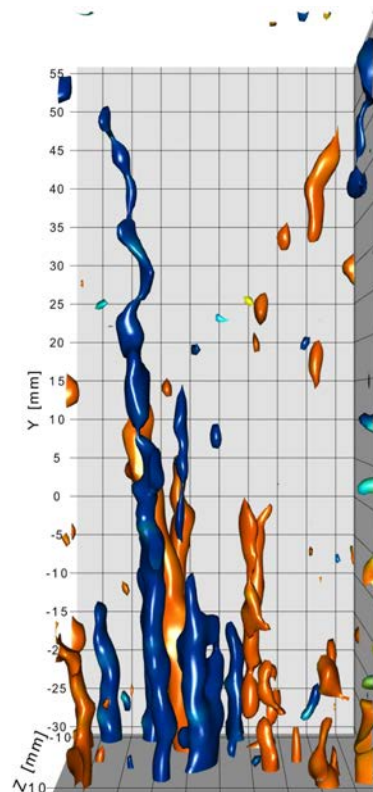

123549

332

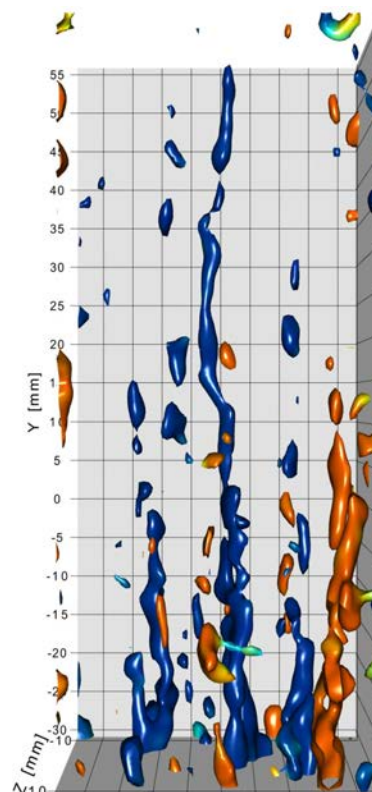

124354

333

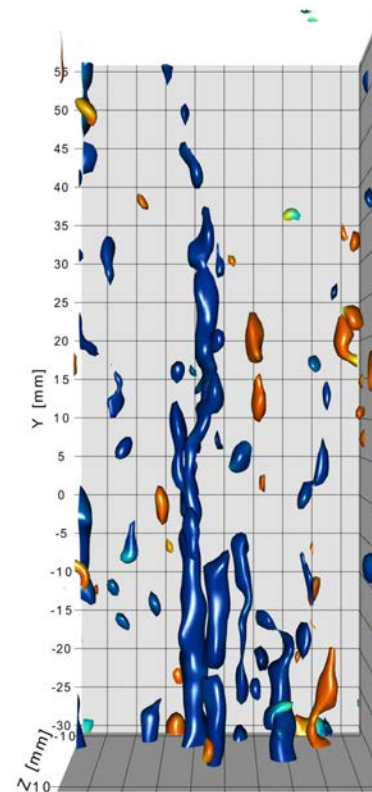

124544

334

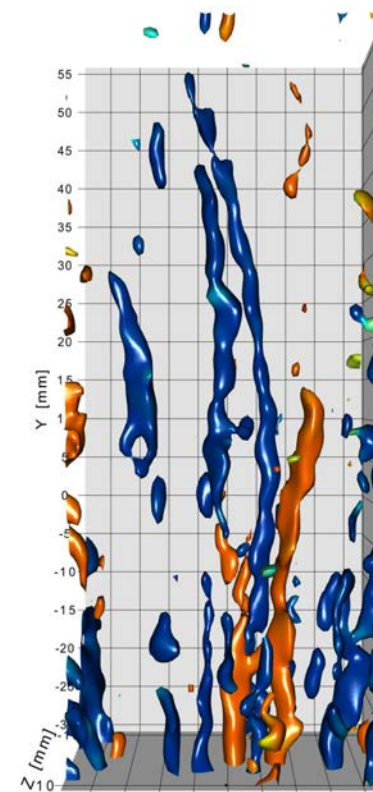

126671

335



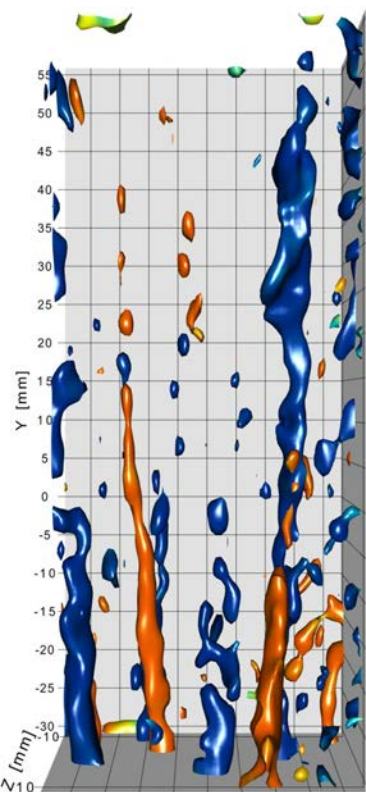

127134

336

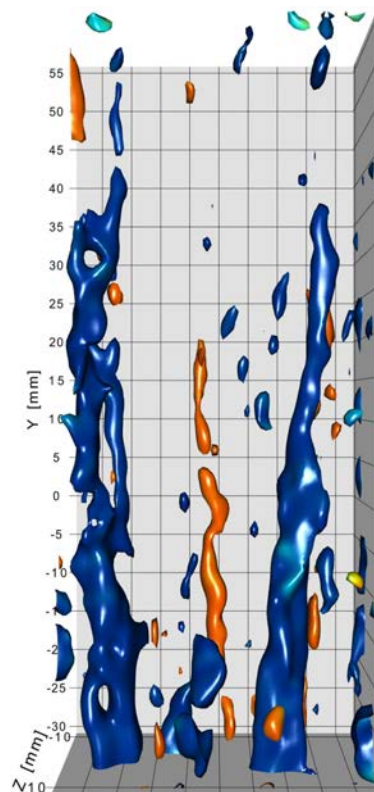

127270

337

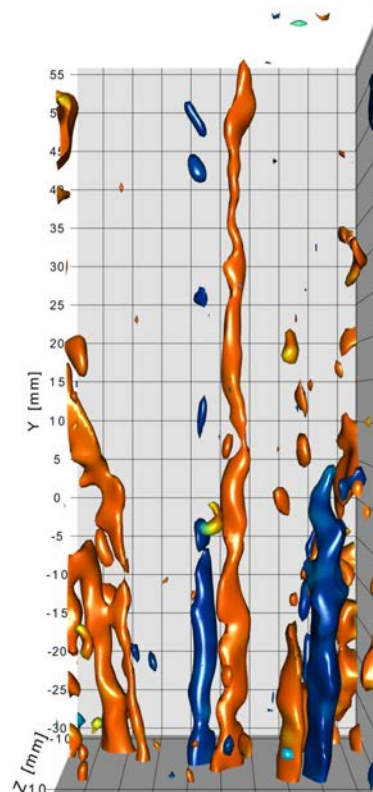

128171

338

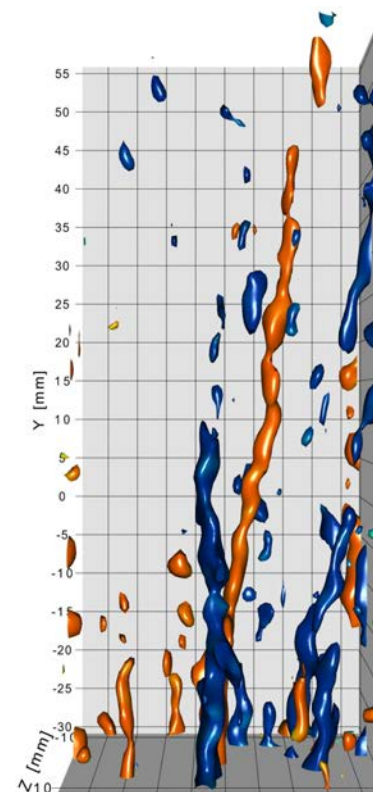

129201

339

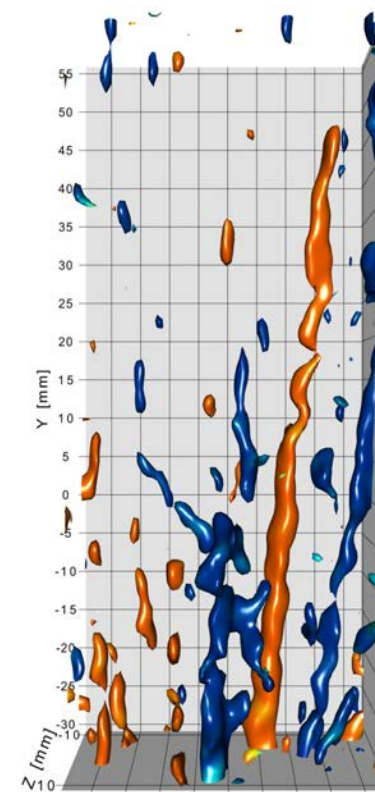

129299

340

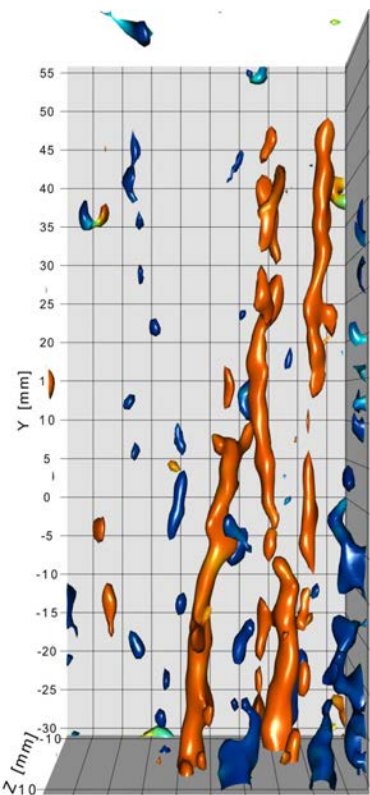

129603

341

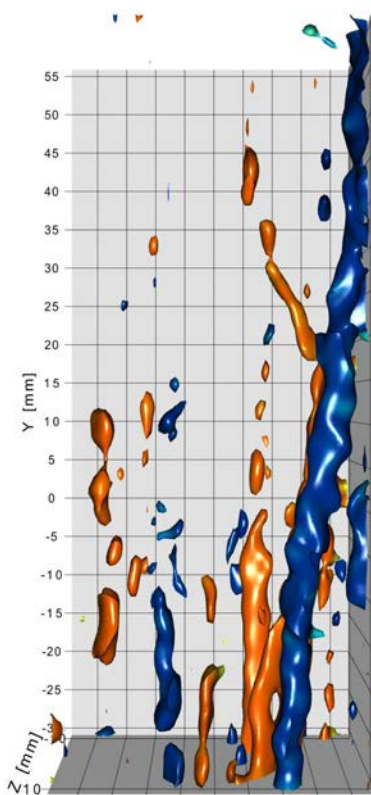

129754

342

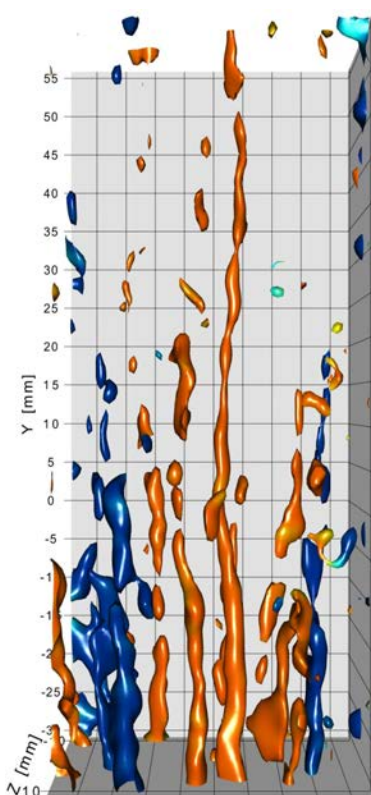

130187

343

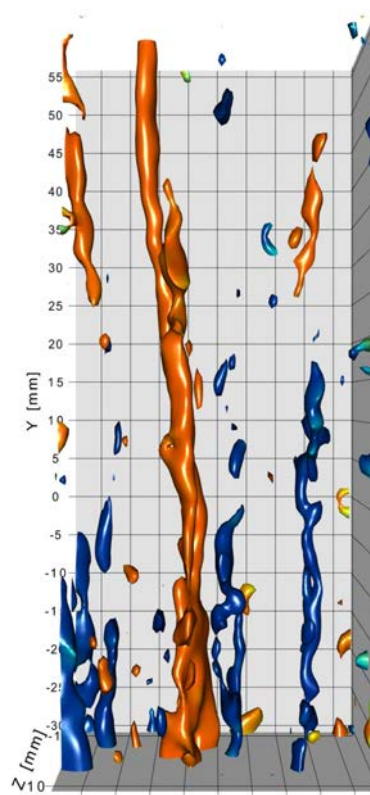

130589

344

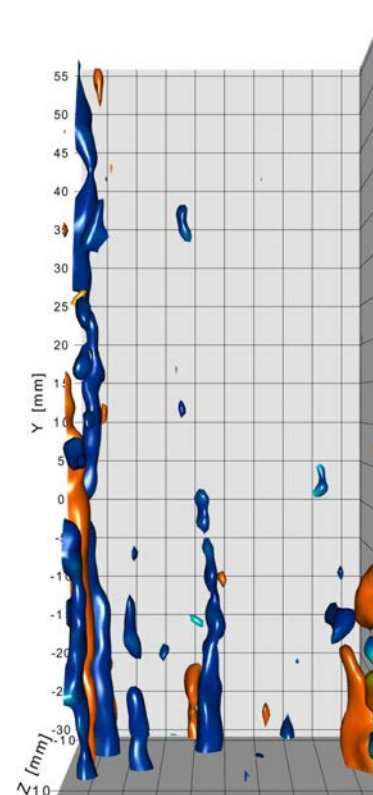

131420

345



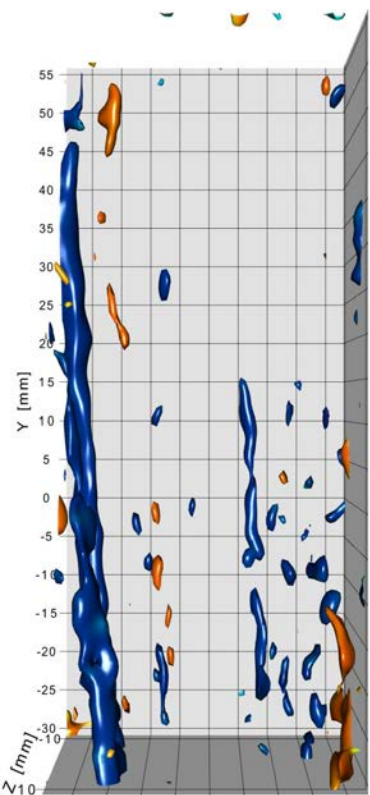

131711

346

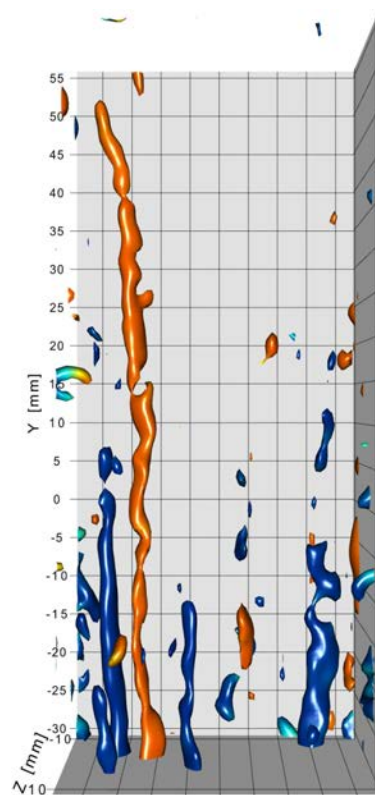

131848

347

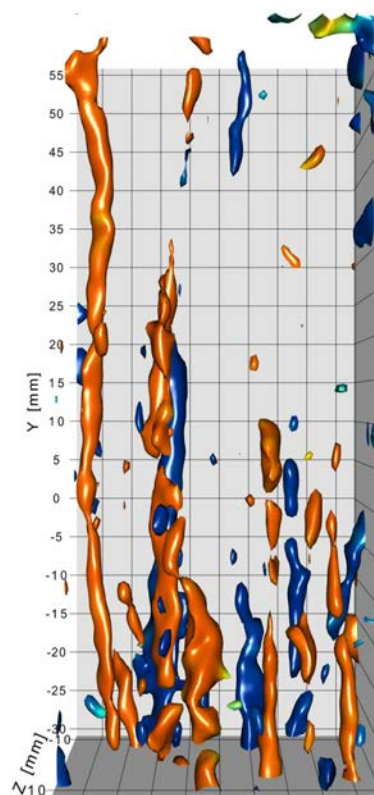

133023

348

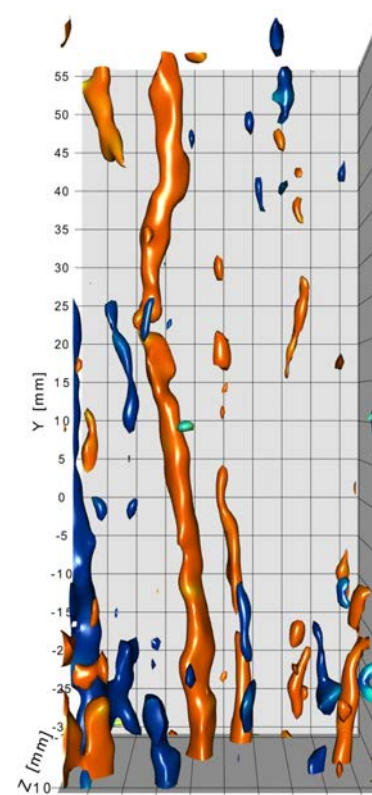

133894

349

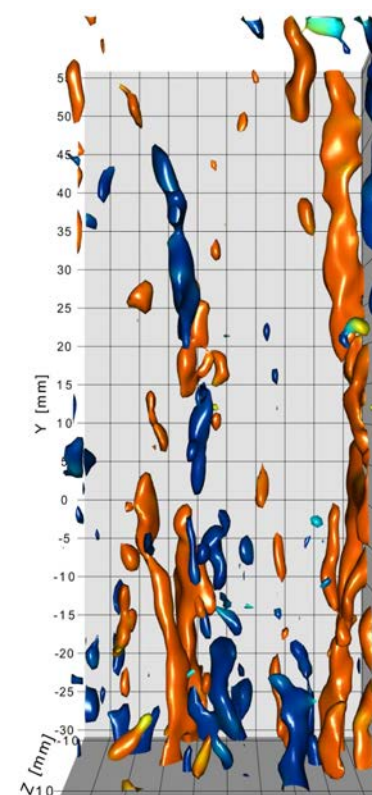

134299

350



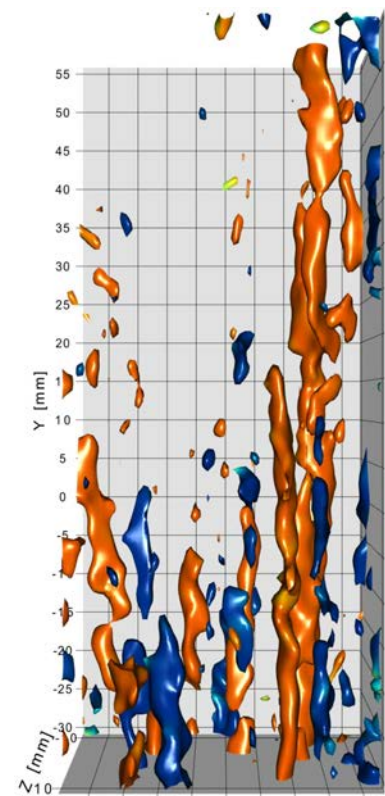

134517

351

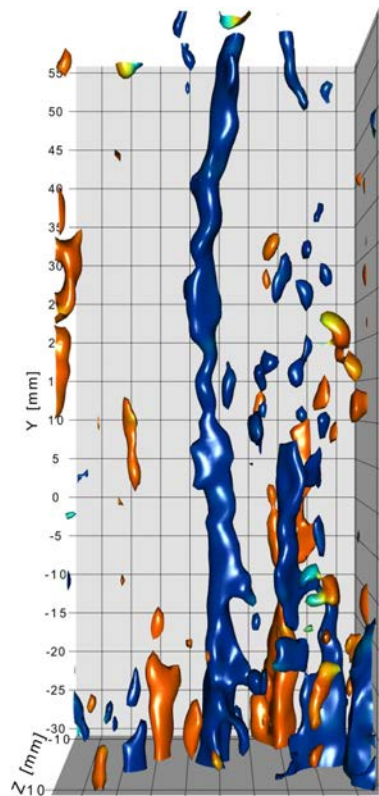

134957

352

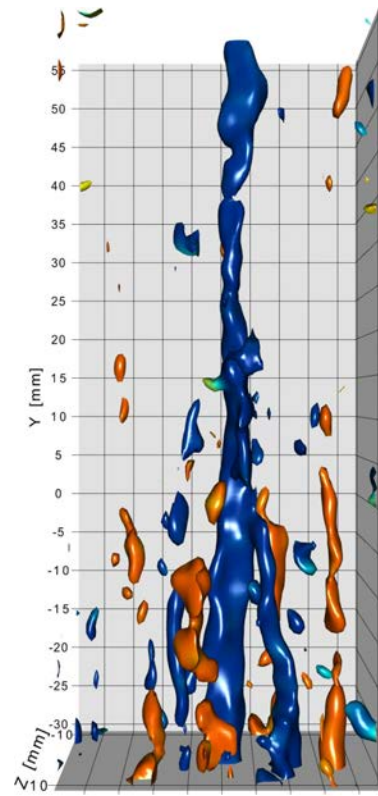

135163

353

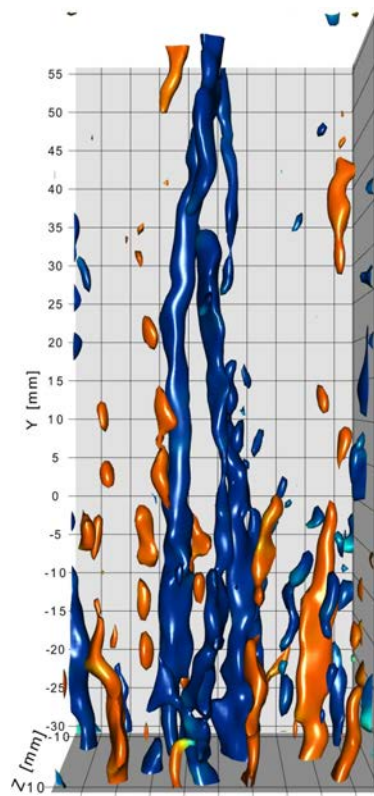

135435

354

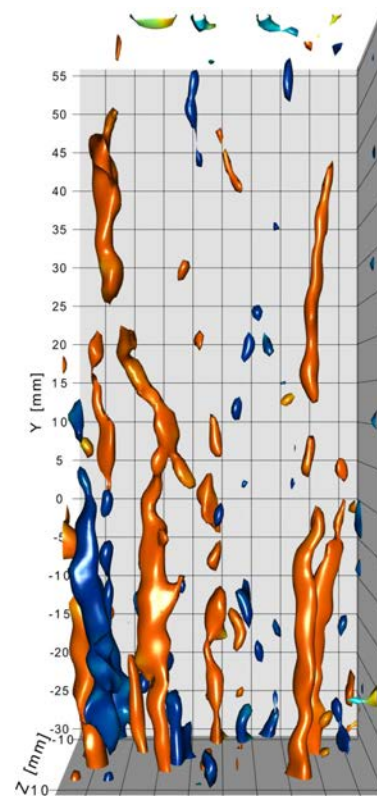

136175

355
