# Supplementary material for: Coherent turbulent structures in a rapid contraction
Source: arXiv:2401.05869 source file (2024-01-11)
Supplement: Supplementary file 3 [file StrRun3.pdf]

# Run3

Iso-surface of  $|\omega| = 40 \text{ } ^1/s$

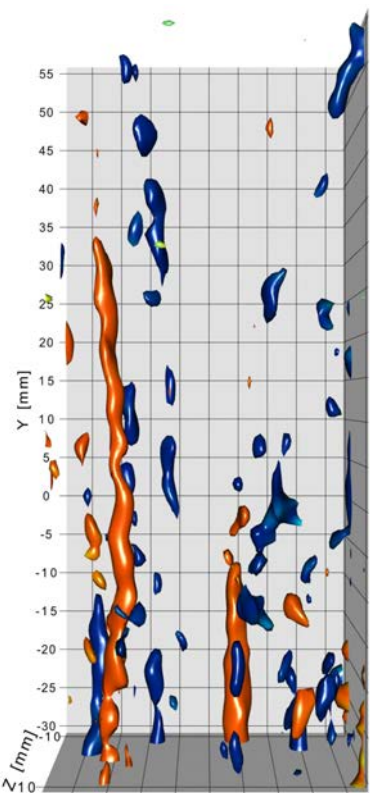

1491

356

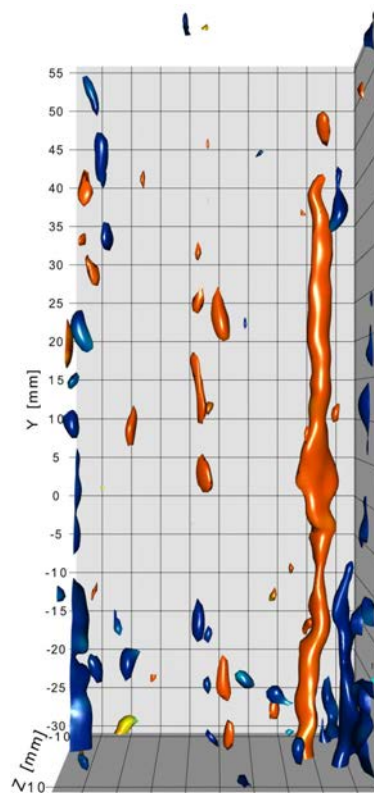

1994

357

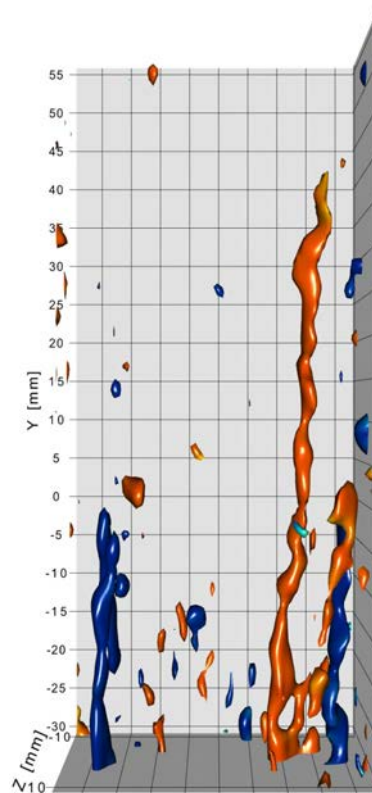

2237

358

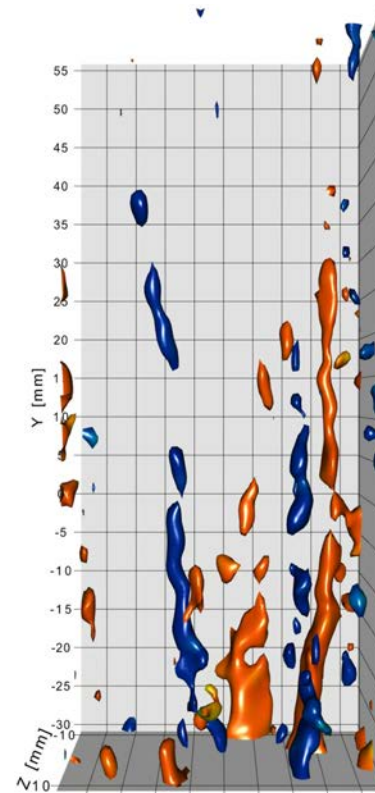

2805

359

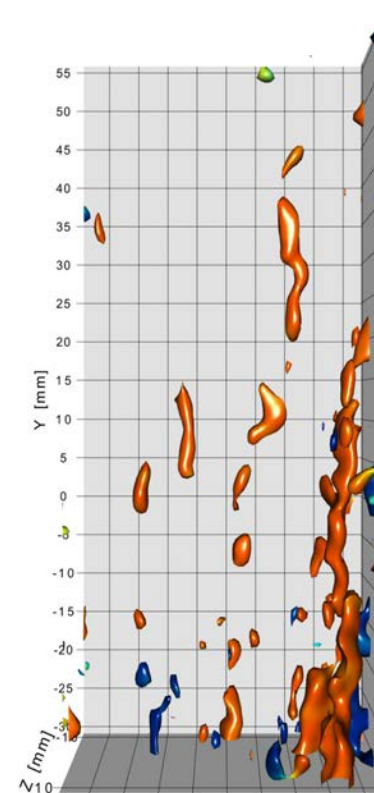

3115

360

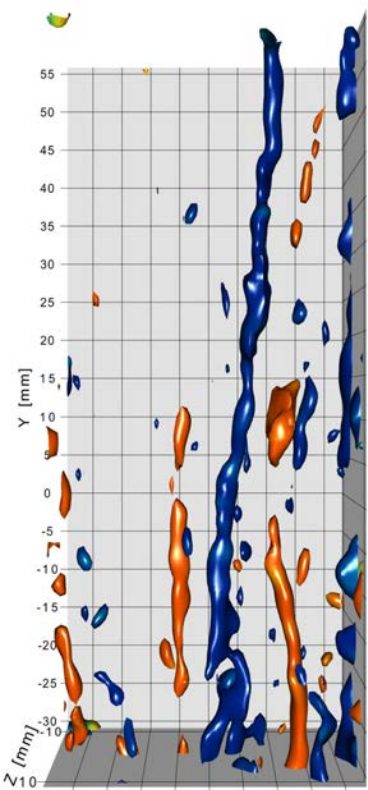

3786

361

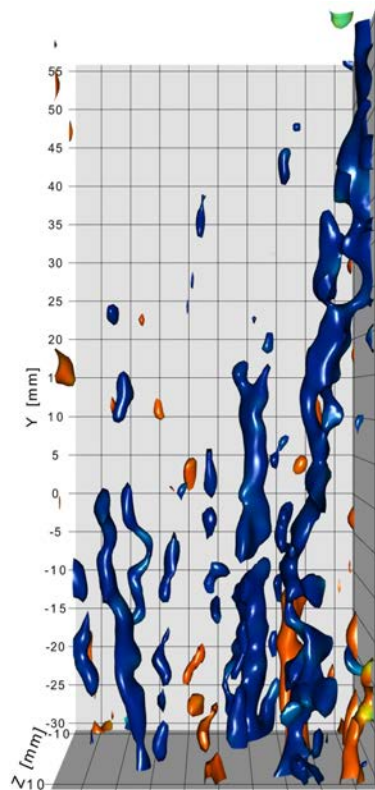

4939

362

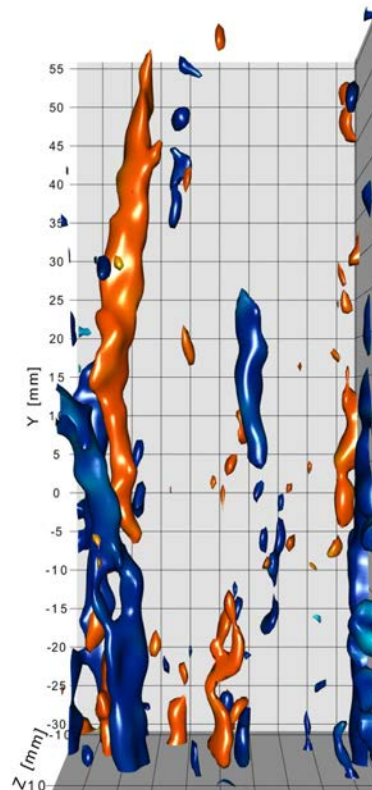

5515

363

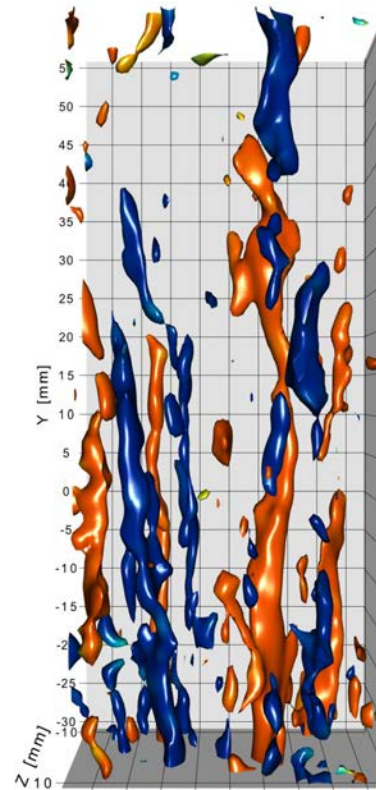

5996

364

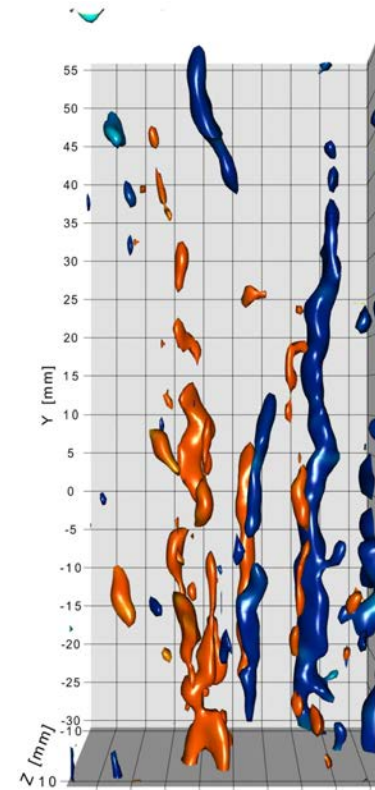

6628

365



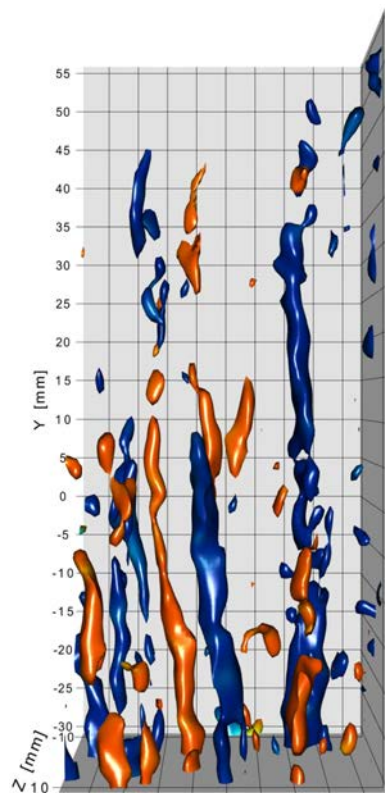

6788

366

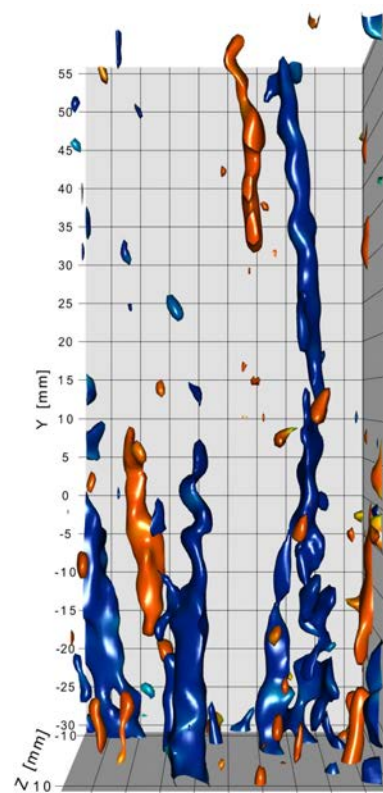

7117

367

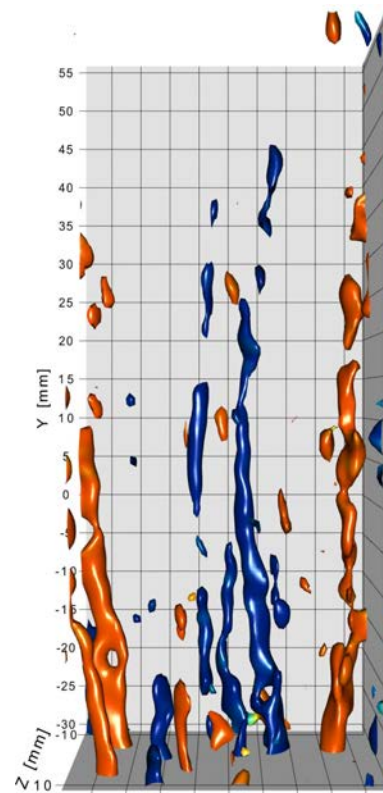

7536

368

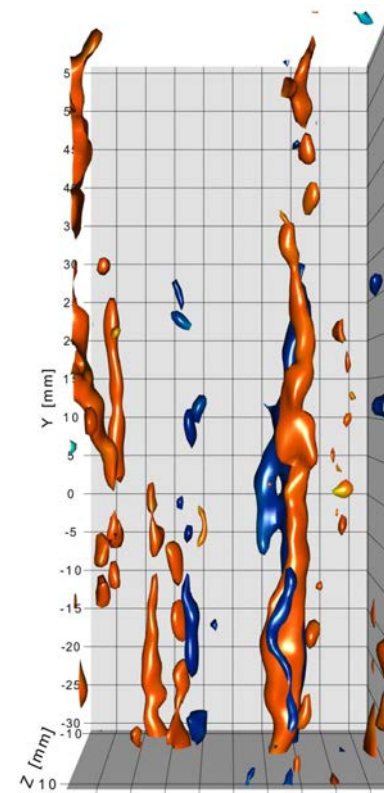

8557

369

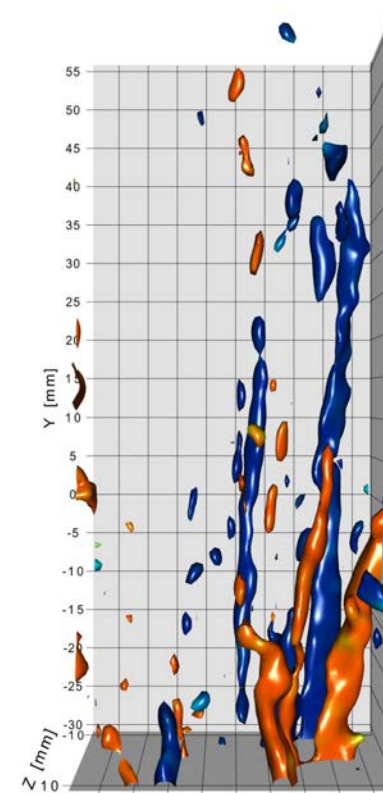

8861

370

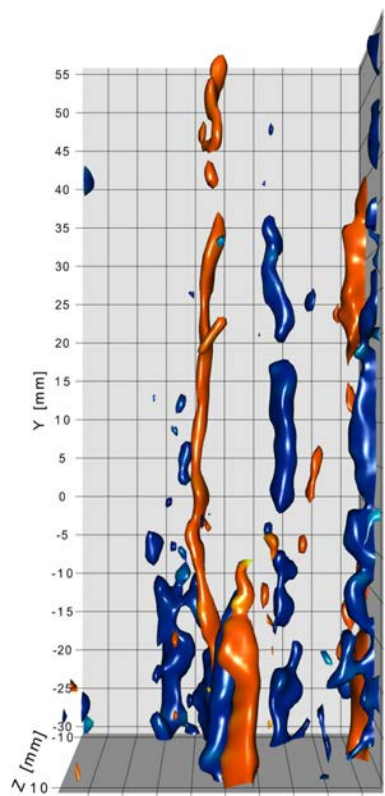

9430

371

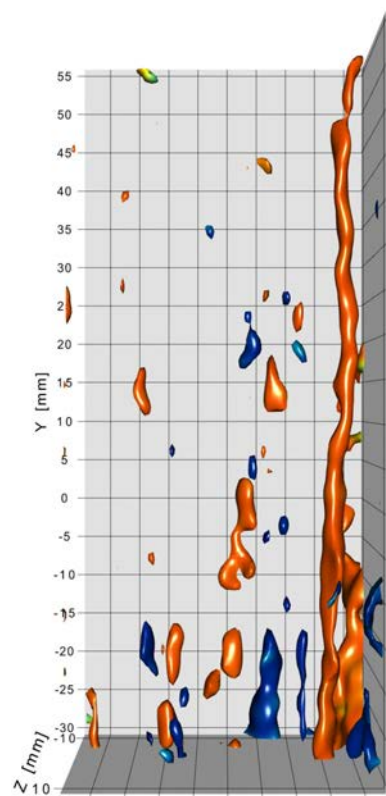

10322

372

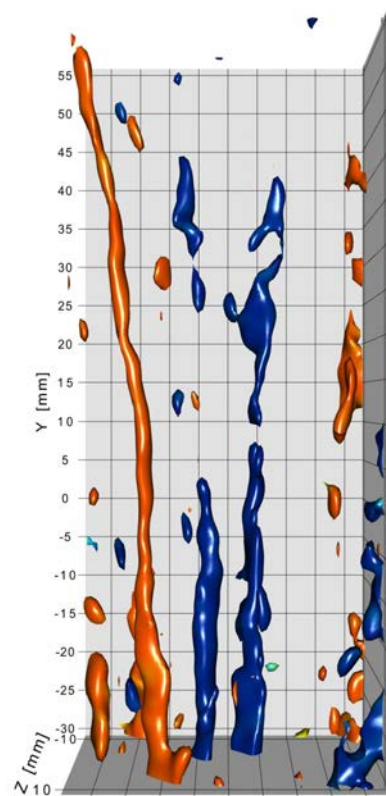

10858

373

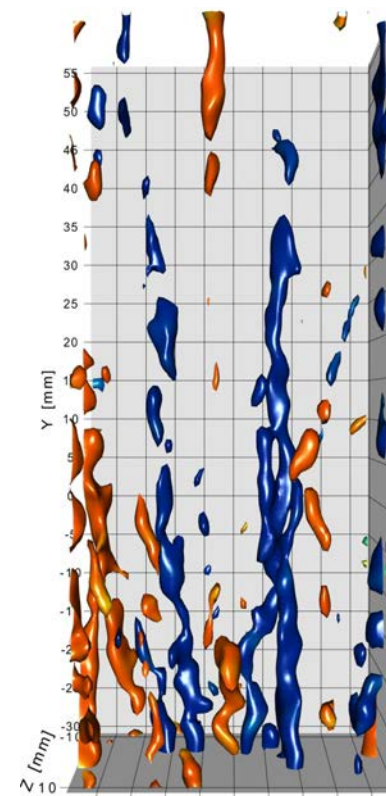

11296

374

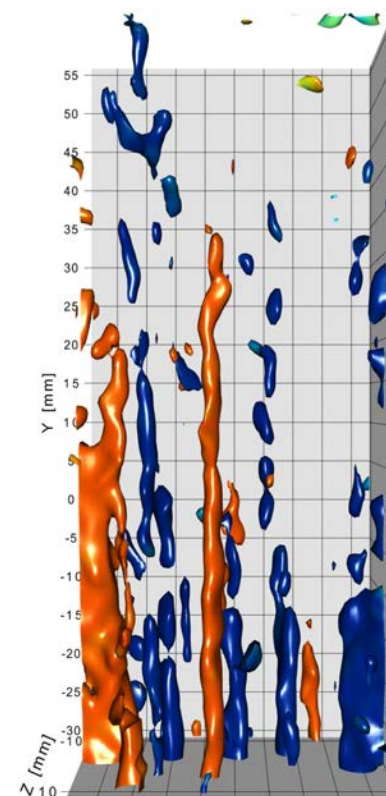

11474

375

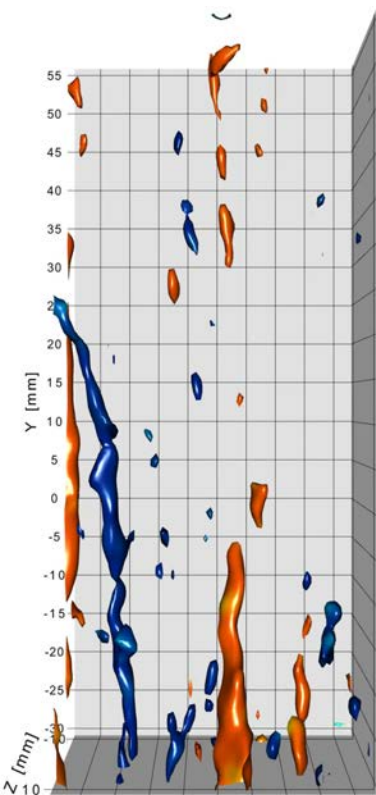

12191

376

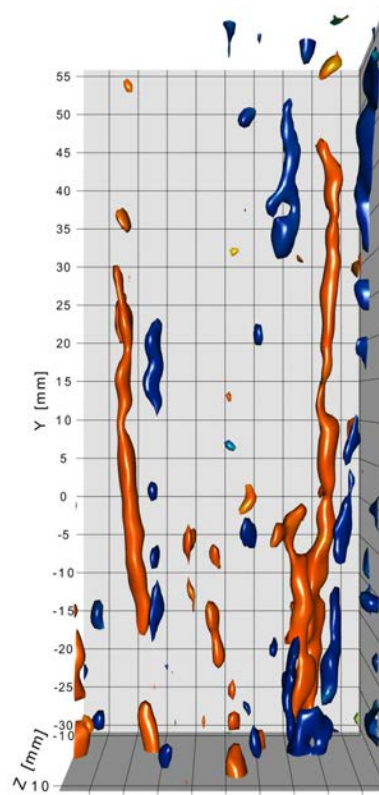

12533

377

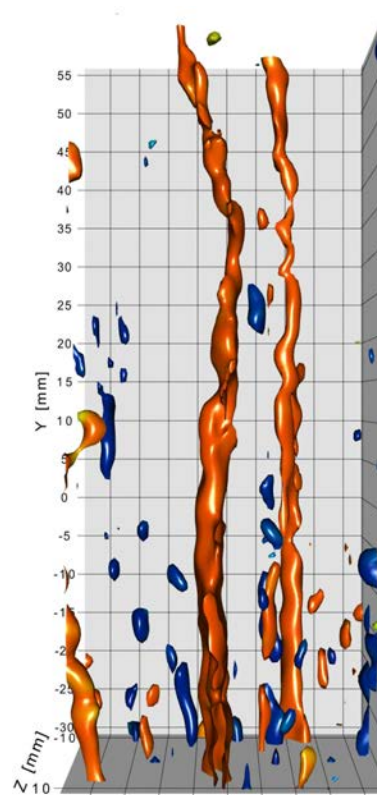

13783

378

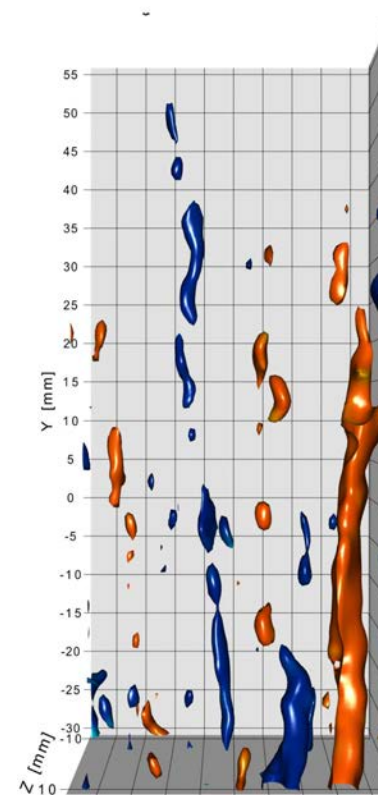

15620

379

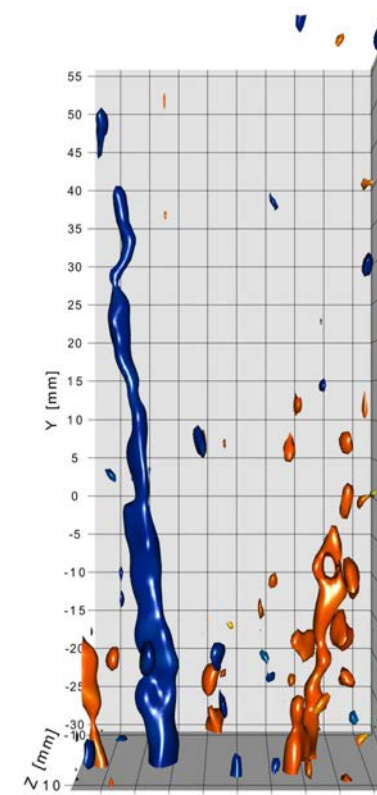

15939

380



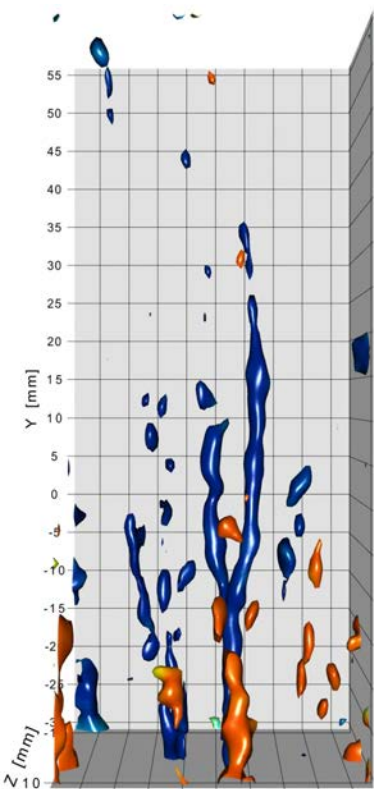

16935

381

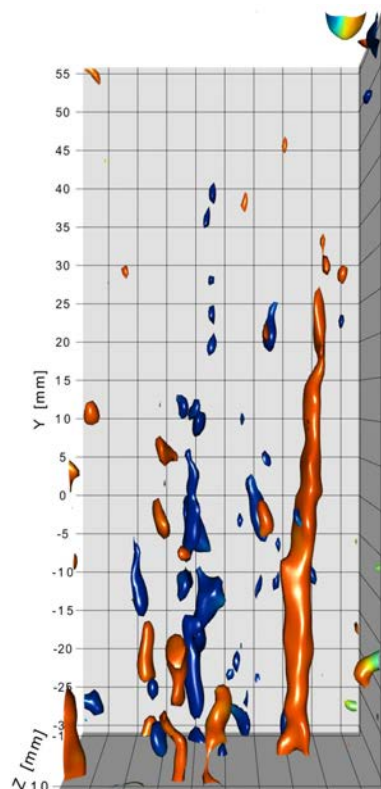

20209

382

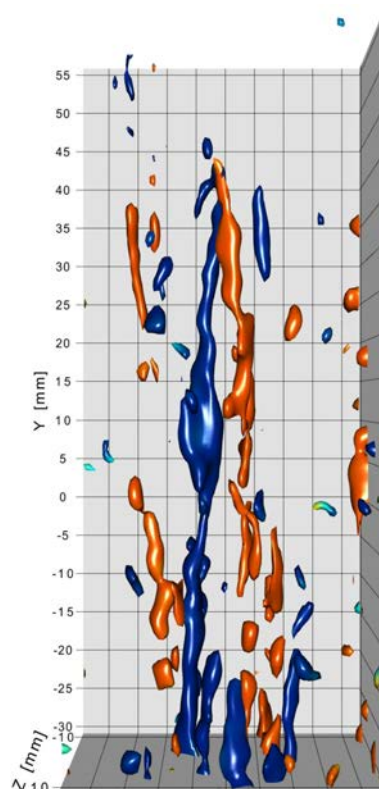

21523

383

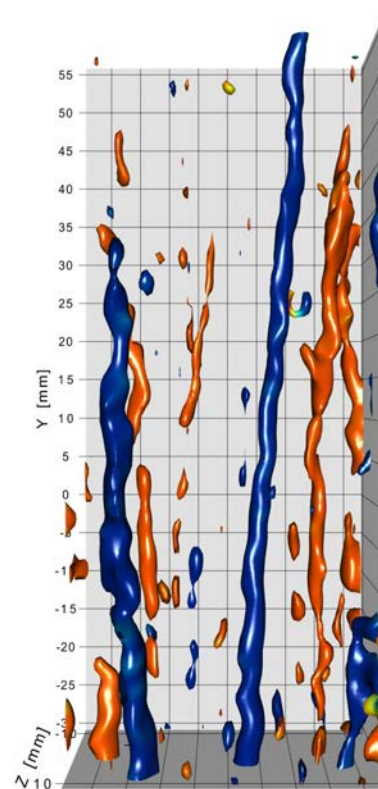

26239

384

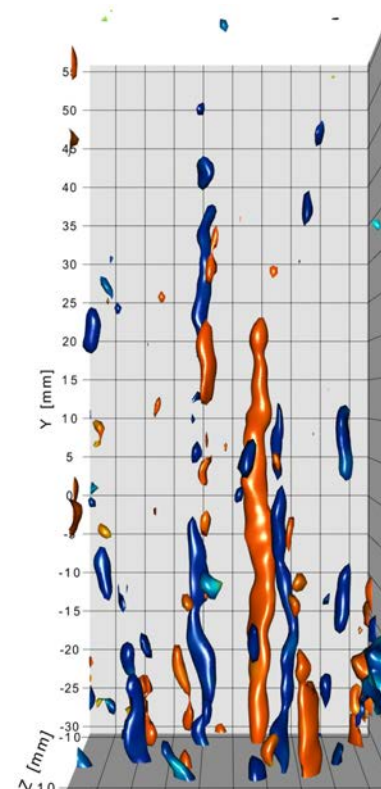

26596

385

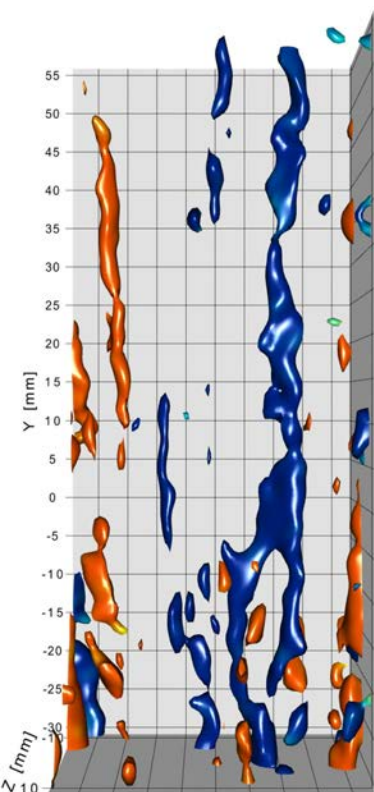

29164

386

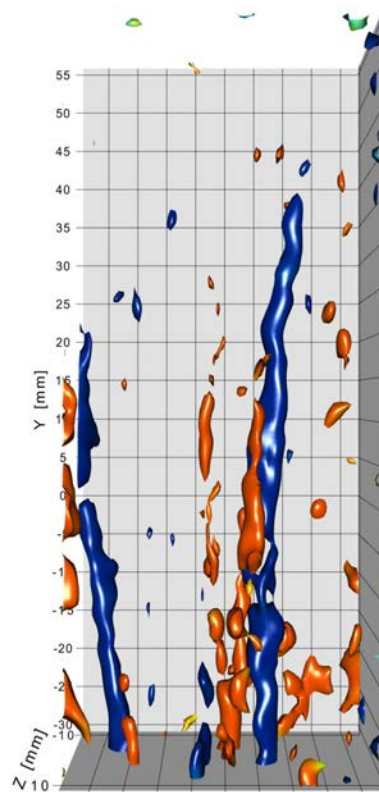

29697

387

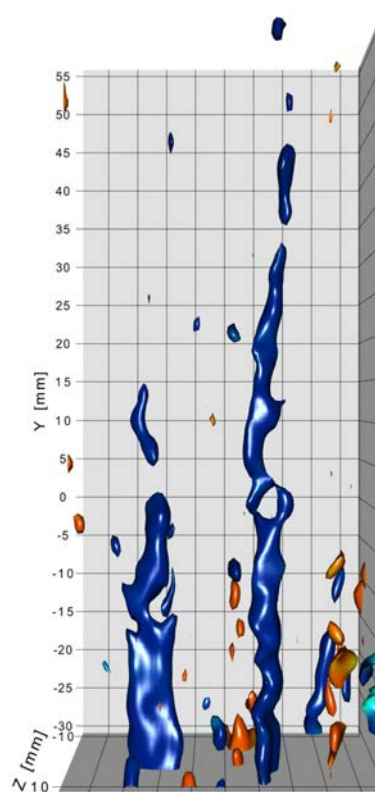

30223

388

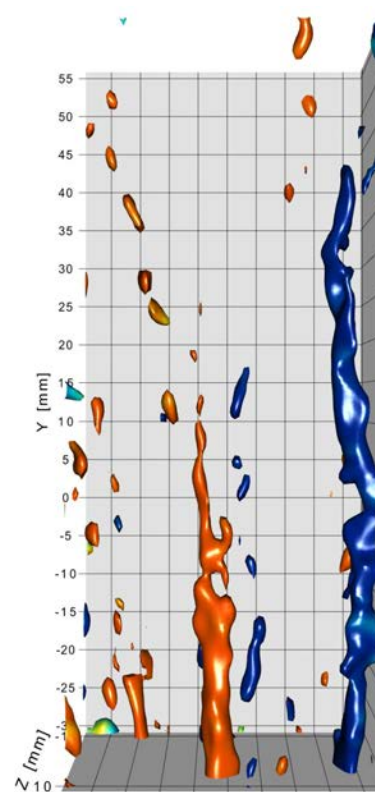

30748

389

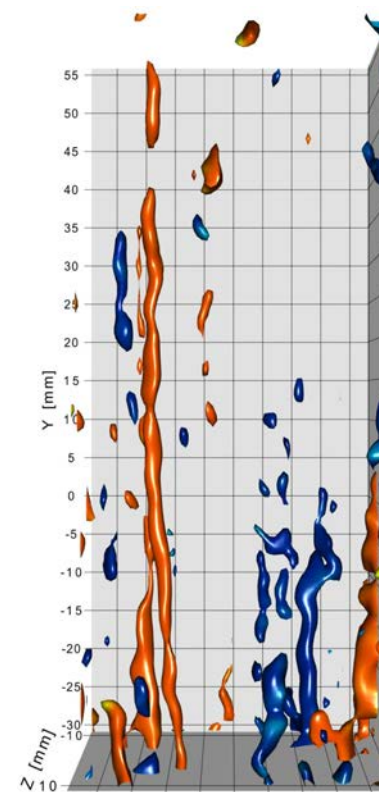

34438

390



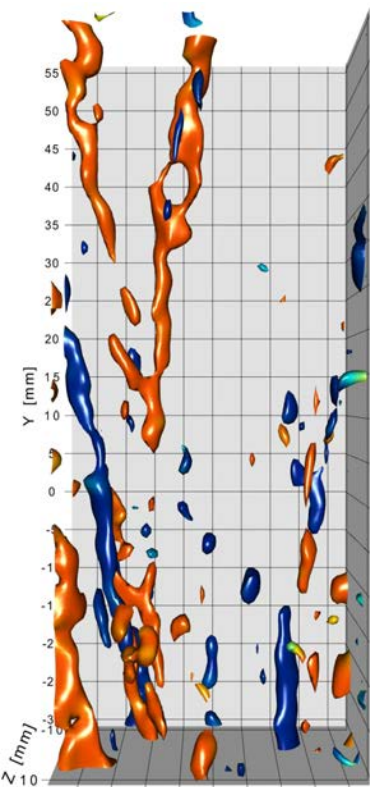

36286

391

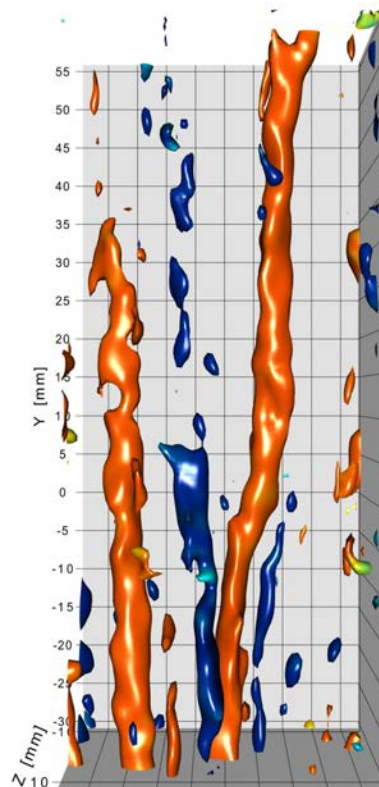

36531

392

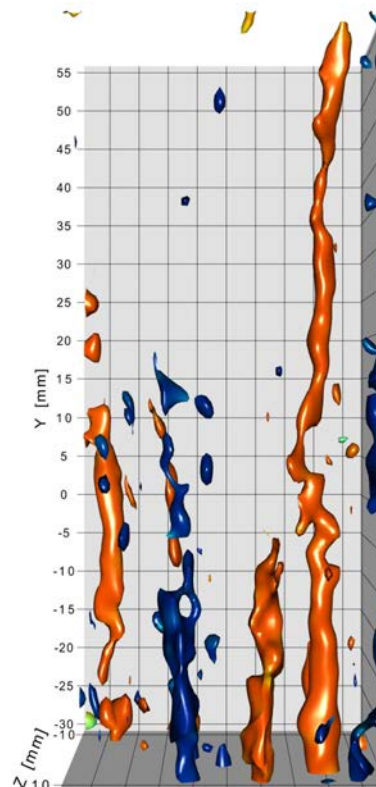

37053

393

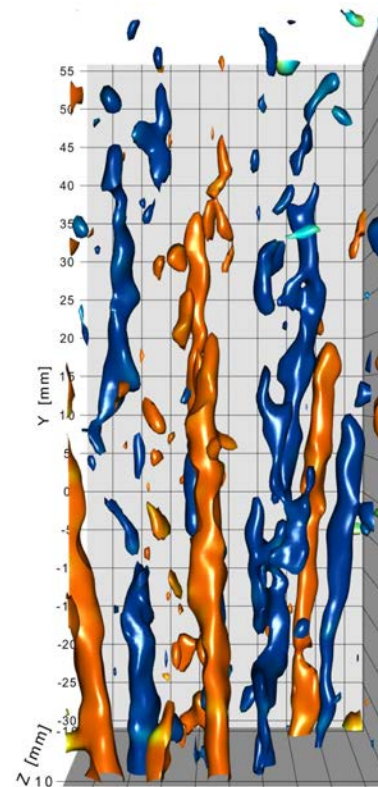

38993

394

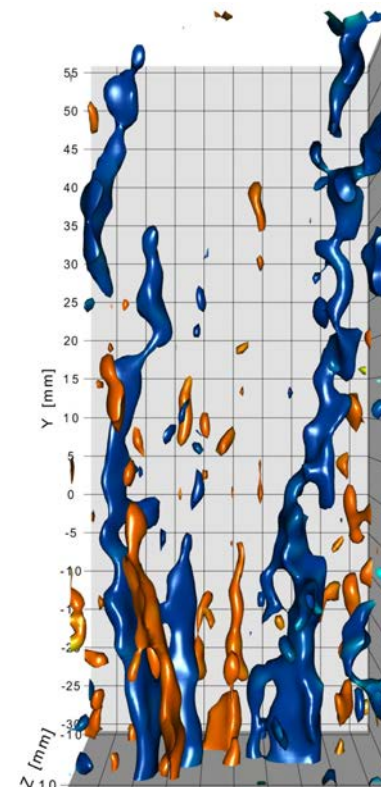

39184

395

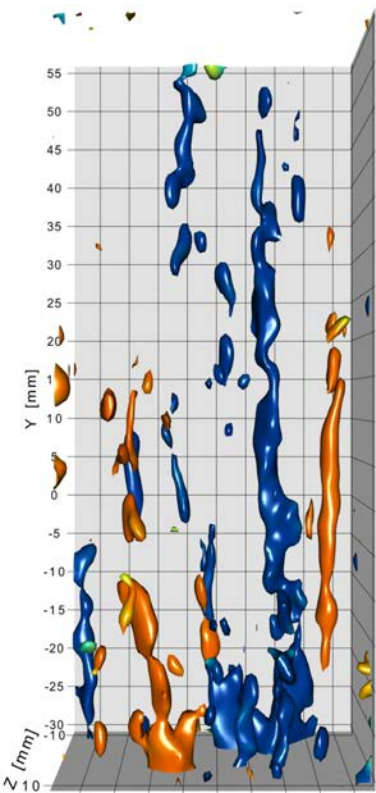

39952

396

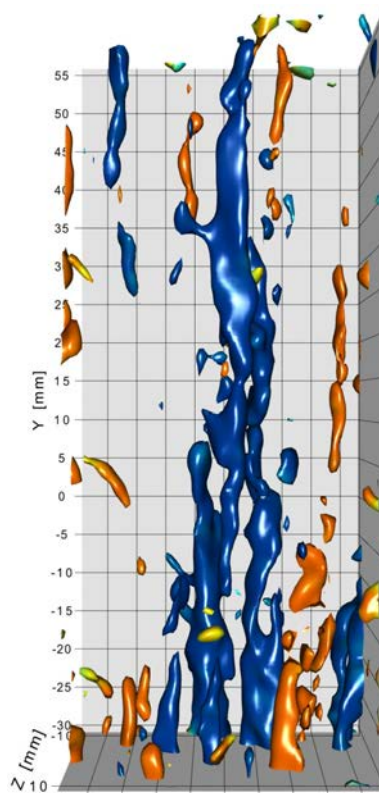

40144

397

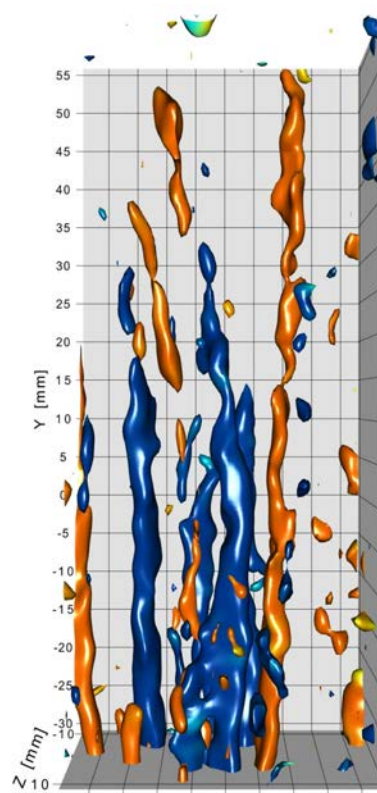

40346

398

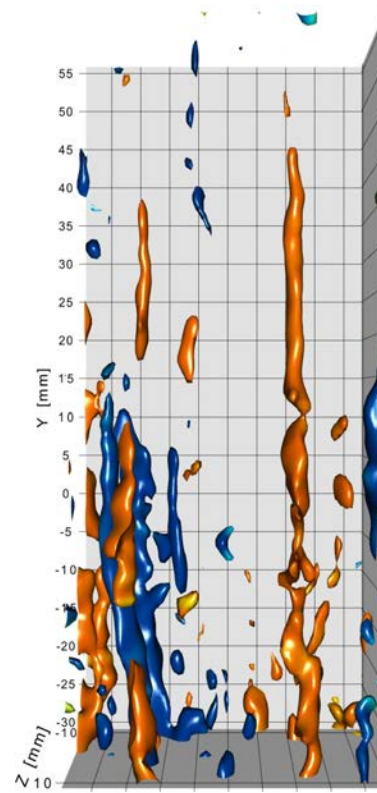

40903

399

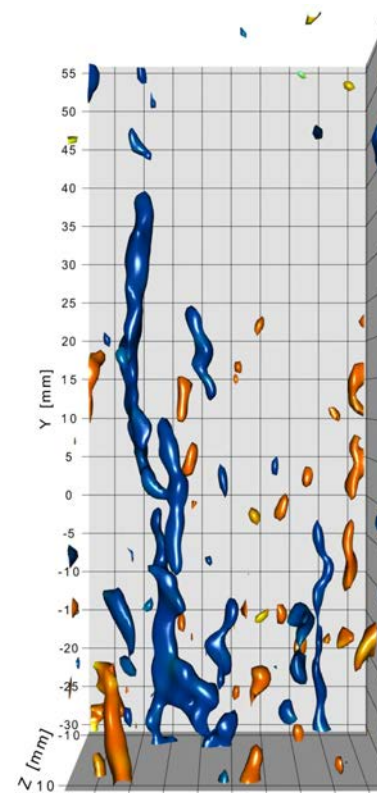

42149

400



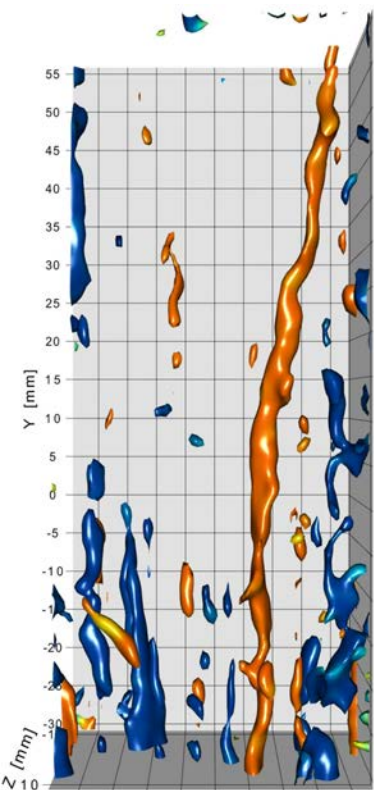

42477

401

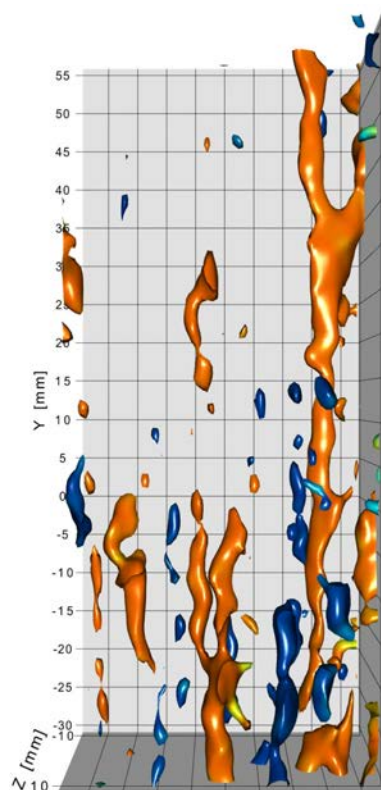

42963

402

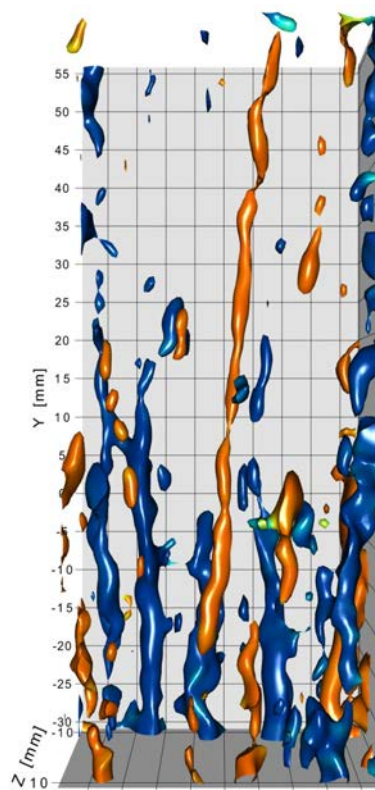

44047

403

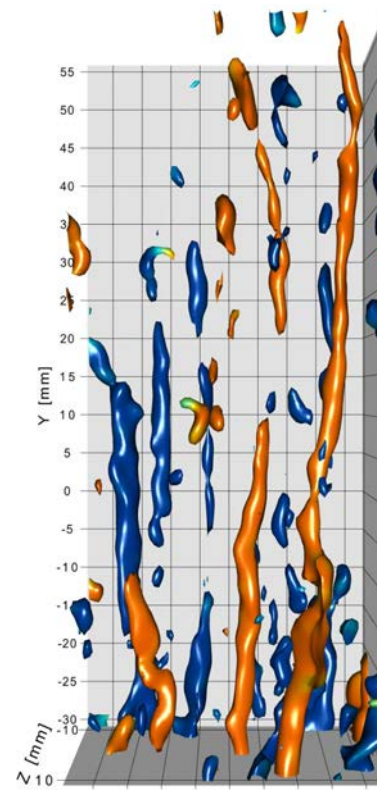

44201

404

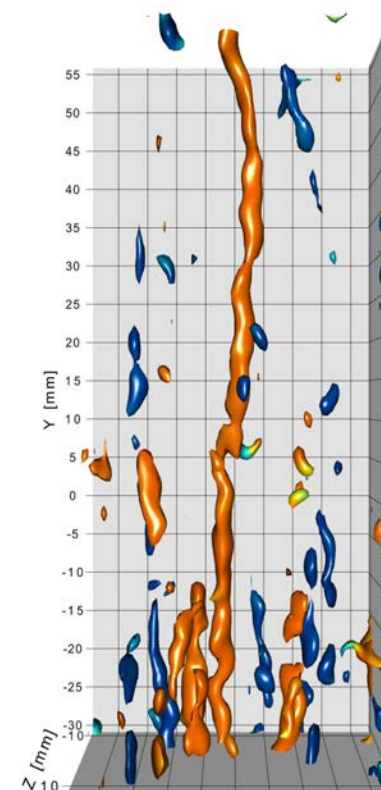

47074

405



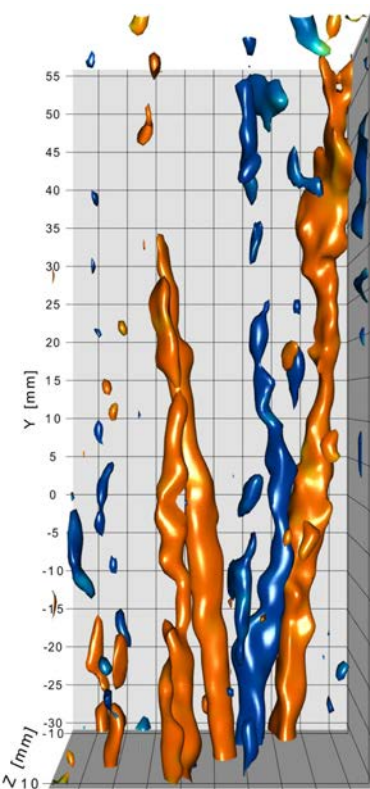

47299

406

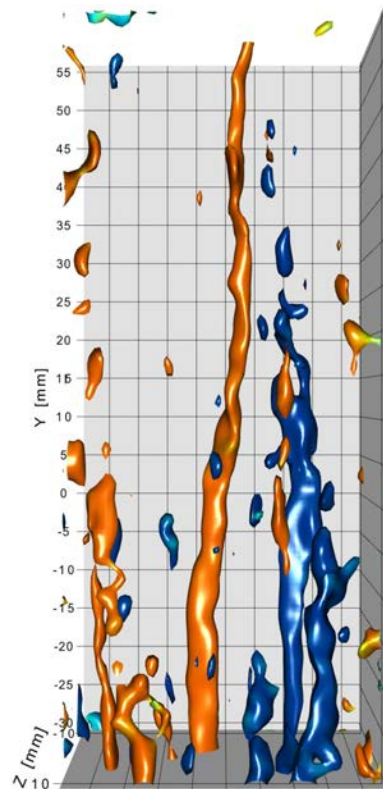

47982

407

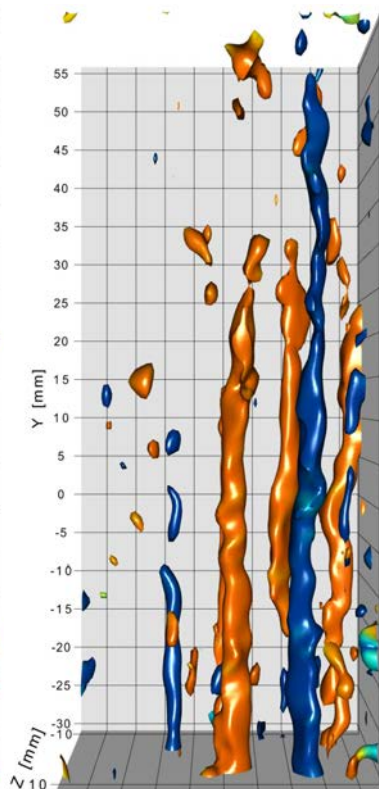

48852

408

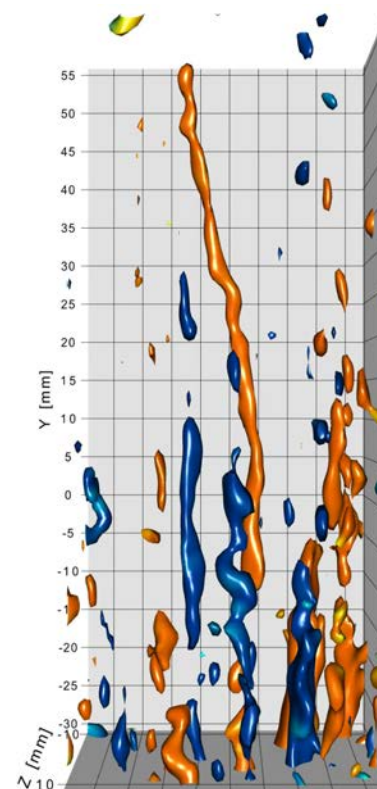

49136

409

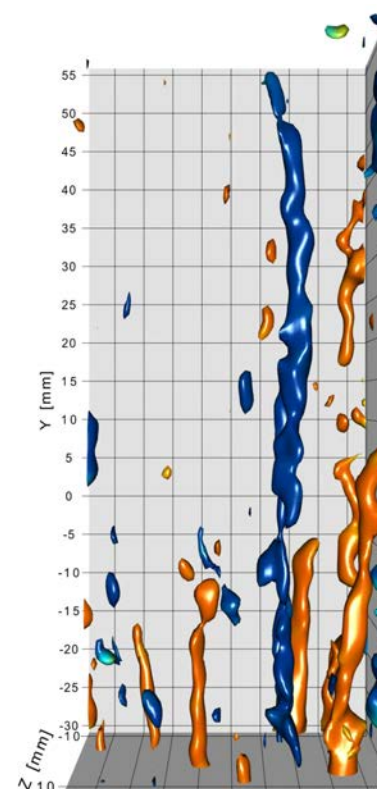

49343

410

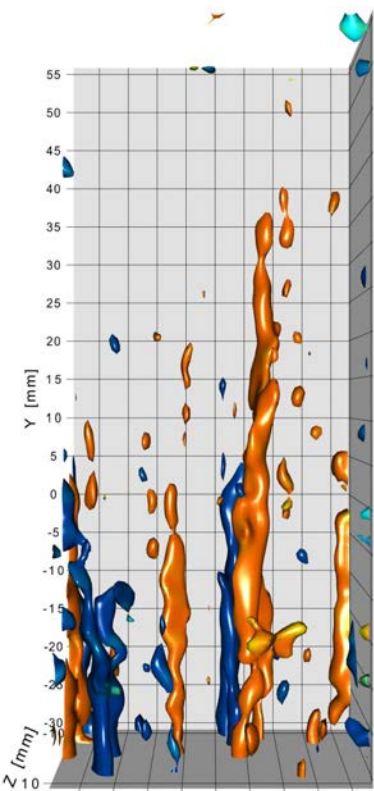

49919

411

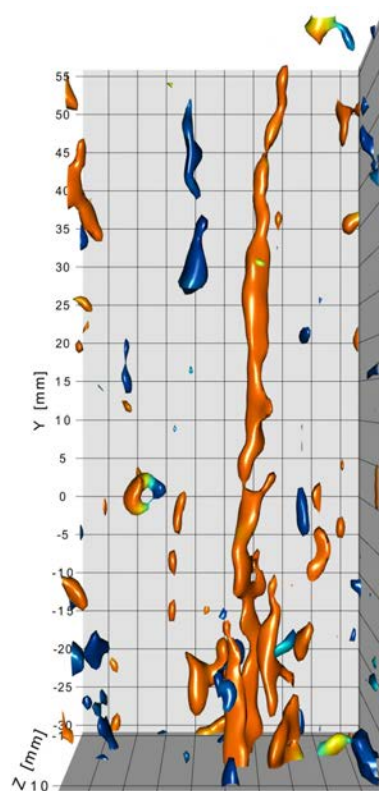

50636

412

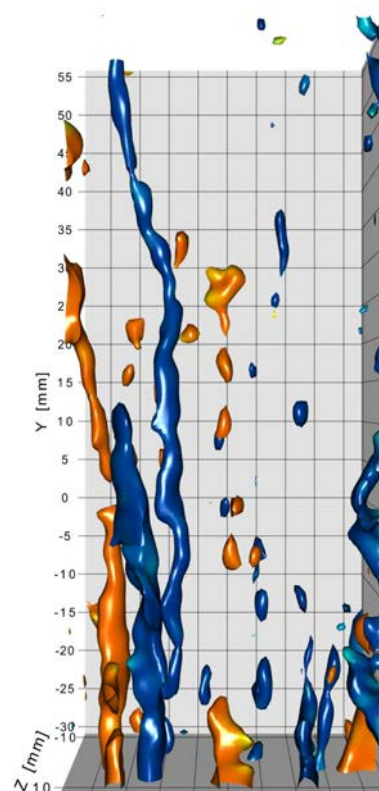

51255

413

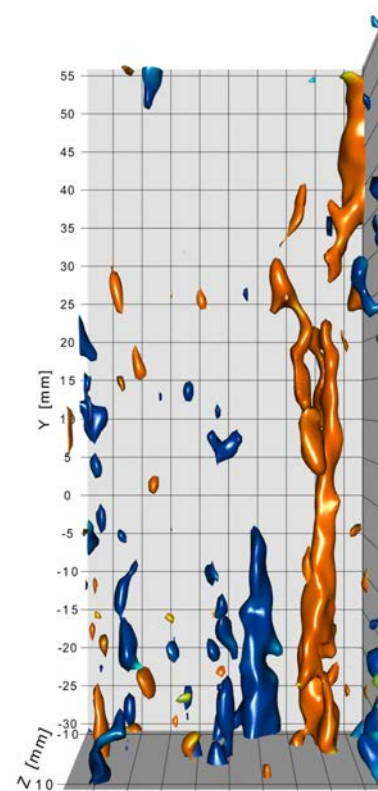

51663

414

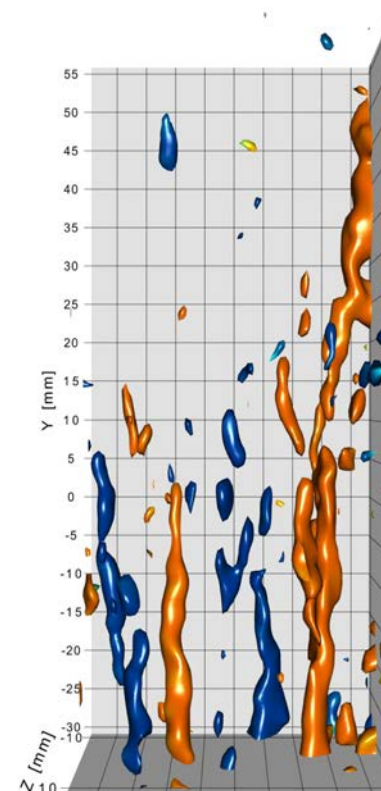

51703

415



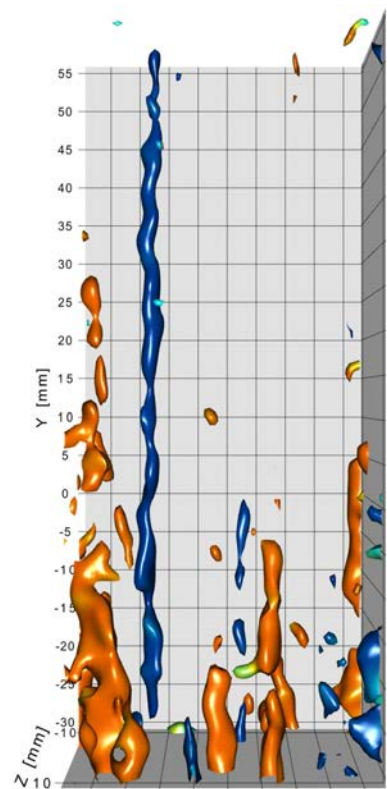

53372

416

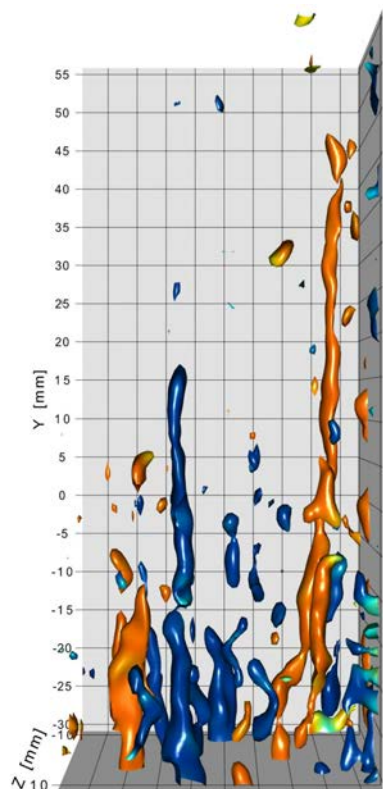

53900

417

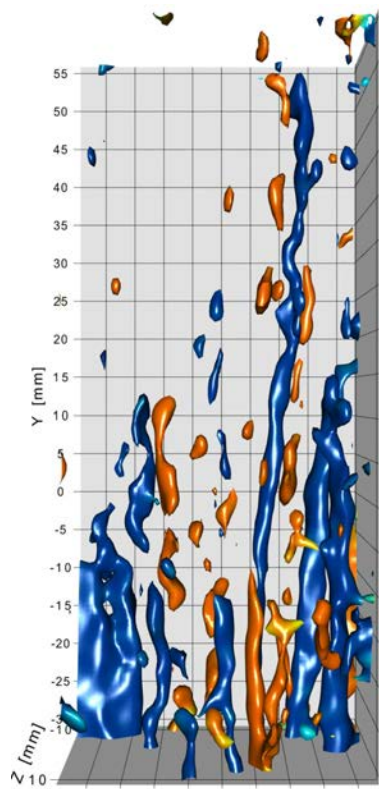

54443

418

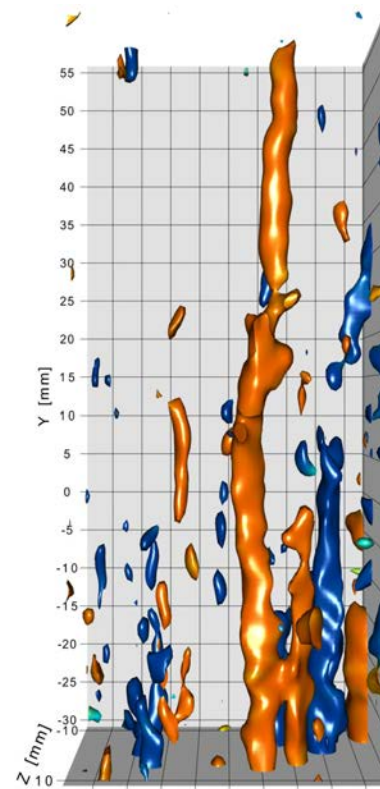

54687

419

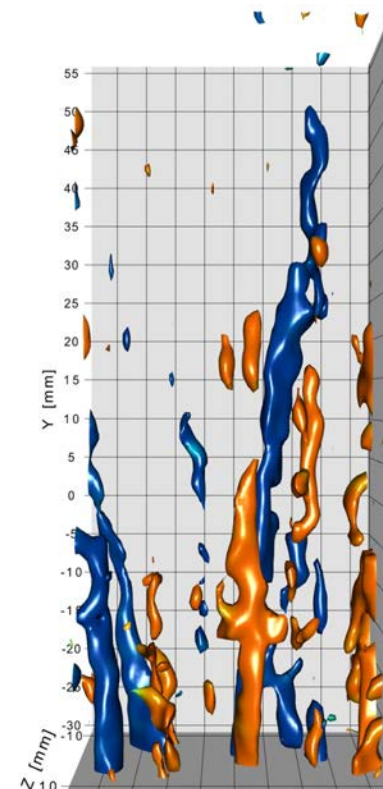

54952

420



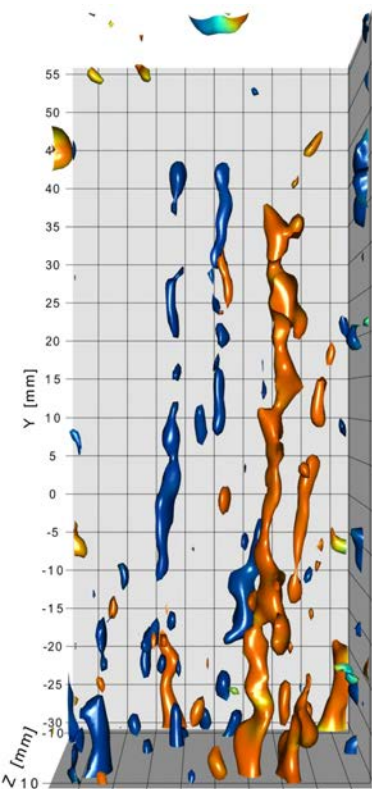

55556

421

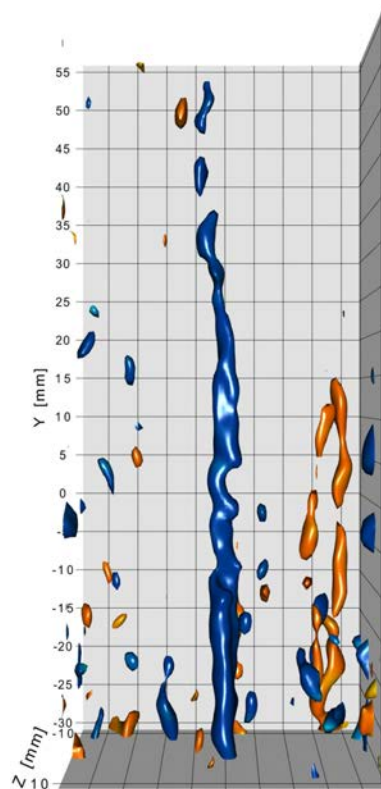

56103

422

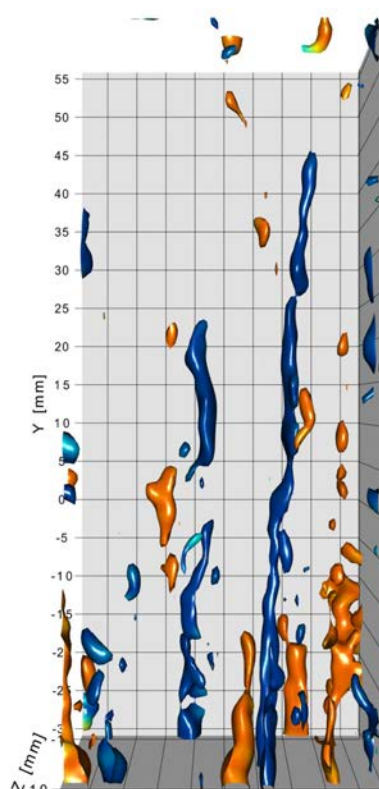

57256

423

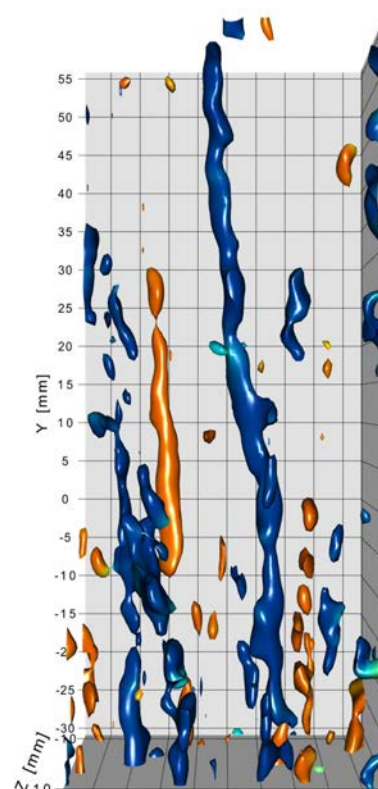

57831

424

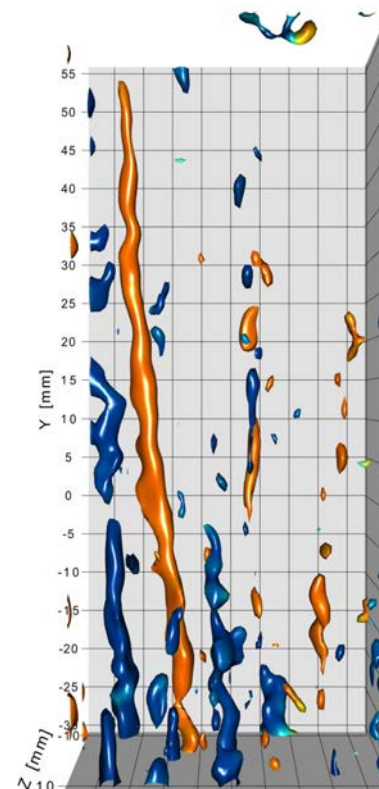

58078

425

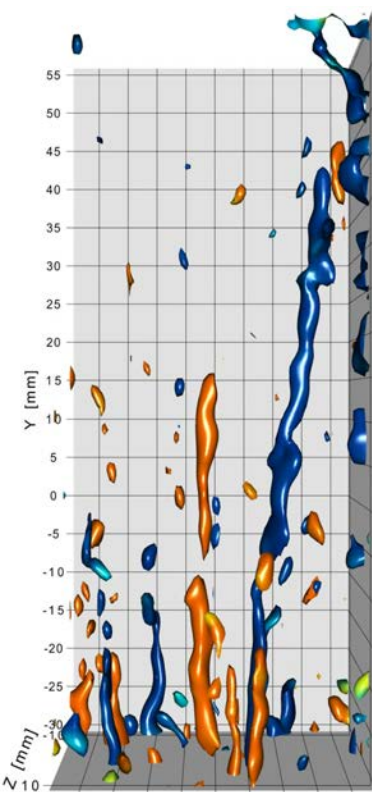

59009

426

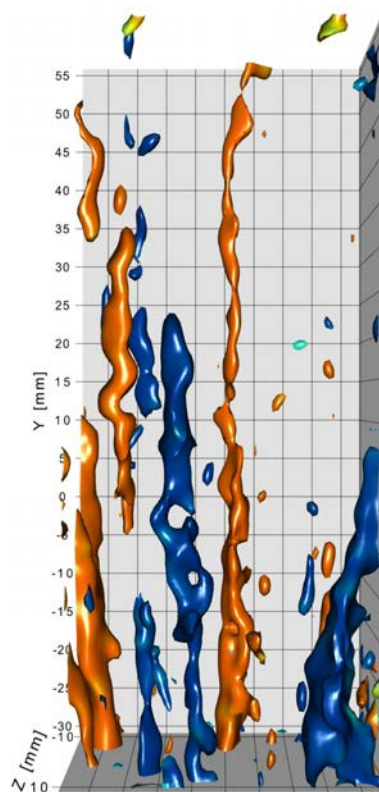

59249

427

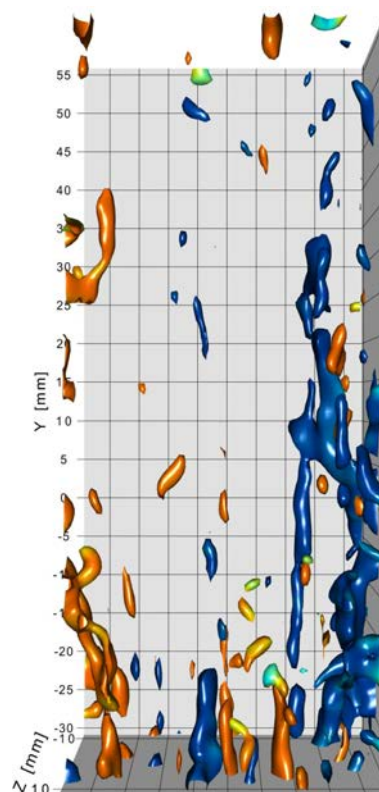

59916

428

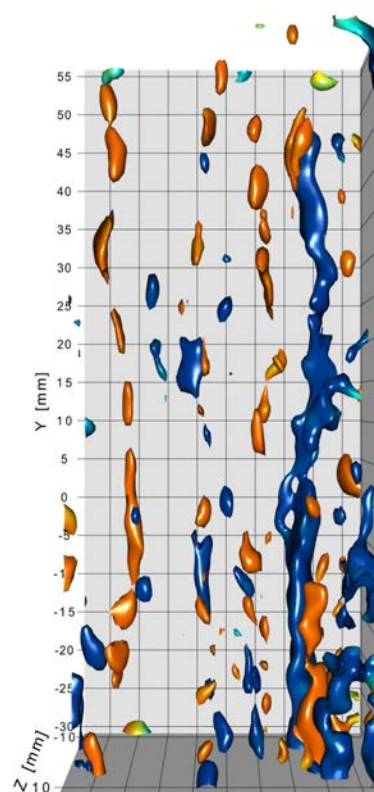

60018

429

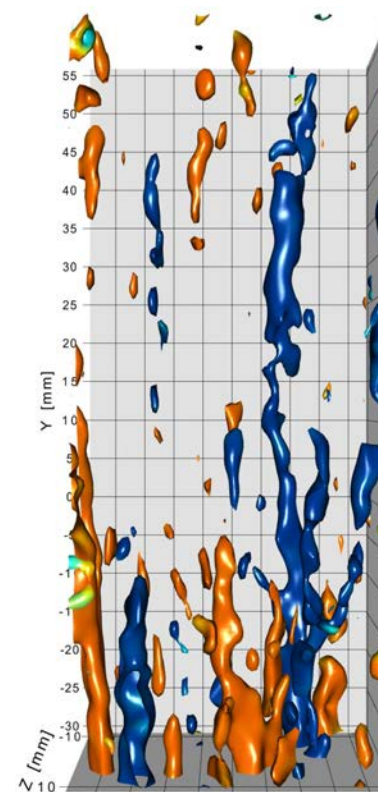

60210

430



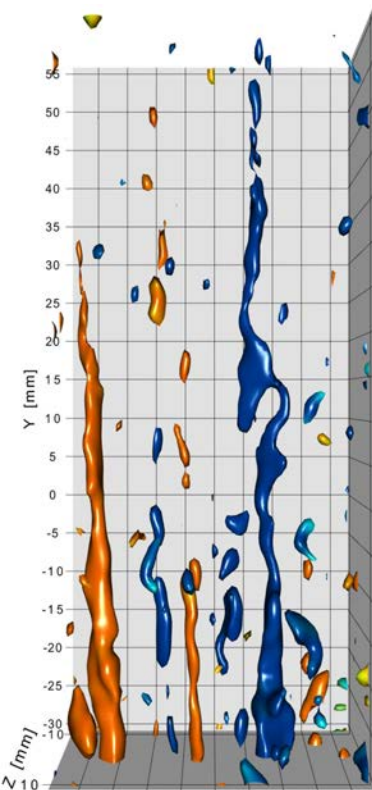

60595

431

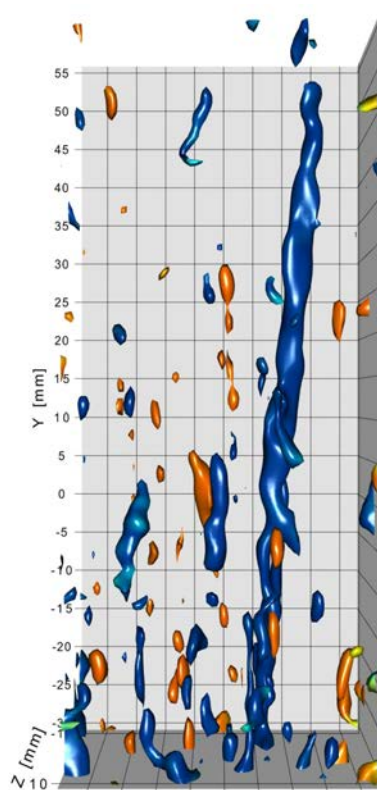

60807

432

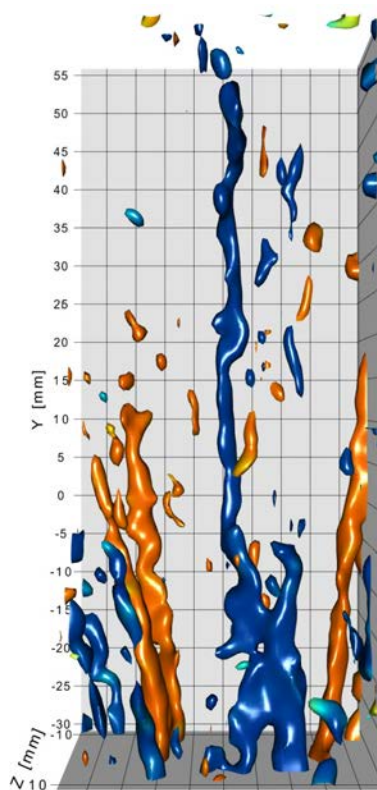

61009

433

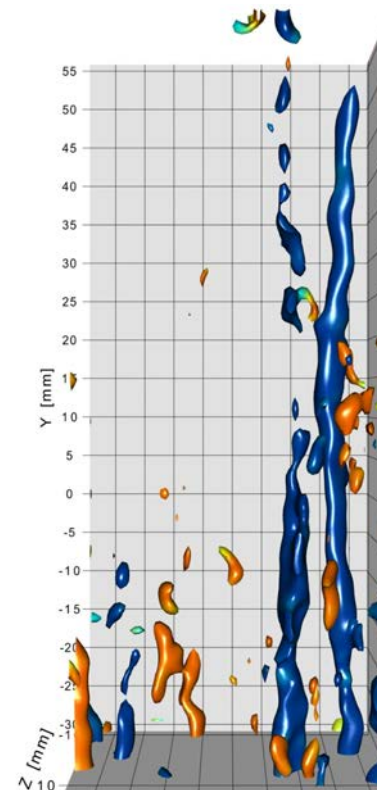

62767

434

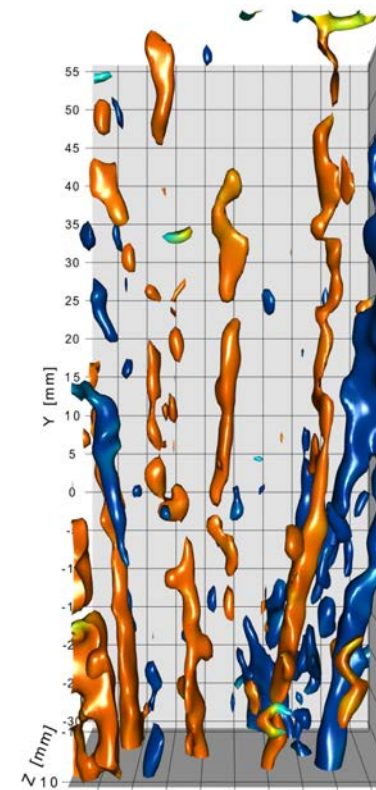

63631

435



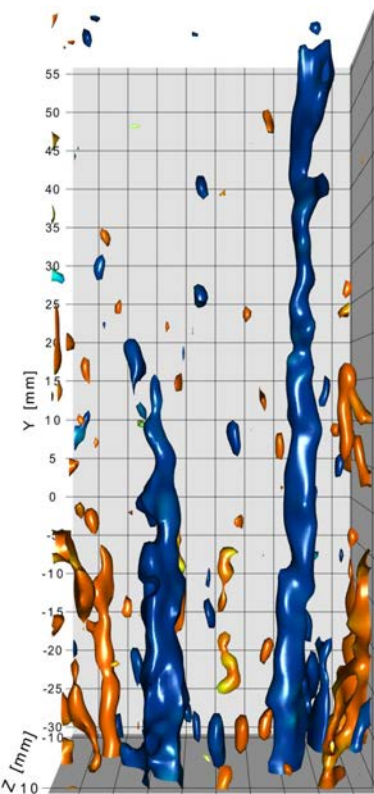

63950

436

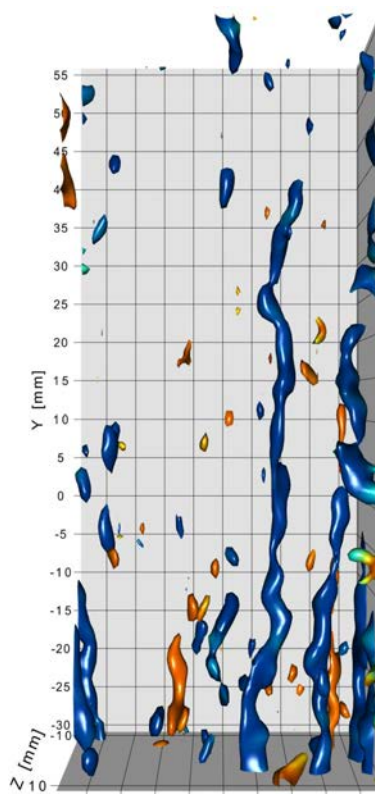

65907

437

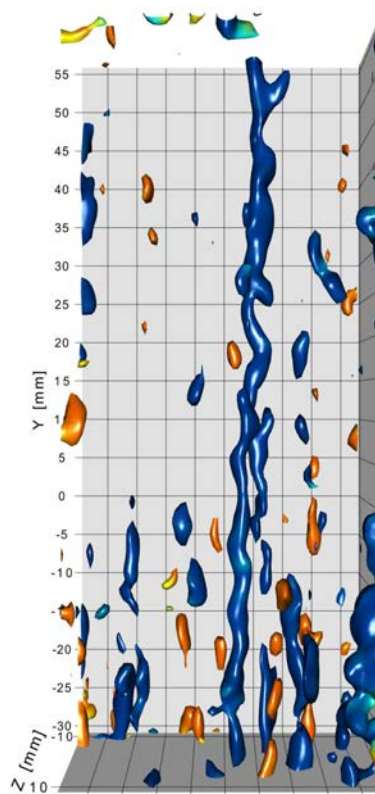

66104

438

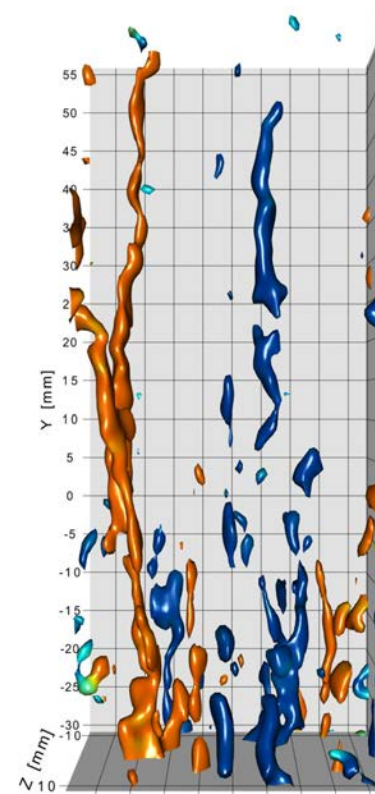

66483

439

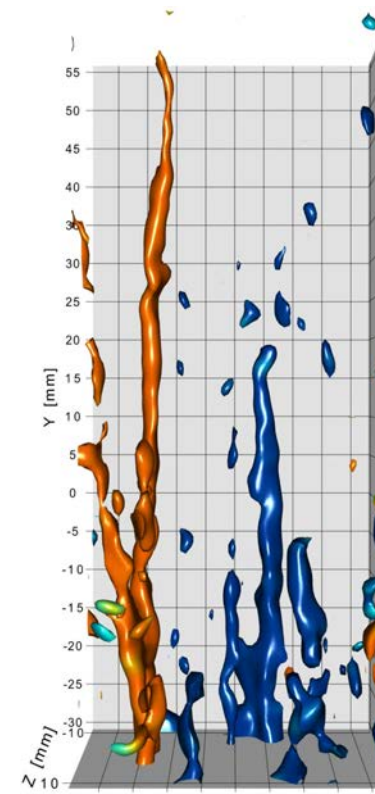

66578

440

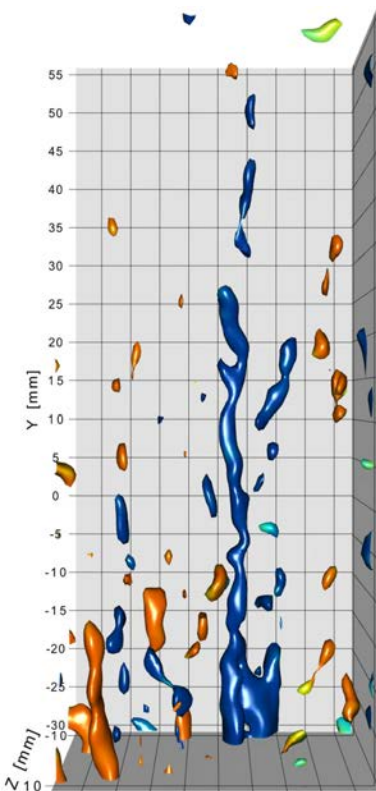

67063

441

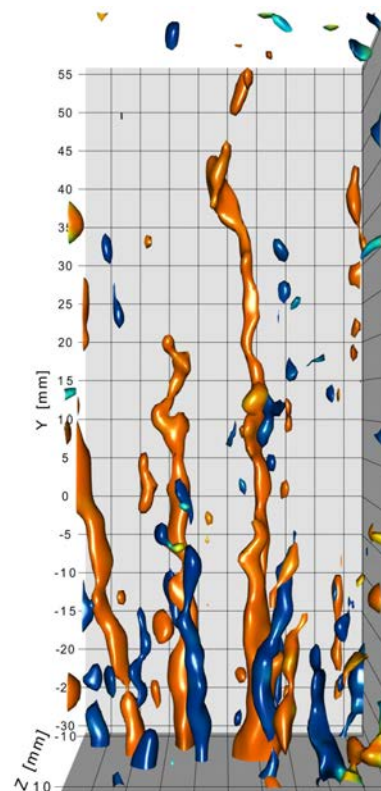

67696

442

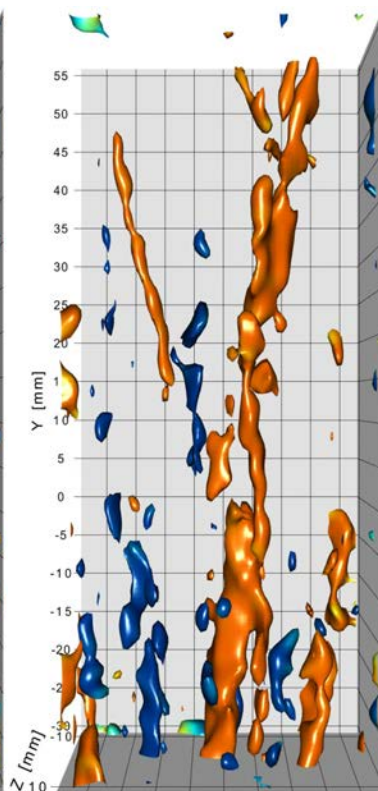

67895

443

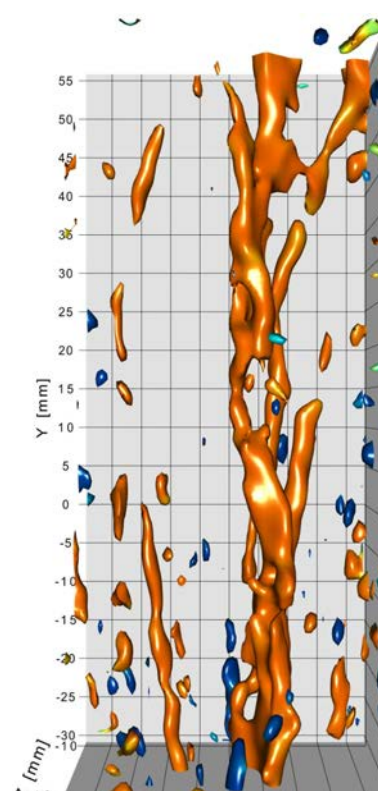

68041

444

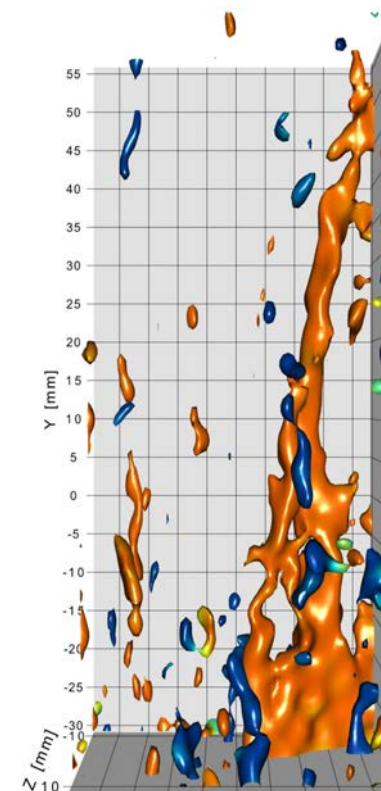

68320

445



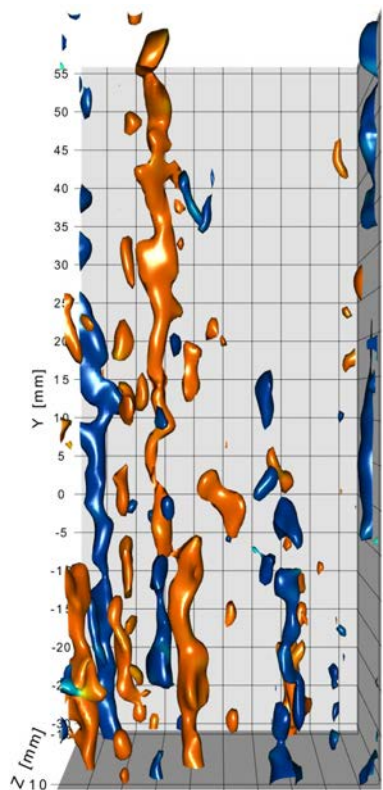

69918

446

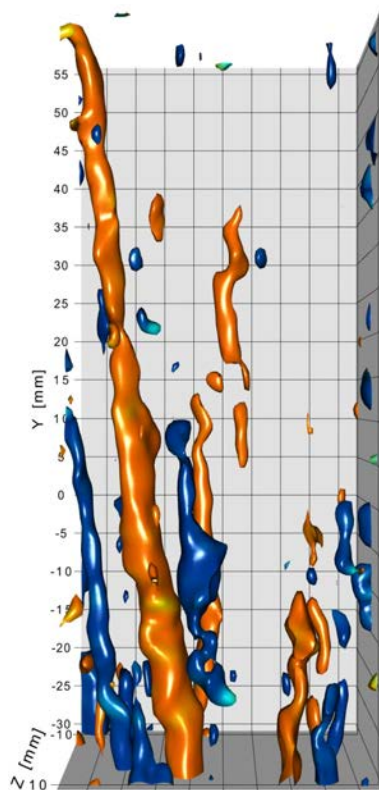

70211

447

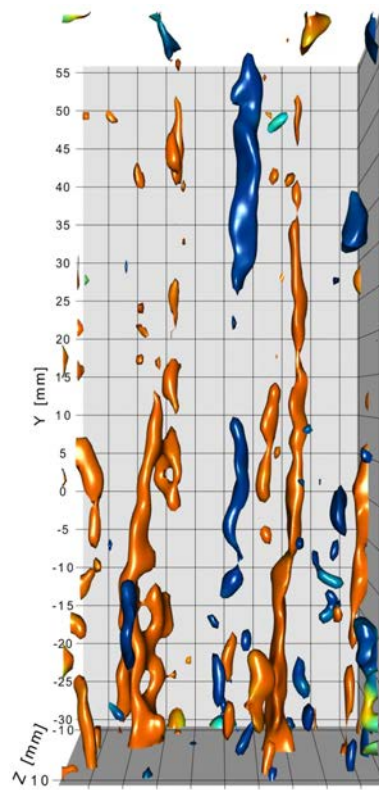

71284

448

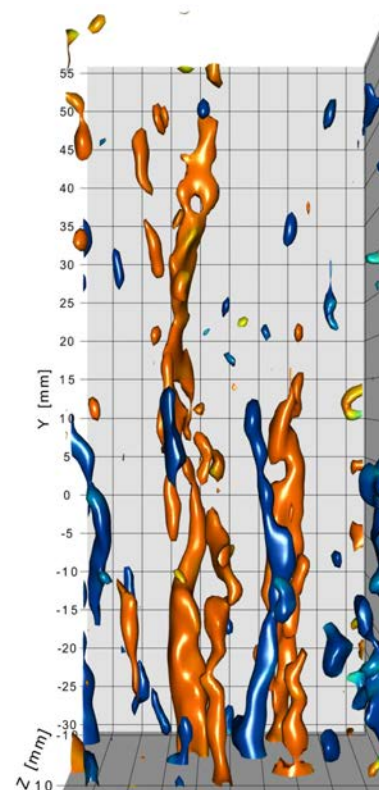

71575

449

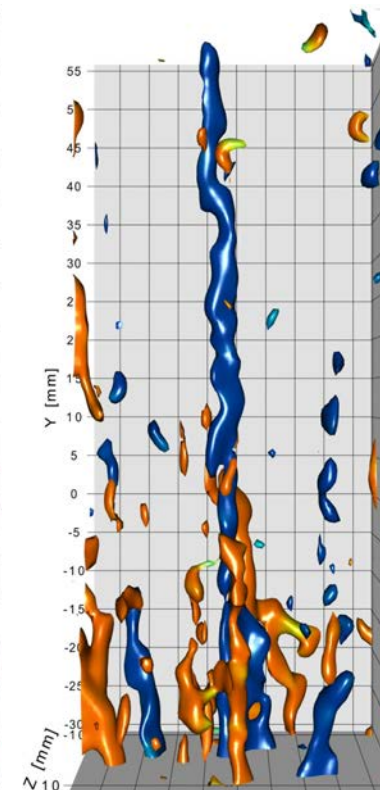

71790

450



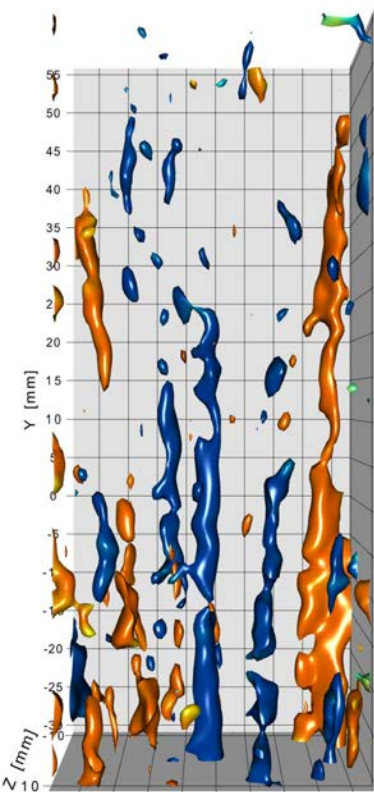

72023

451

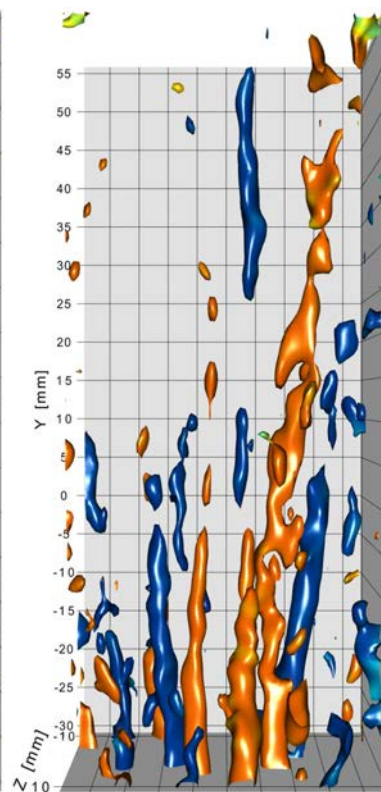

72567

452

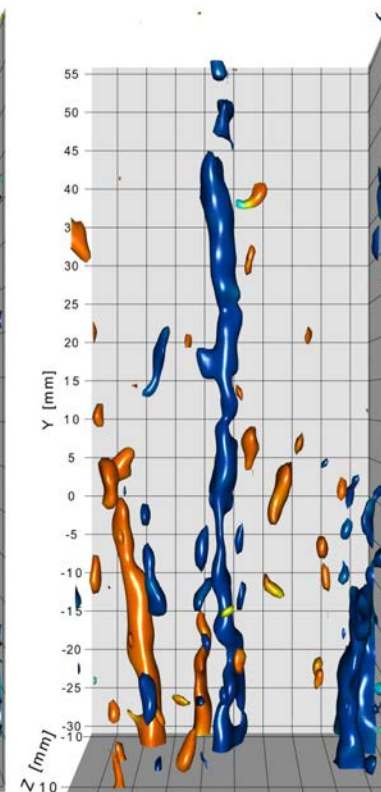

72992

453

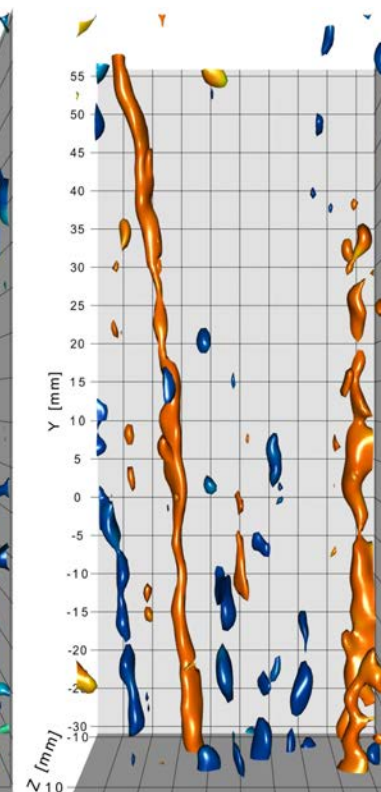

75038

454

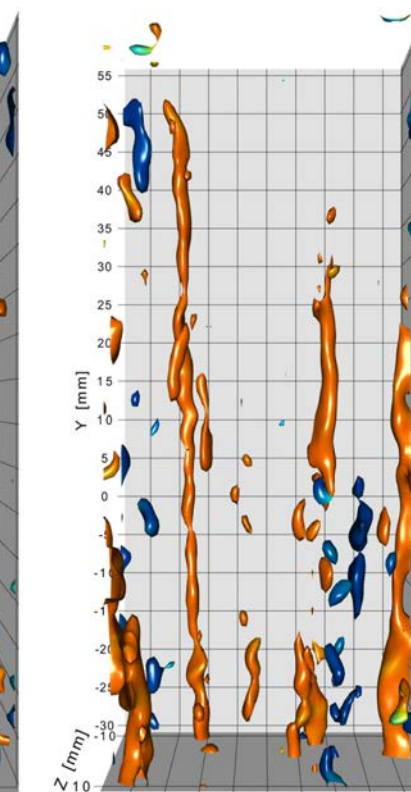

76200

455

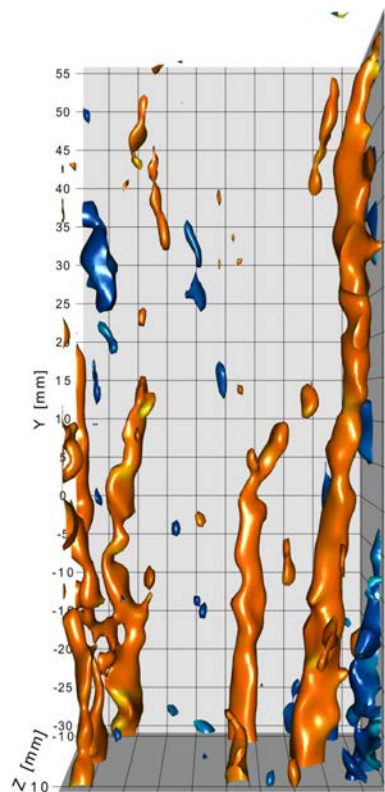

77040

456

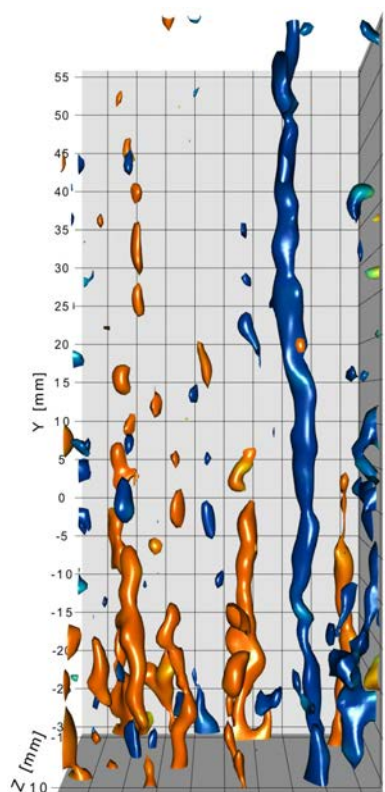

79517

457

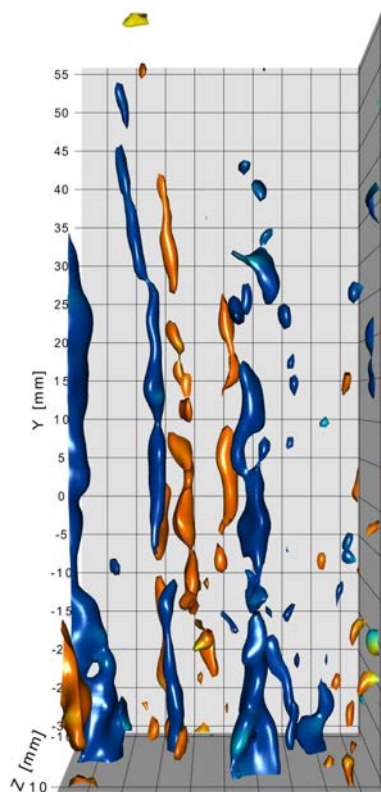

79749

458

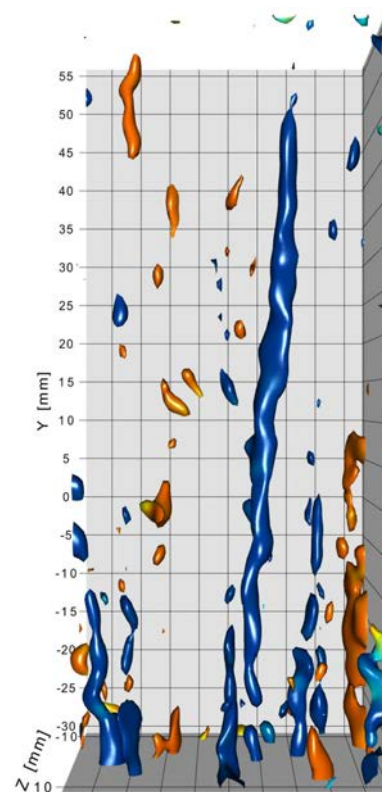

80602

459

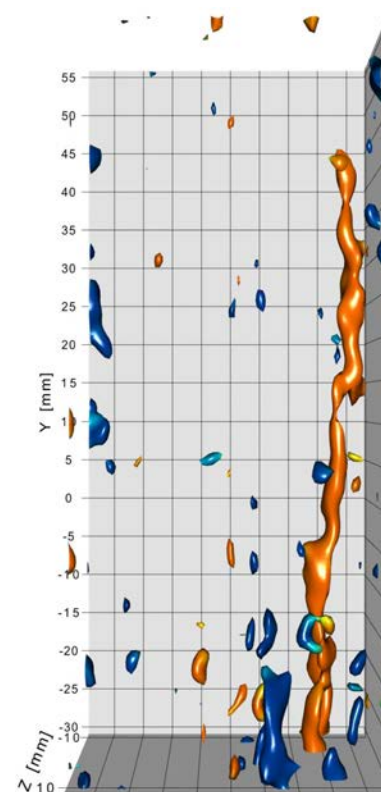

84022

460



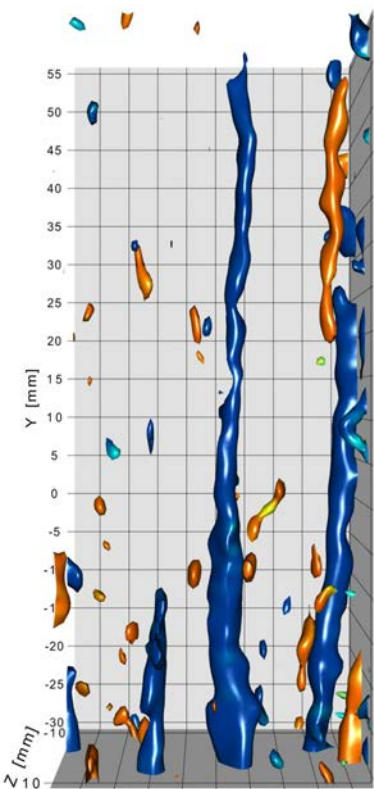

85670

461

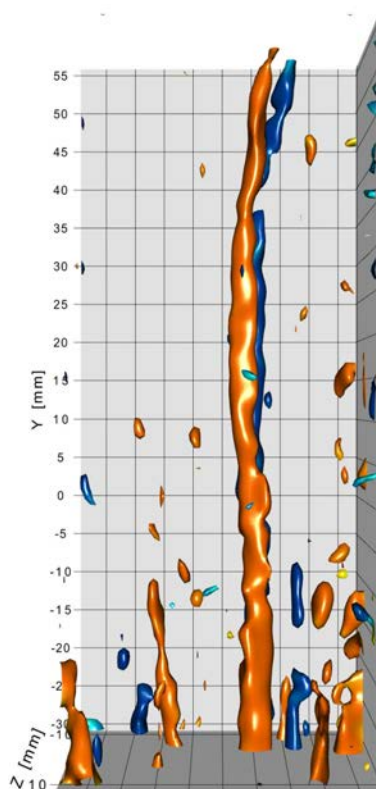

86512

462

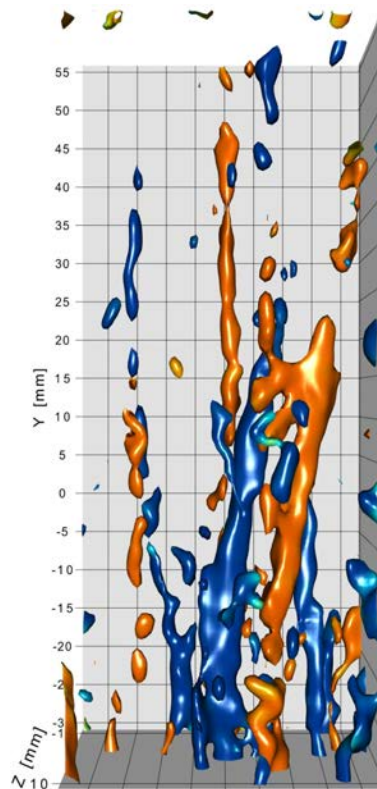

87296

463

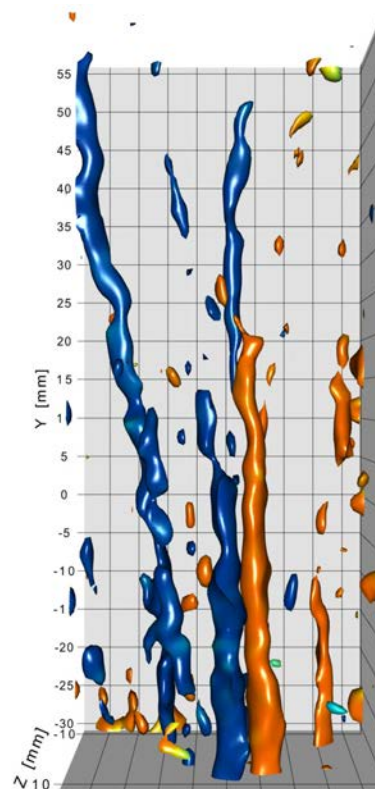

88493

464

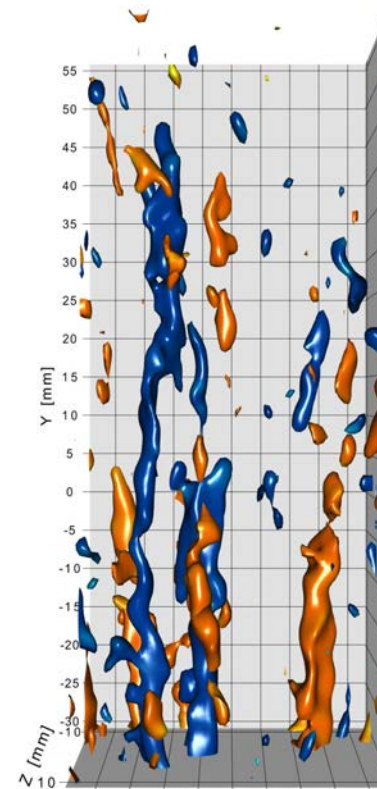

88769

465



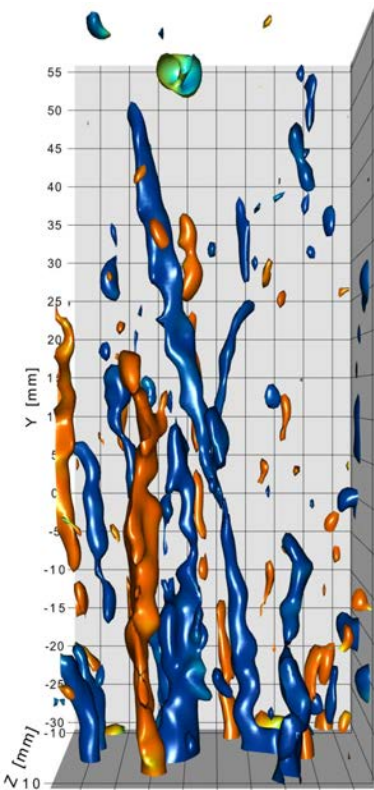

88953

466

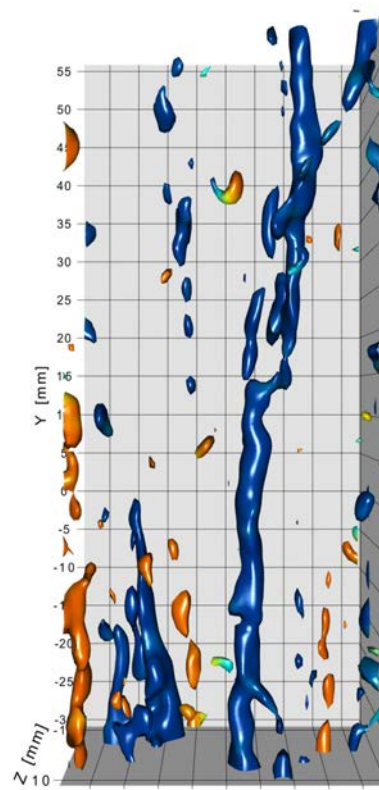

89605

467

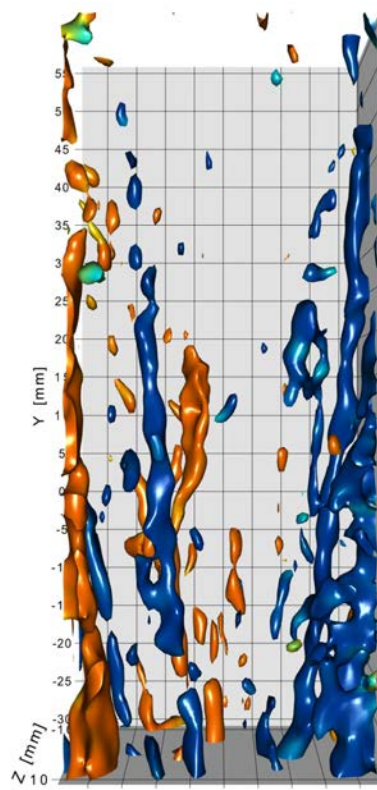

92712

468

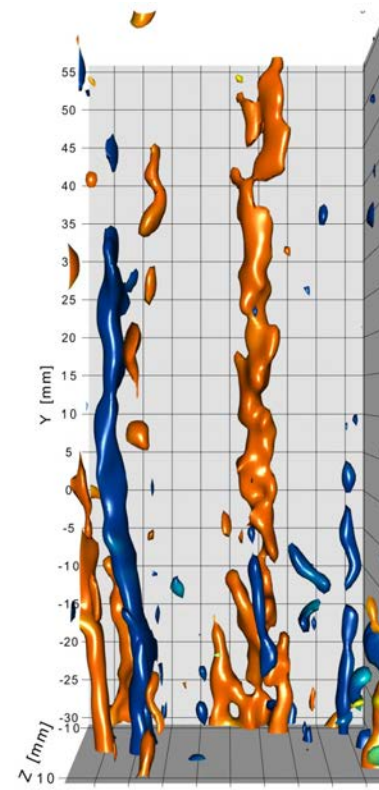

93579

469

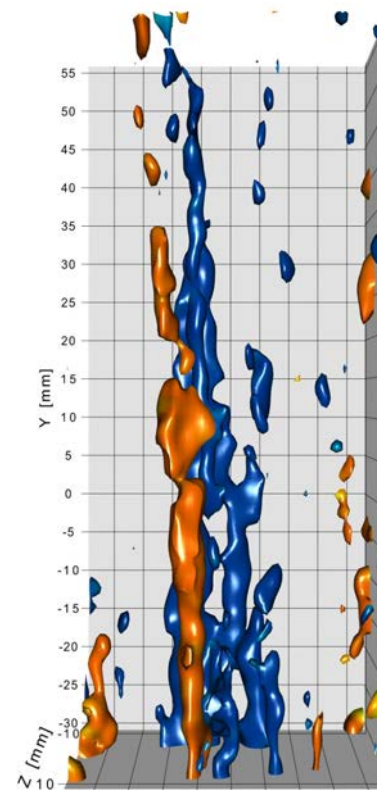

94972

470

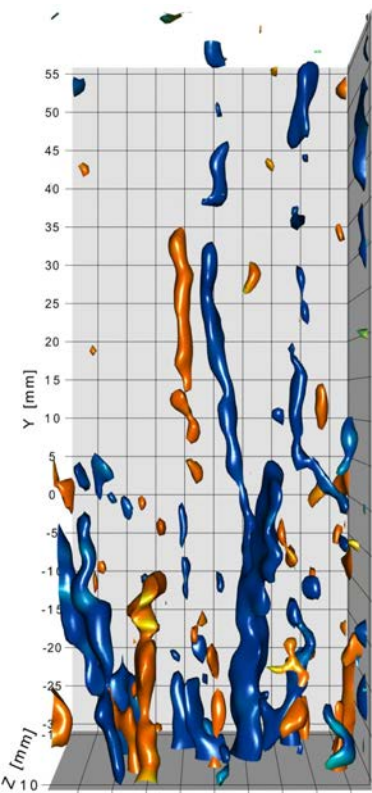

95324

471

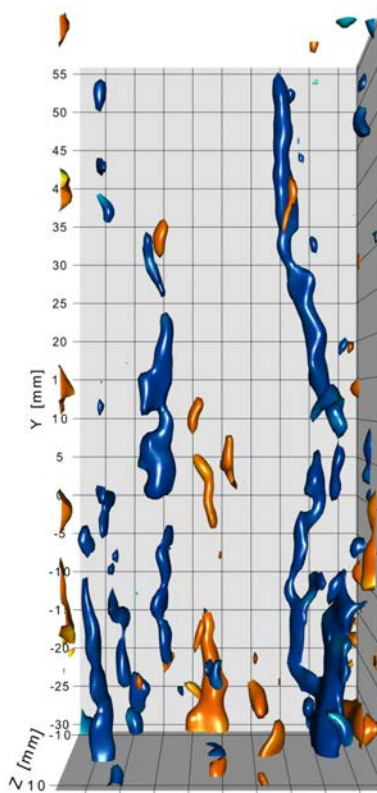

98055

472

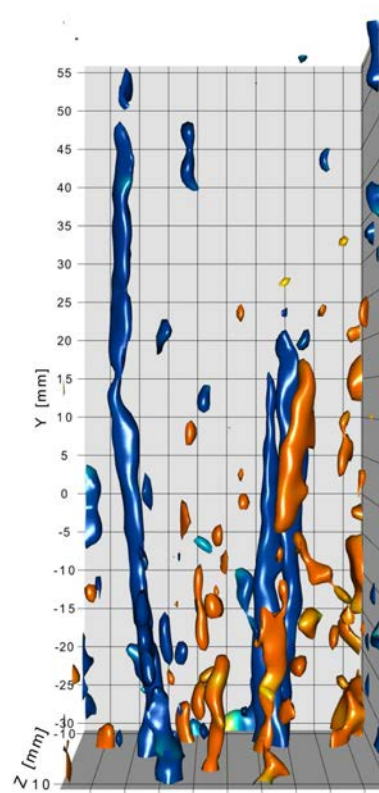

98219

473

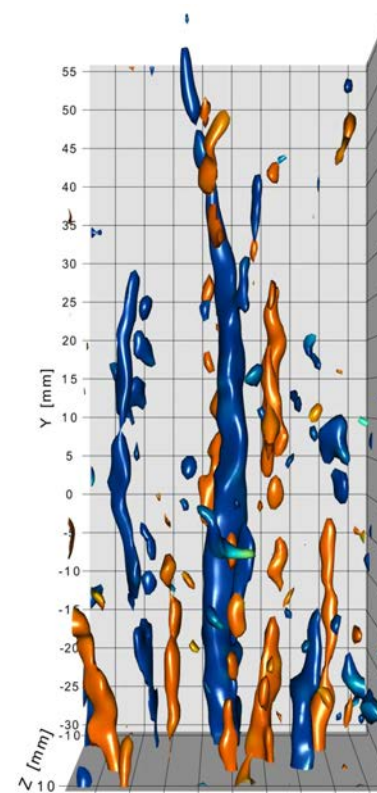

99192

474

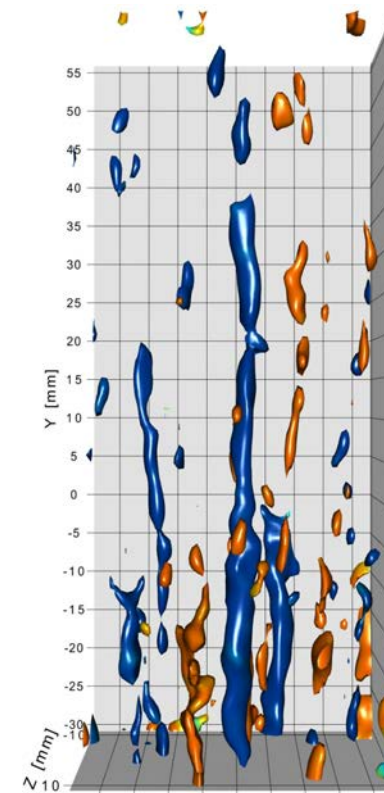

99578

475



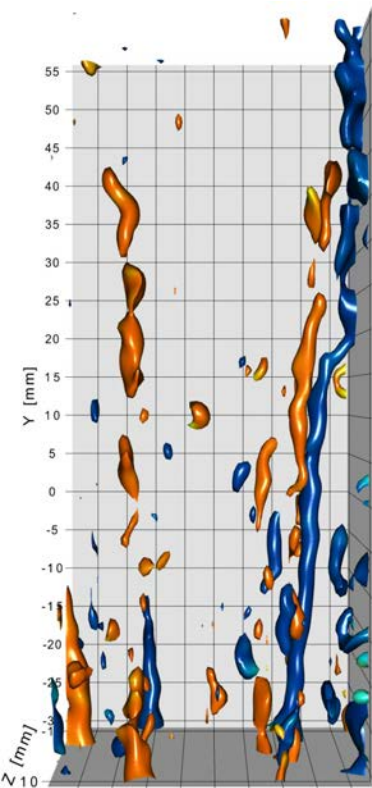

100186

476

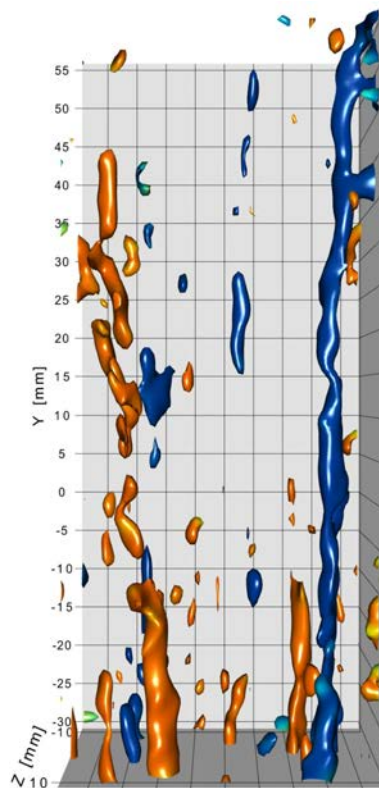

100329

477

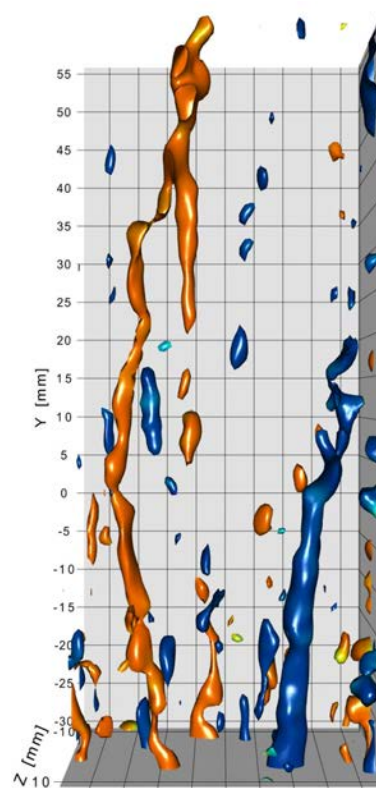

101023

478

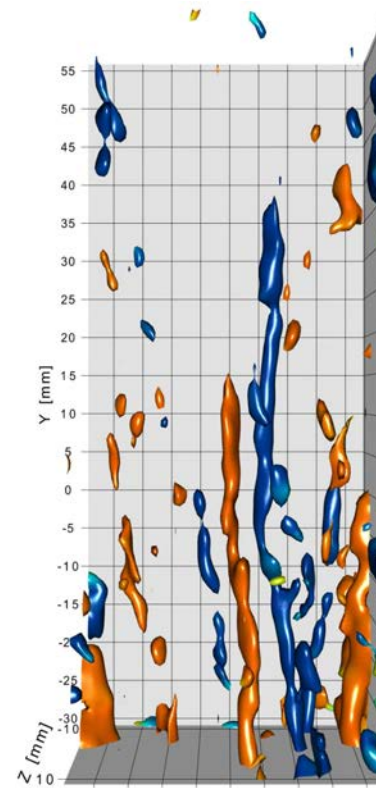

101702

479

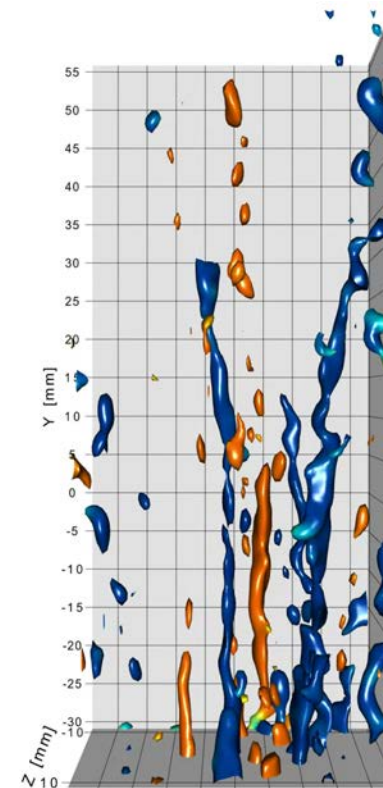

103460

480



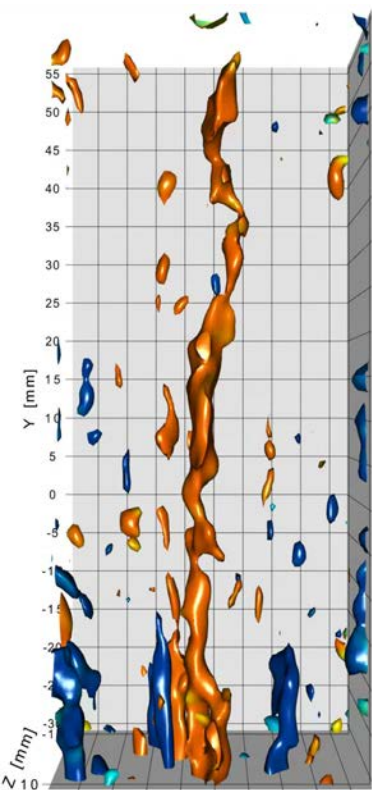

103832

481

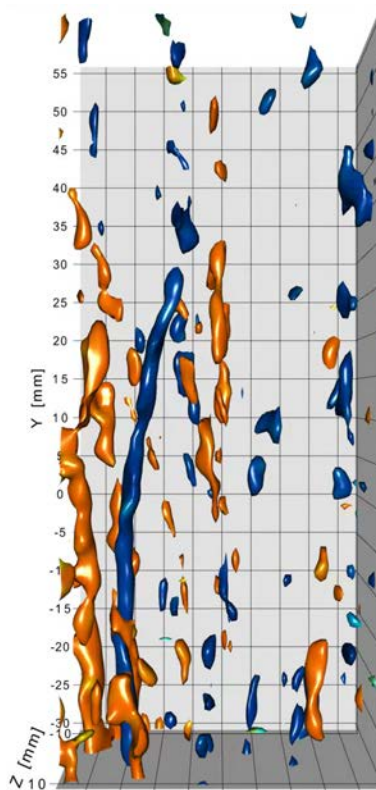

104954

482

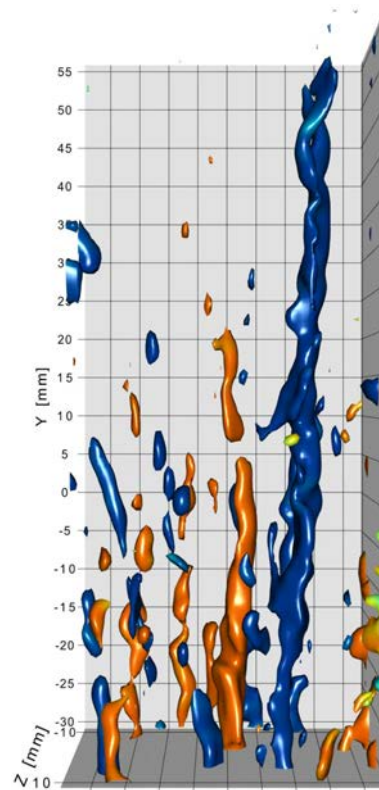

105192

483

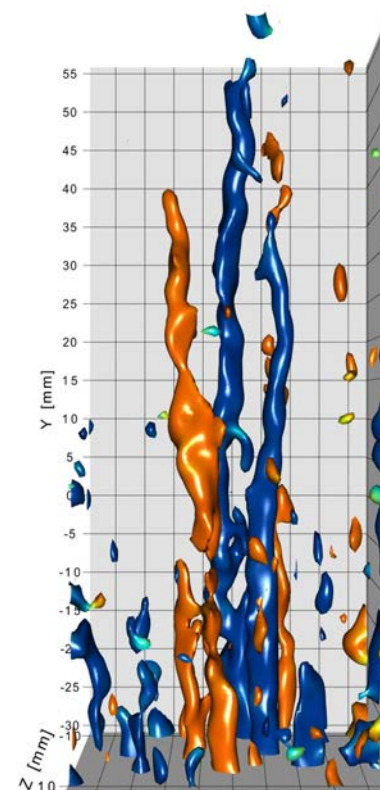

105496

484

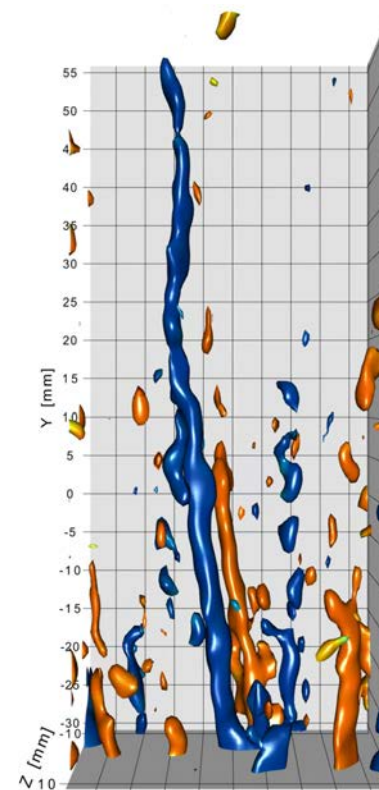

105852

485

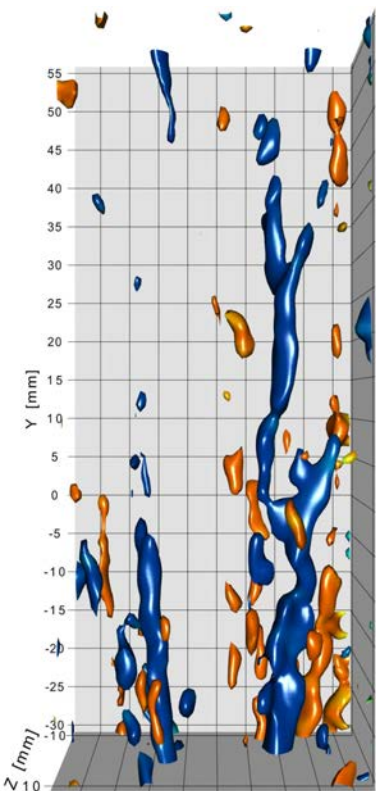

108446

486

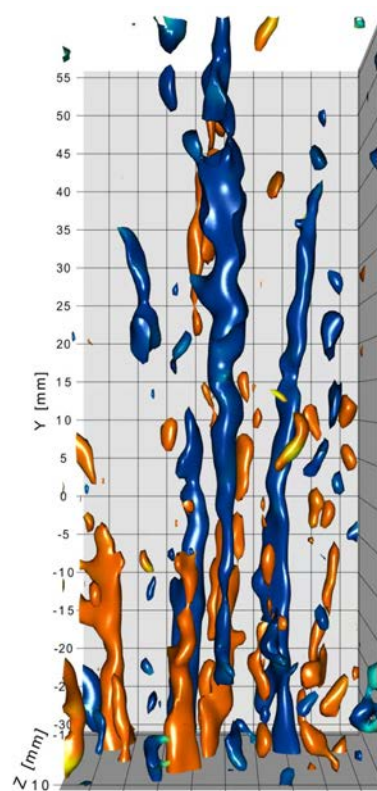

108702

487

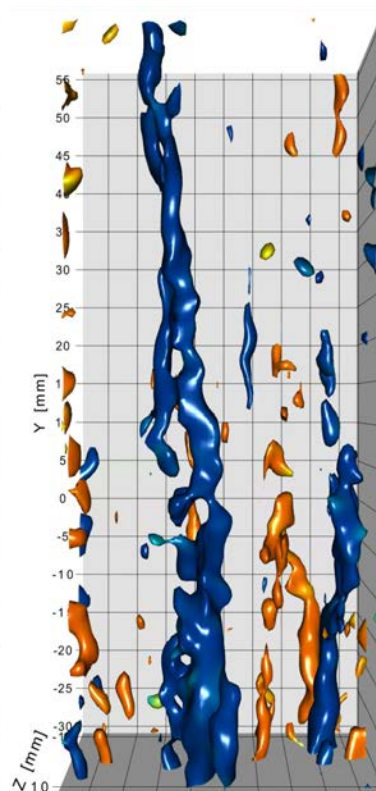

109095

488

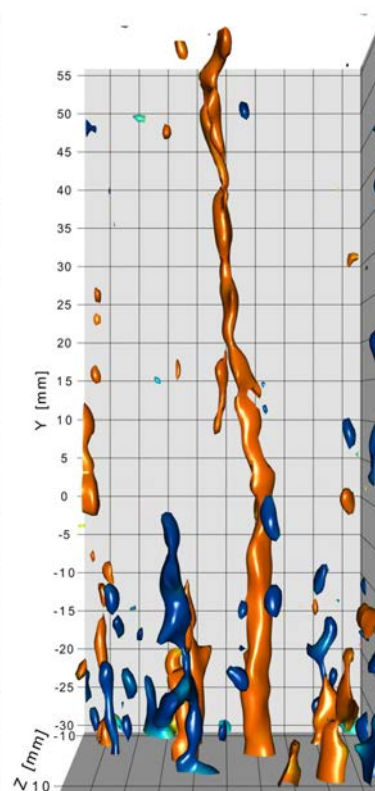

109521

489

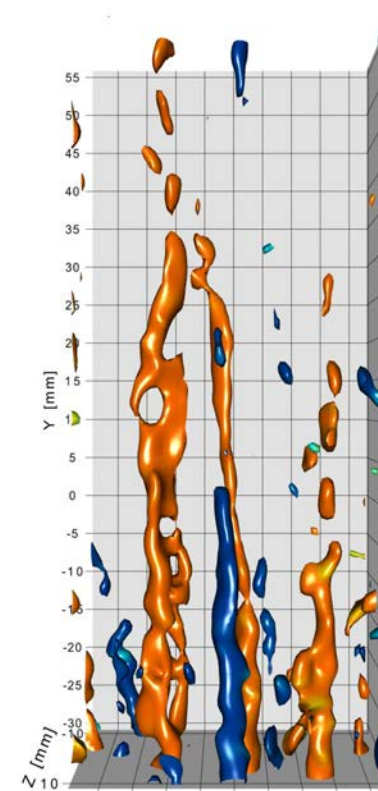

109877

490



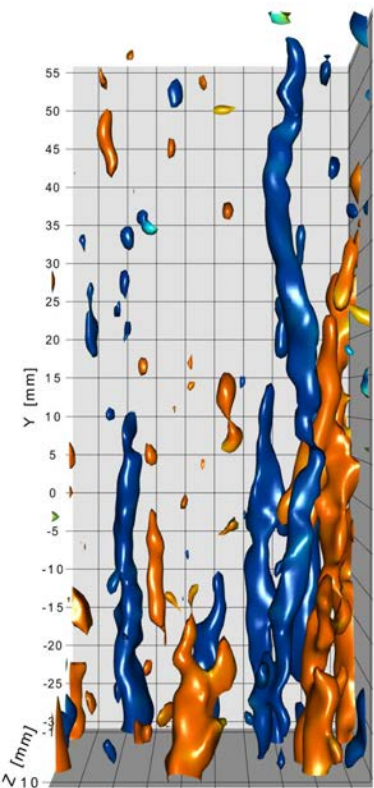

111425

491

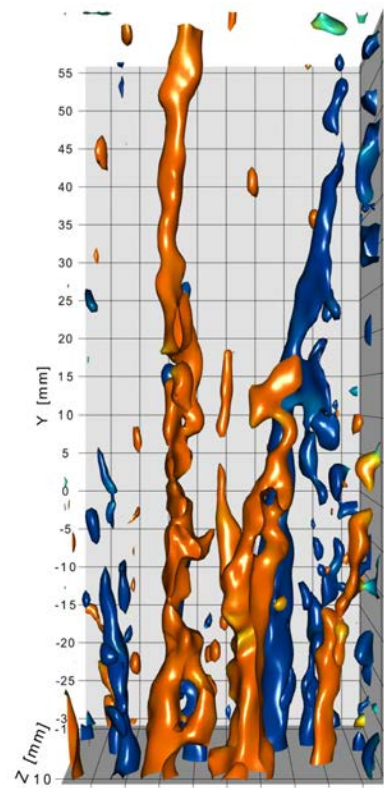

111670

492

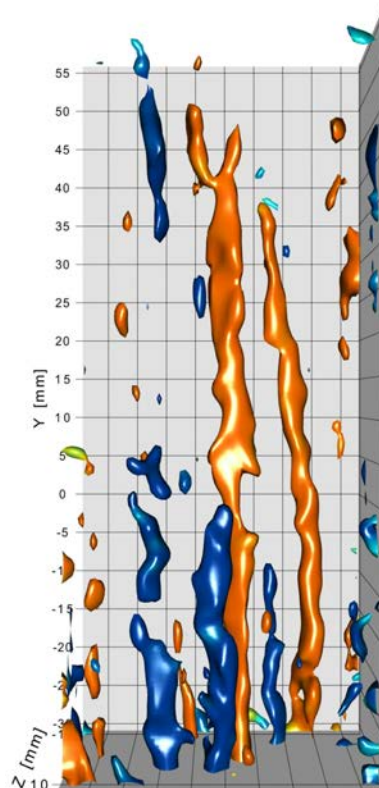

112346

493

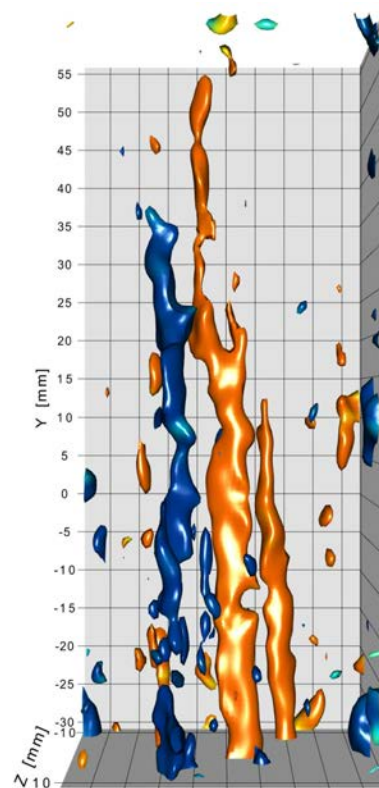

112434

494

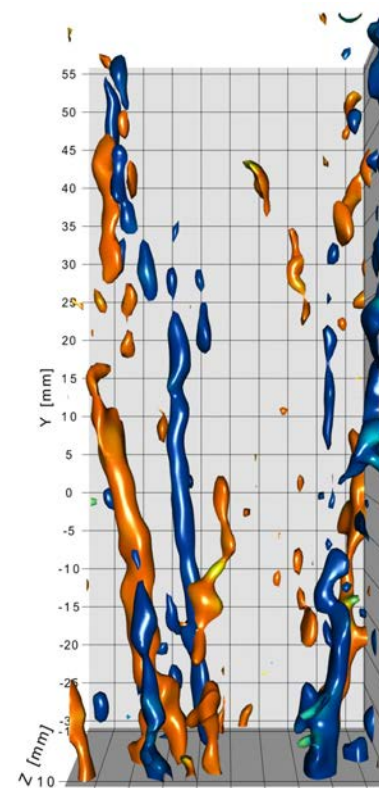

113106

495



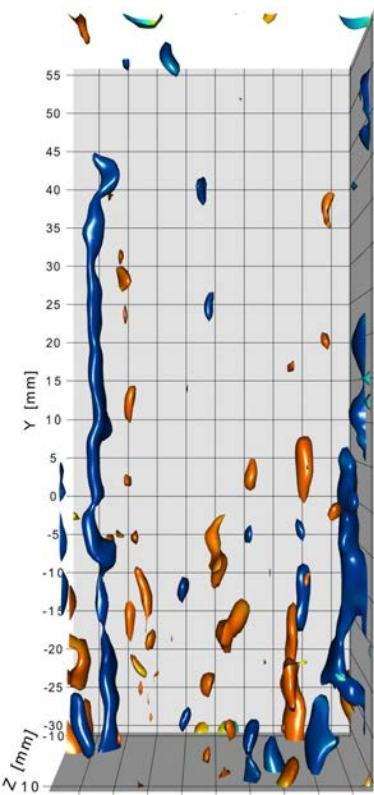

114155

496

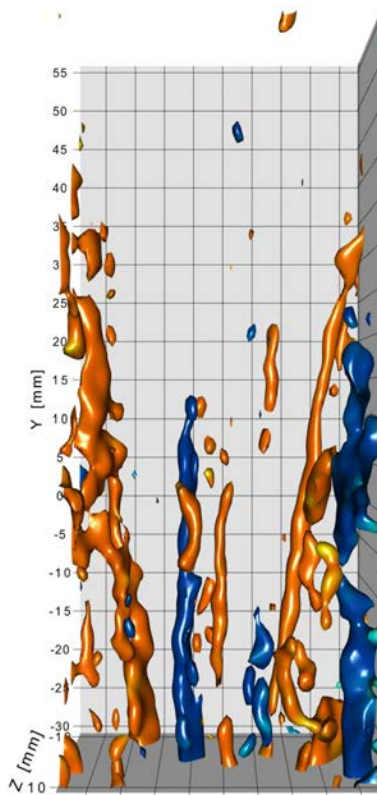

114634

497

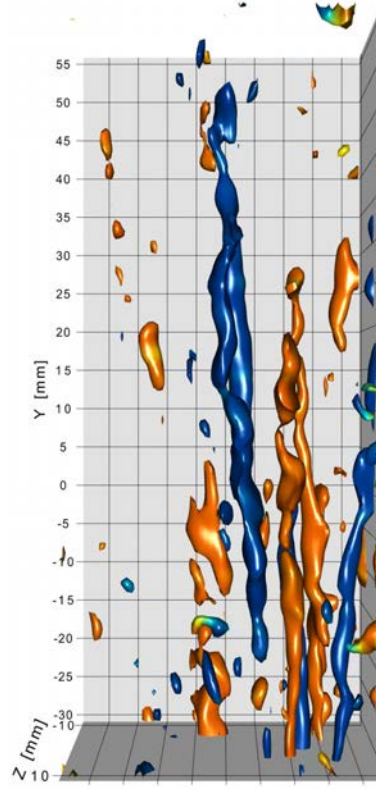

115177

498

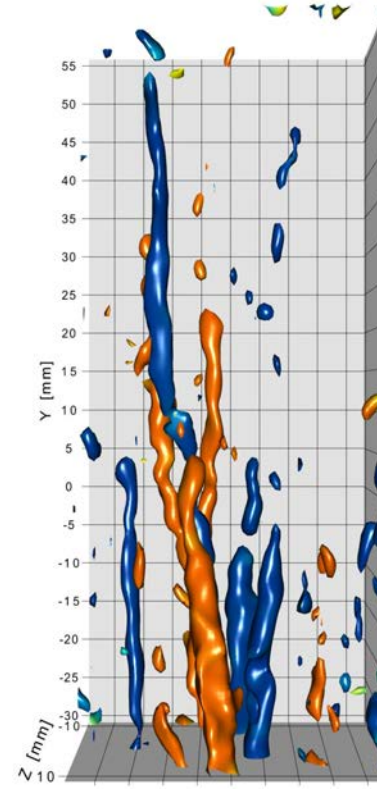

115551

499

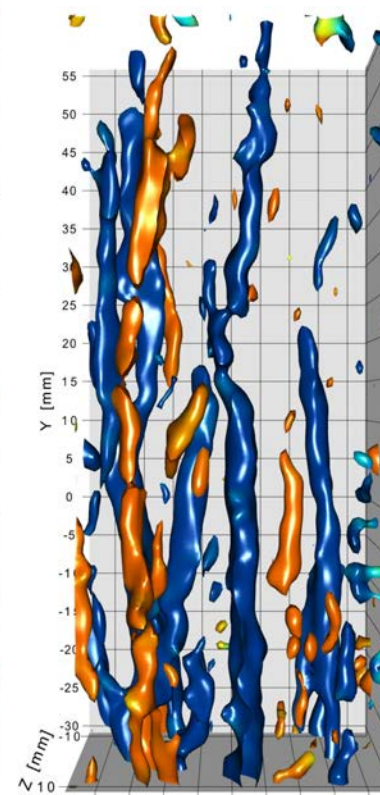

116600

500

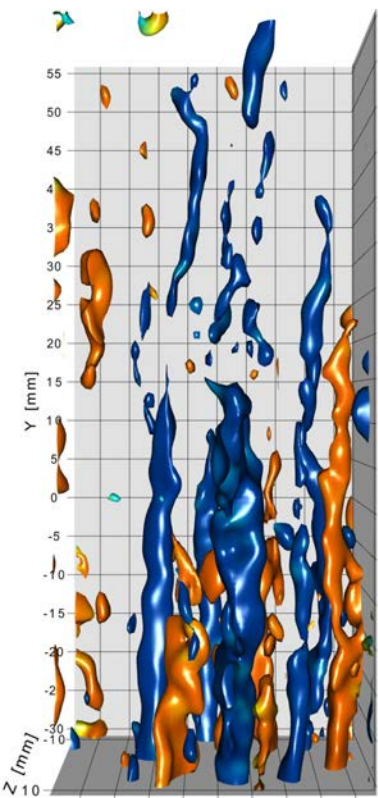

116804

501

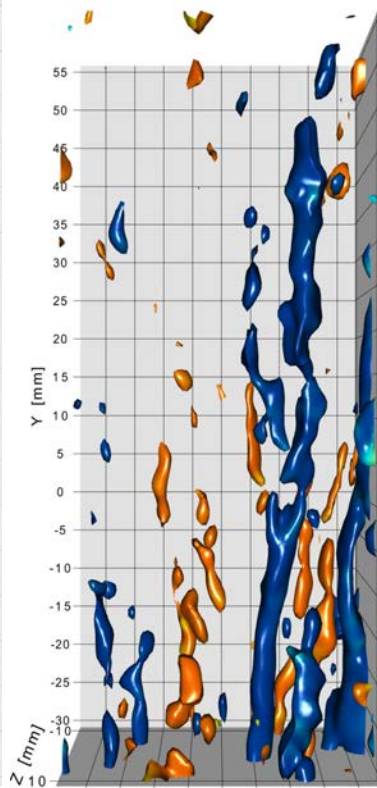

117941

502

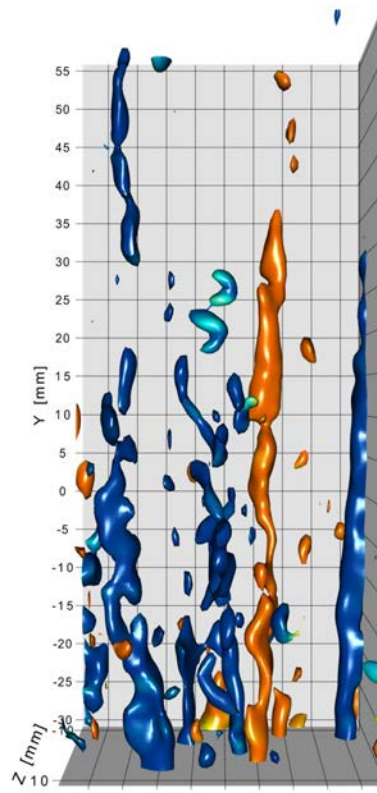

119081

503

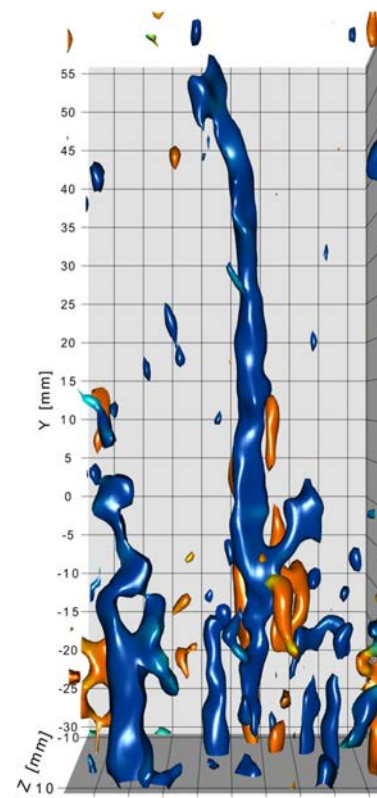

119692

504

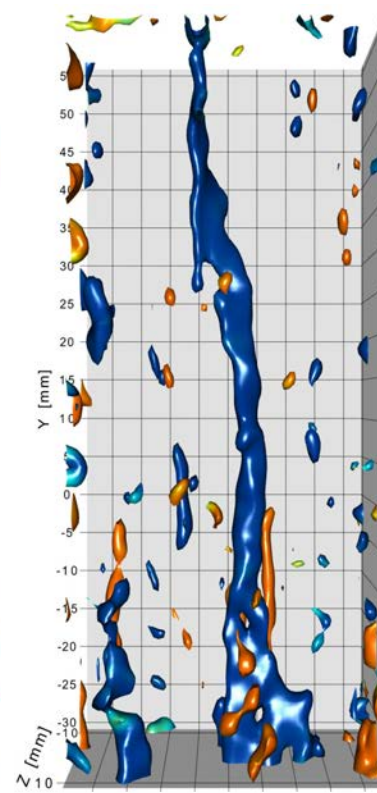

119743

505



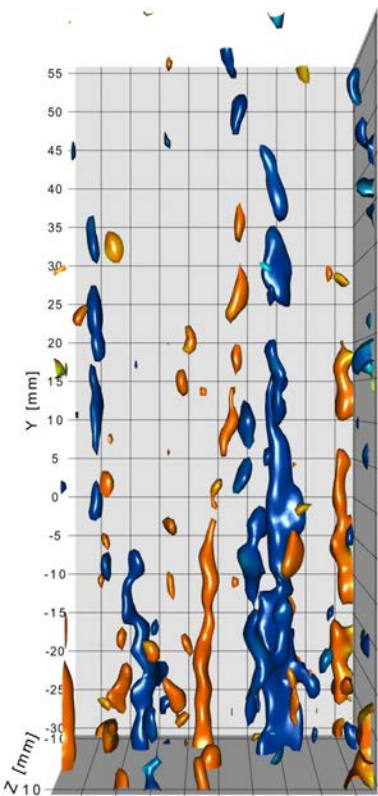

120489

506

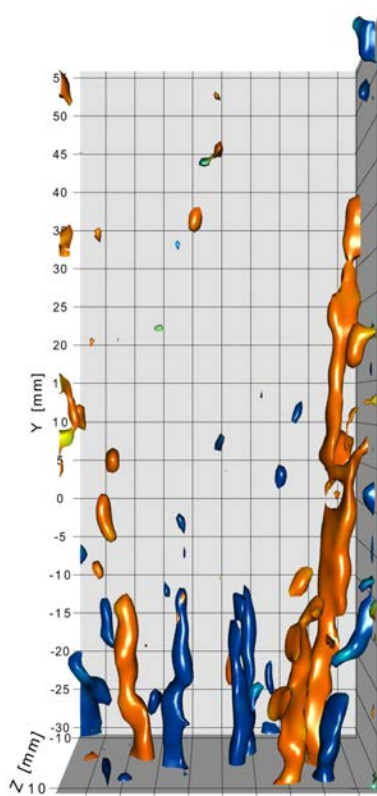

121118

507

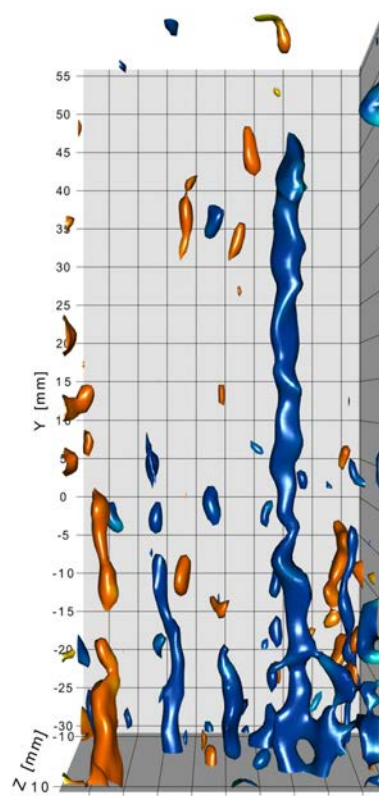

123439

508

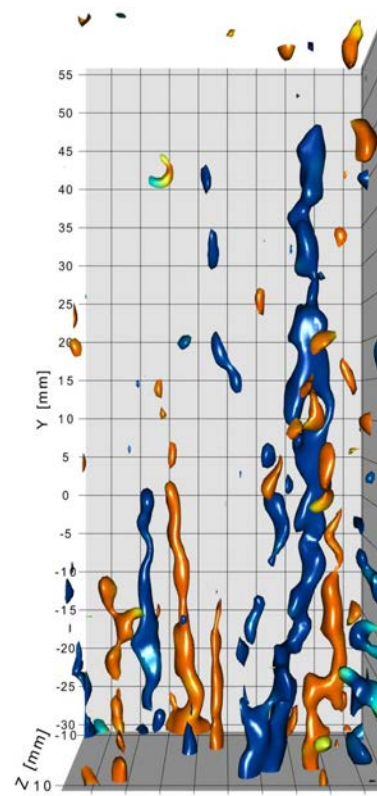

124056

509

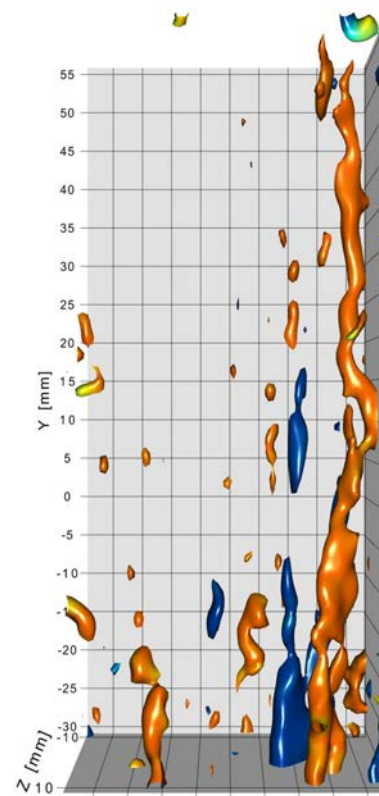

124248

510



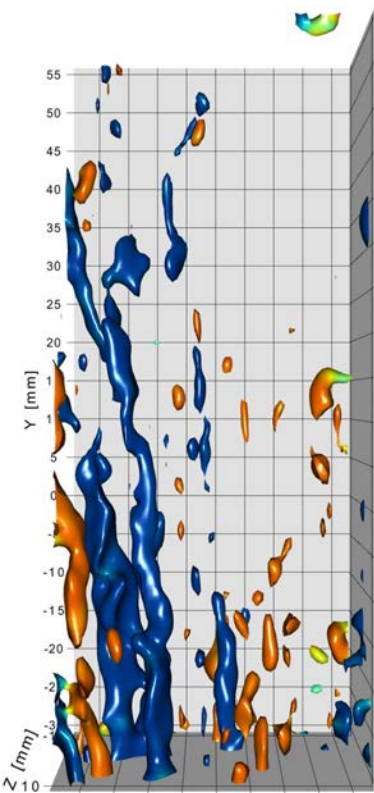

125176

511

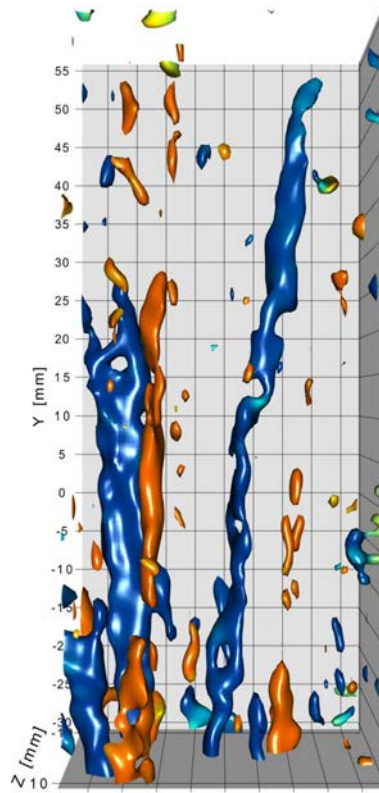

125508

512

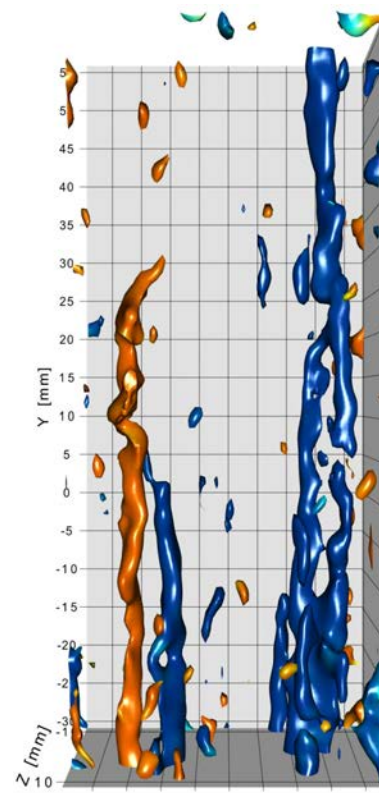

126754

513

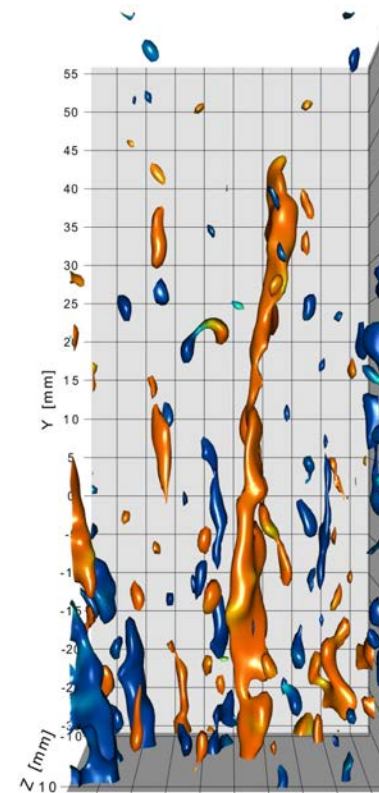

127867

514

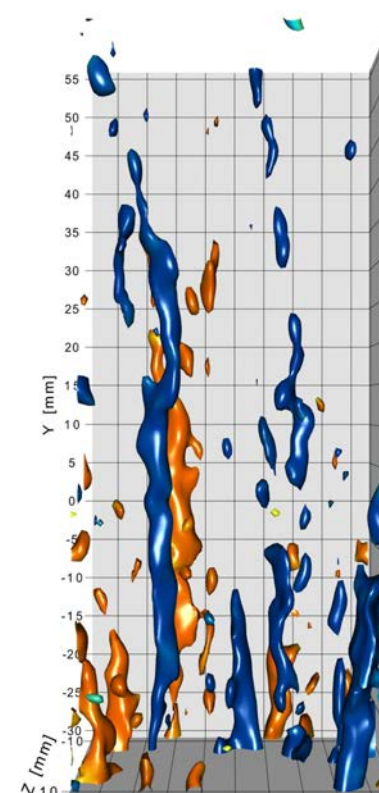

128295

515

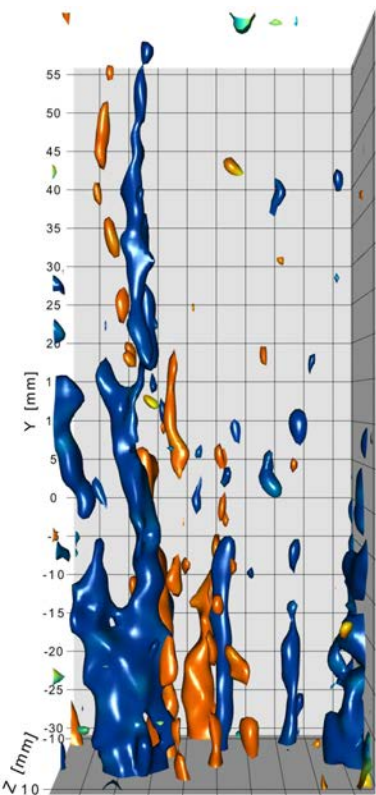

128759

516

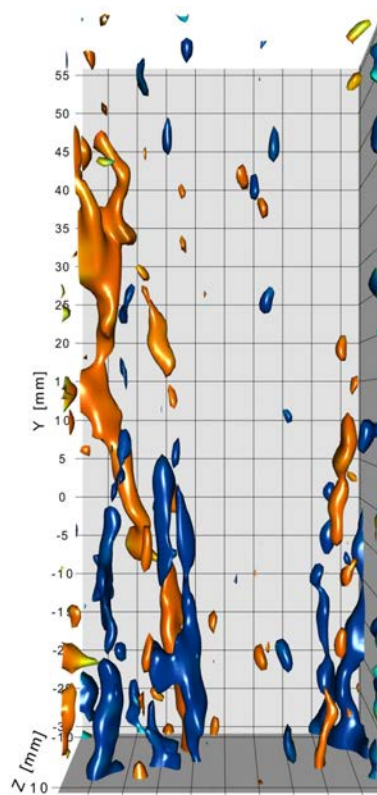

129024

517

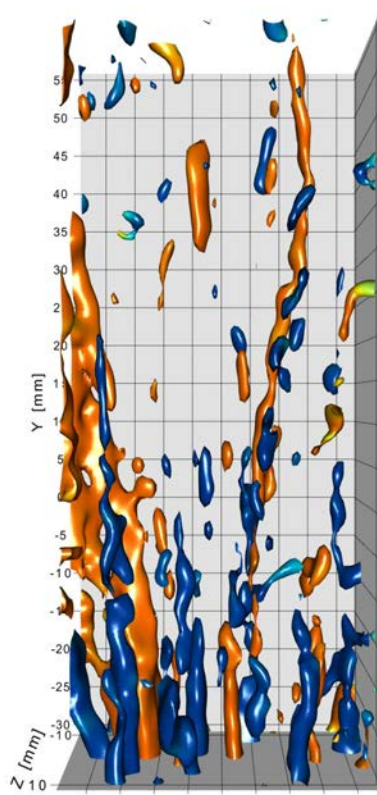

129216

518

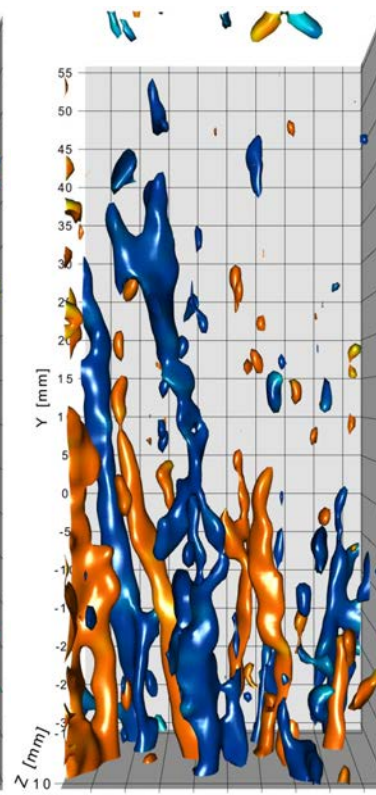

129457

519

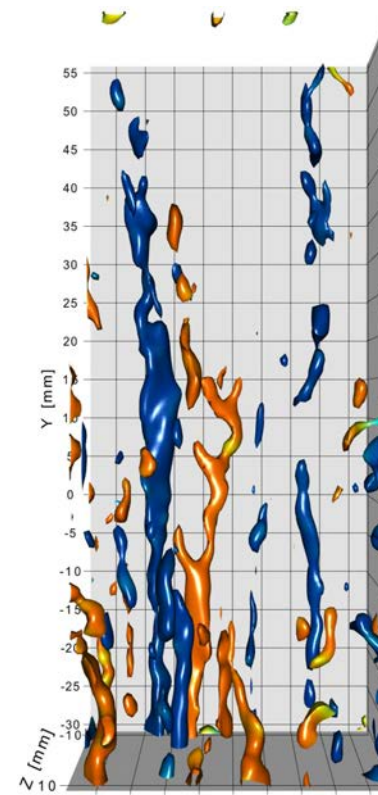

129998

520



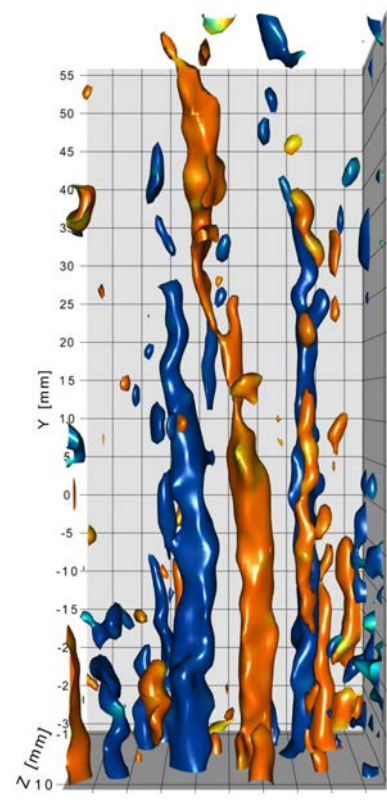

130276

521

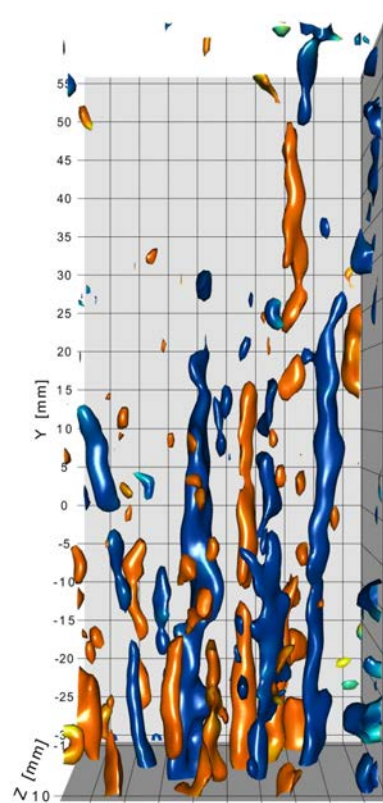

131274

522

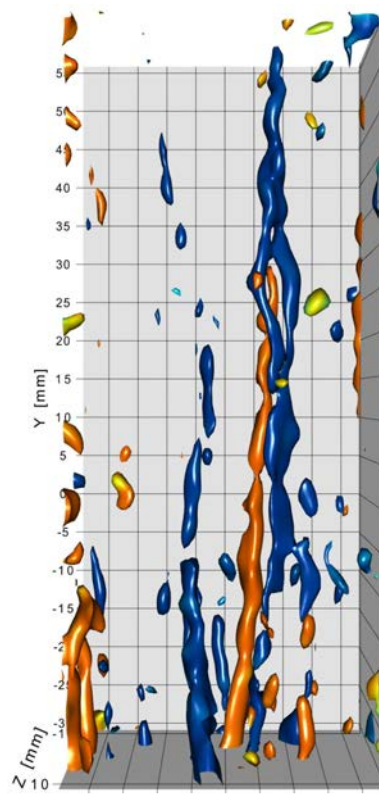

132723

523

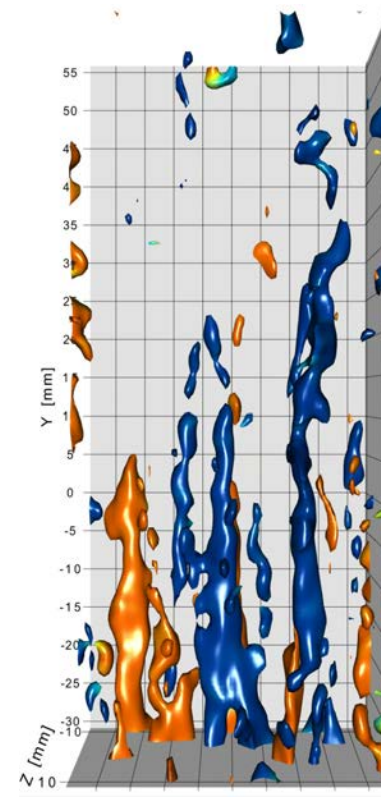

133796

524

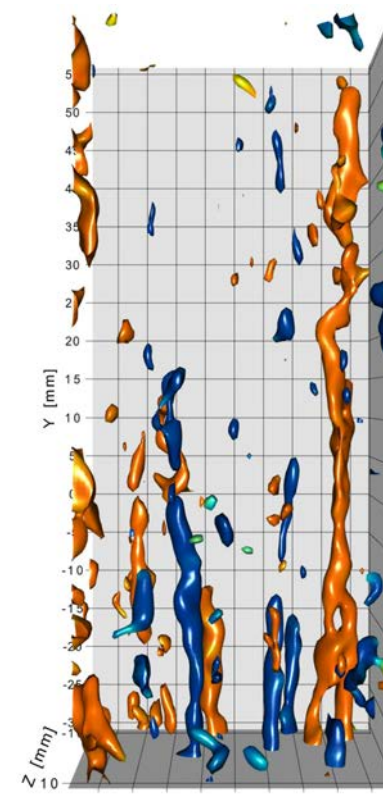

136465

525
