# Supplementary material for: Coherent turbulent structures in a rapid contraction
Source: arXiv:2401.05869 source file (2024-01-11)
Supplement: Supplementary file 4 [file StrRun4.pdf]

# Run4

Iso-surface of  $|\omega| = 40 \text{ } ^1/s$

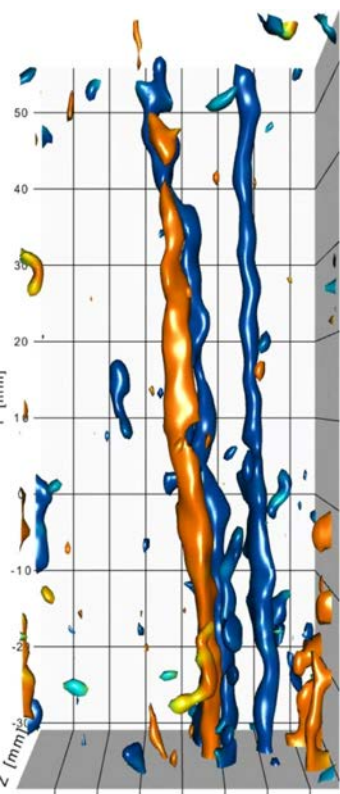

518

526

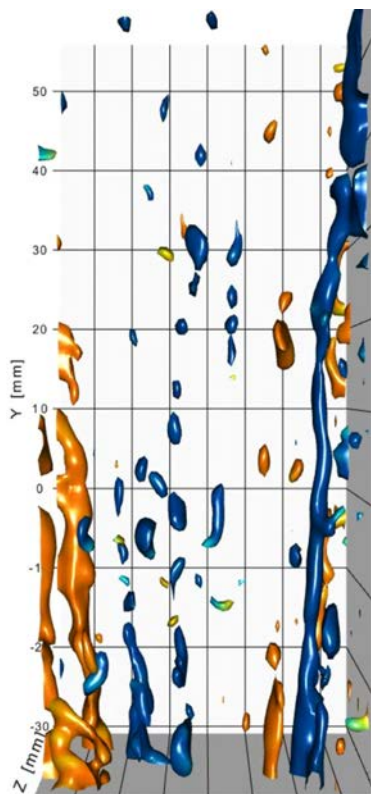

1766

527

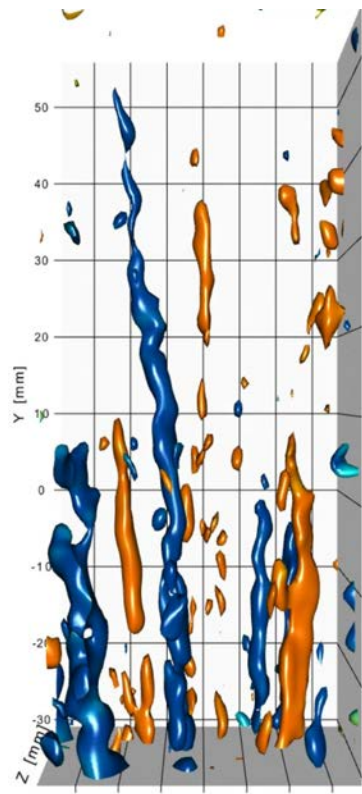

2293

528

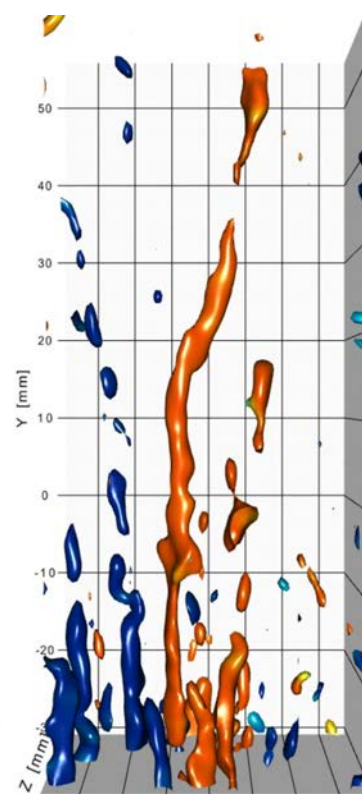

3665

529

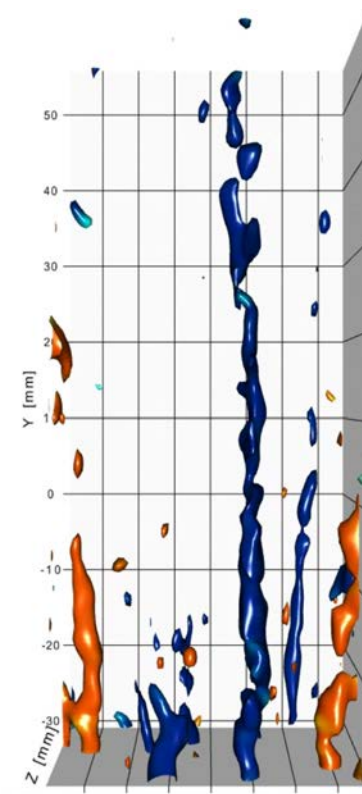

4817

530

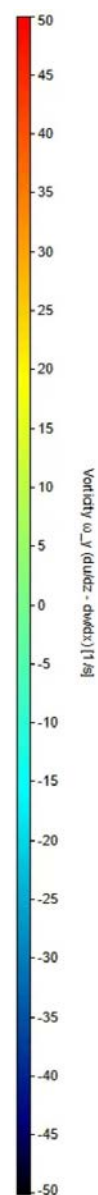

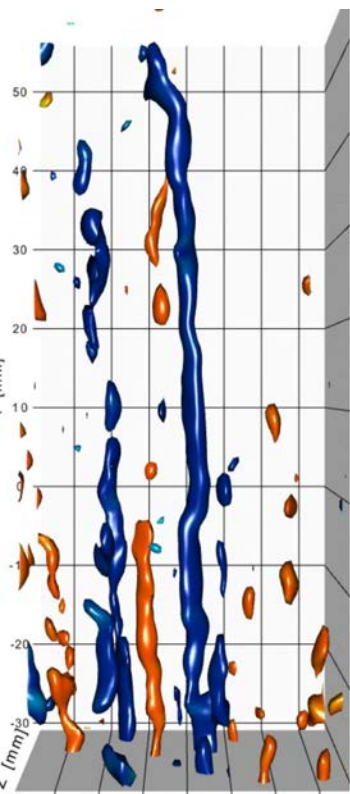

5077

531

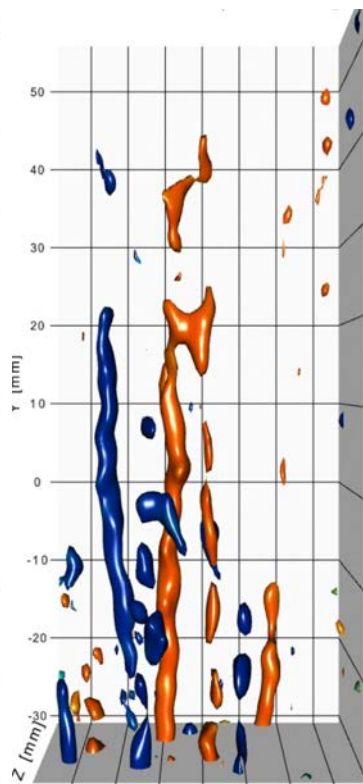

6938

532

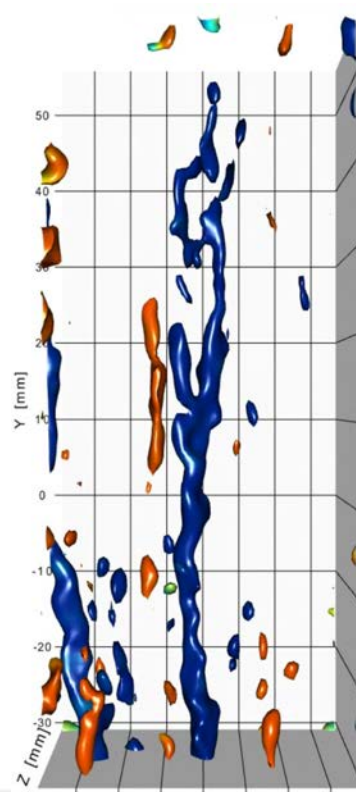

9005

533

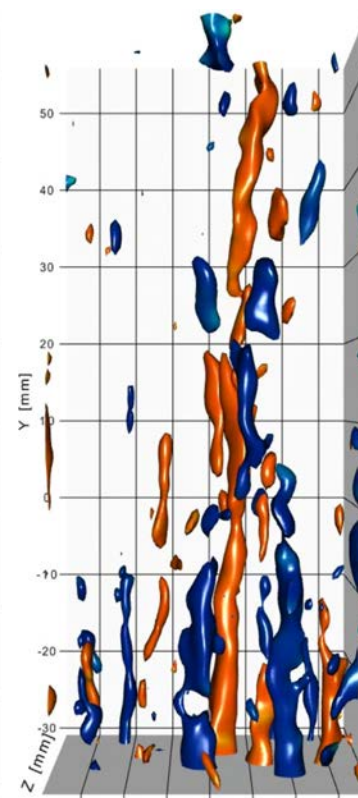

10975

534

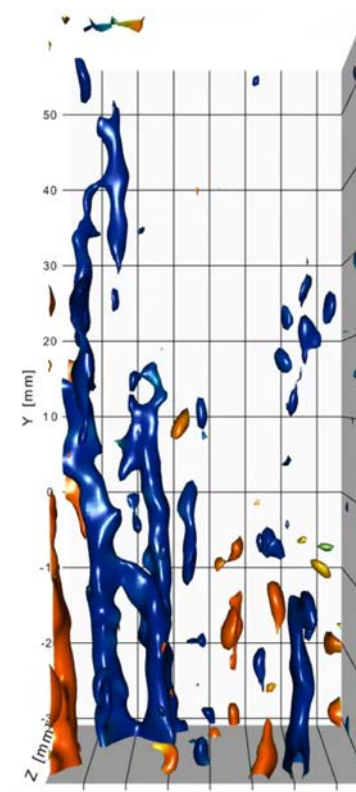

12082

535

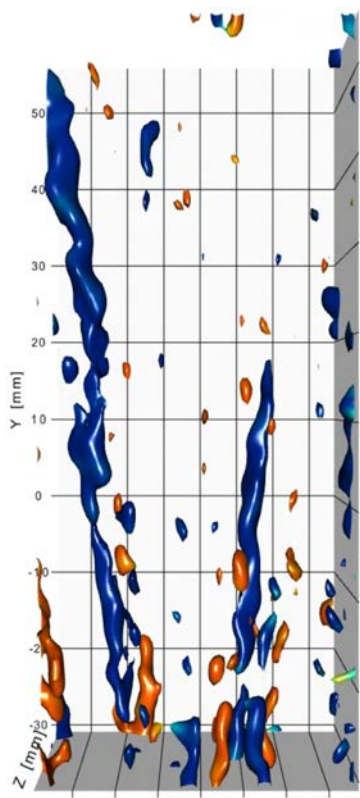

14212

536

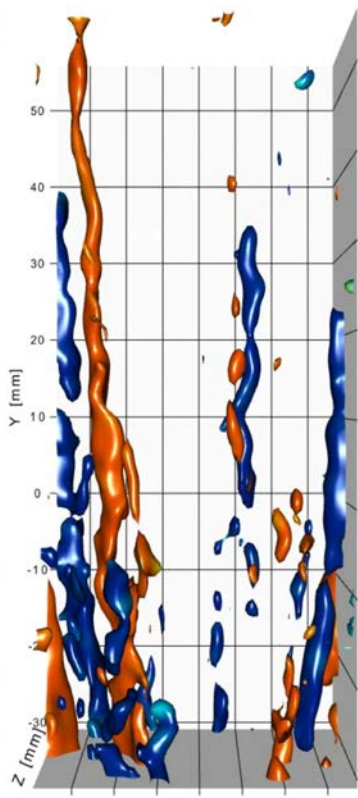

21342

537

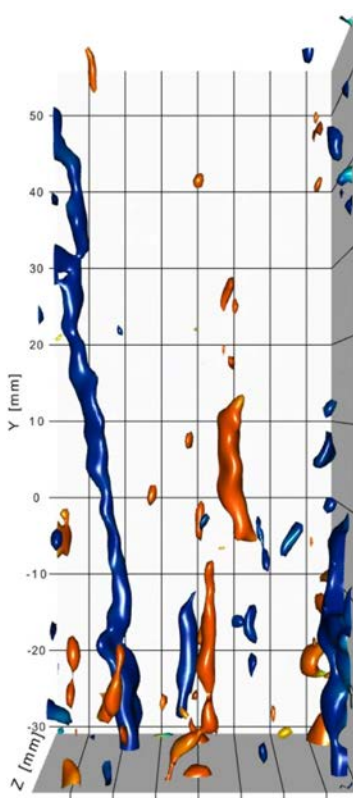

21903

538

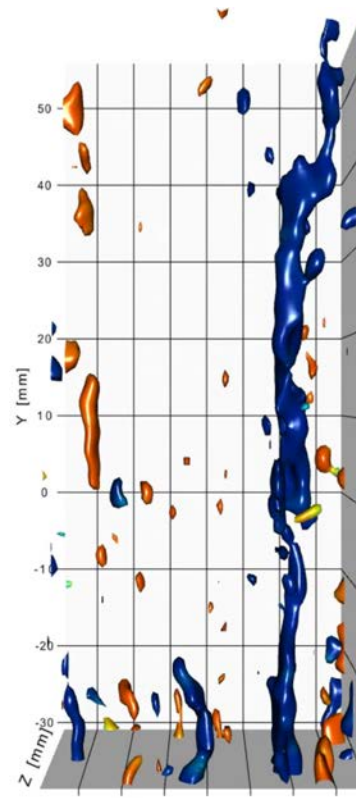

25169

539

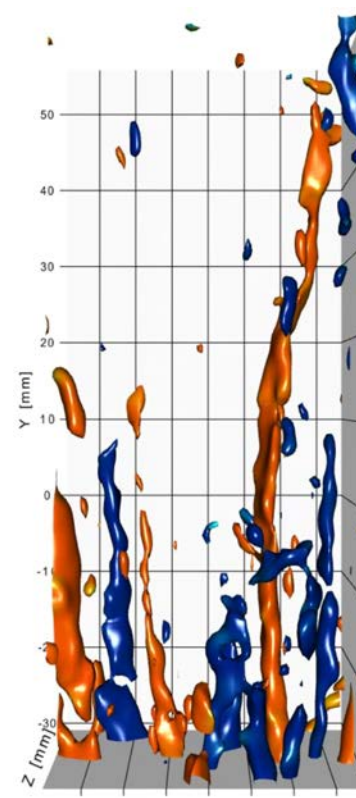

26443

540



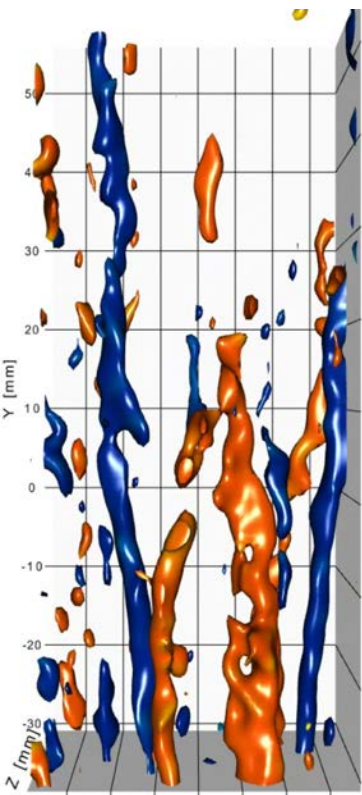

28587

541

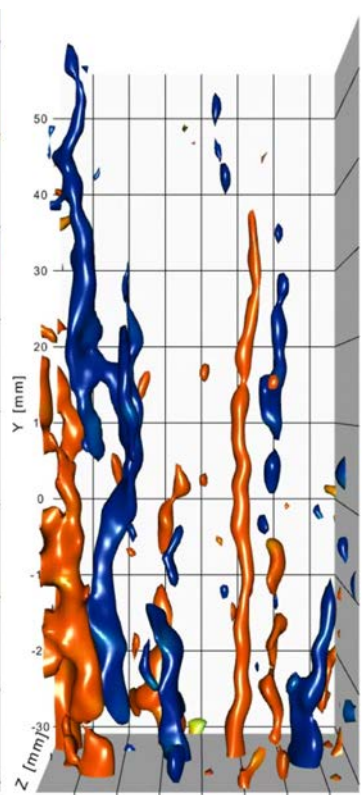

28872

542

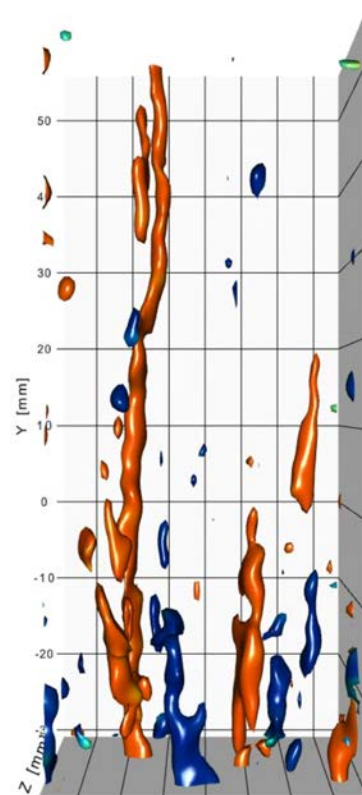

29719

543

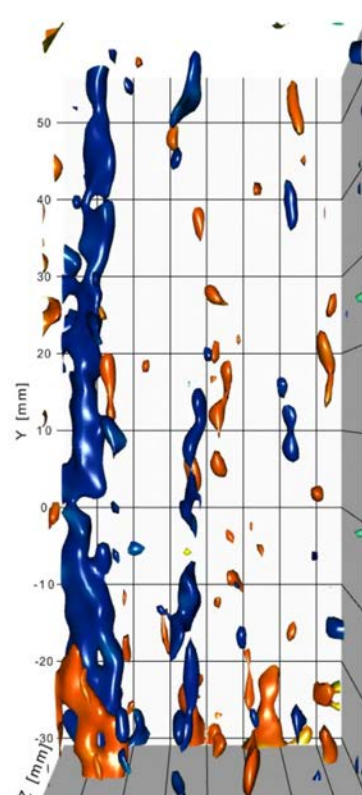

31839

544

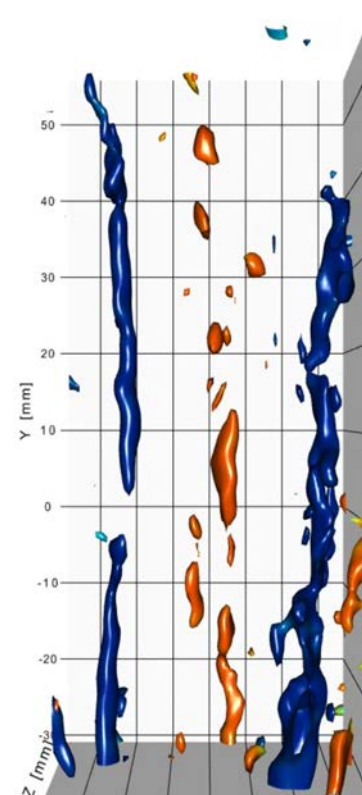

33922

545

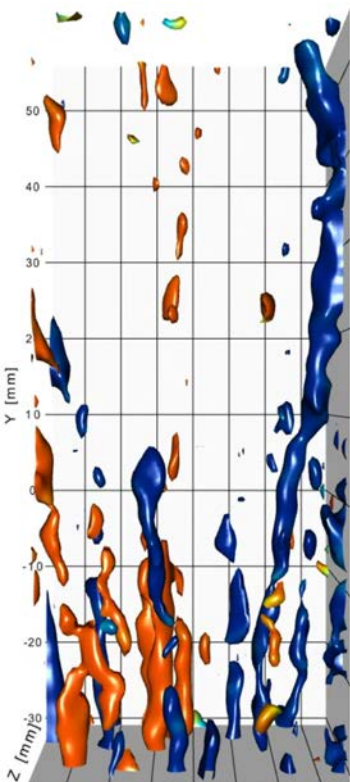

35435

546

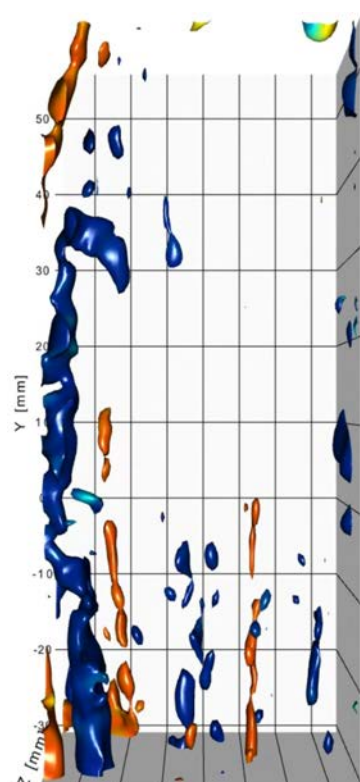

38333

547

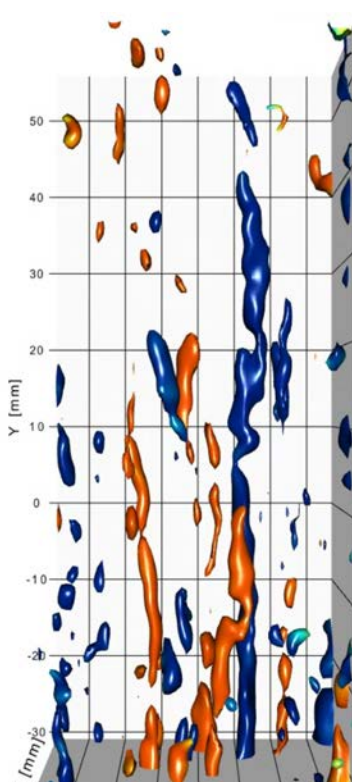

38940

548

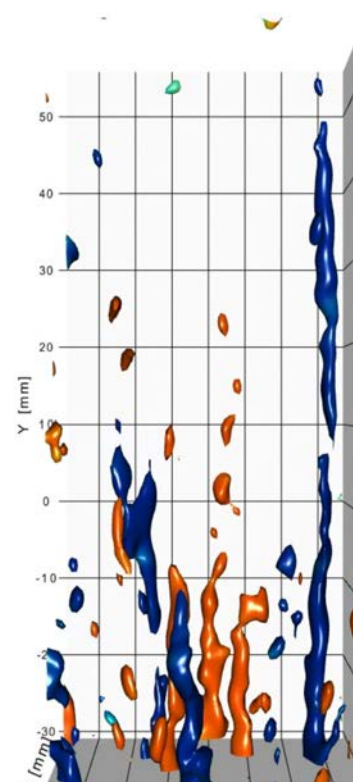

41741

549

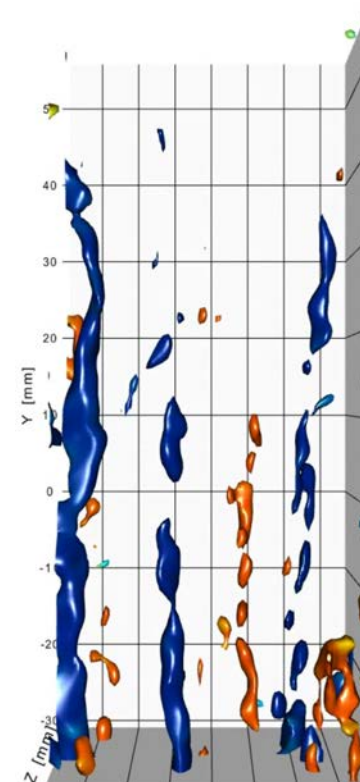

45037

550

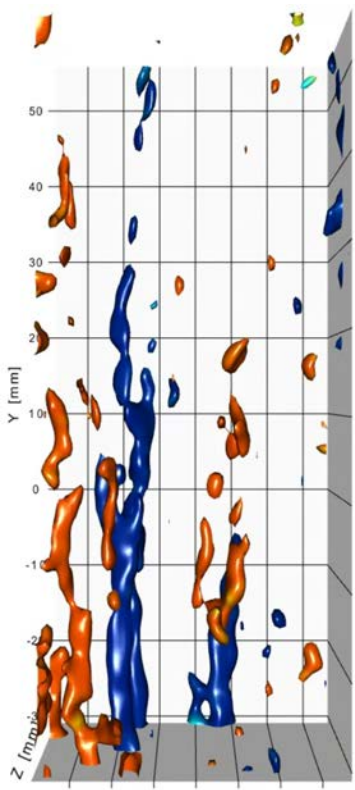

47543

551

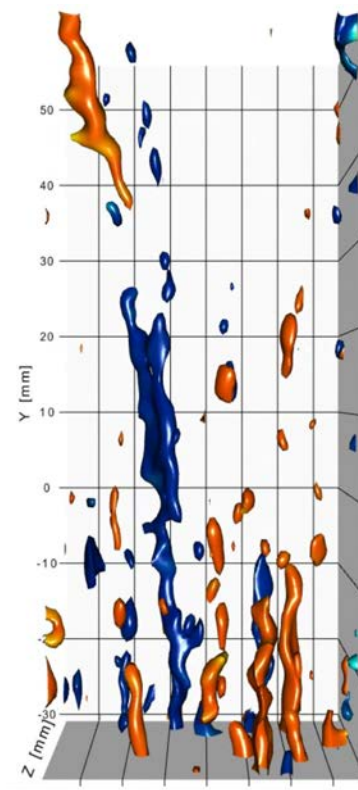

49084

552

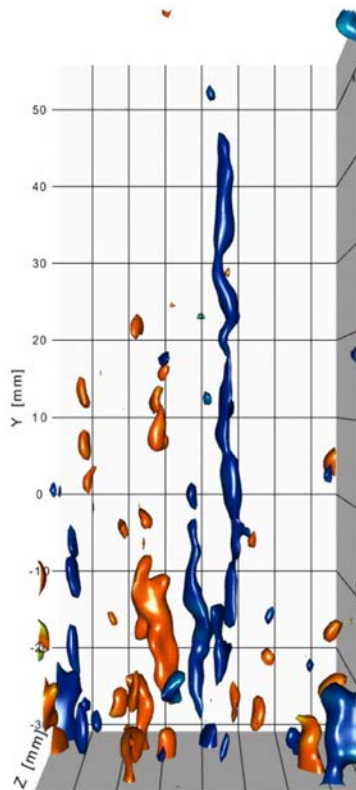

50561

553

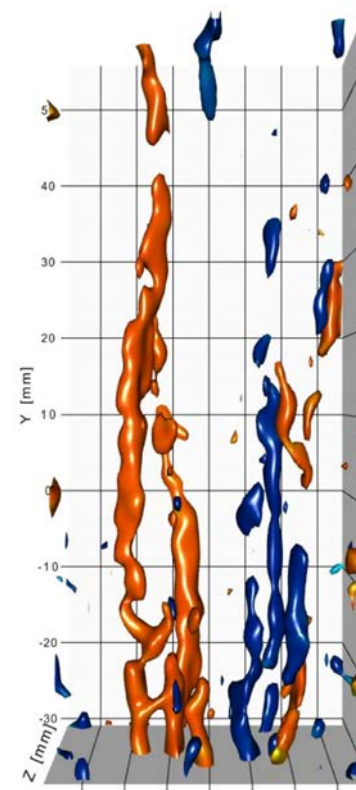

50928

554

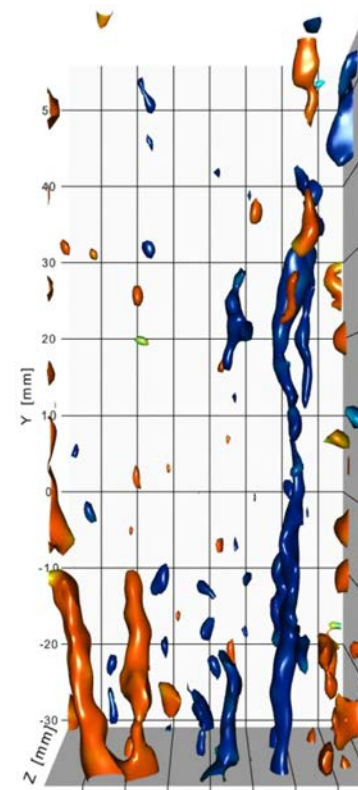

53785

555



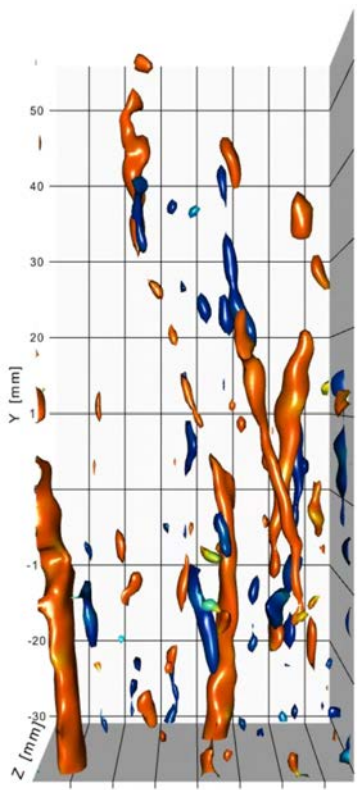

54180

556

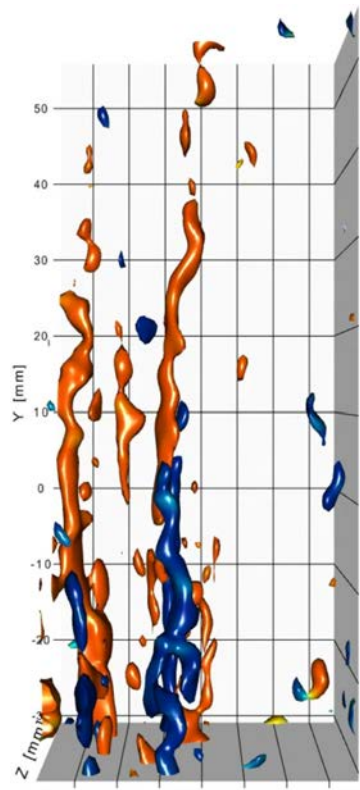

54589

557

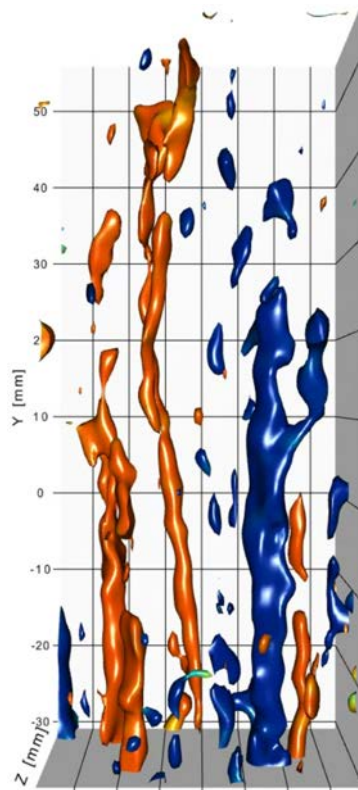

55688

558

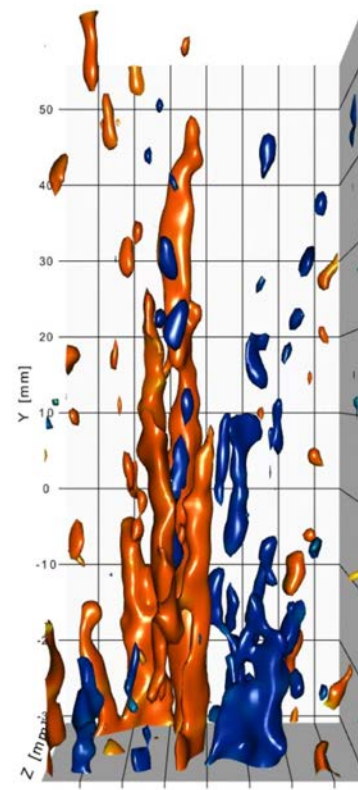

55867

559

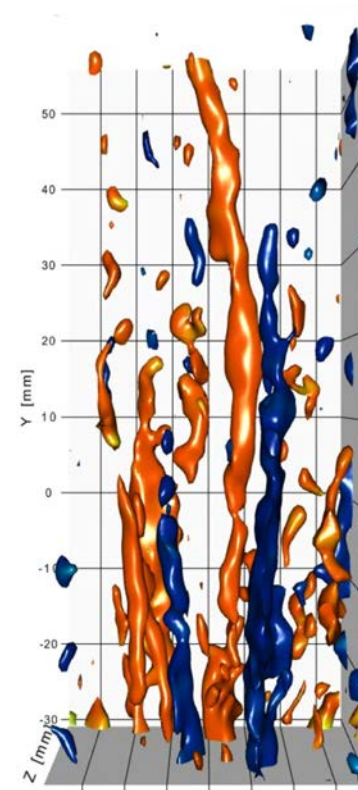

56065

560



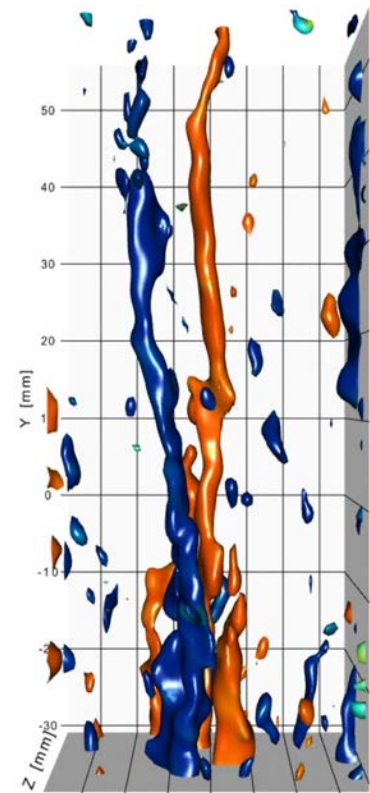

56431

561

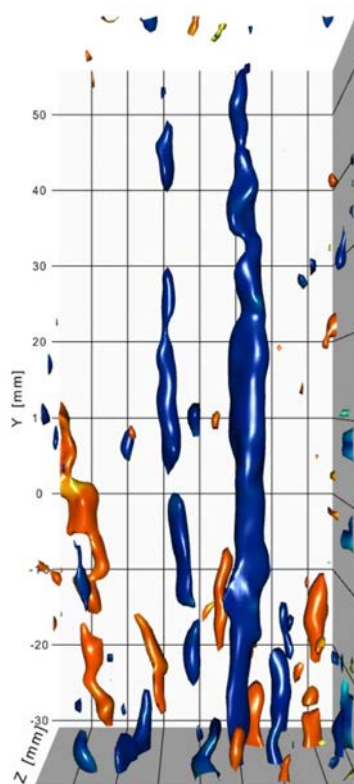

58137

562

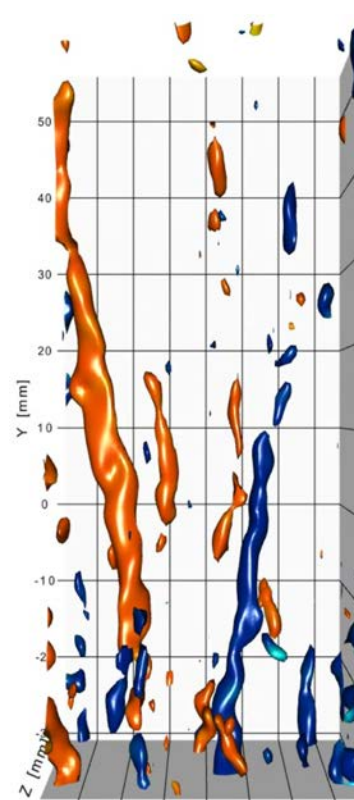

58471

563

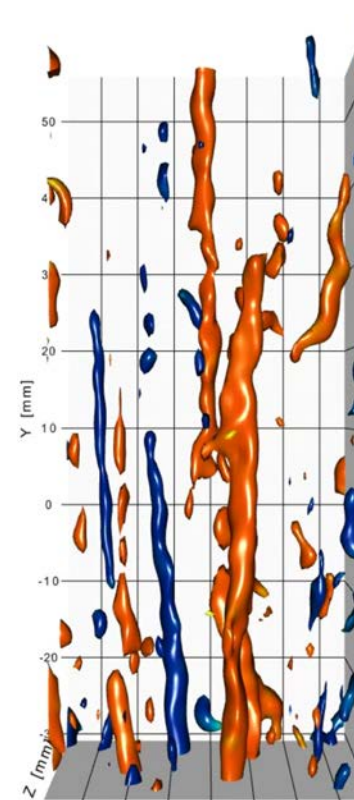

59173

564

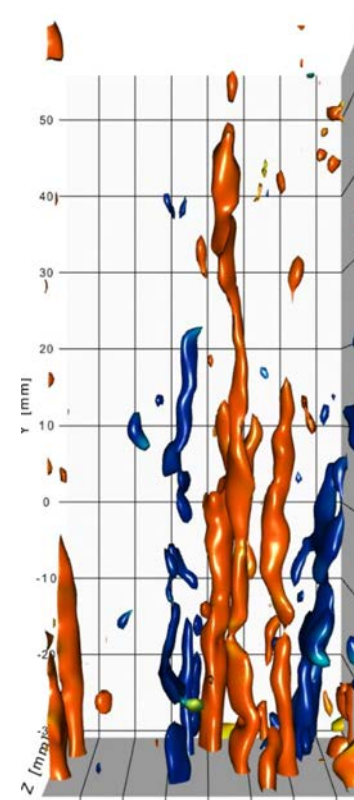

59482

565

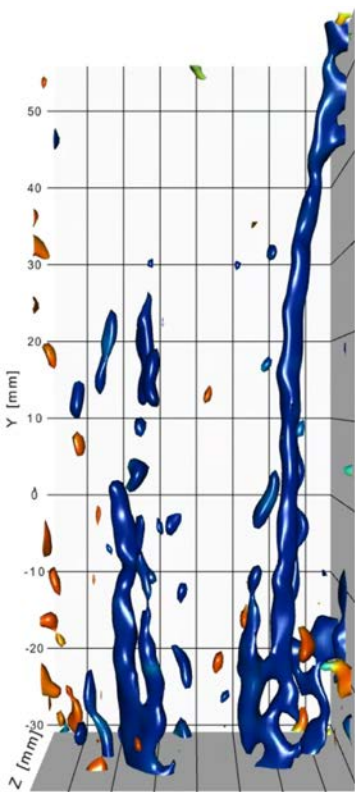

60683

566

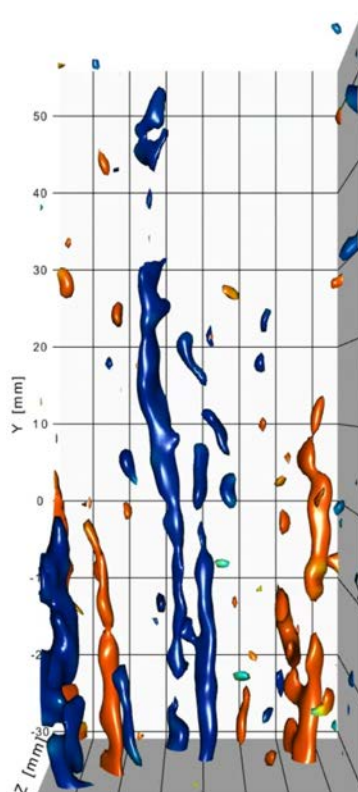

66089

567

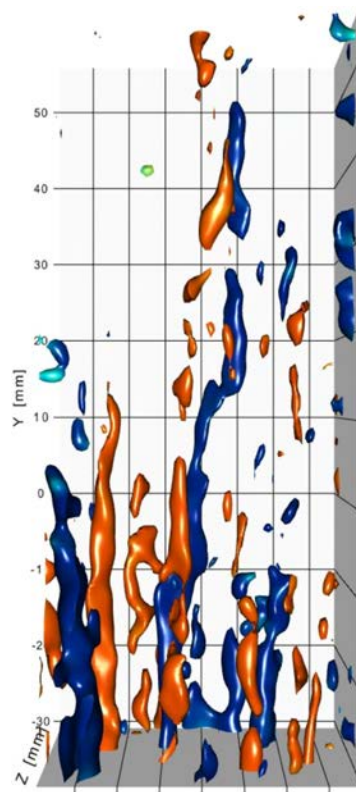

66368

568

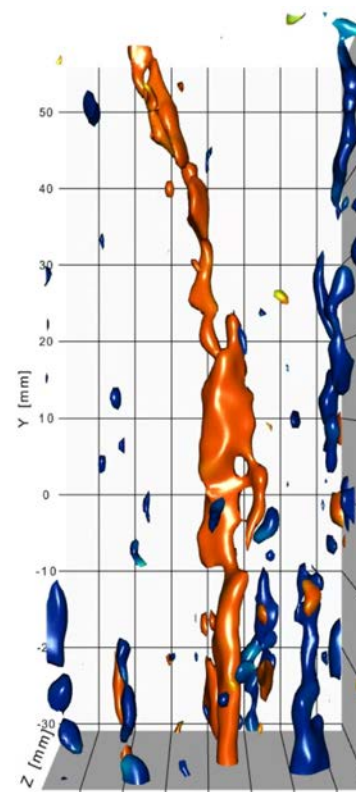

66653

569

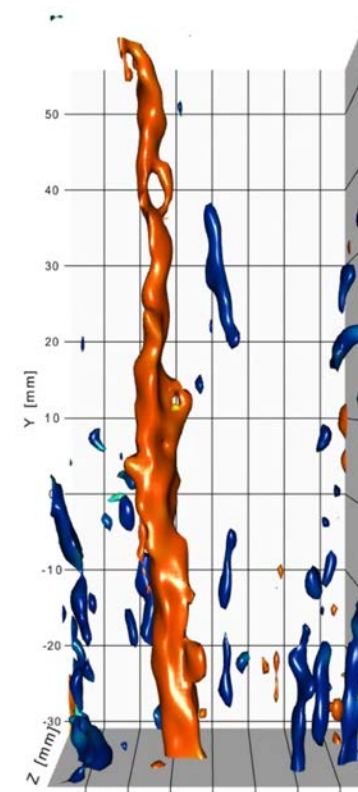

66881

570

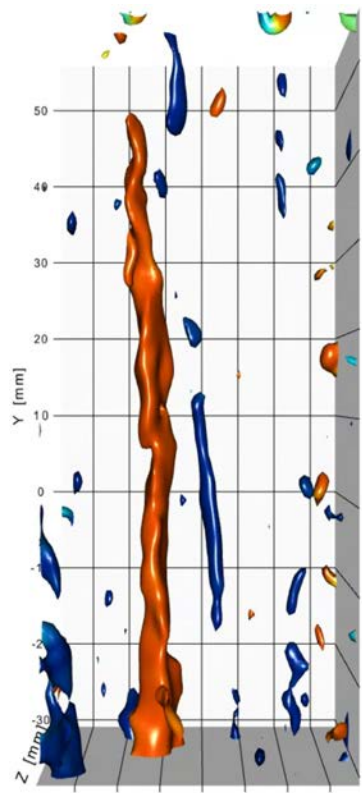

66965

571

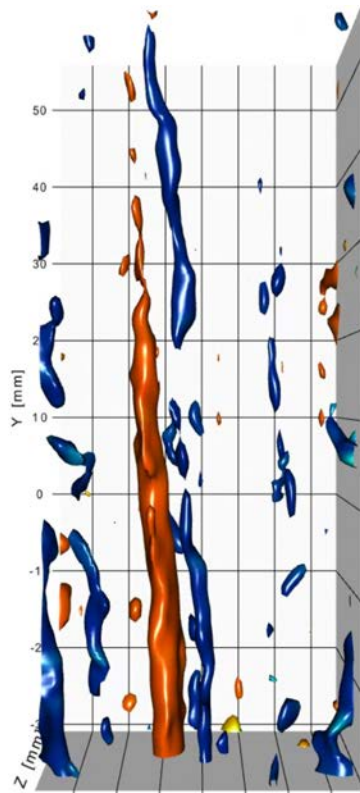

67047

572

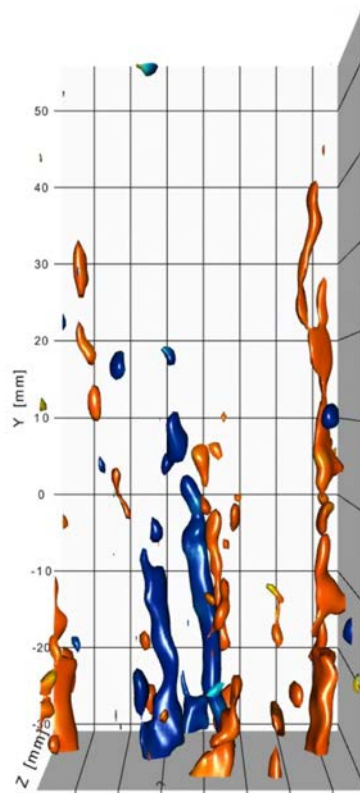

67498

573

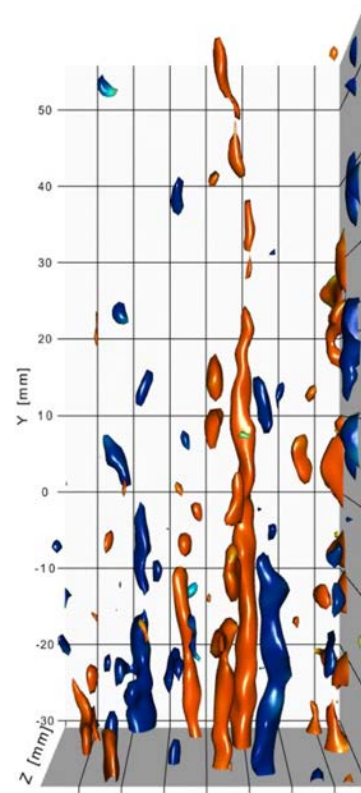

68370

574

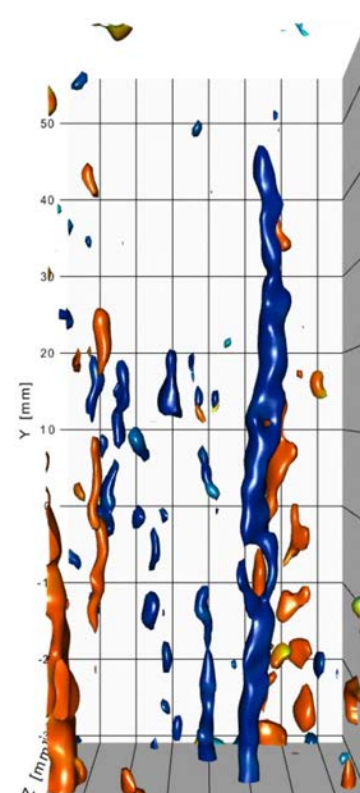

71272

575



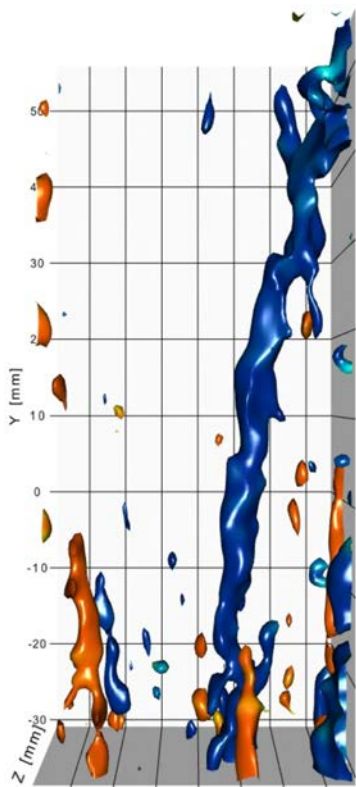

72707

576

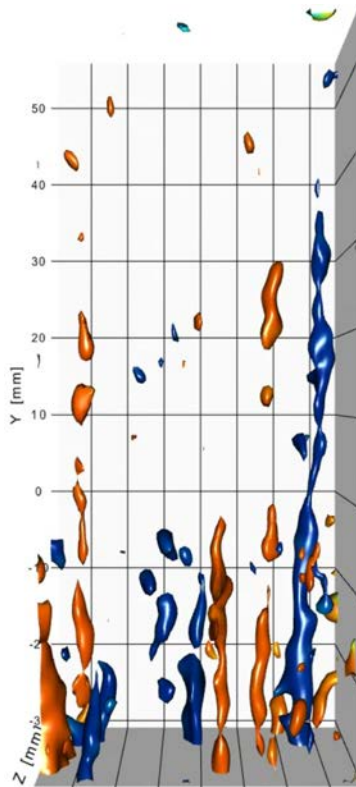

77740

577

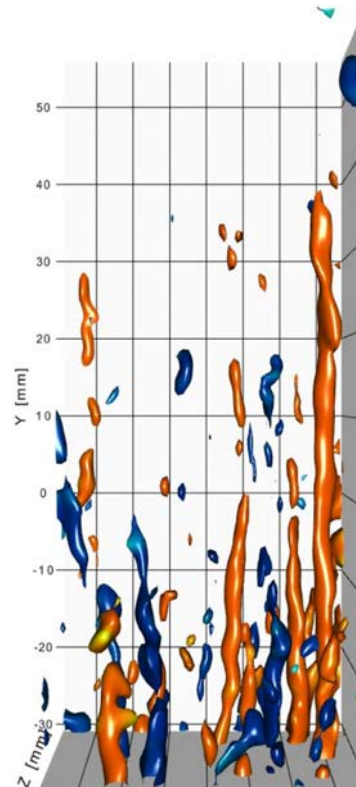

79323

578

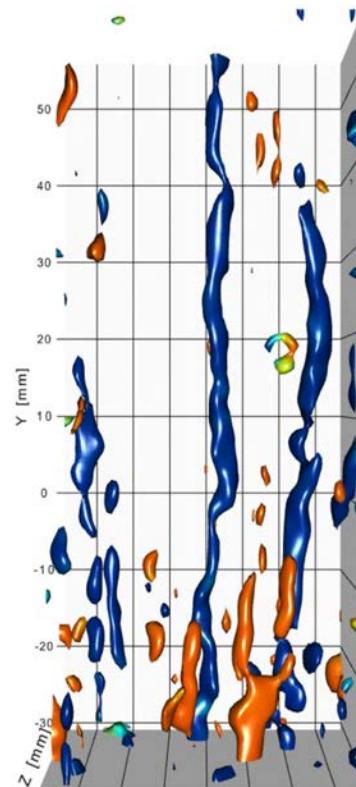

82124

579

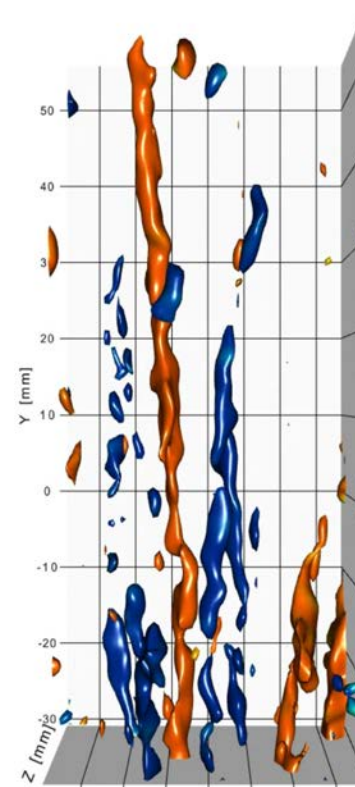

83171

580

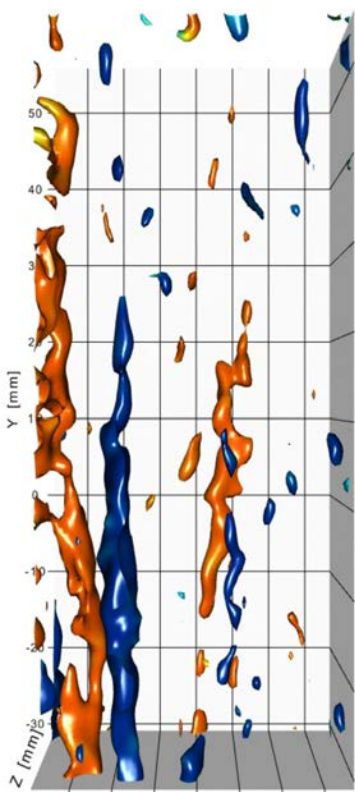

83933

581

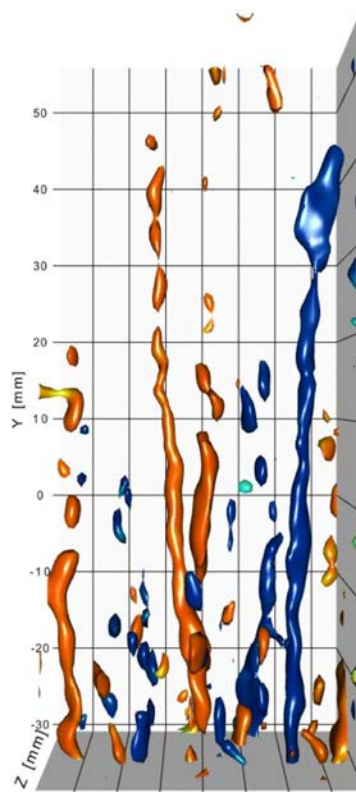

86229

582

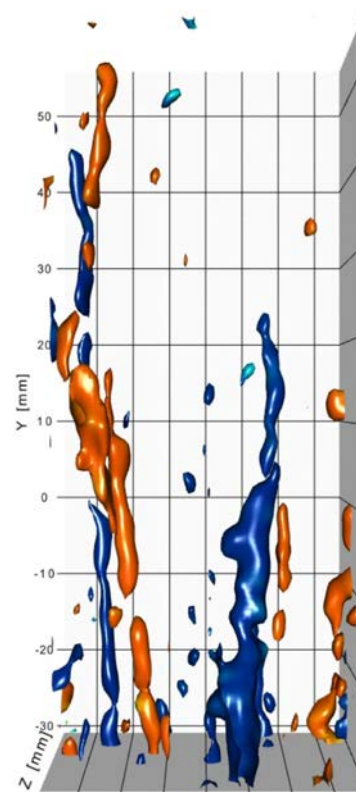

87834

583

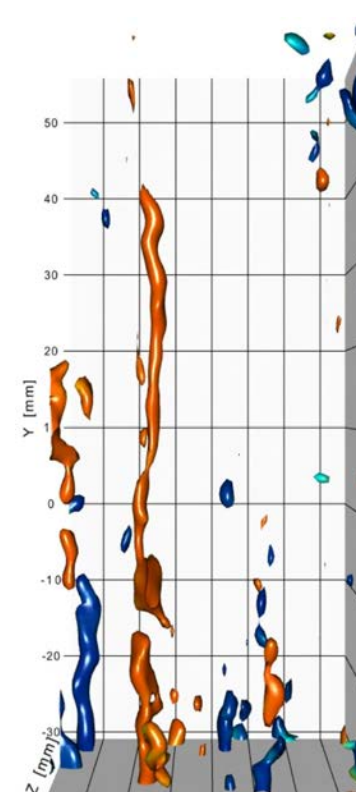

88439

584

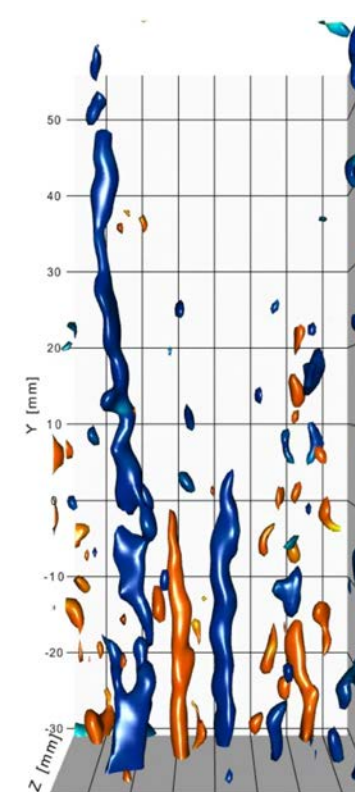

89707

585

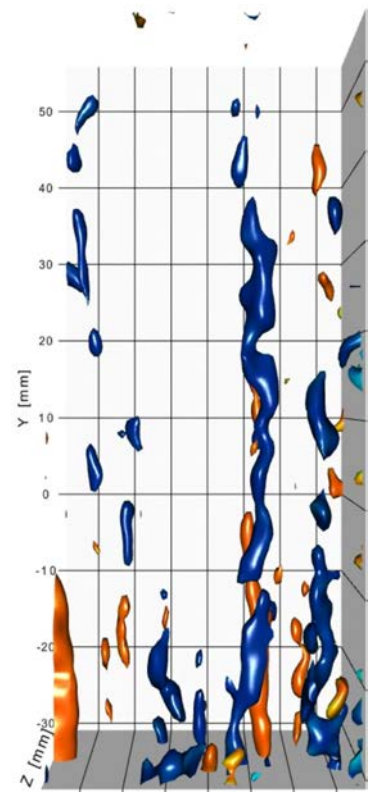

91015

586

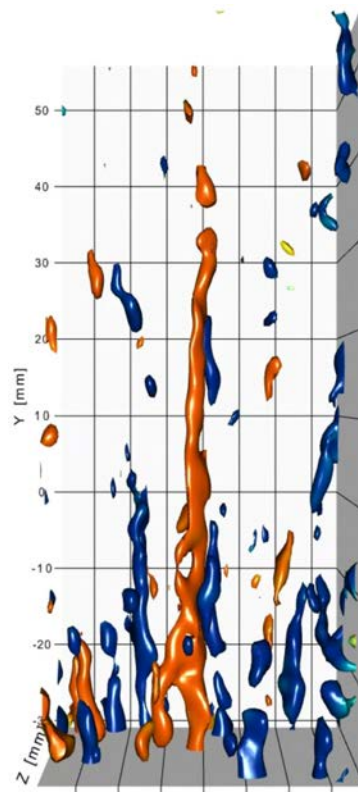

91333

587

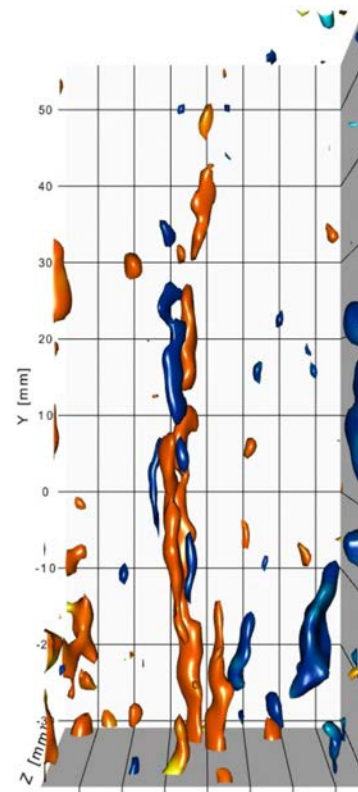

92776

588

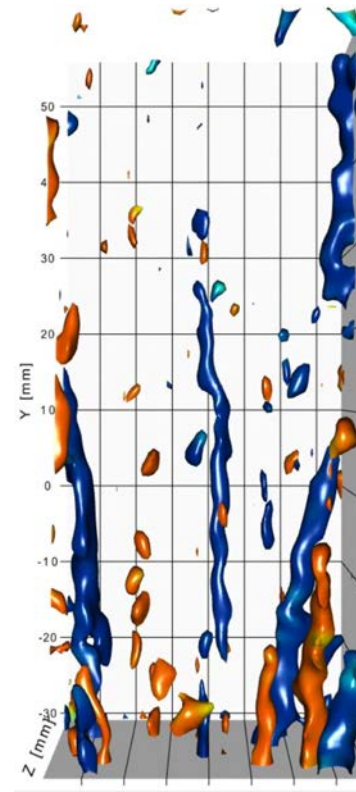

93637

589

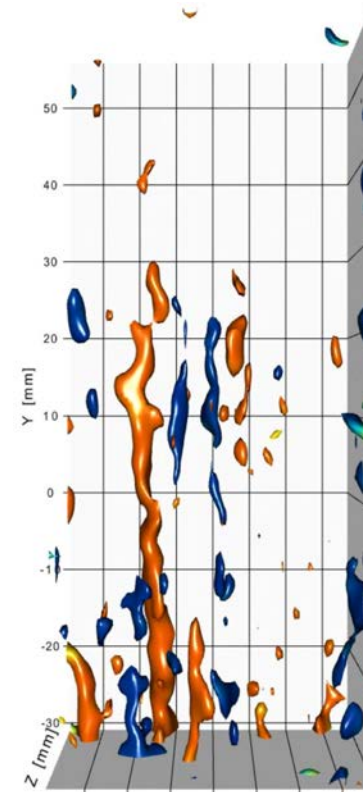

95581

590



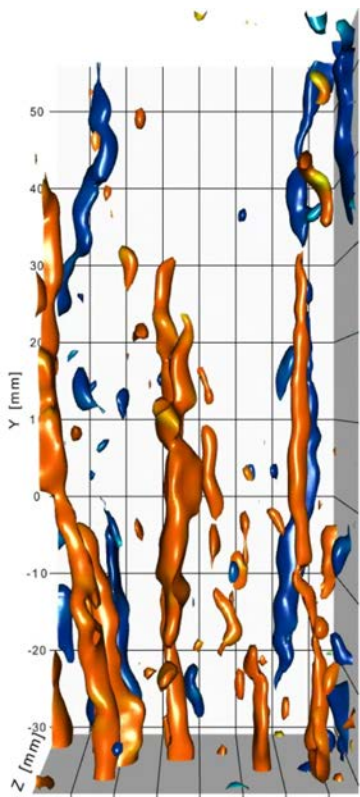

96353

591

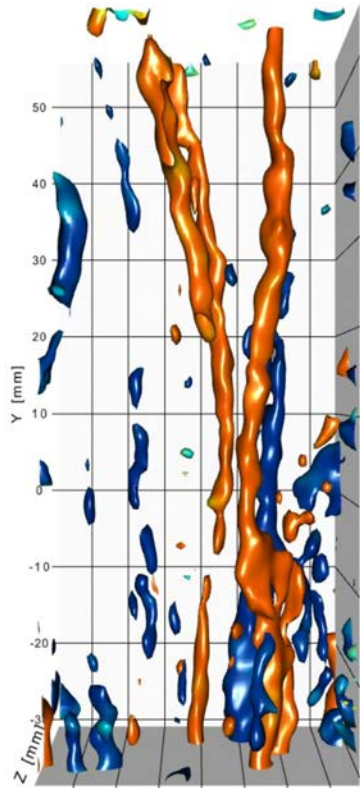

97378

592

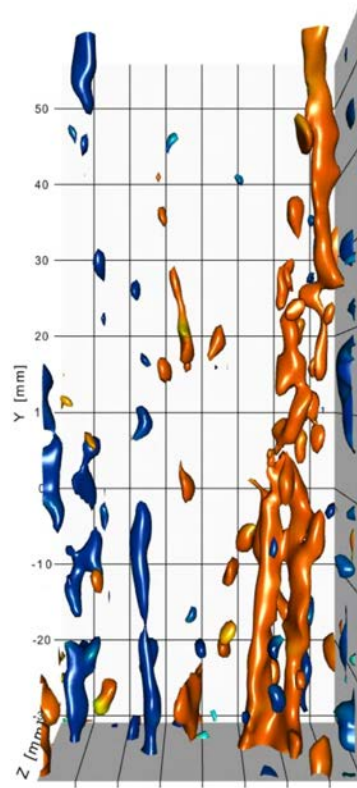

98483

593

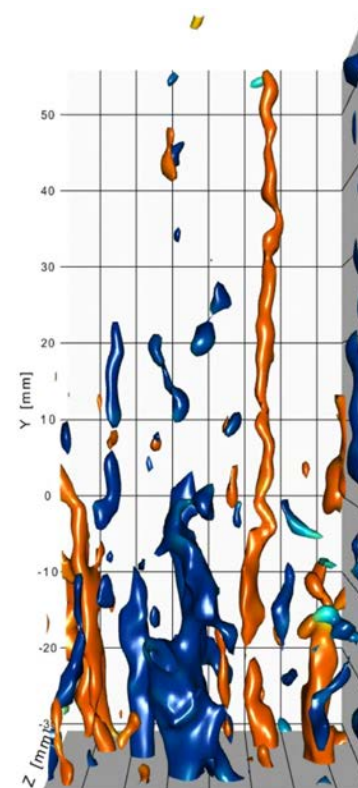

98801

594

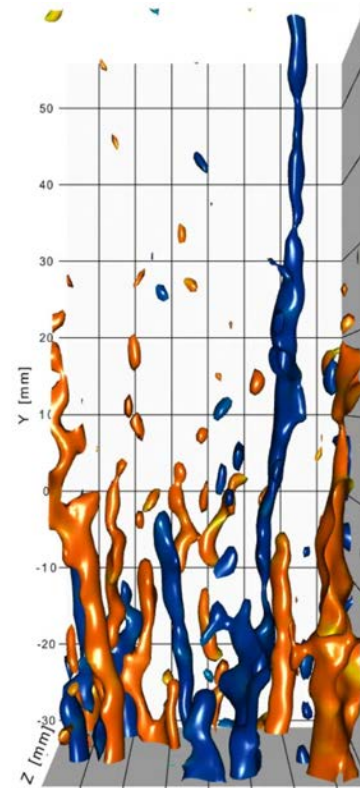

99932

595

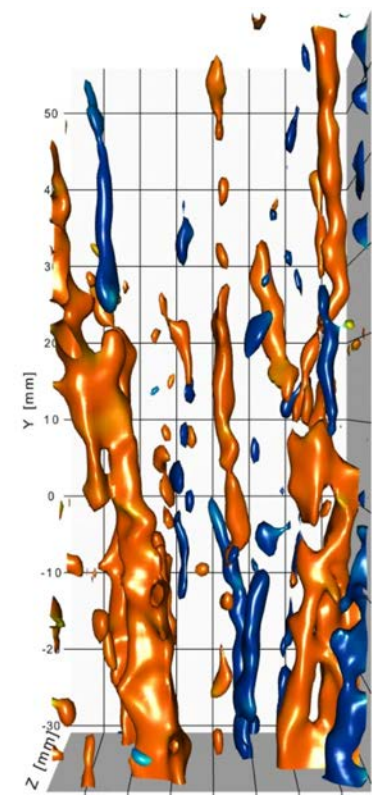

100503

596

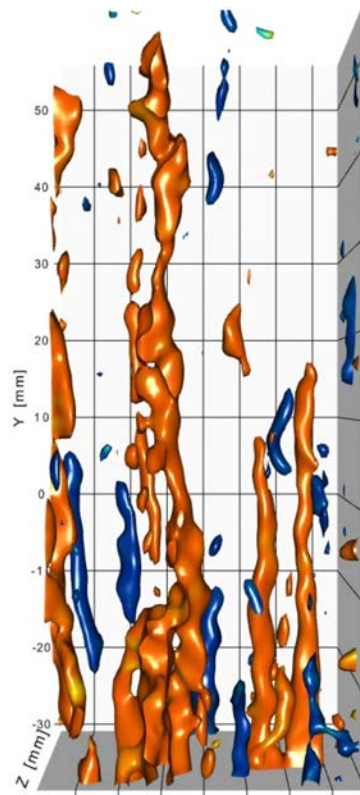

100825

597

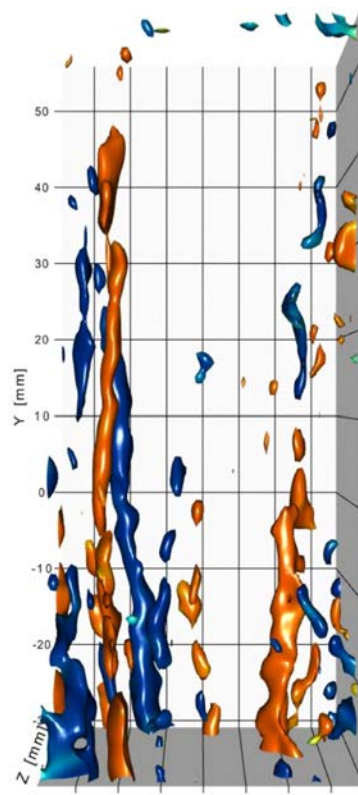

101248

598

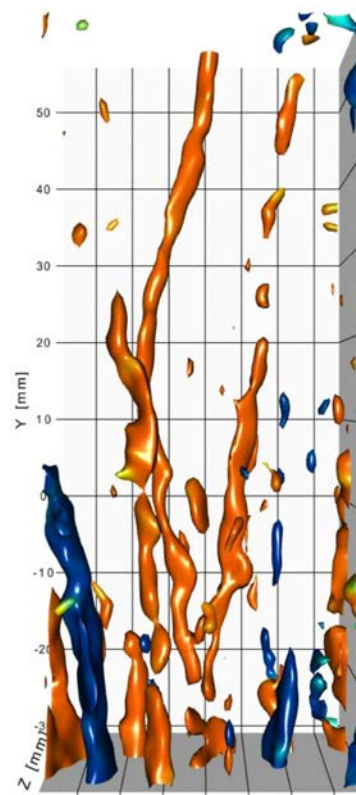

101692

599

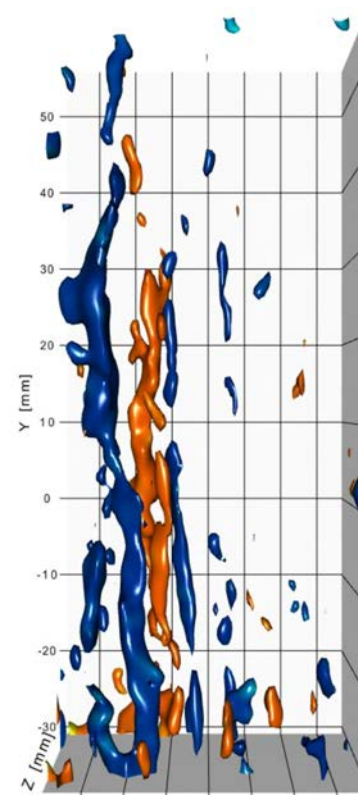

102412

600



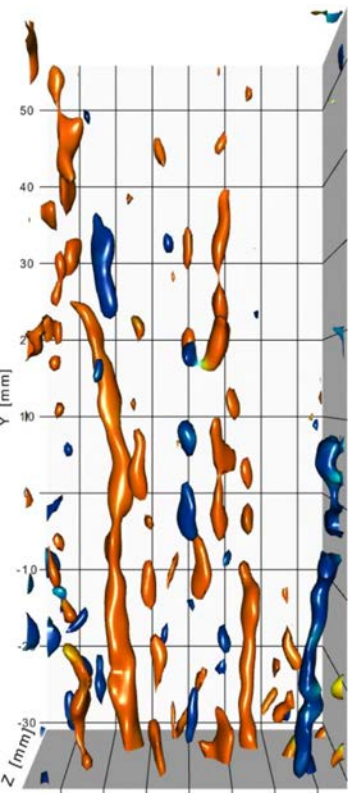

104452

601

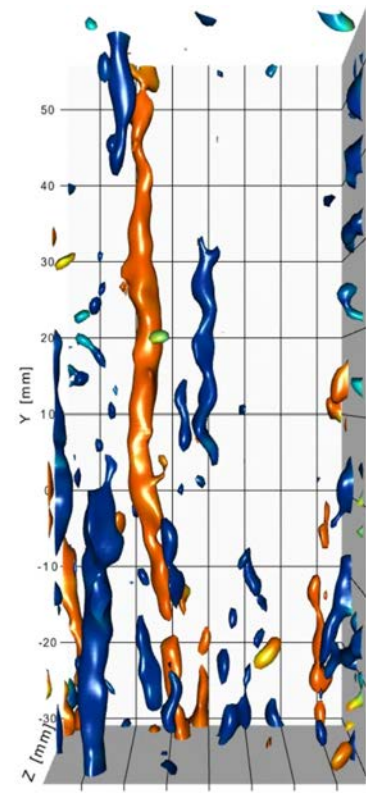

107736

602

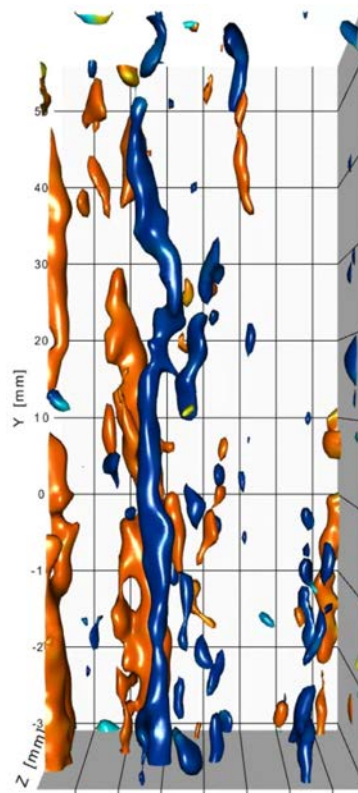

107913

603

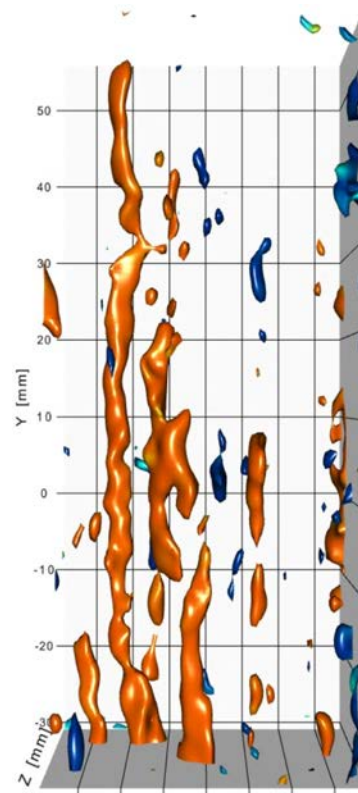

108272

604

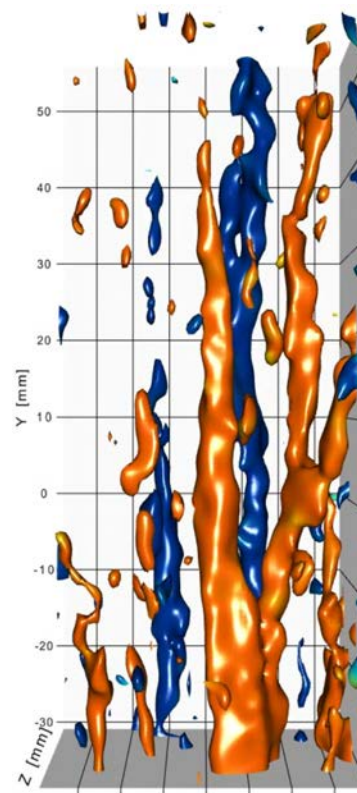

110093

605



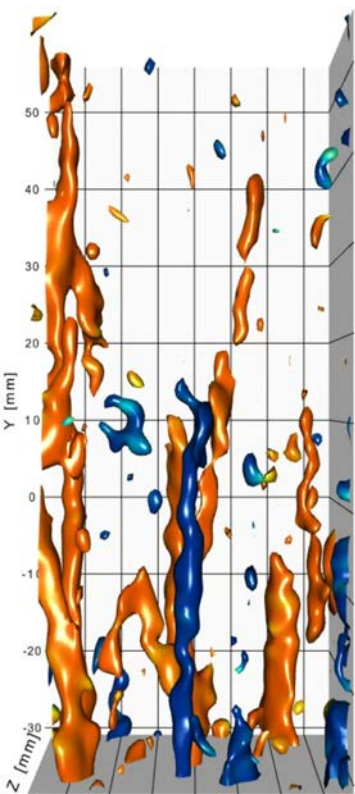

110671

606

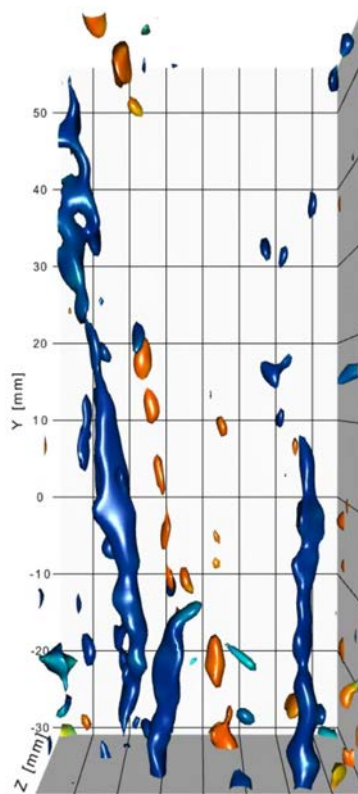

112189

607

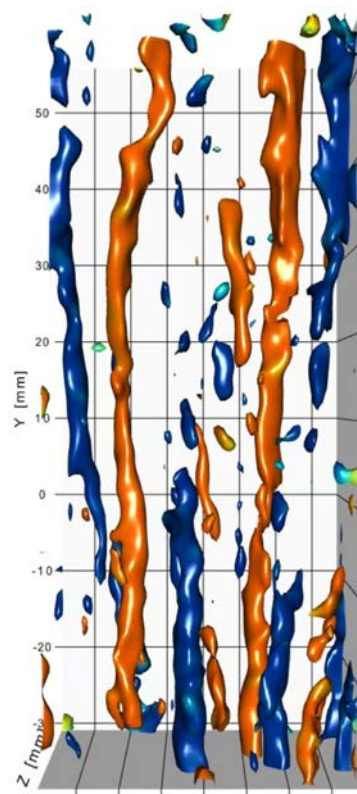

112860

608

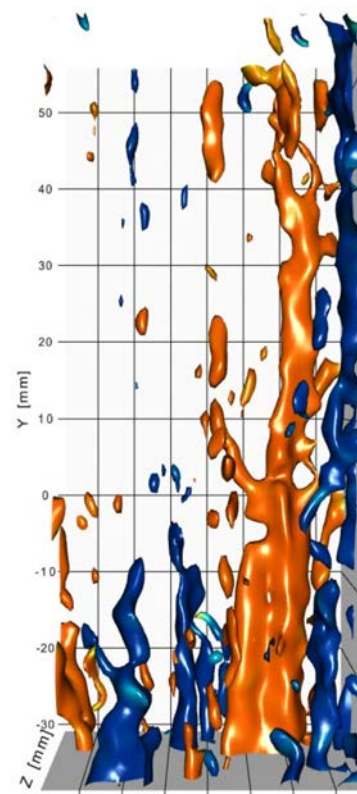

113496

609

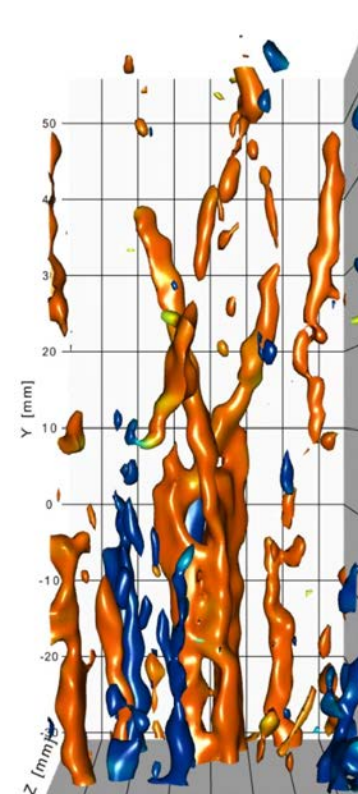

113882

610

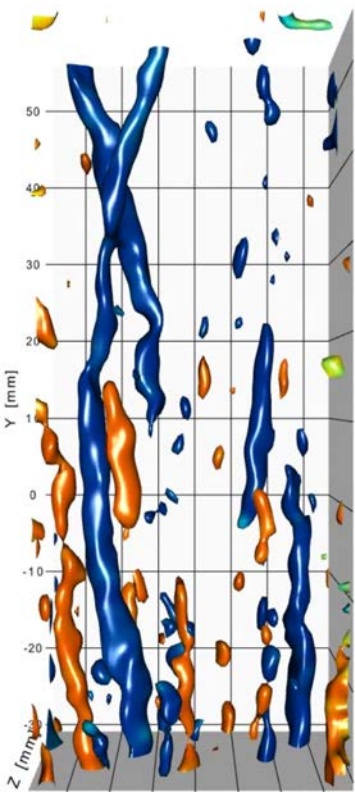

114580

611

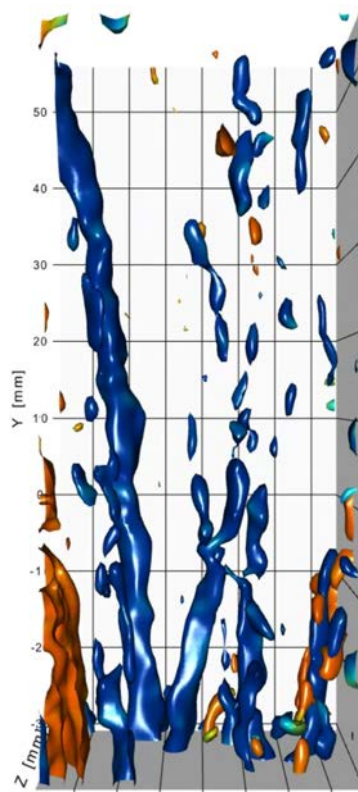

114823

612

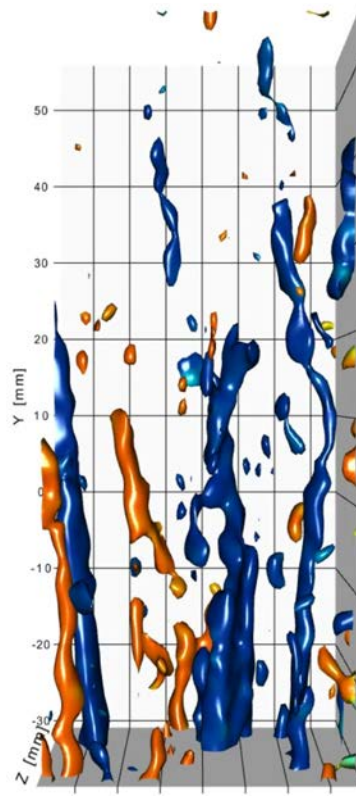

115113

613

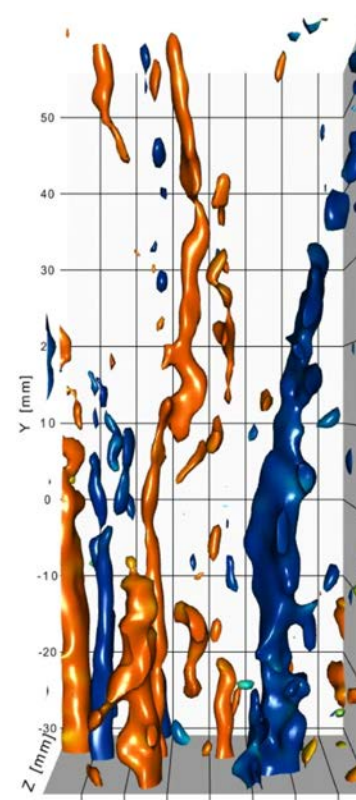

115962

614

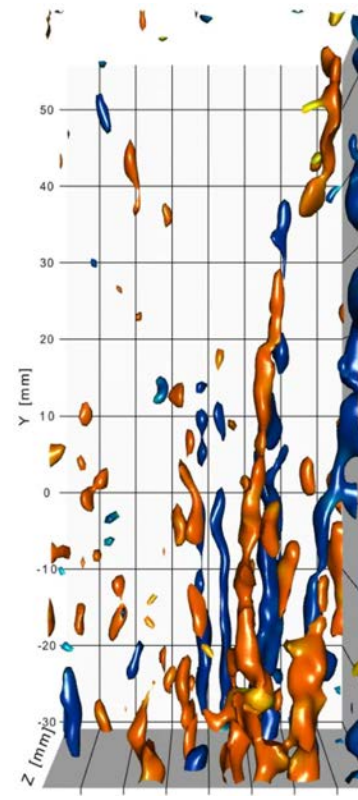

116908

615



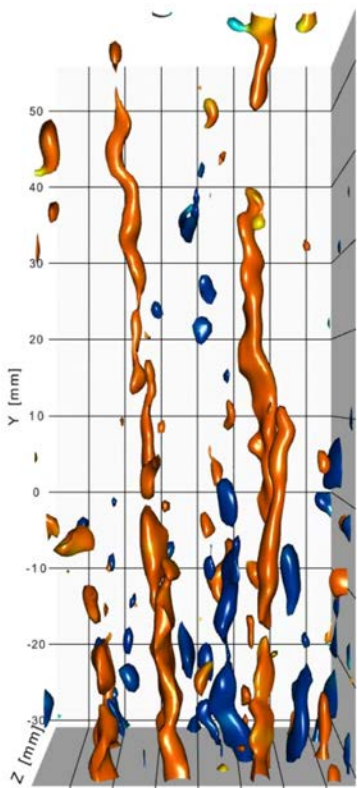

117207

616

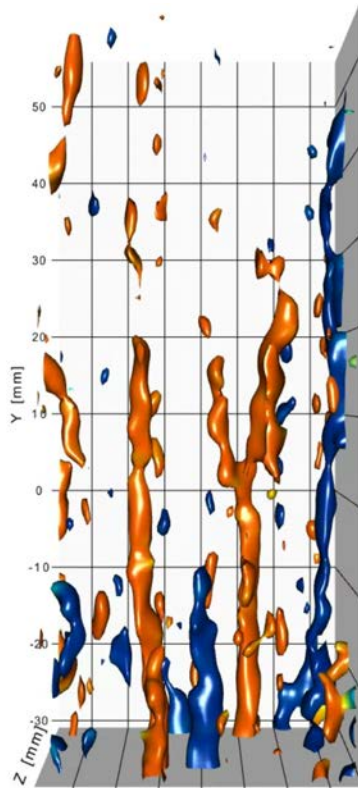

117337

617

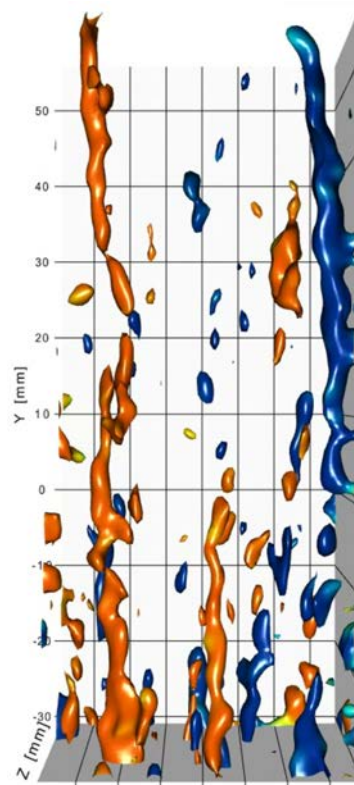

118819

618

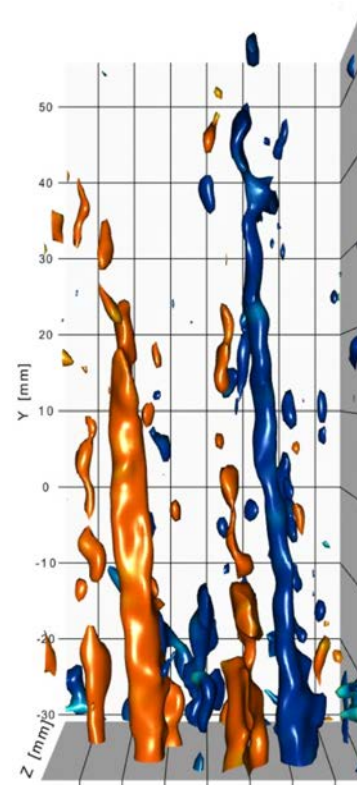

118969

619

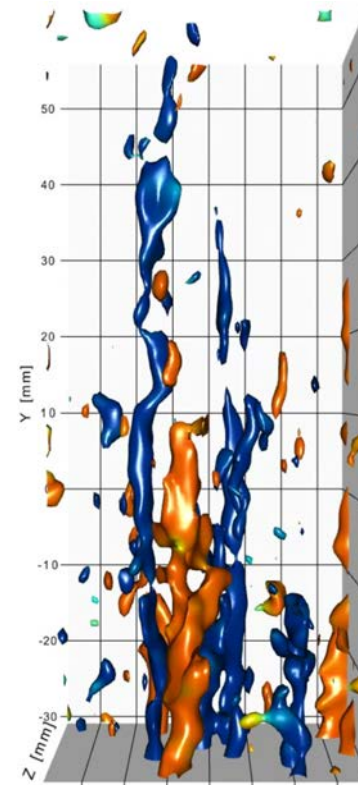

119908

620



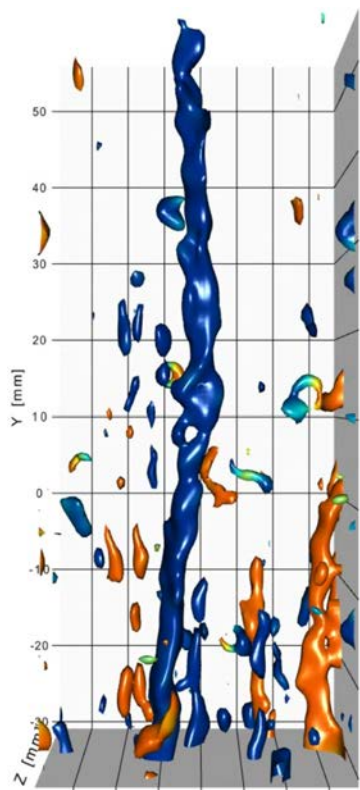

120093

621

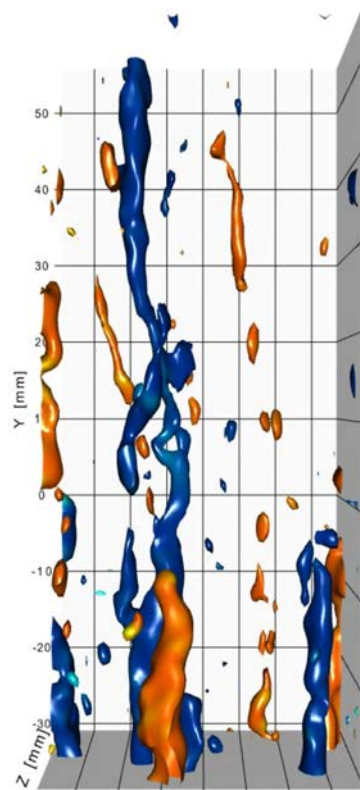

120413

622

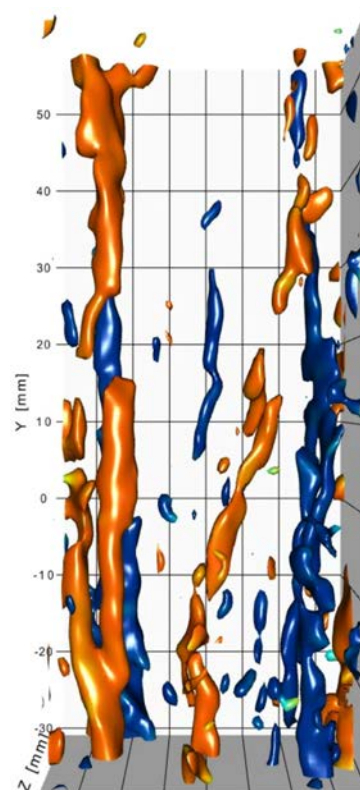

120851

623

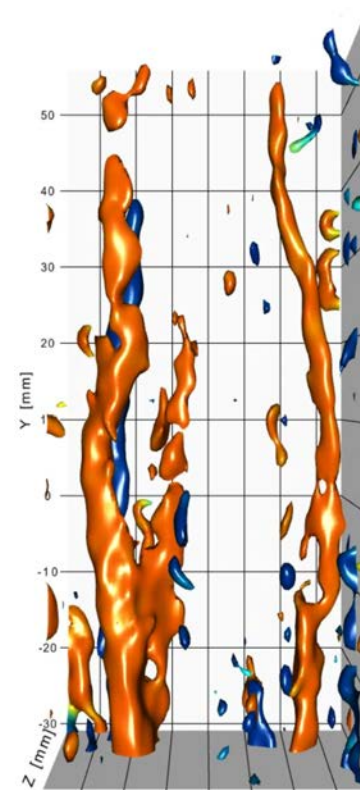

121090

624

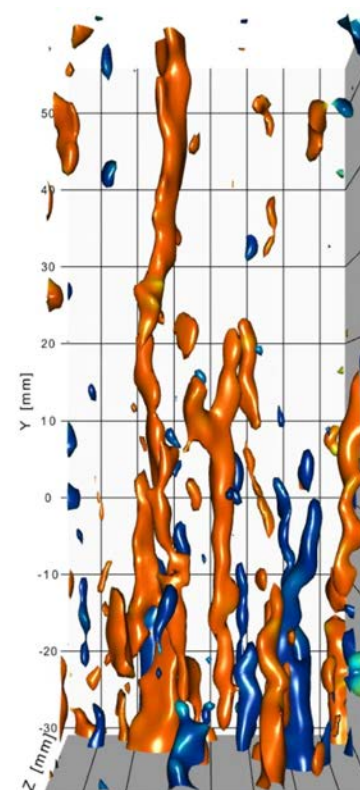

121329

625

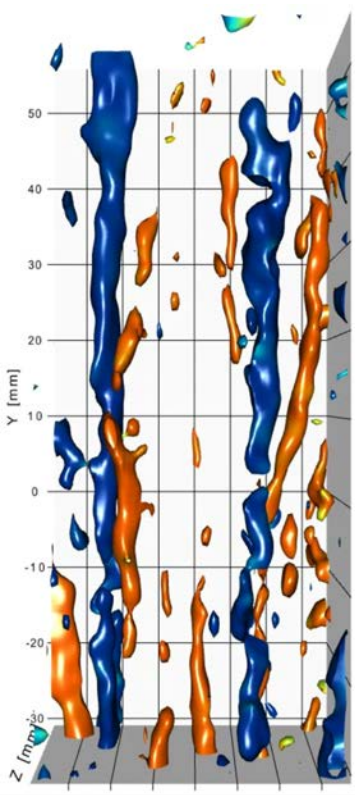

121957

626

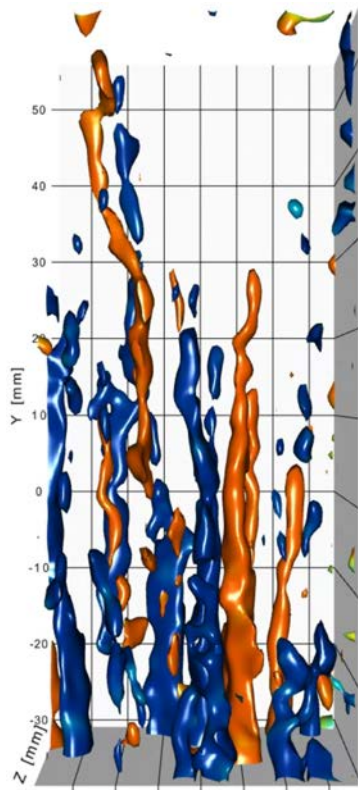

122518

627

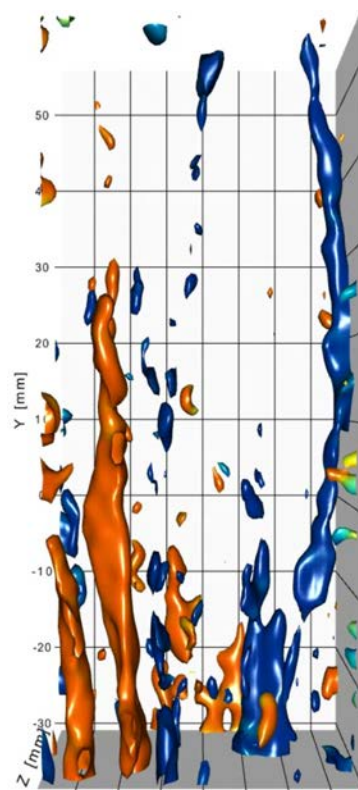

123777

628

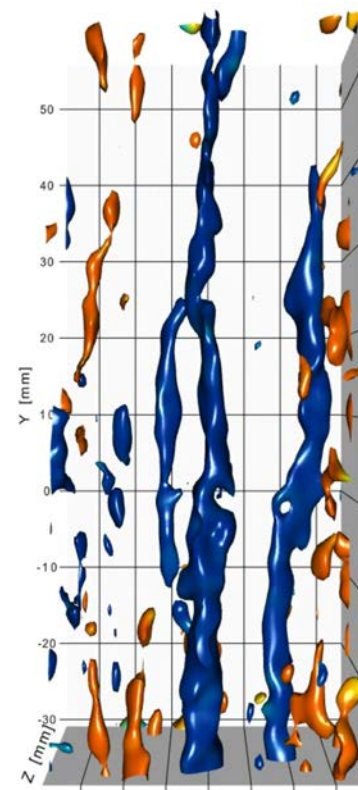

123987

629

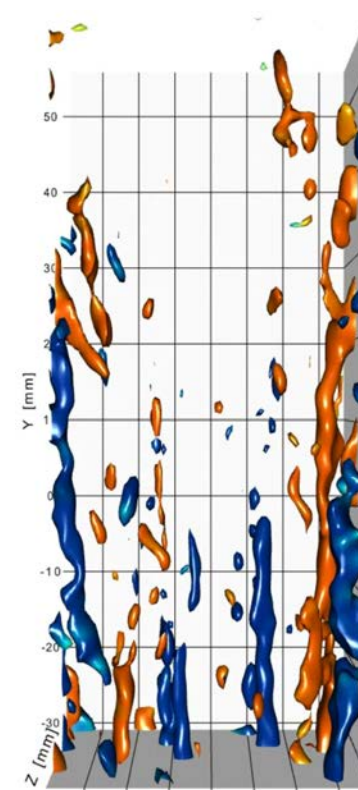

125208

630



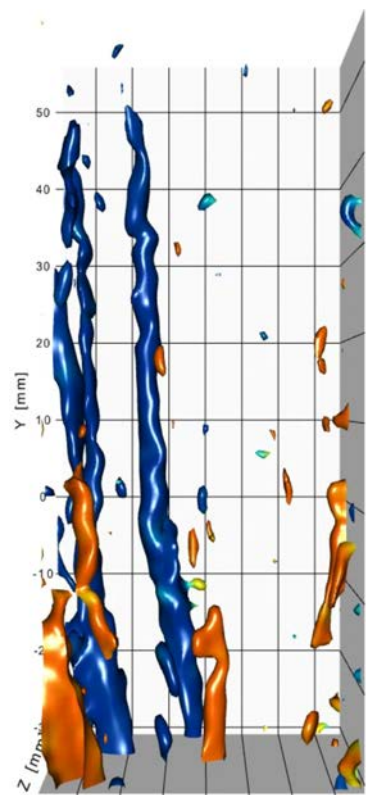

125849

631

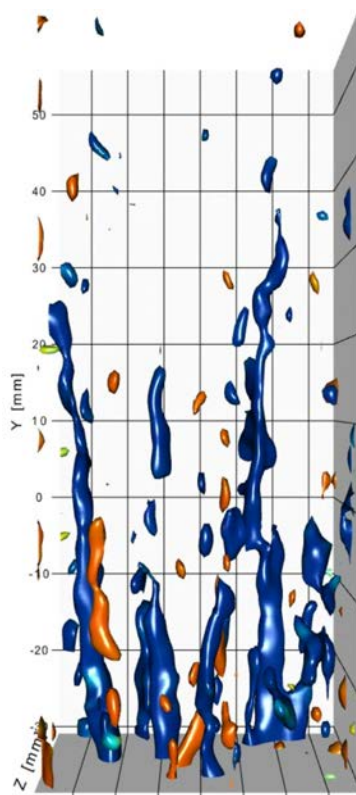

126215

632

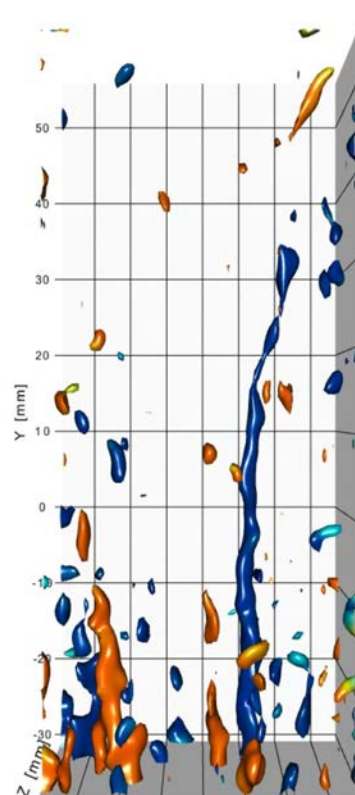

126358

633

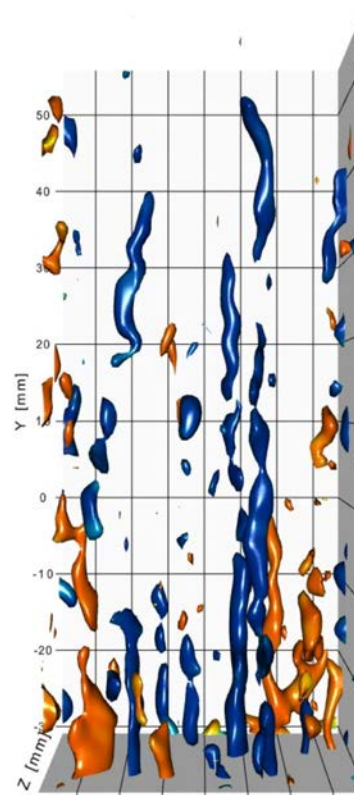

127867

634

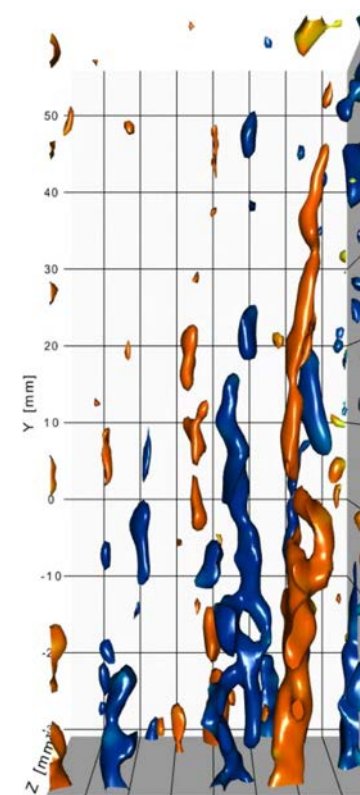

128268

635



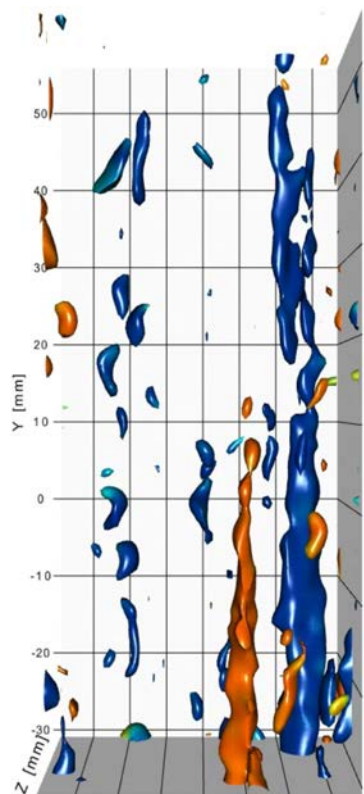

128766

636

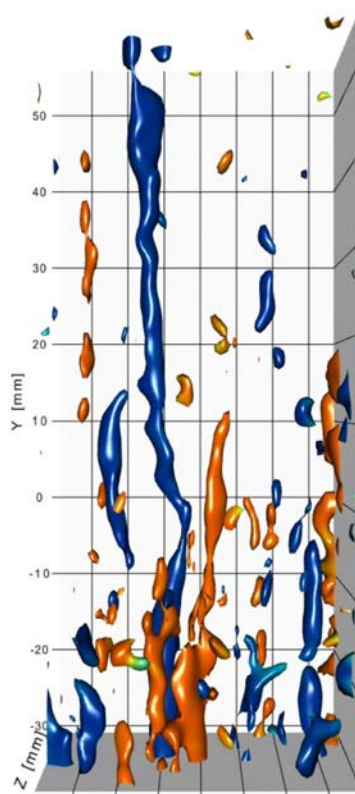

129903

637

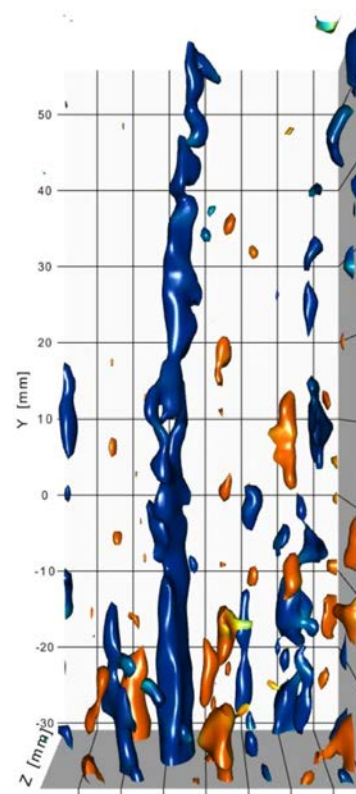

130190

638

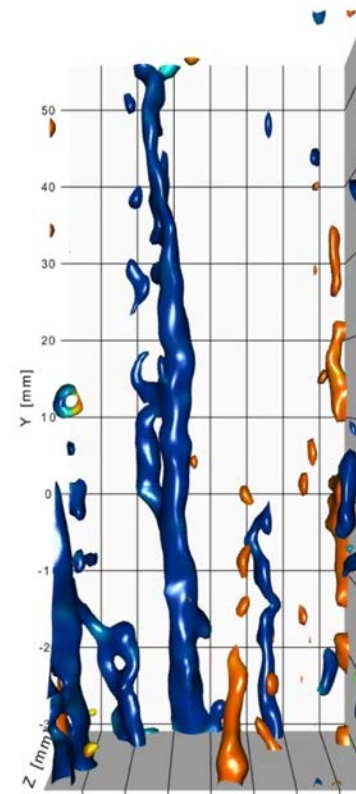

131741

639

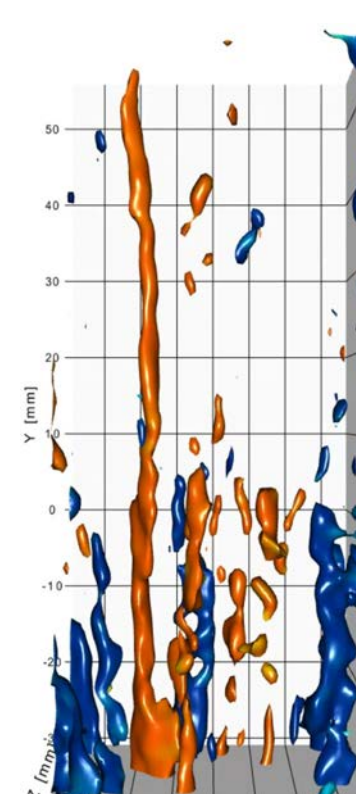

132524

640

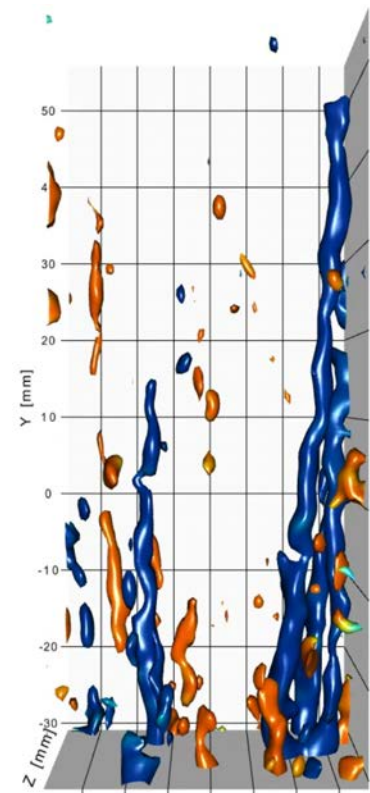

132857

641

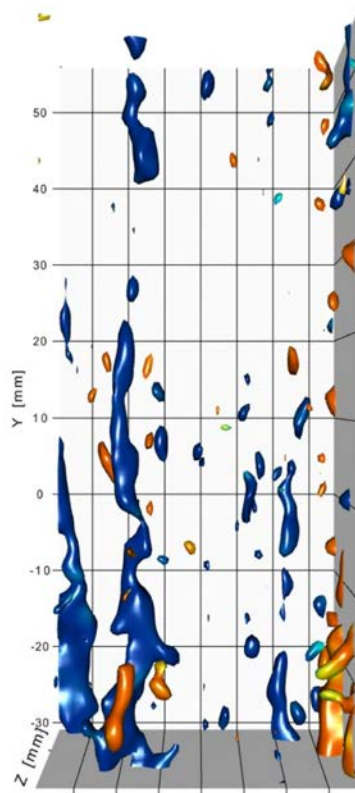

133897

642

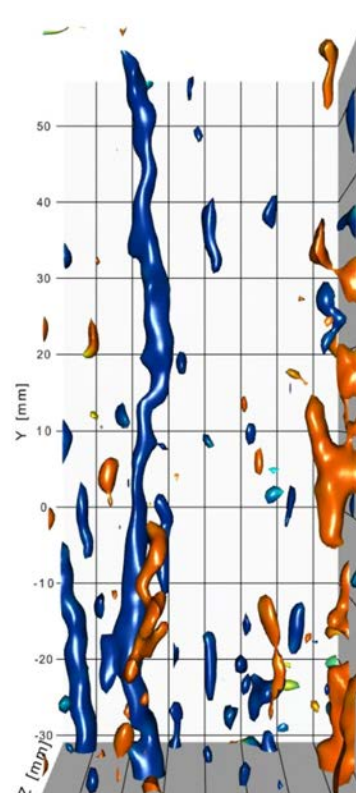

133956

643

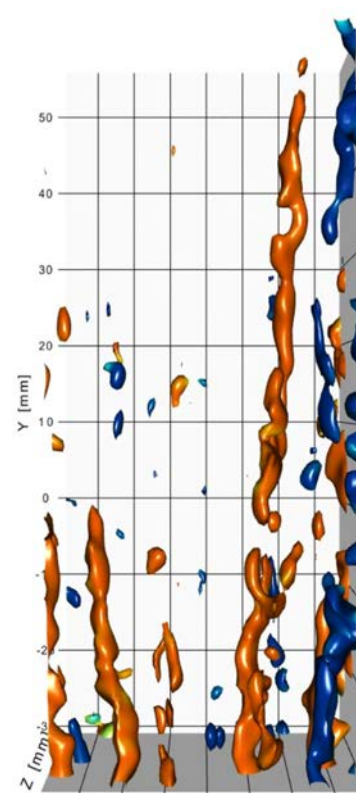

134673

644

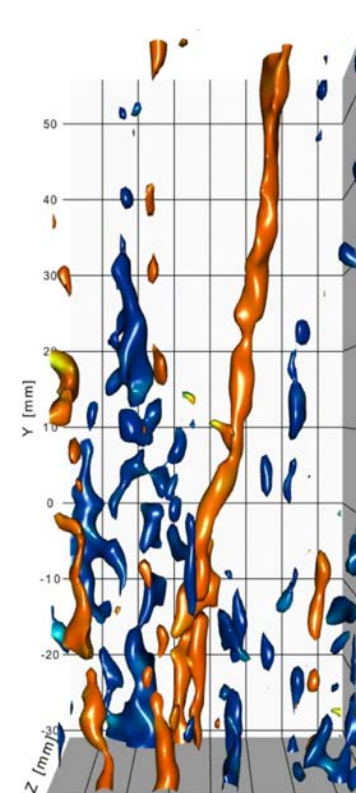

135009

645



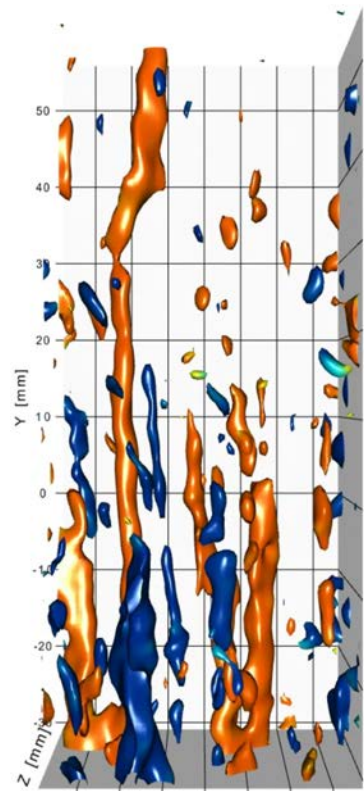

135553

646

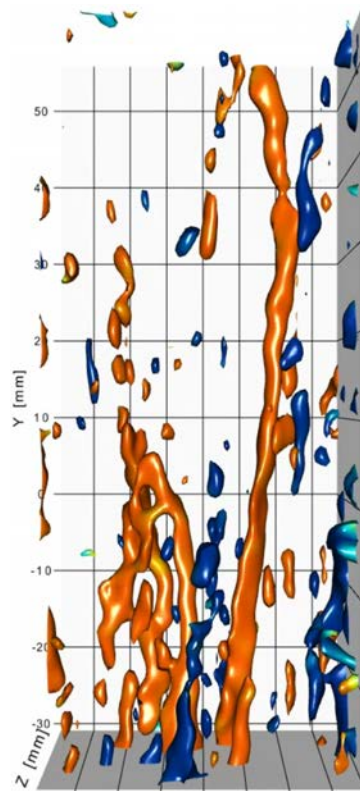

135798

647

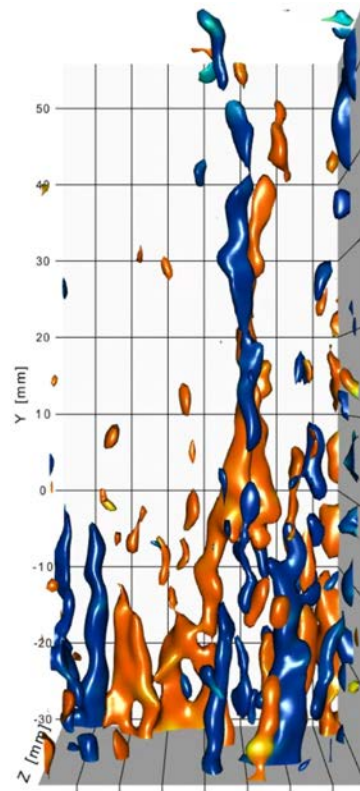

135956

648

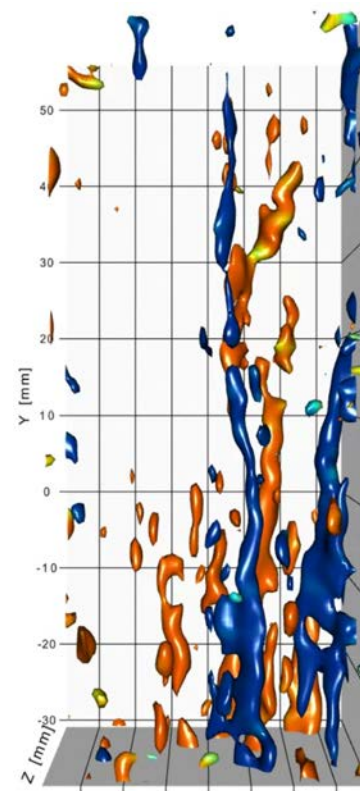

136090

649

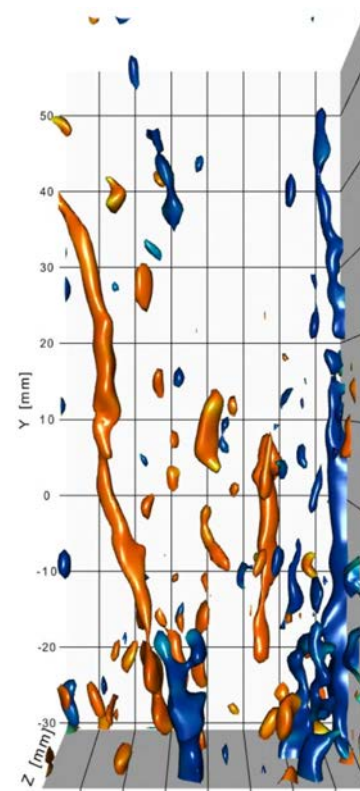

136488

650
