# Supplementary material for: Coherent turbulent structures in a rapid contraction
Source: arXiv:2401.05869 source file (2024-01-11)
Supplement: Supplementary file 5 [file StrRun5.pdf]

# Run5

Iso-surface of  $|\omega| = 40 \text{ } ^1/s$

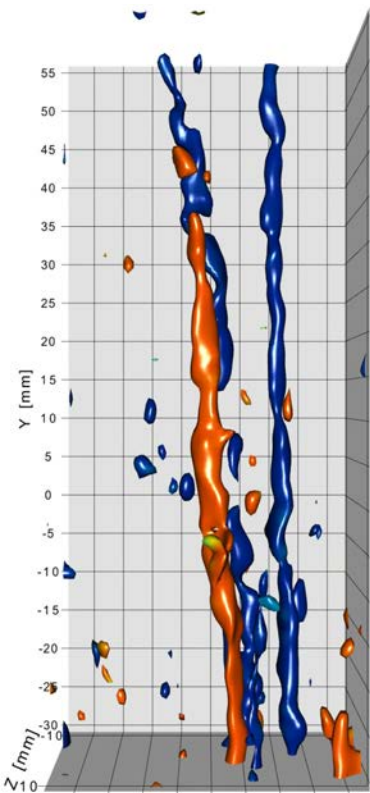

534

651

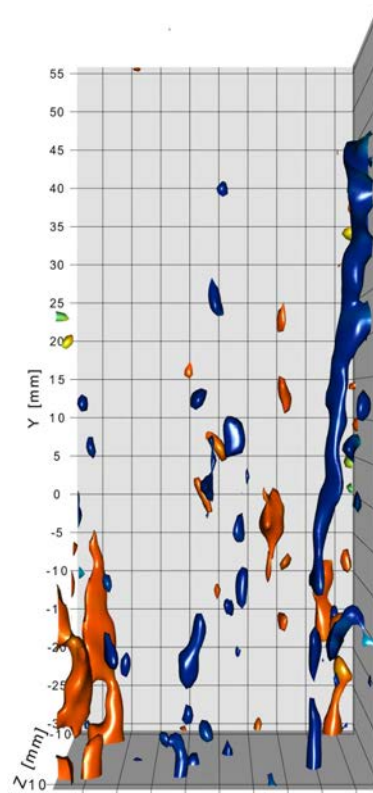

1839

652

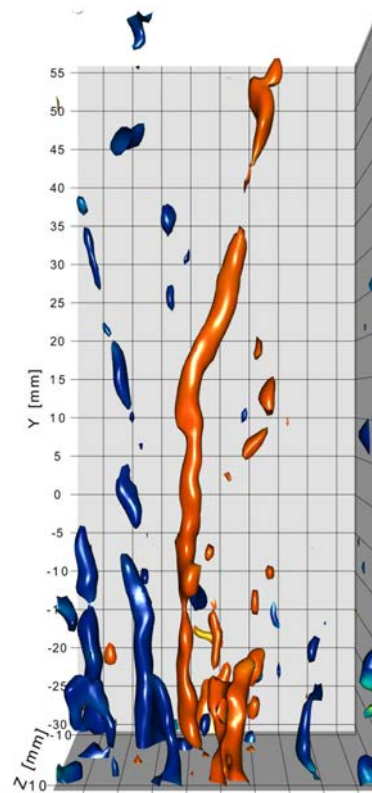

3663

653

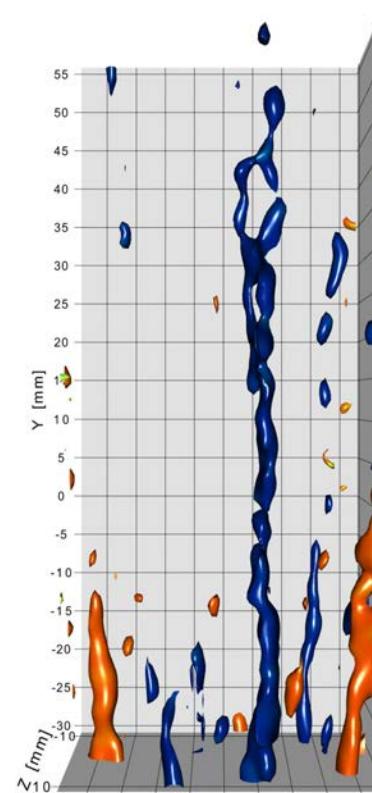

4827

654

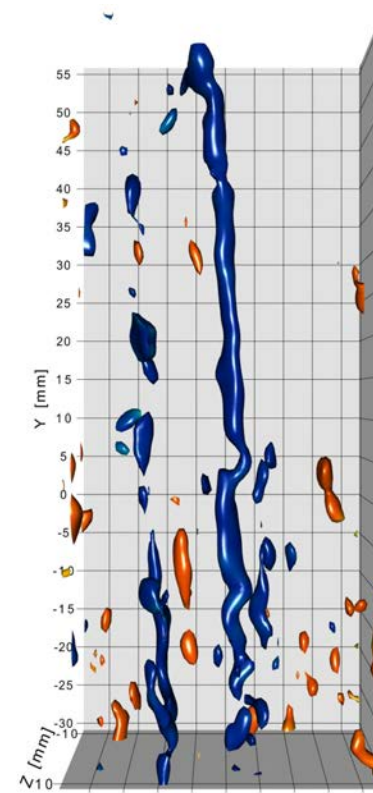

5062

655

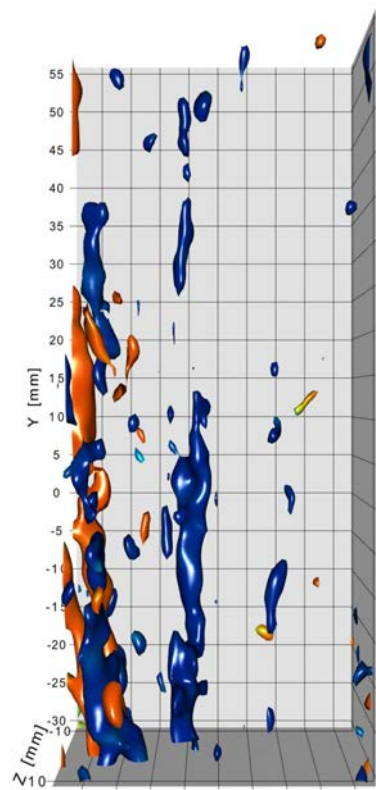

5495

656

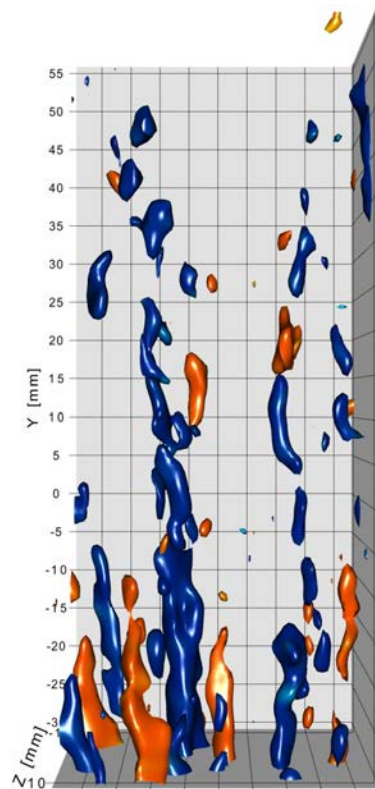

5808

657

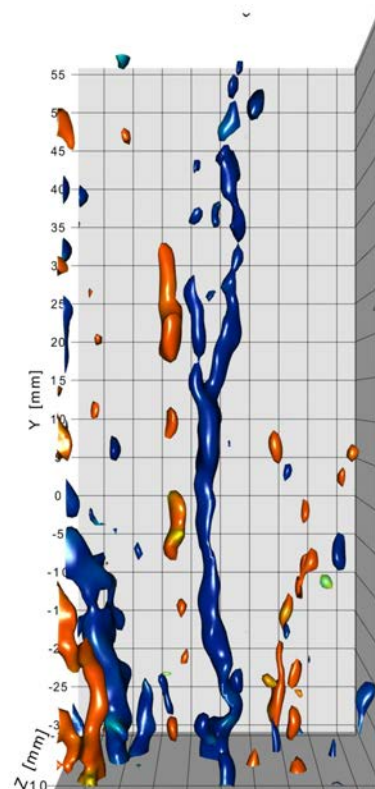

8988

658

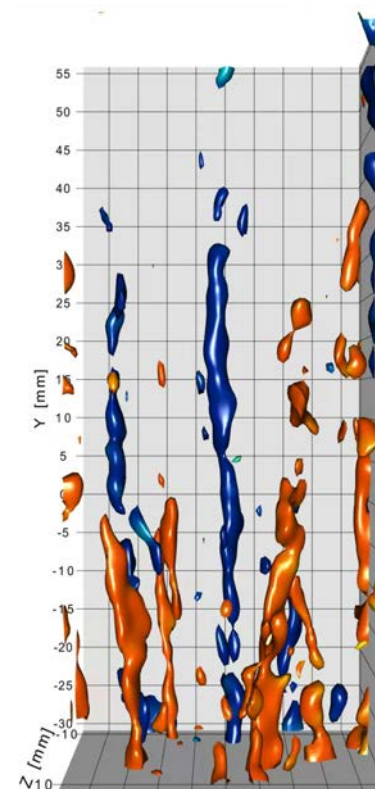

10263

659

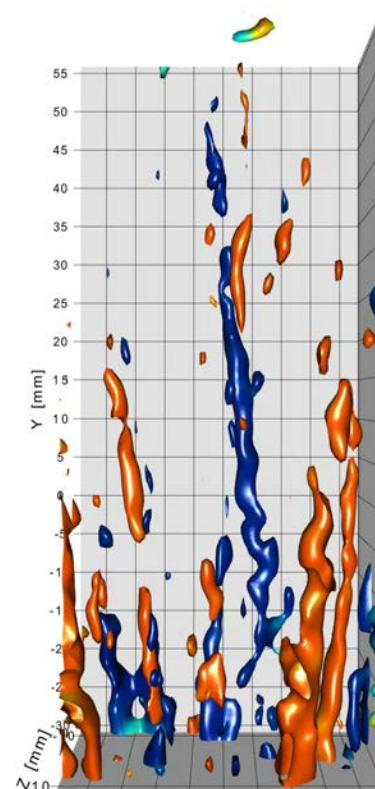

10480

660

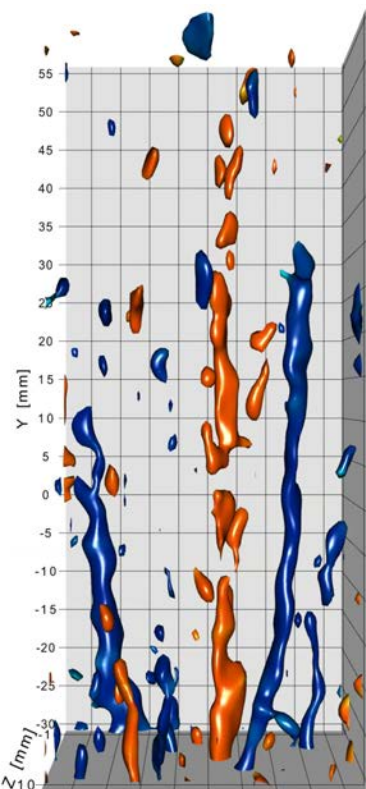

10864

661

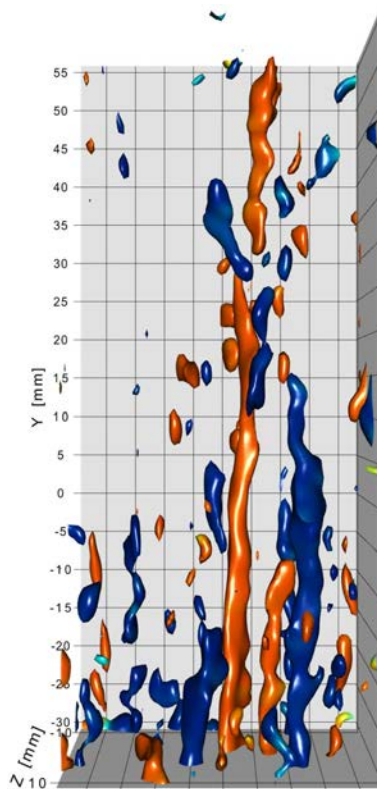

10947

662

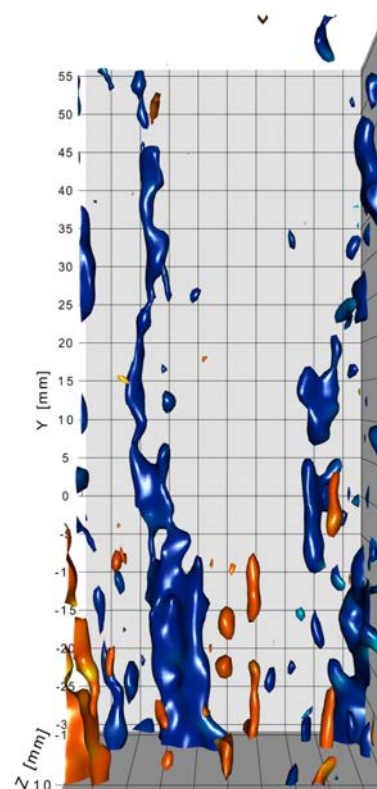

11902

663

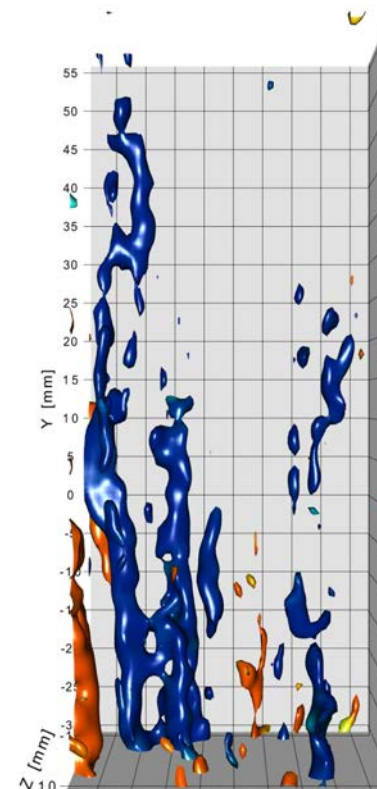

12093

664

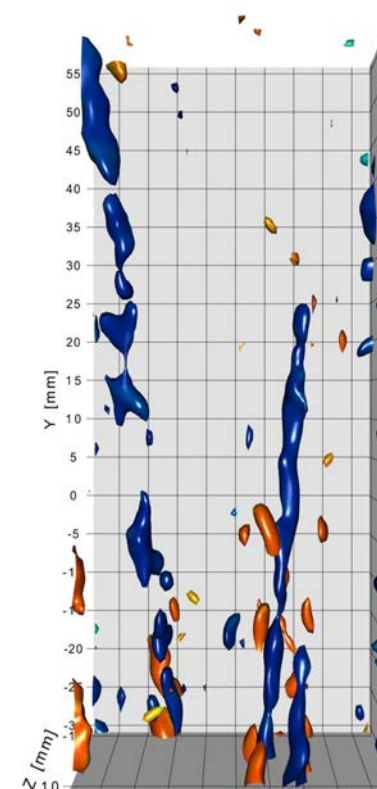

14191

665



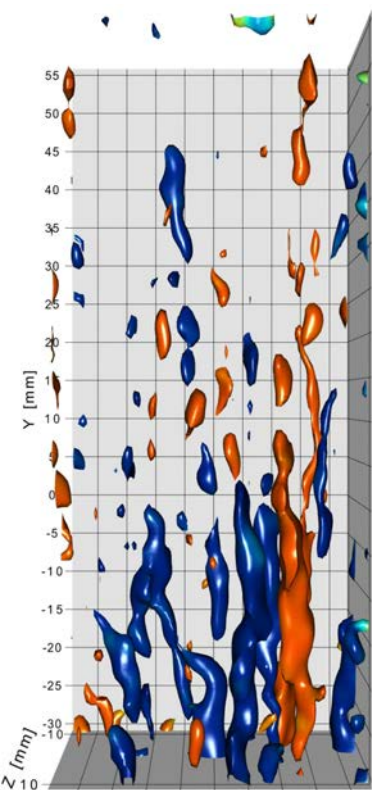

15761

666

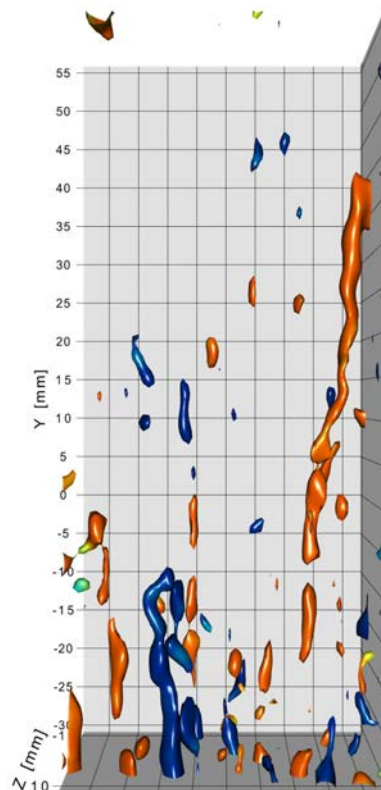

16012

667

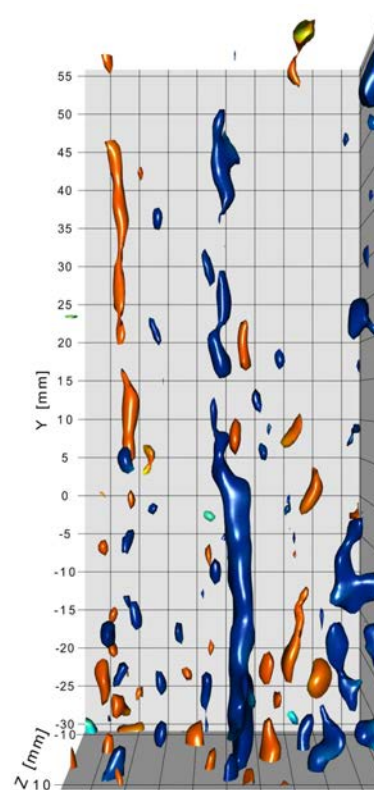

17999

668

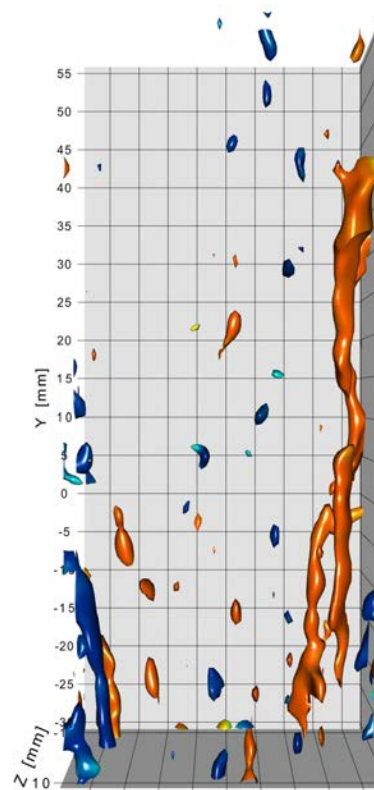

19147

669

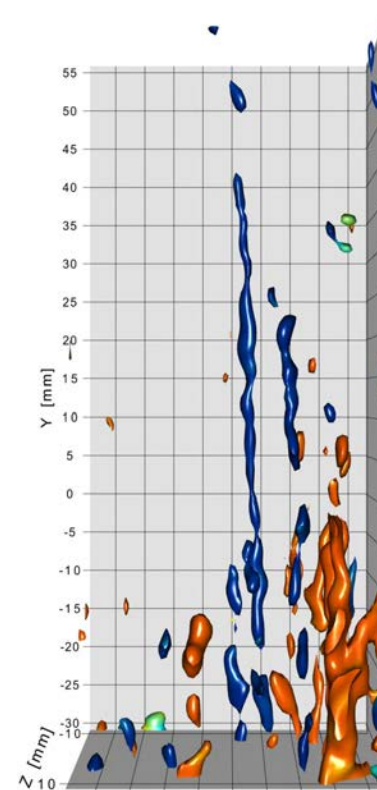

19376

670

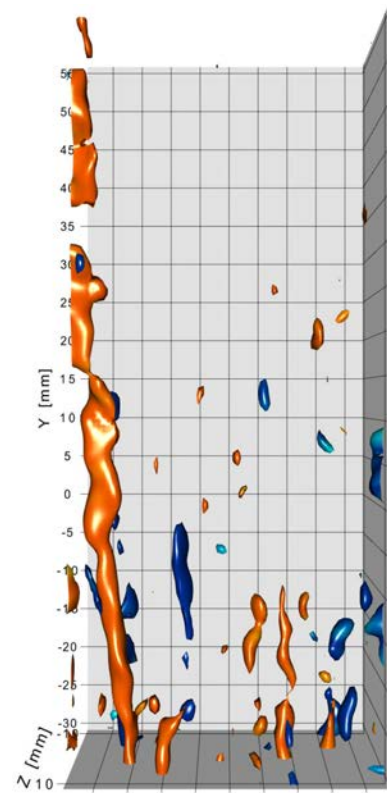

19899

671

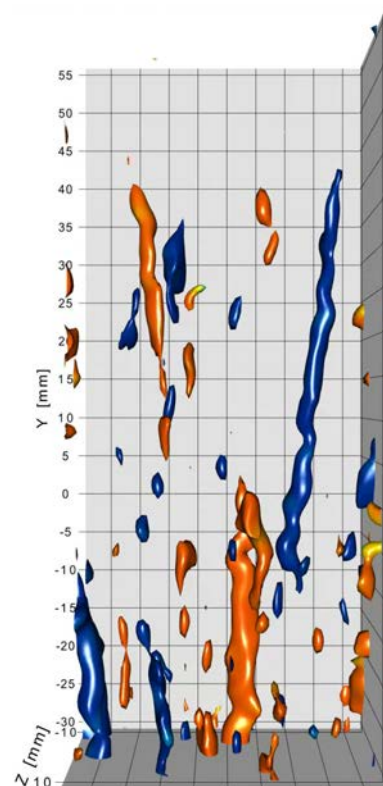

20659

672

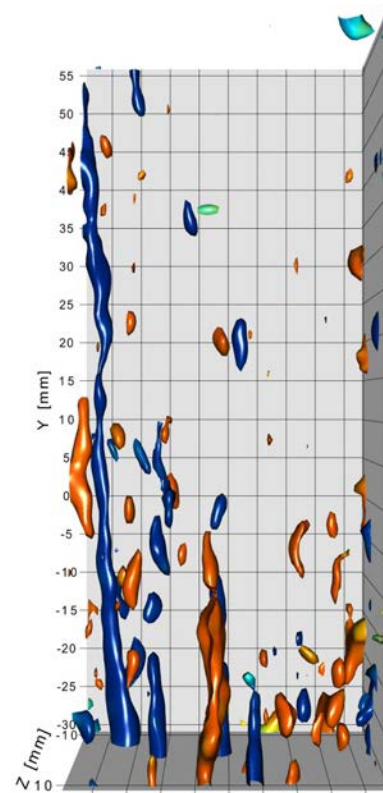

21624

673

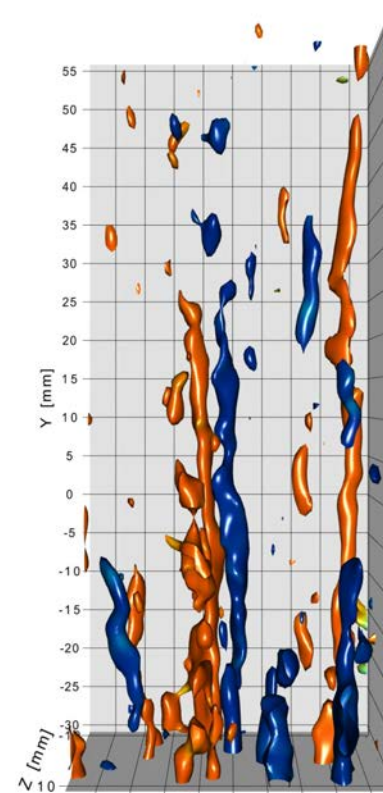

22940

674

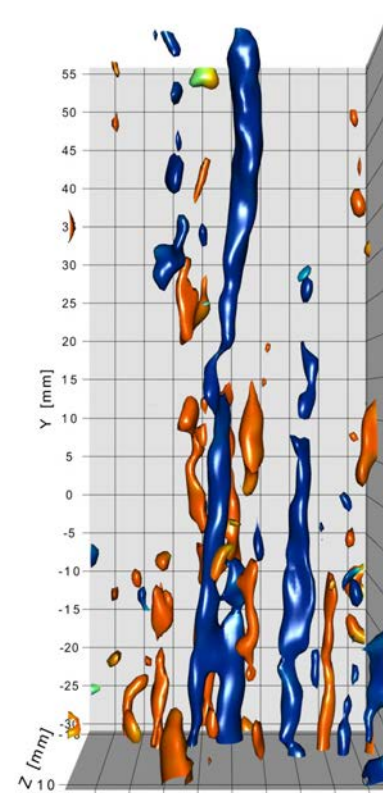

23174

675

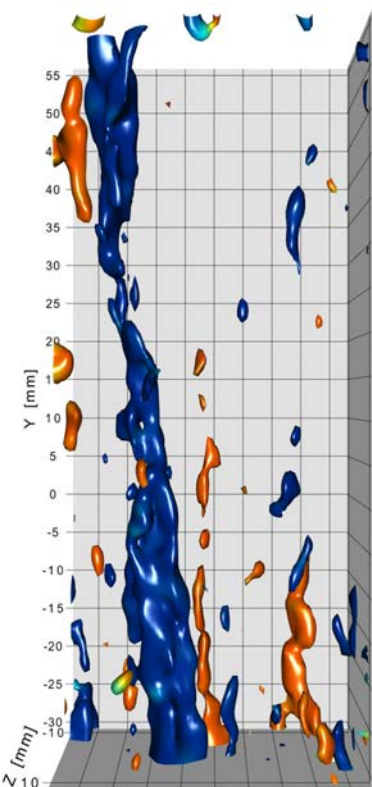

23603

676

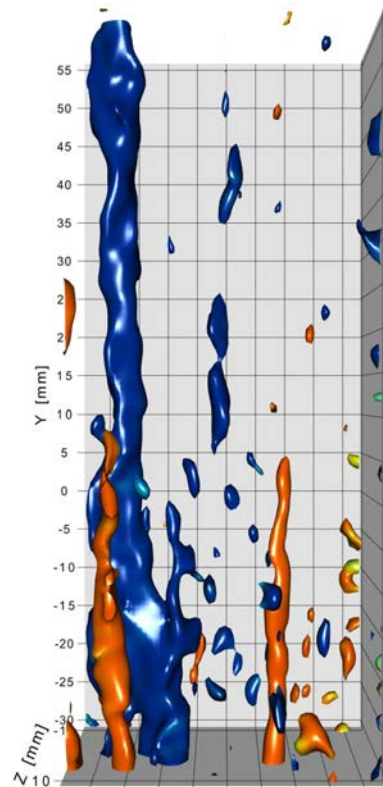

23866

677

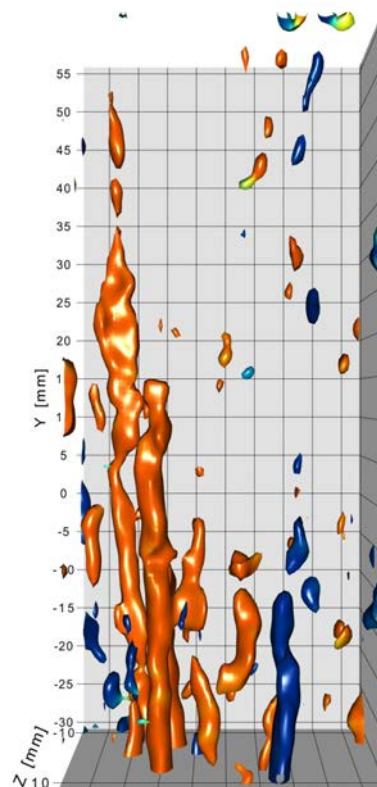

25279

678

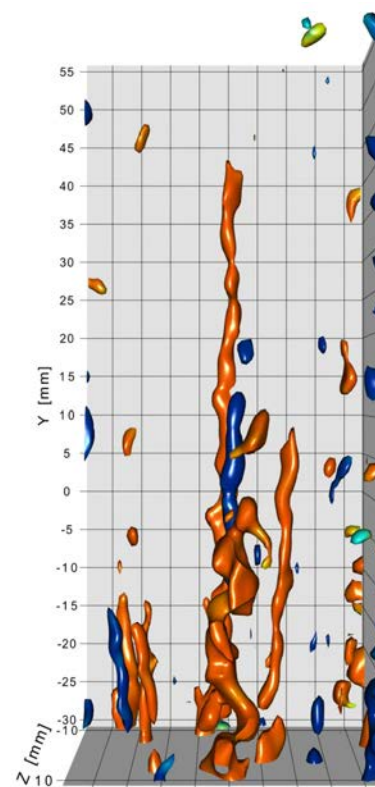

25585

679

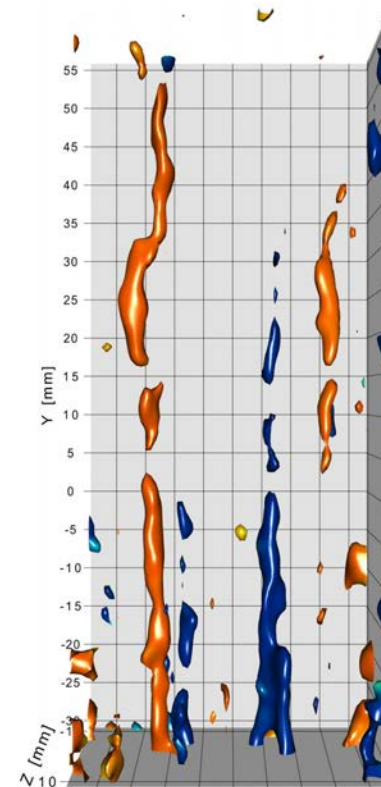

26749

680



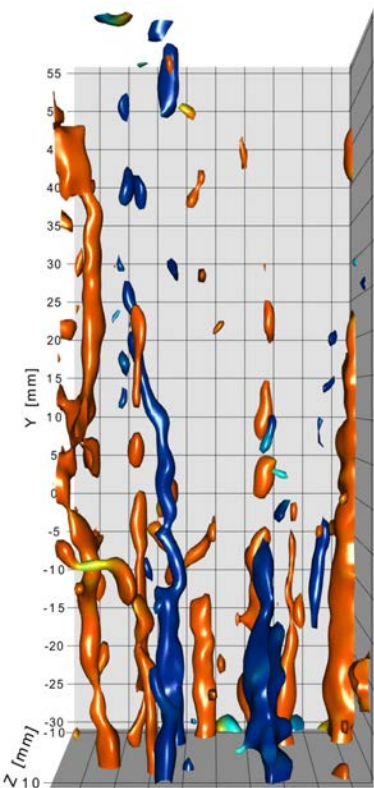

27045

681

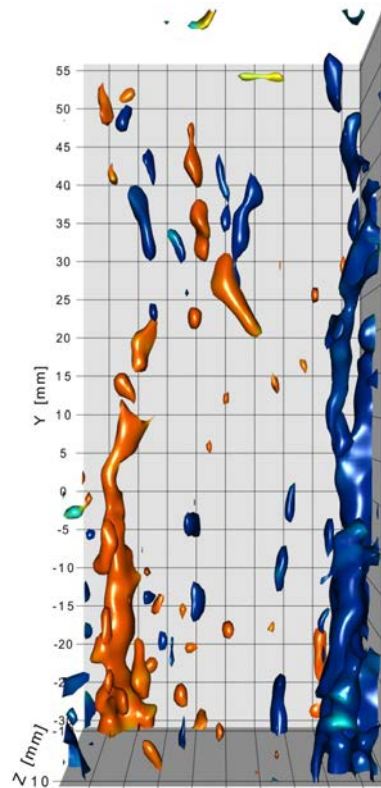

27817

682

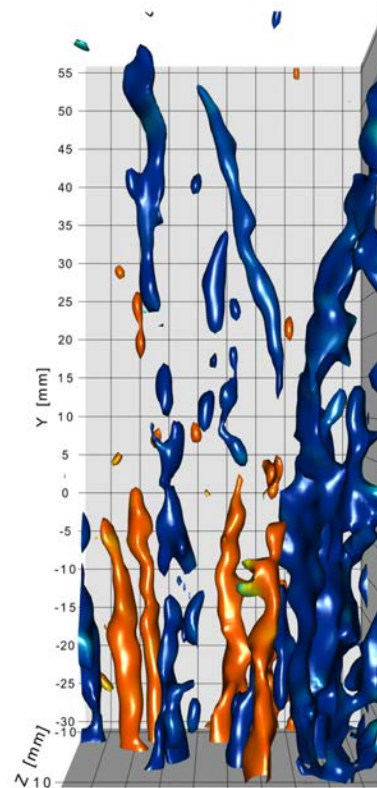

28029

683

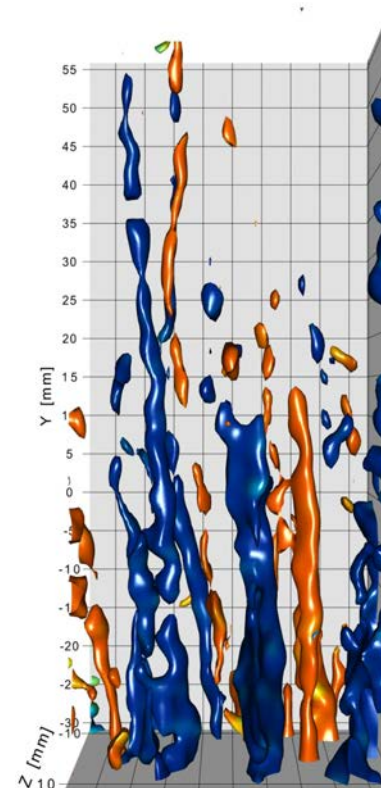

28385

684

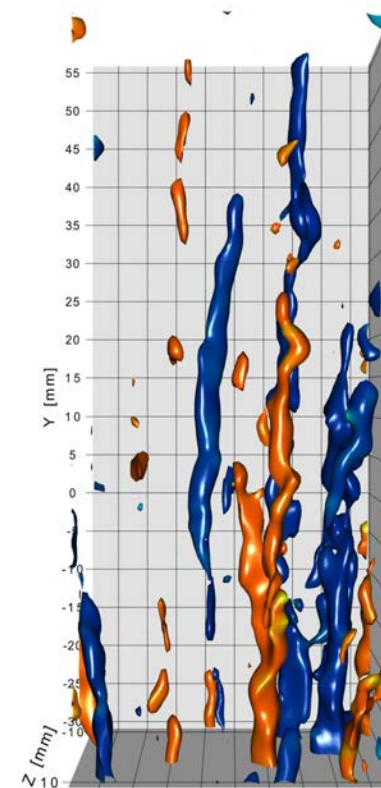

28885

685



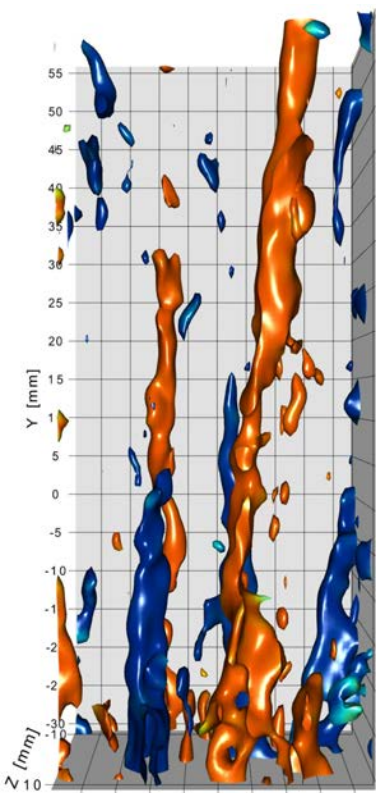

29876

686

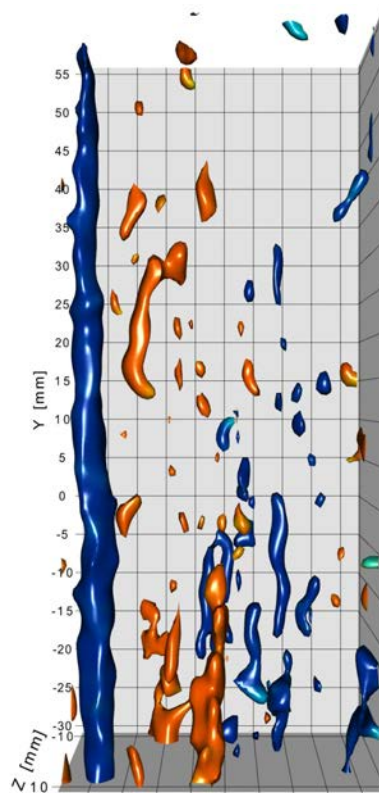

31212

687

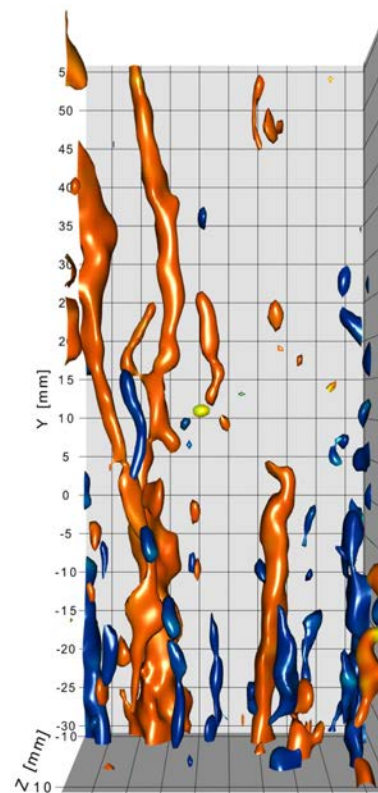

32639

688

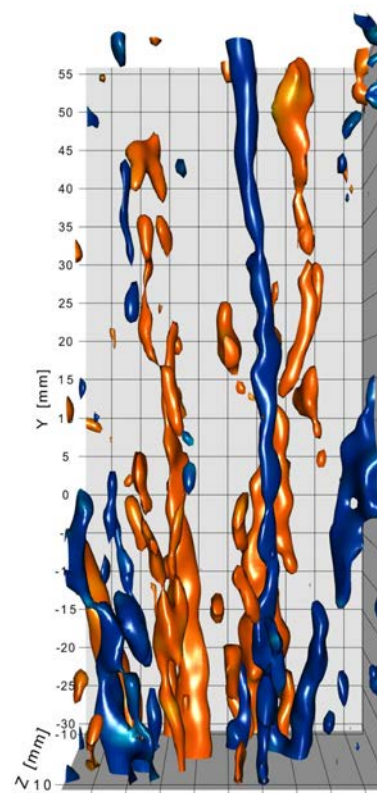

33220

689

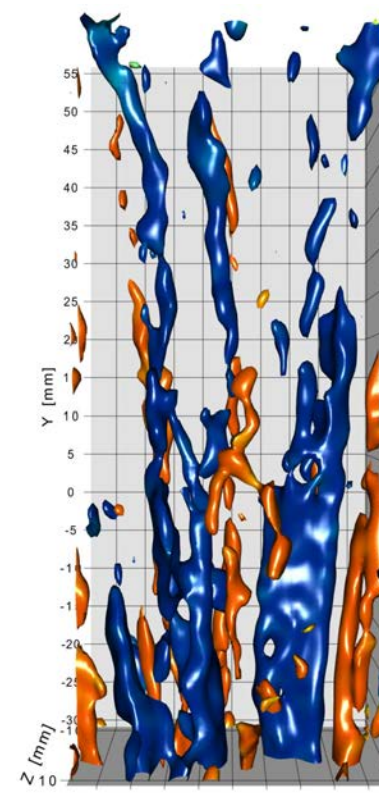

33840

690

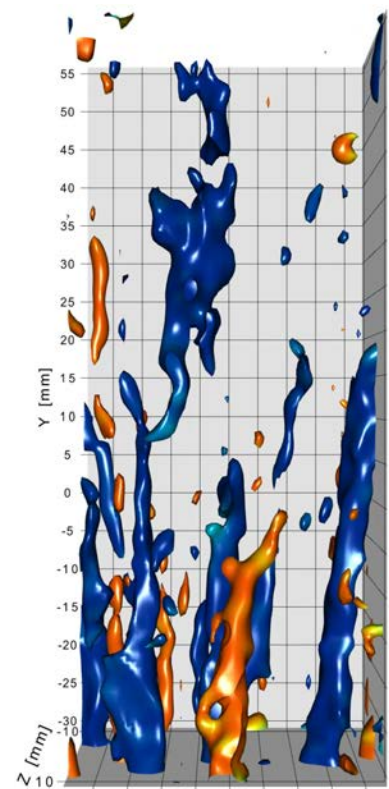

34131

691

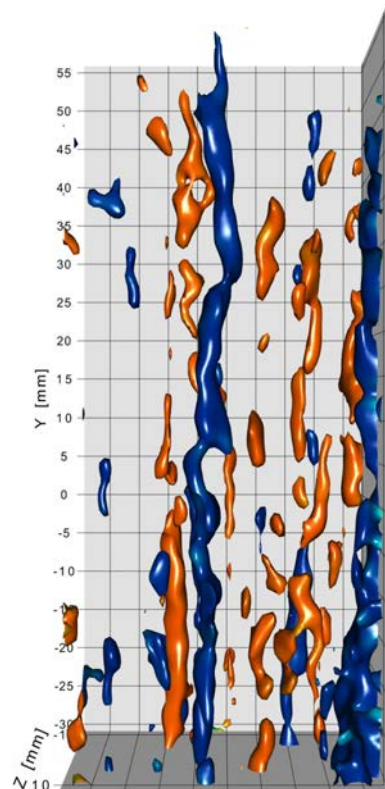

35238

692

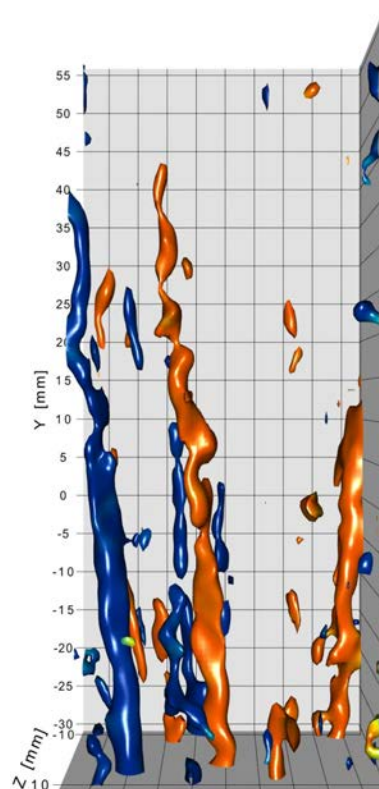

36503

693

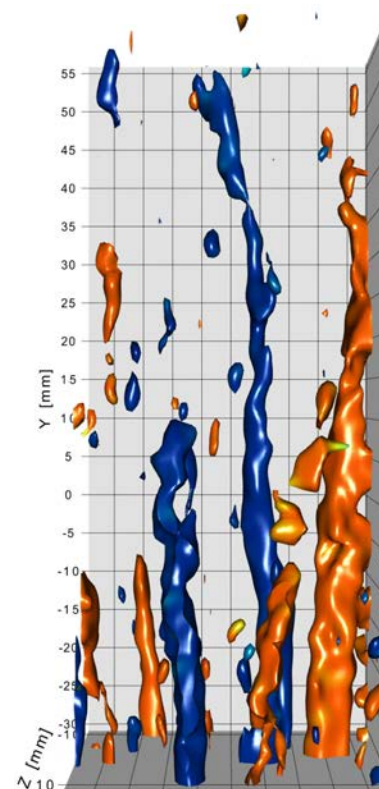

39286

694

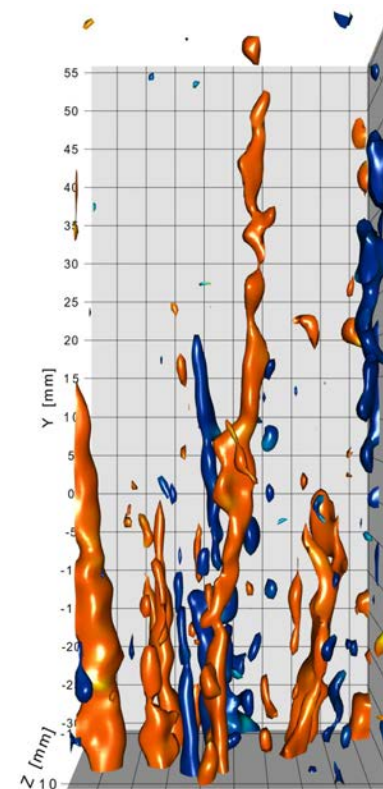

39781

695



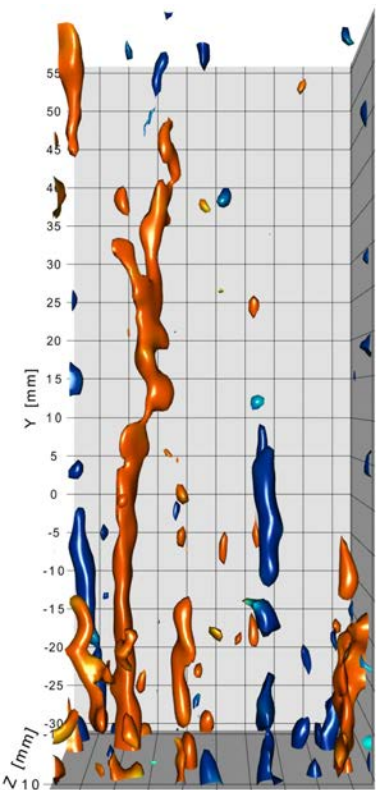

41542

696

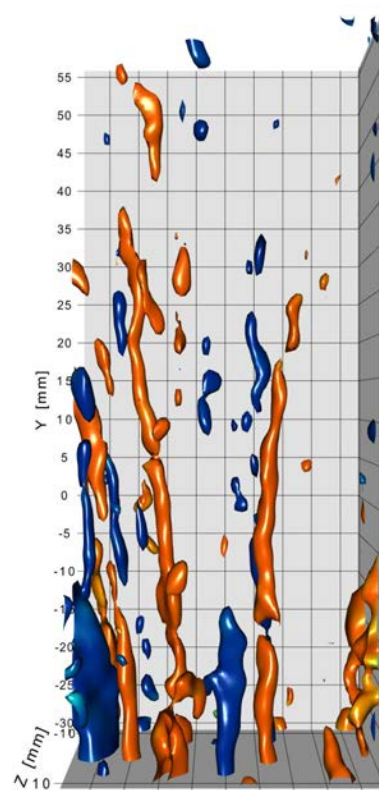

42542

697

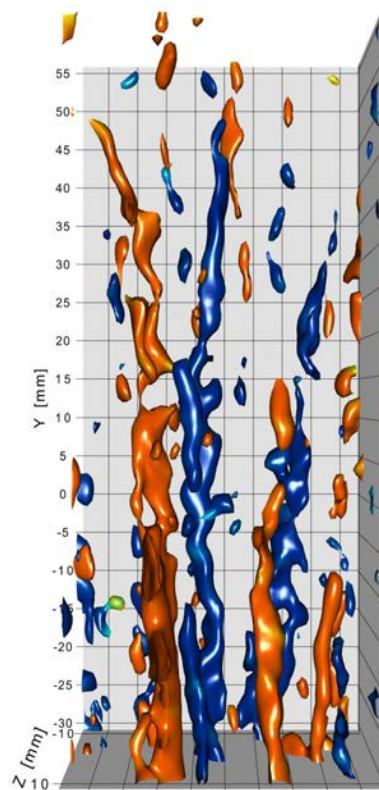

42731

698

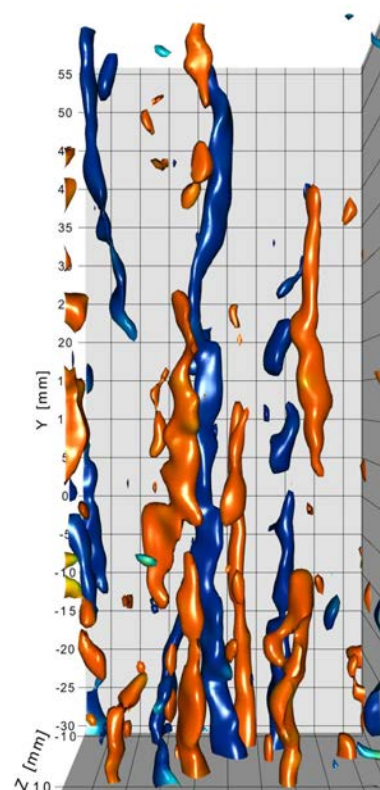

42971

699

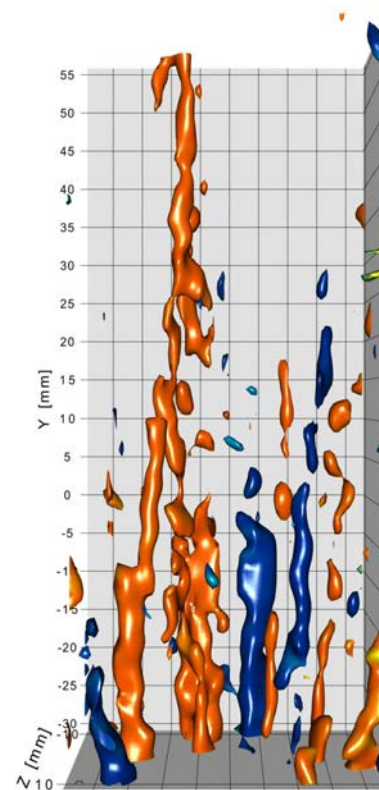

45225

700



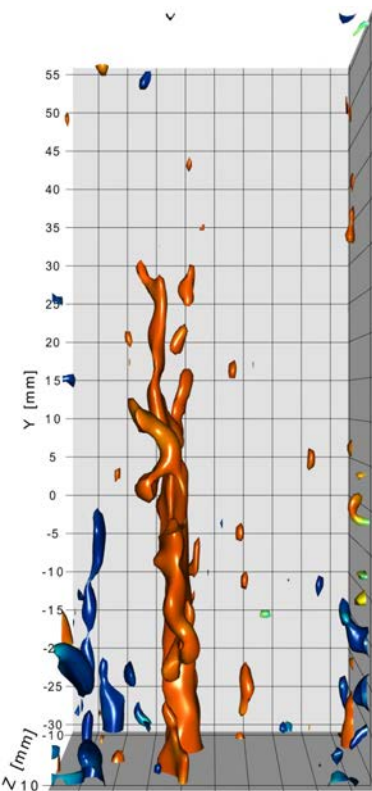

45488

701

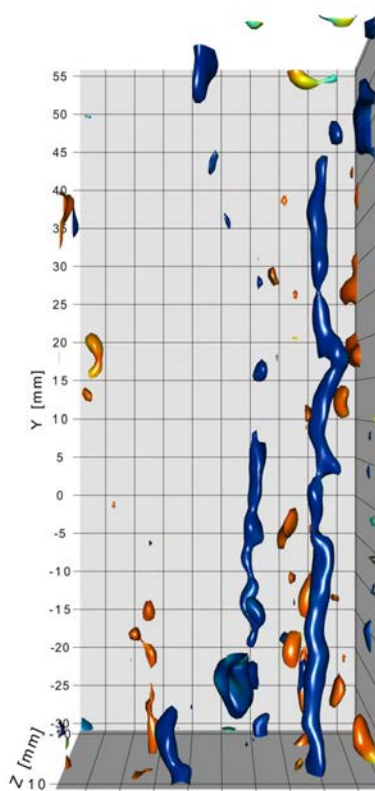

46699

702

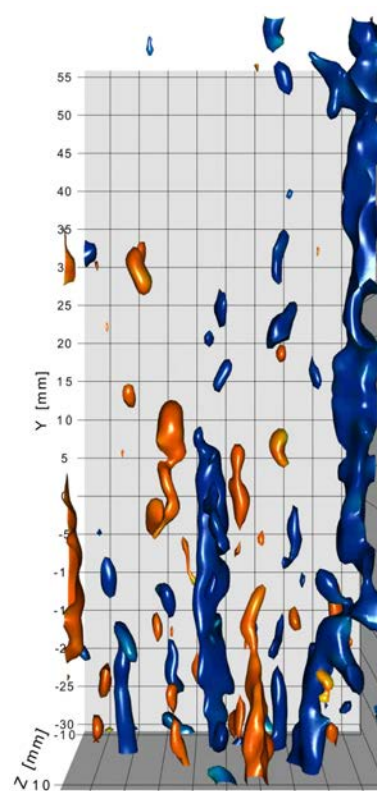

46886

703

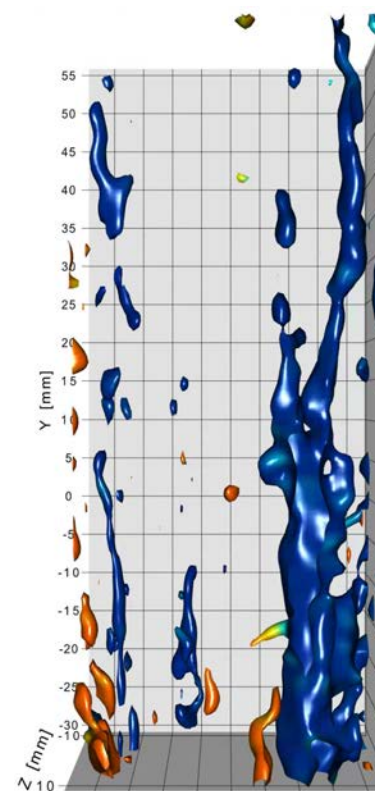

47194

704

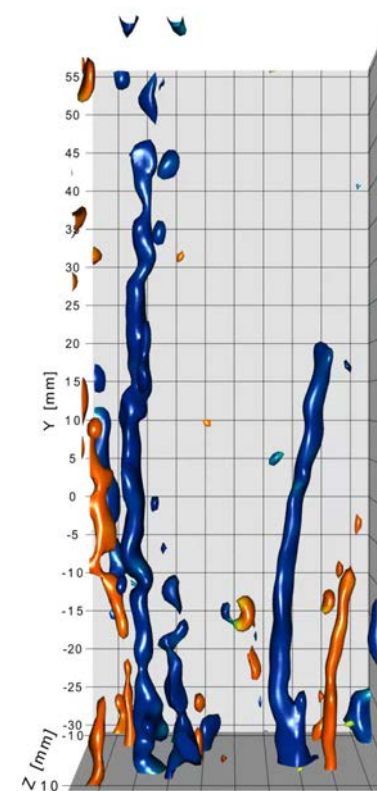

47614

705

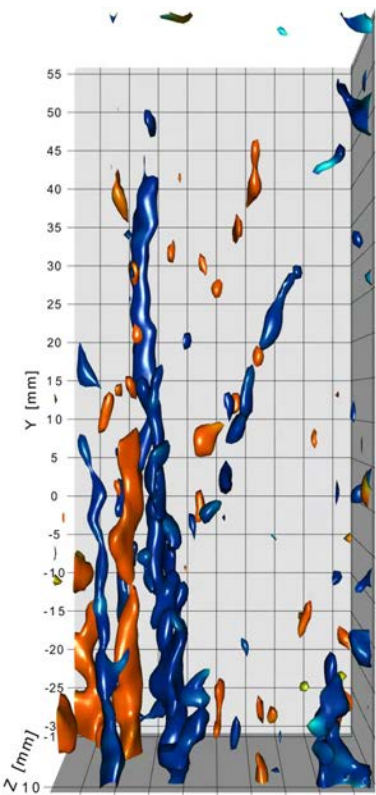

47822

706

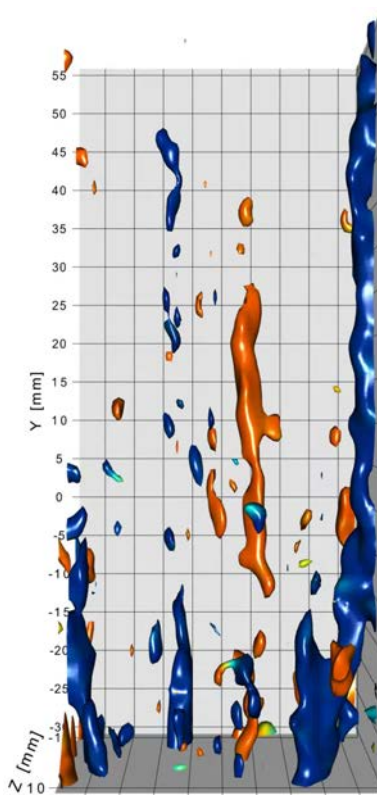

48039

707

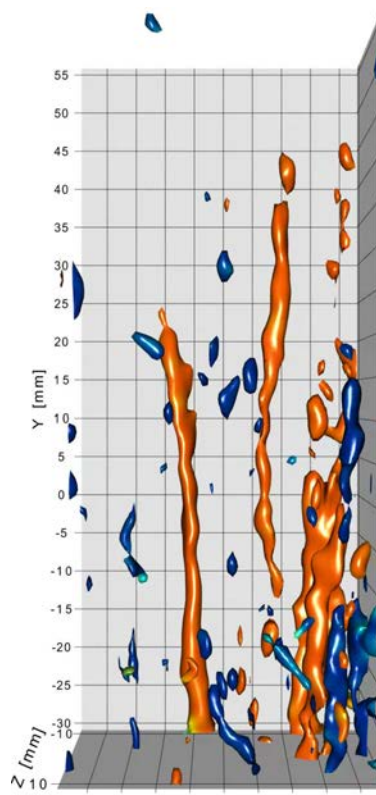

48310

708

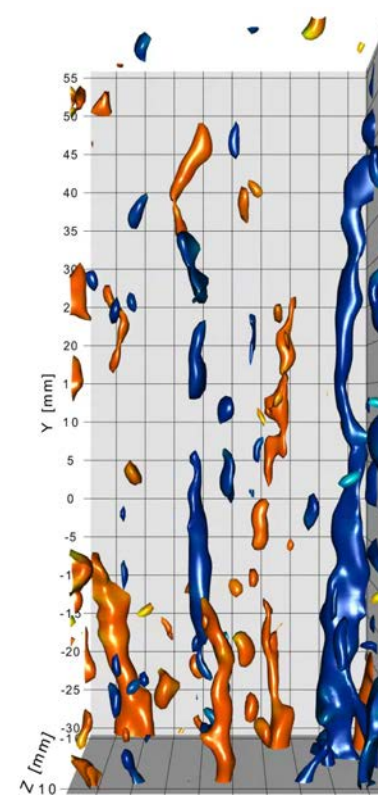

50742

709

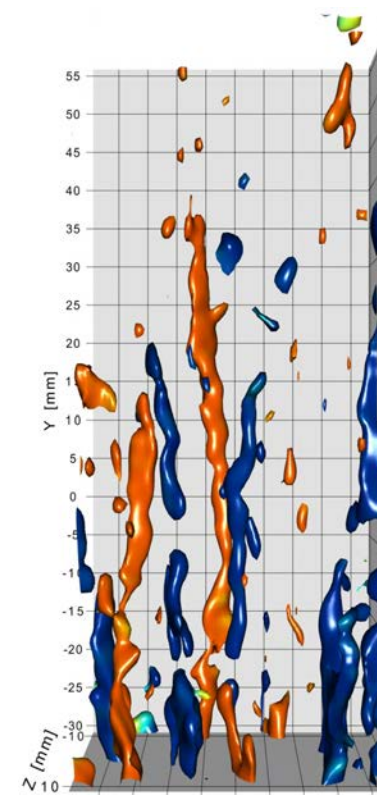

50921

710



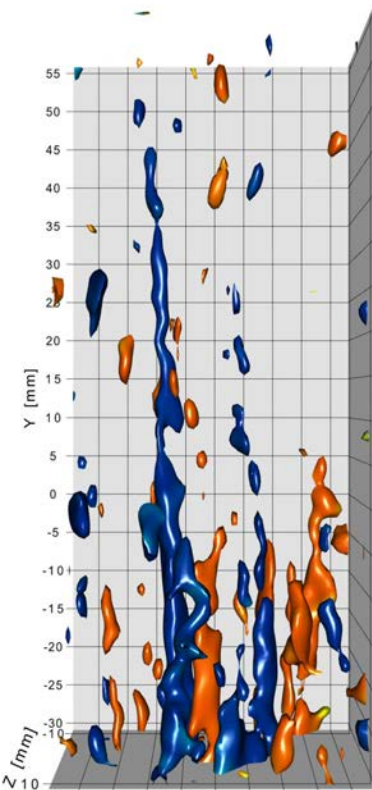

51372

711

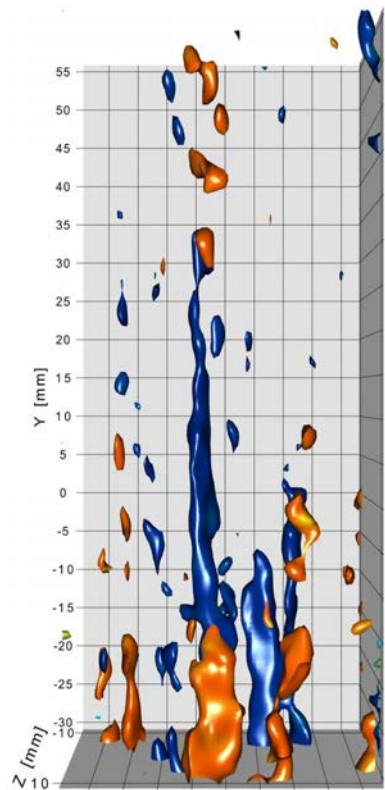

52519

712

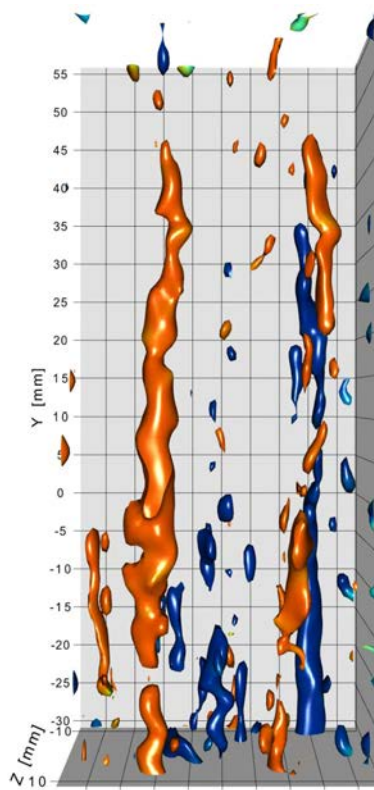

52825

713

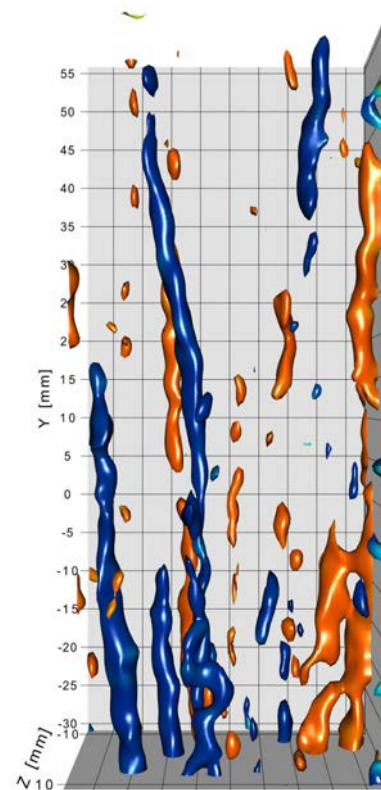

53343

714

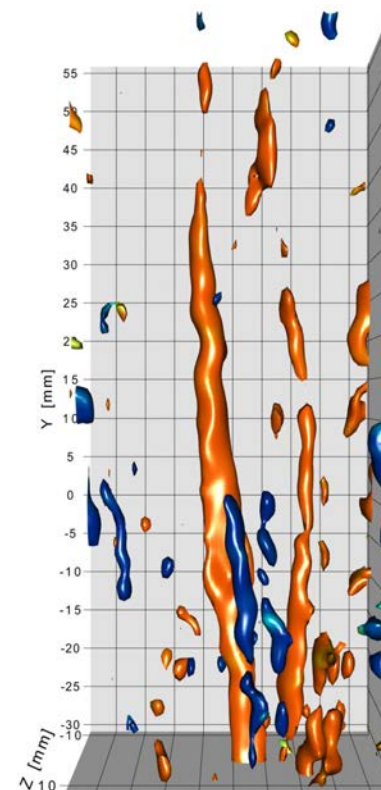

54356

715



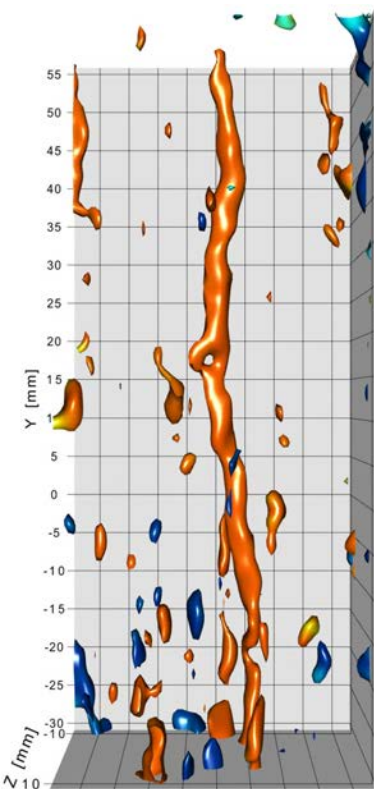

55412

716

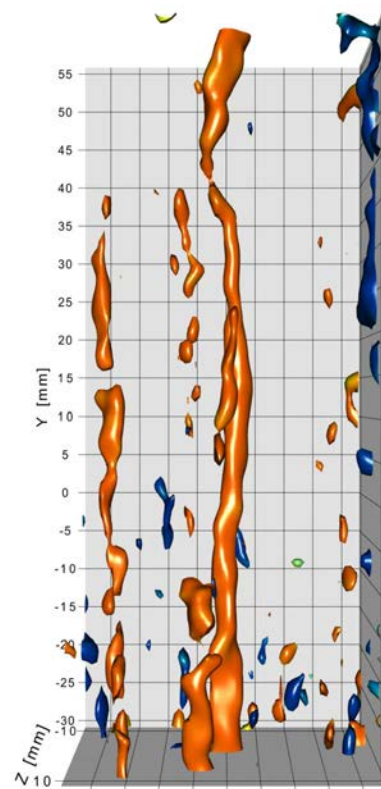

55502

717

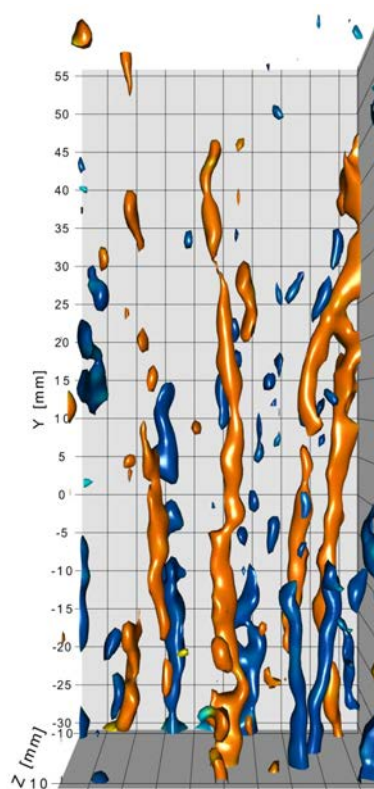

55761

718

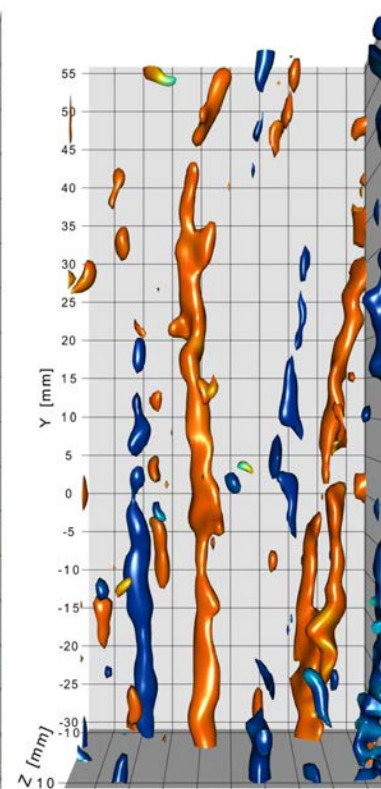

58784

719

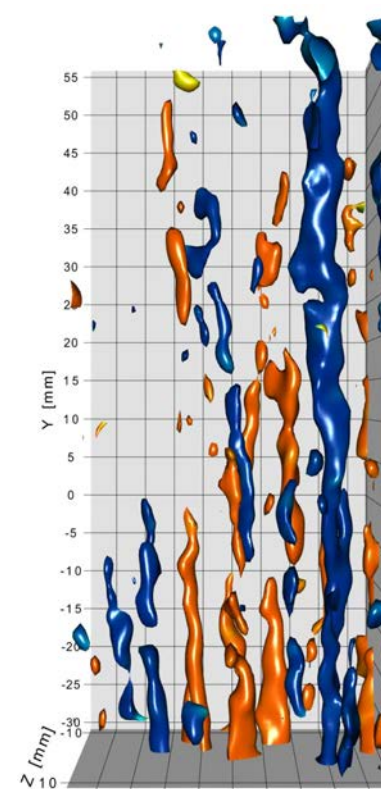

59097

720

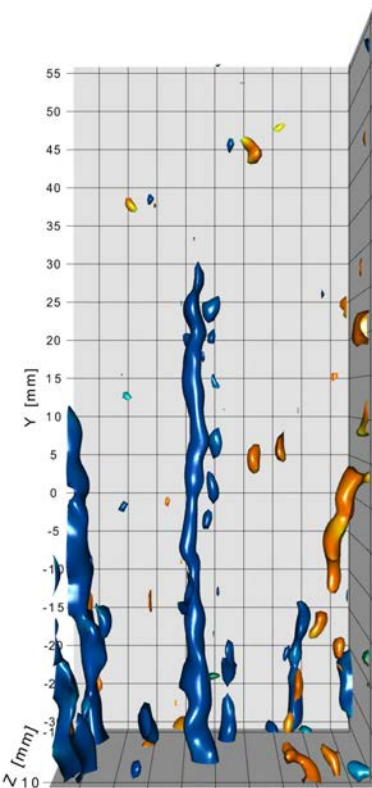

60843

721

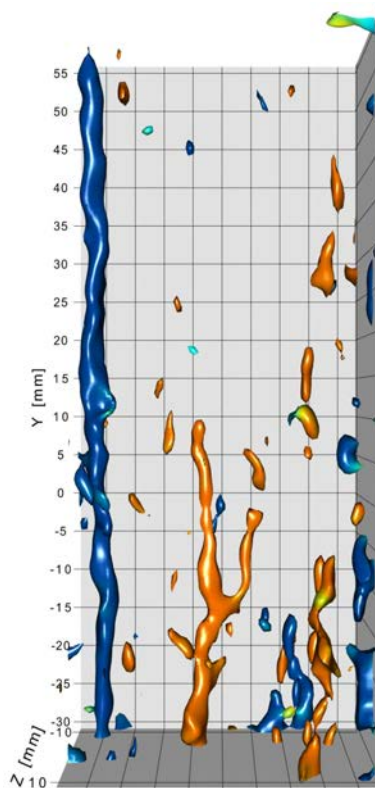

62289

722

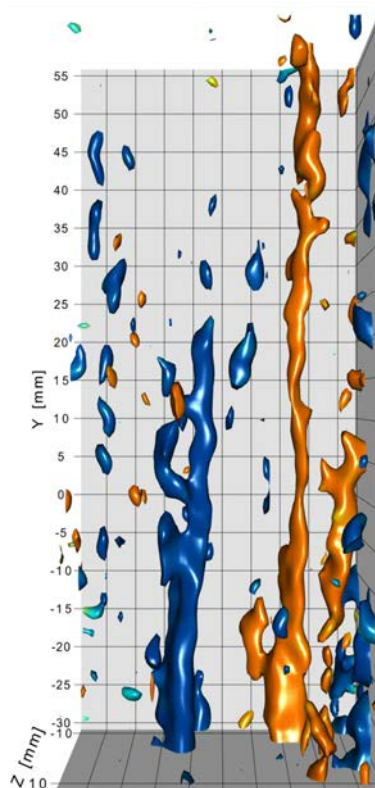

62670

723

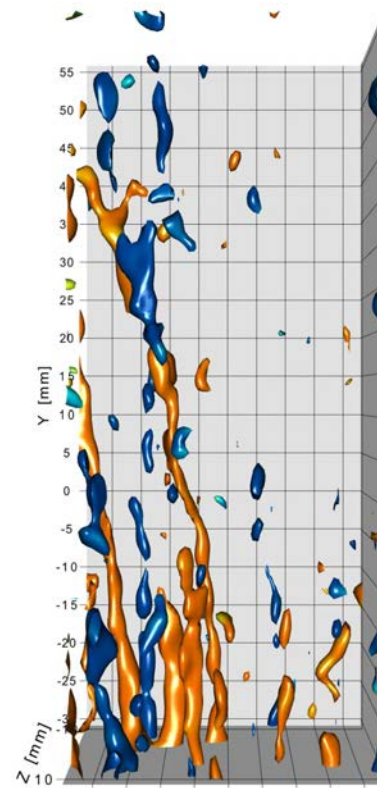

65154

724

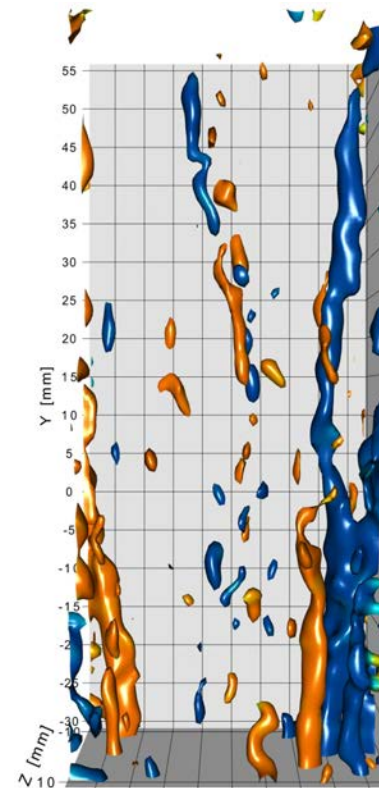

66816

725



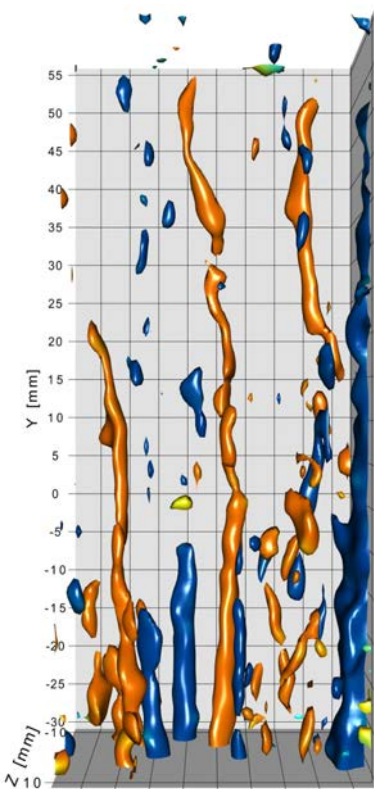

67106

726

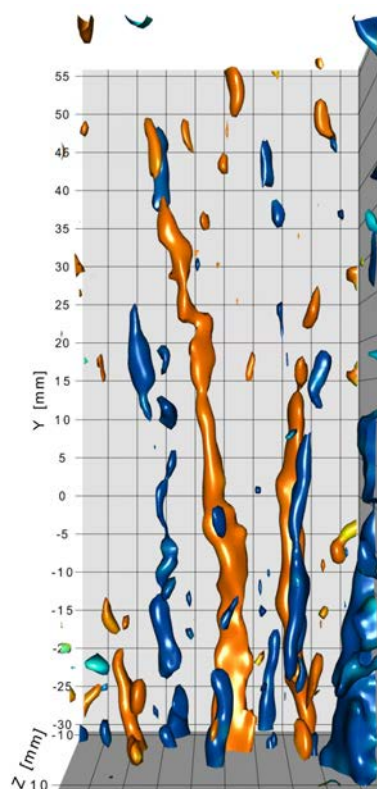

67227

727

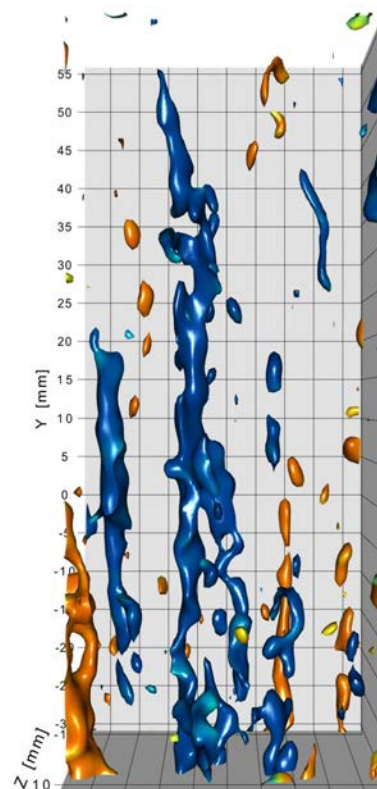

68404

728

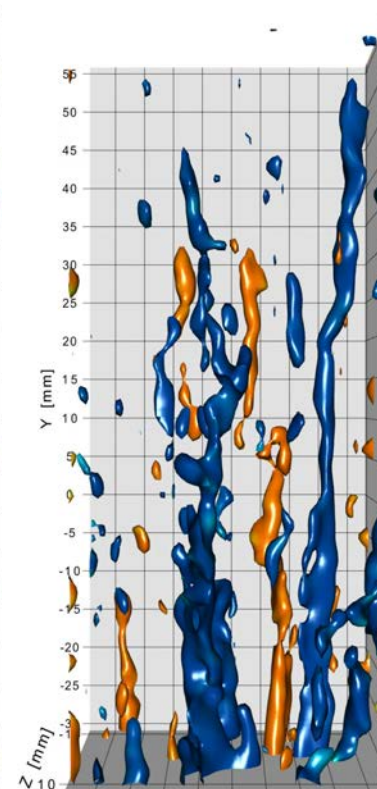

68626

729

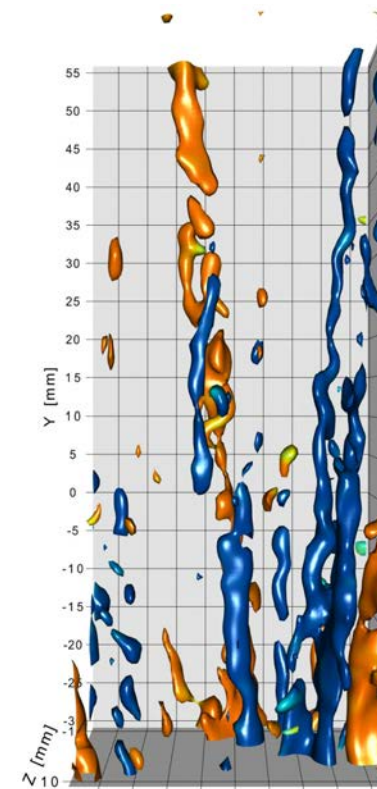

68980

730



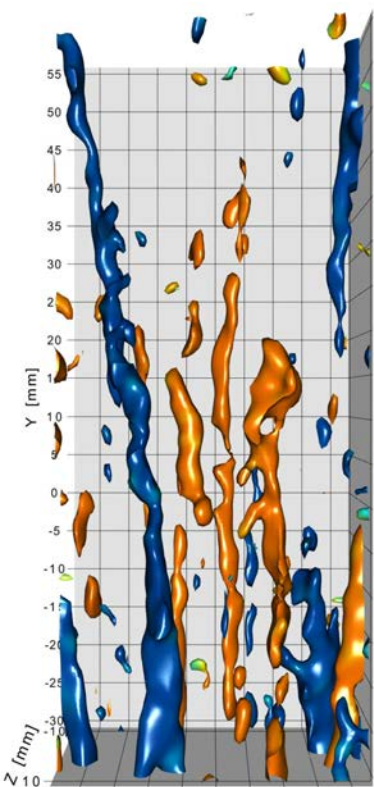

69517

731

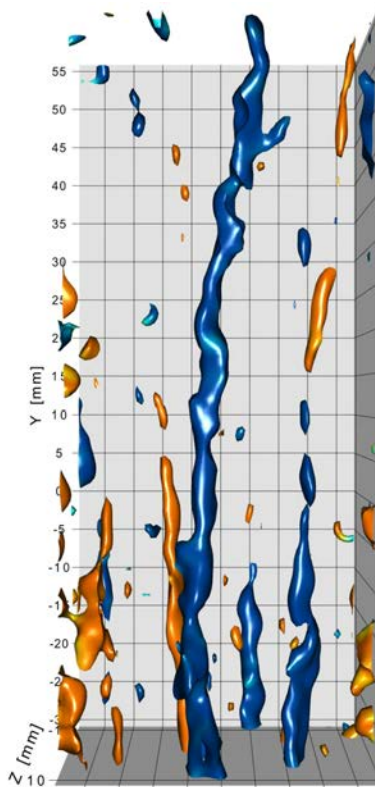

70722

732

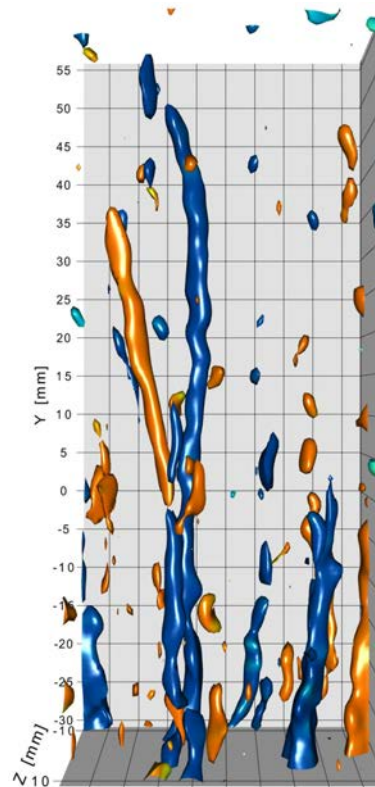

71429

733

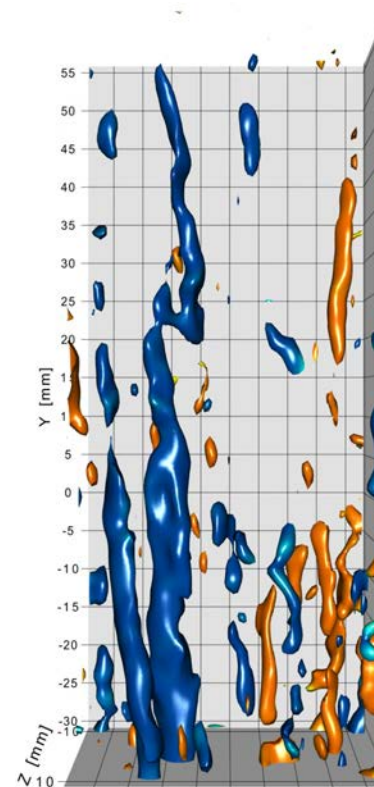

71852

734

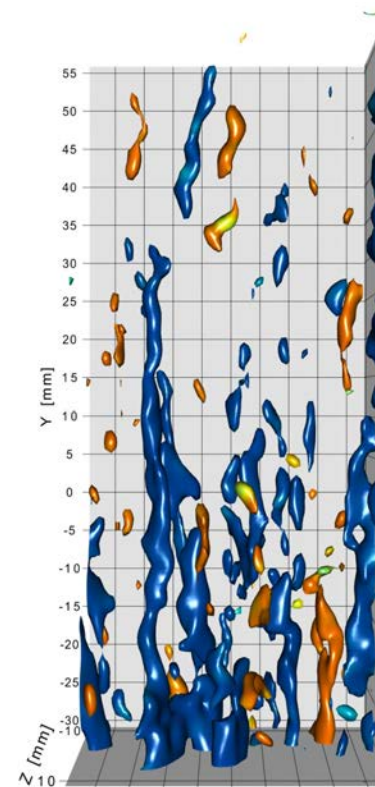

72444

735

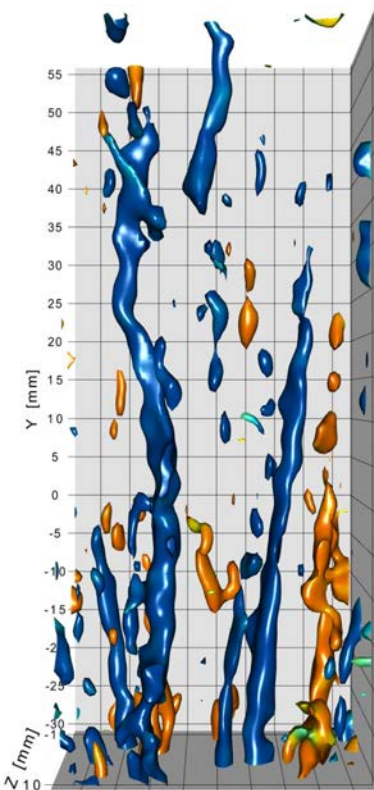

73661

736

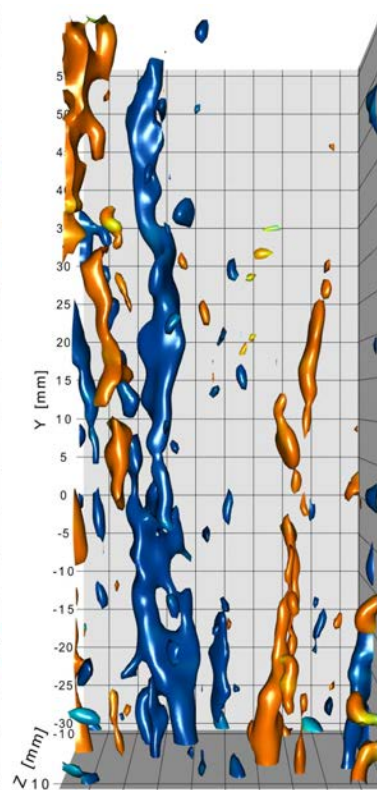

75652

737

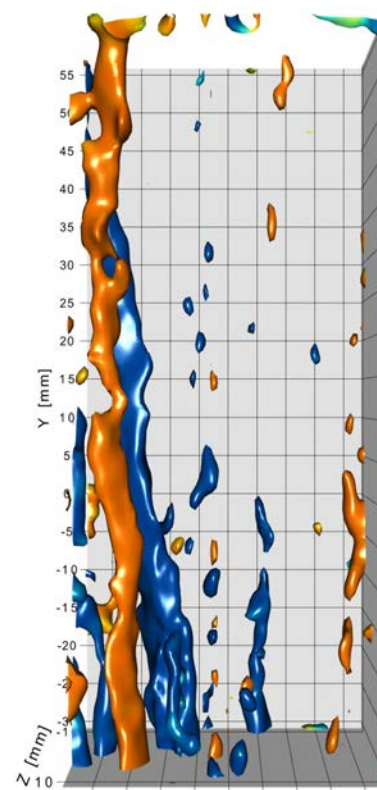

75894

738

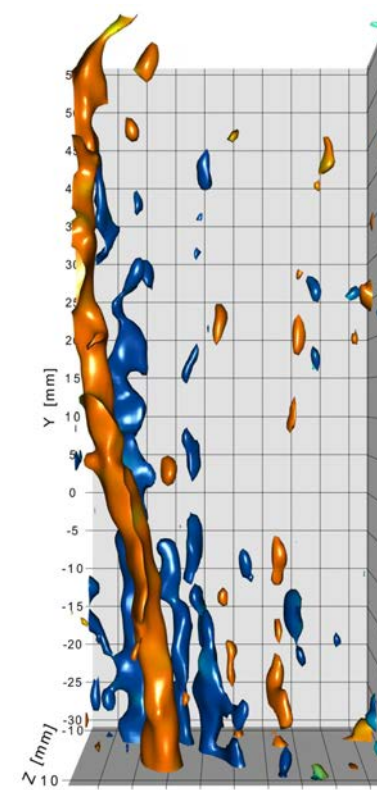

76175

739

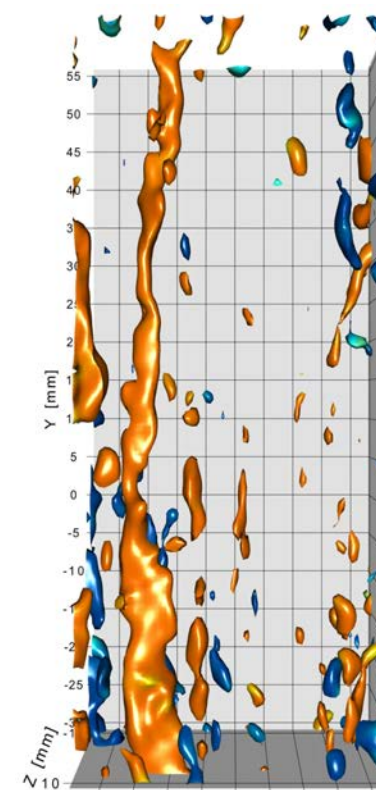

76529

740



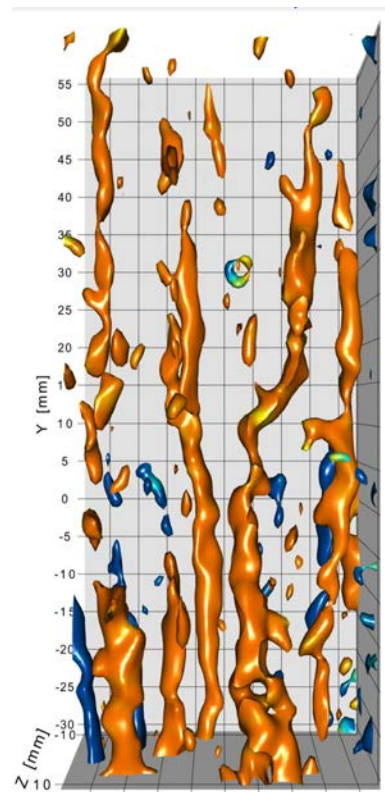

77456

741

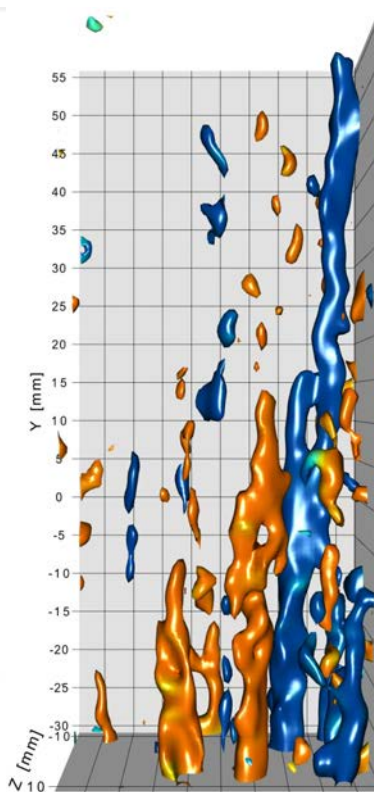

77857

742

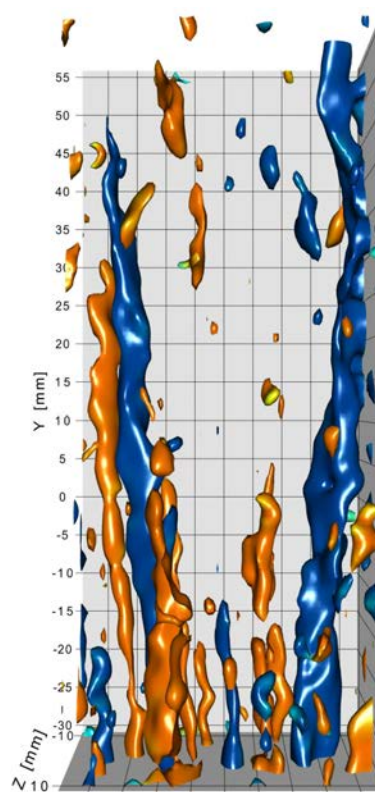

78832

743

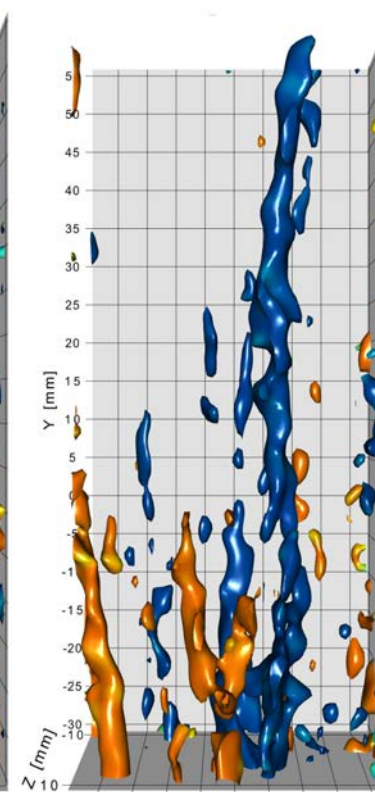

79277

744

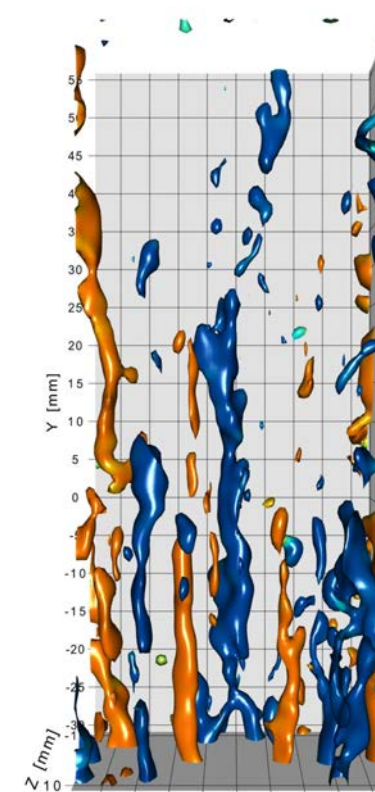

79871

745



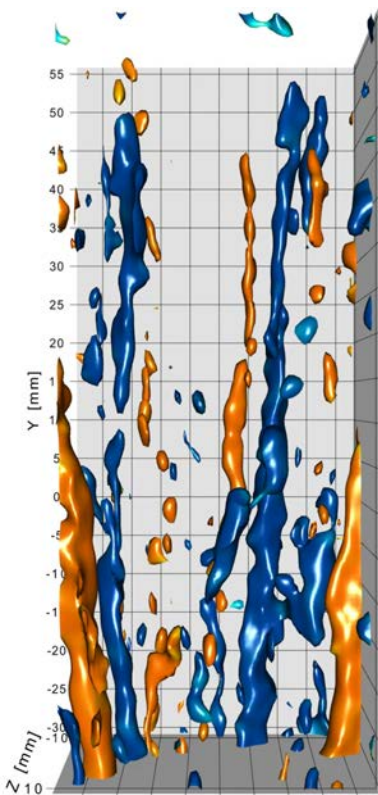

80149

746

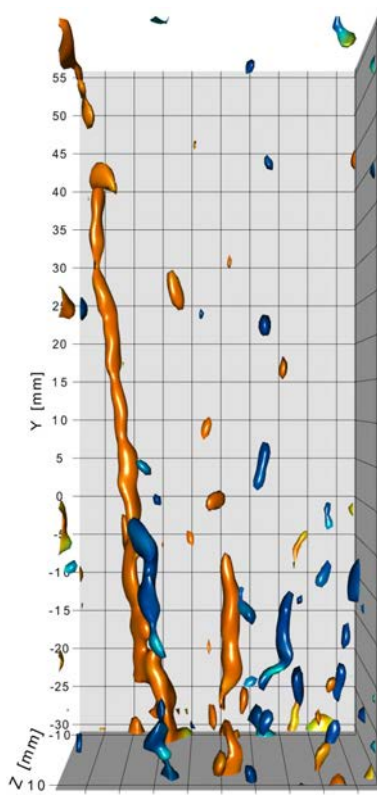

80711

747

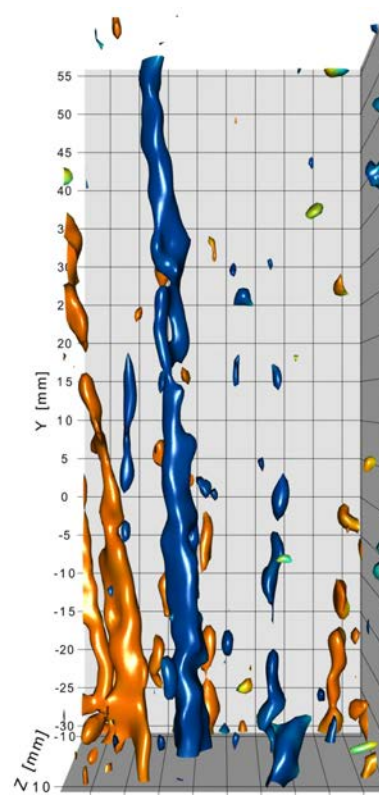

81132

748

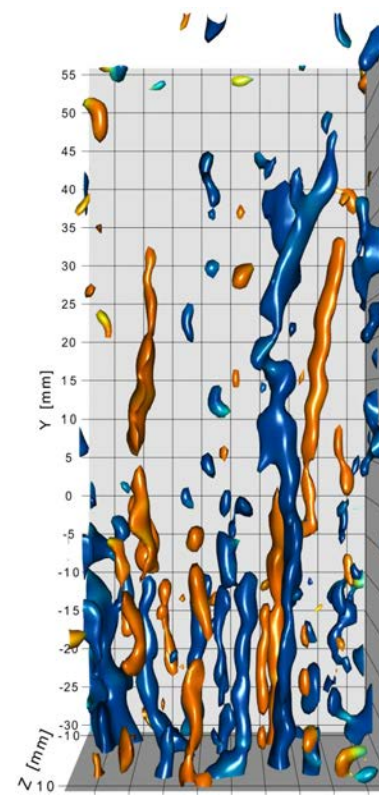

81684

749

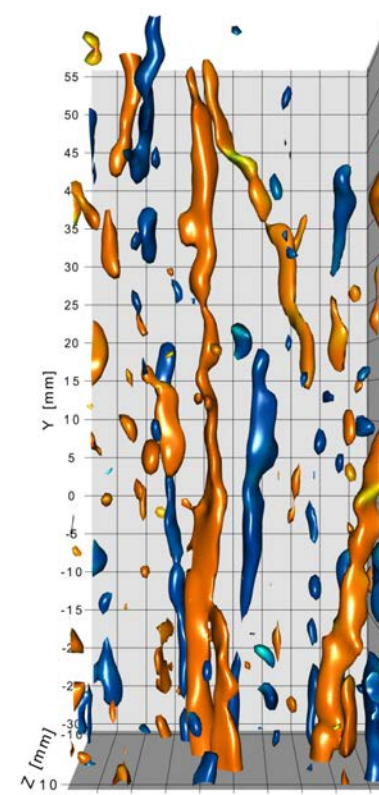

82200

750

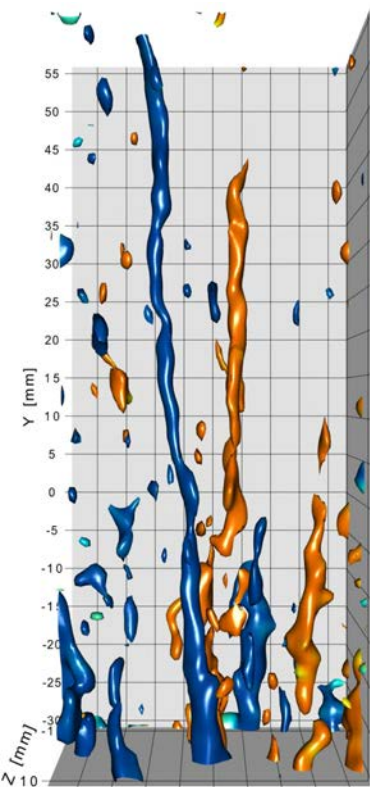

82711

751

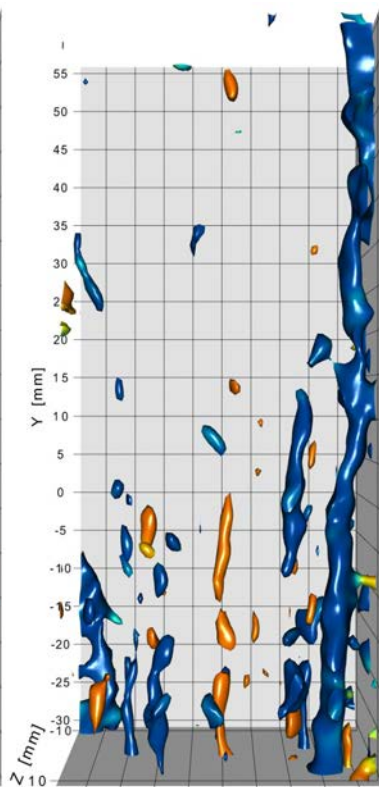

83614

752

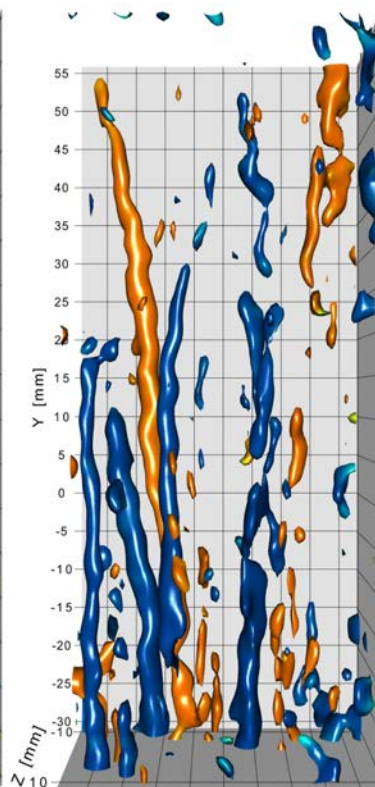

84871

753

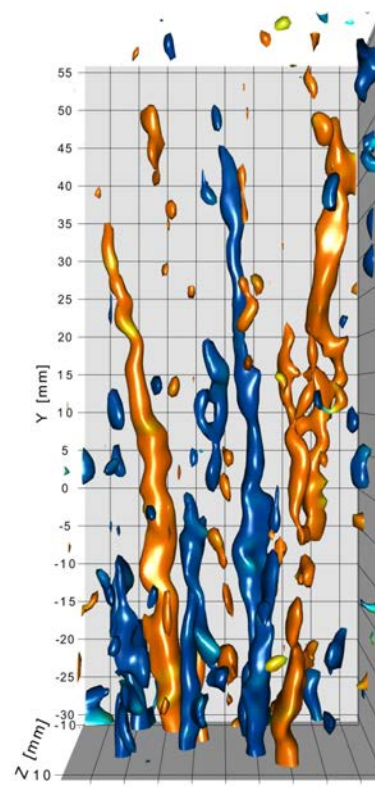

84957

754

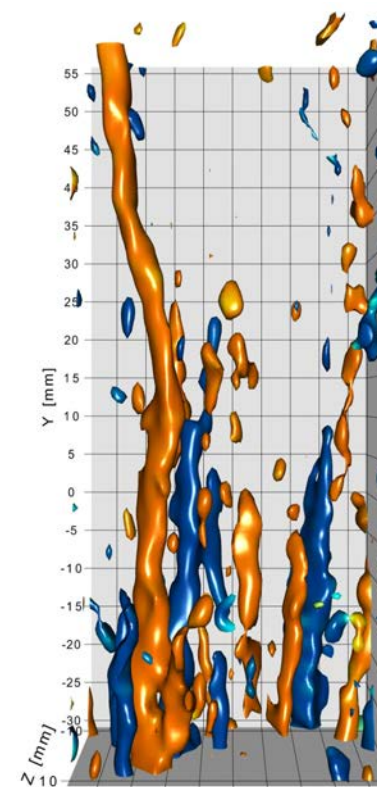

86223

755



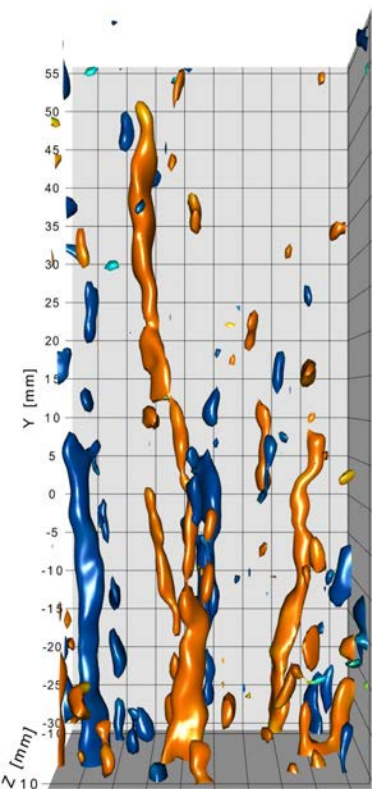

88289

756

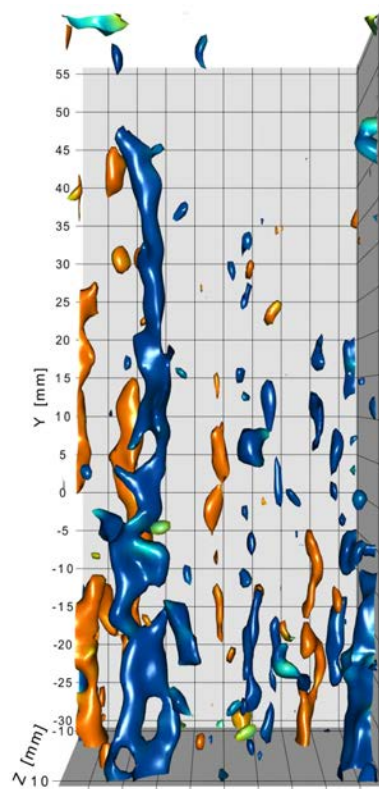

89051

757

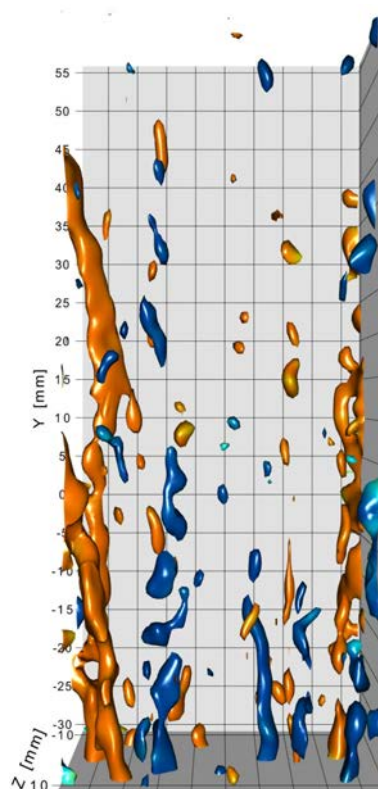

93643

758

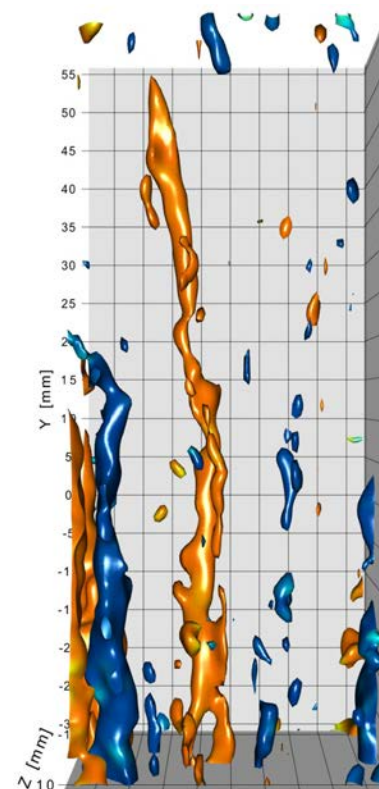

96111

759

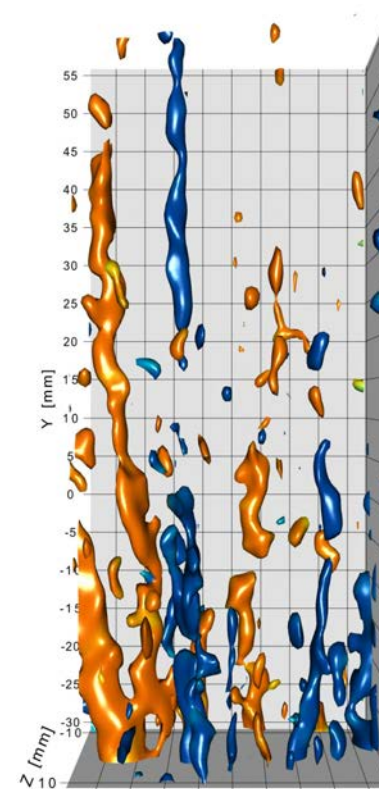

96446

760



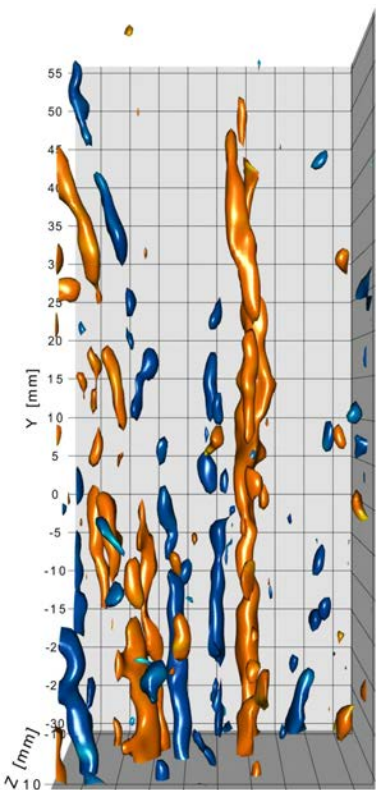

96736

761

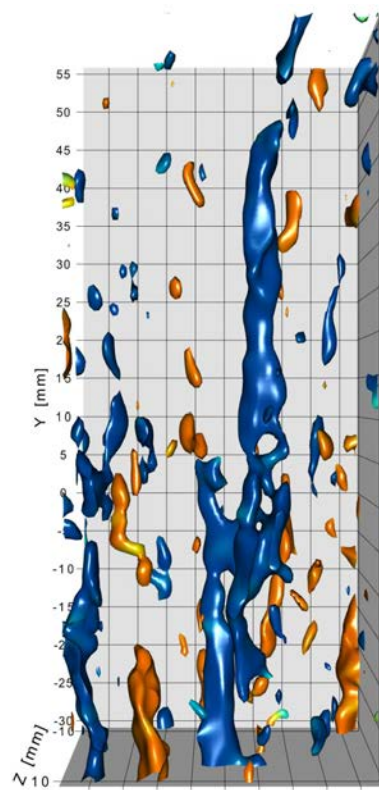

98331

762

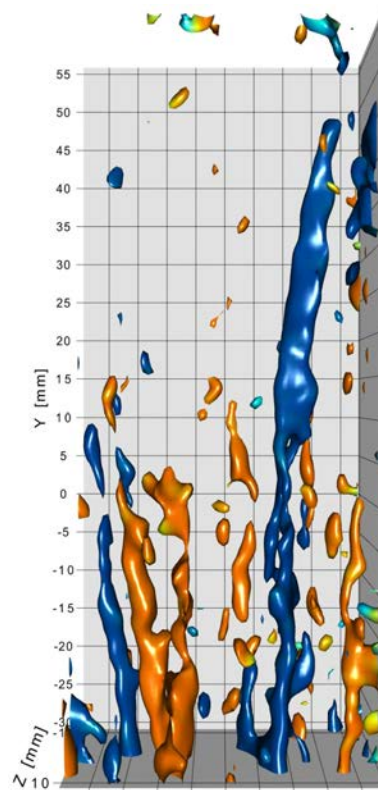

98823

763

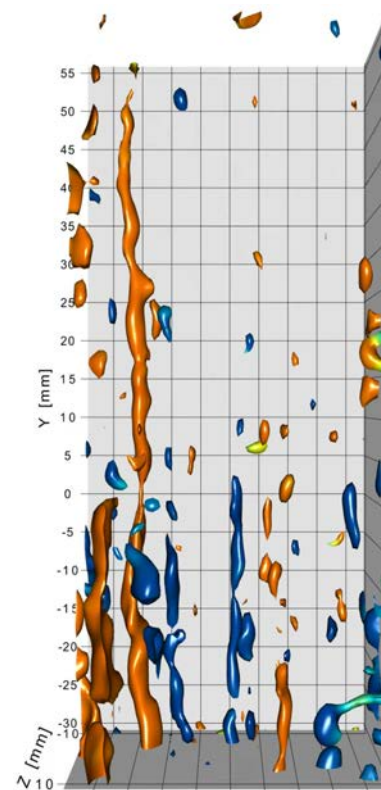

101680

764

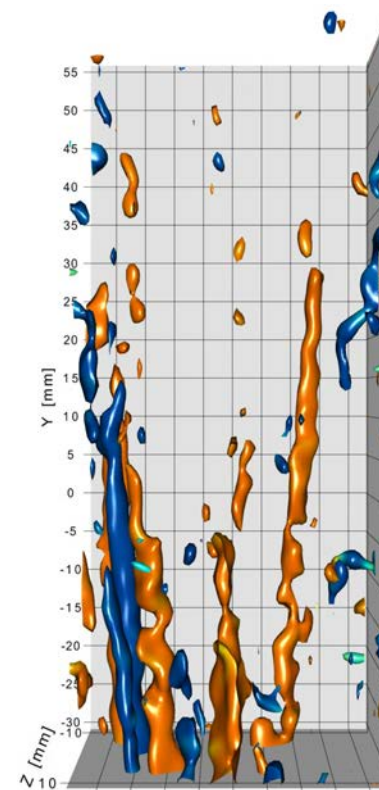

107350

765

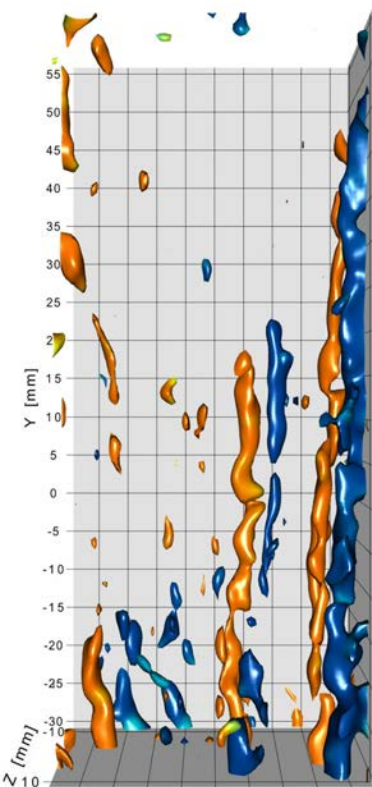

108168

766

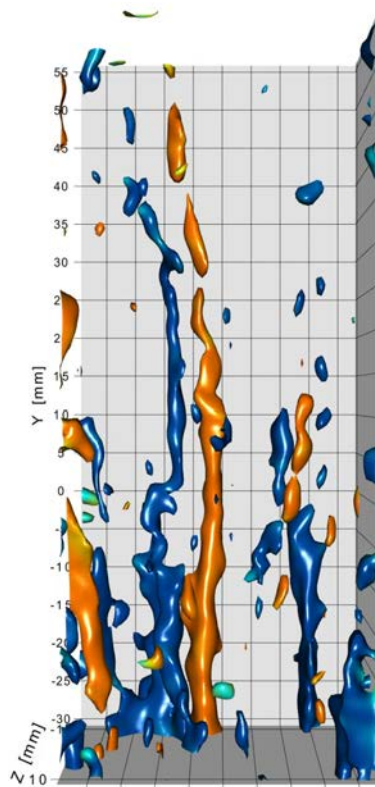

108682

767

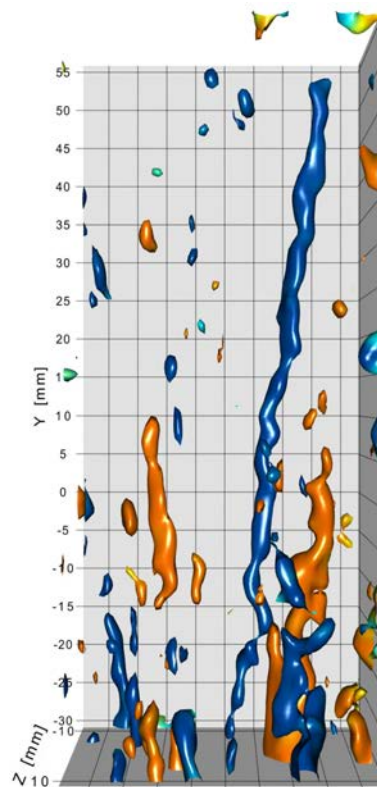

109633

768

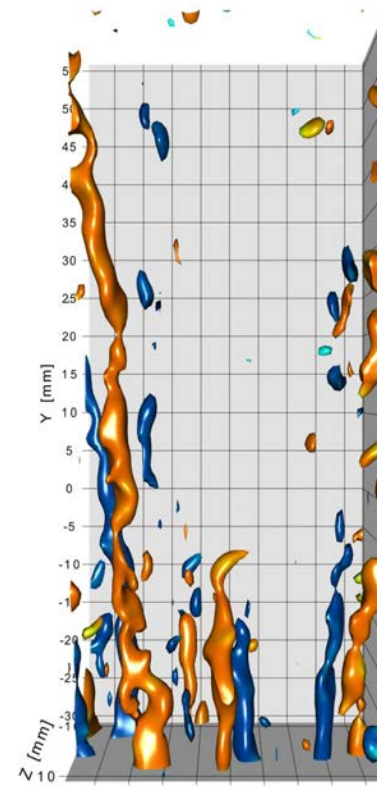

112735

769

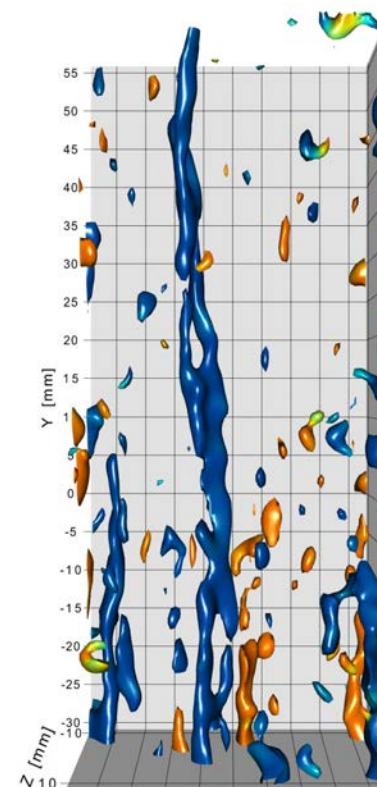

115787

770



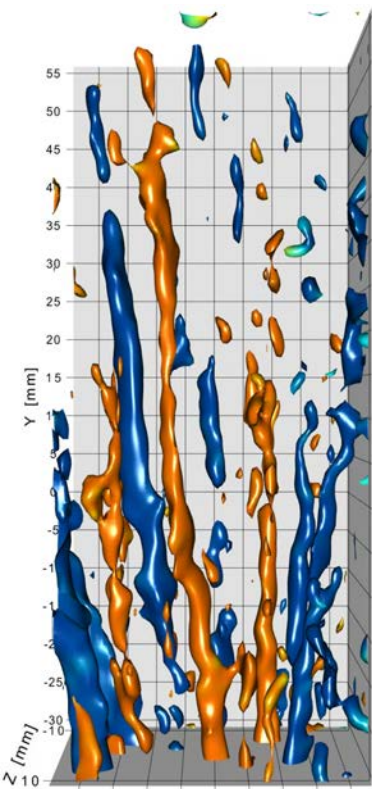

116226

771

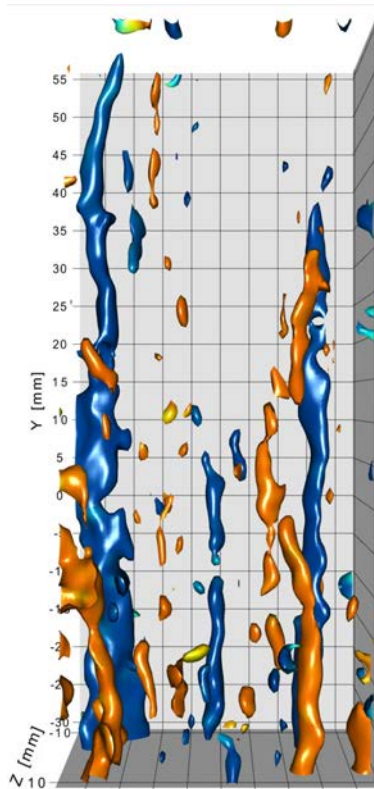

117588

772

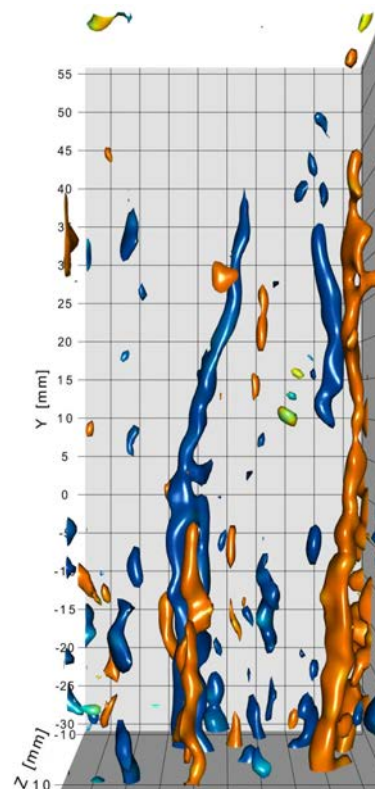

117989

773

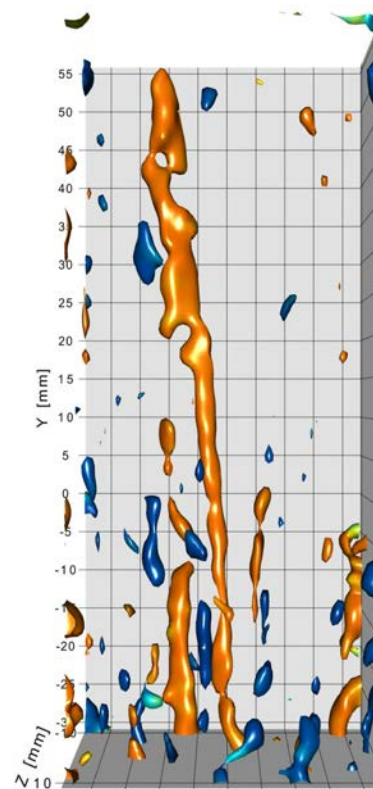

121688

774

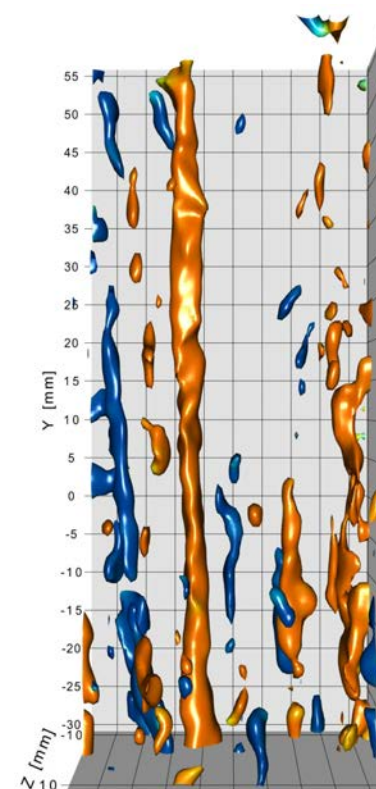

121881

775



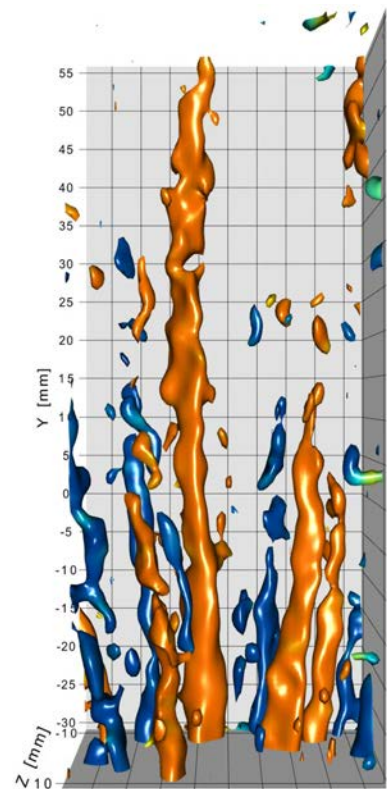

122062

776

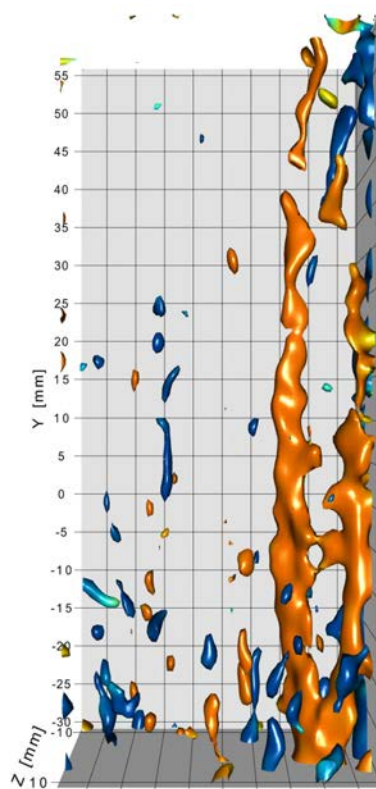

122694

777

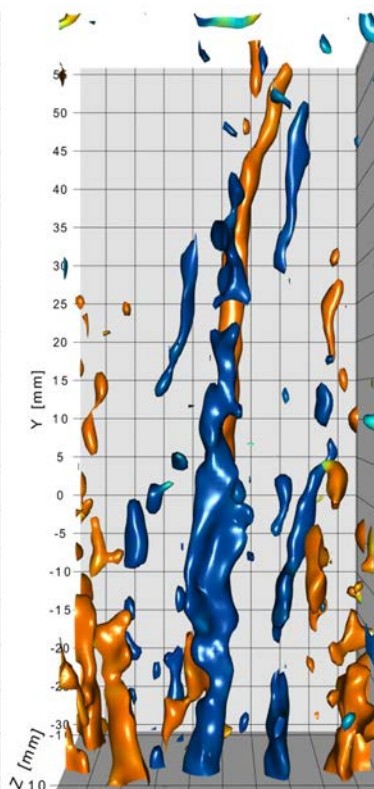

123672

778

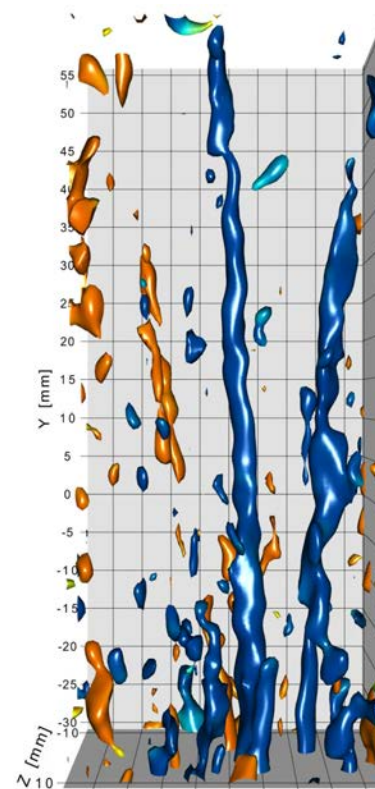

124032

779

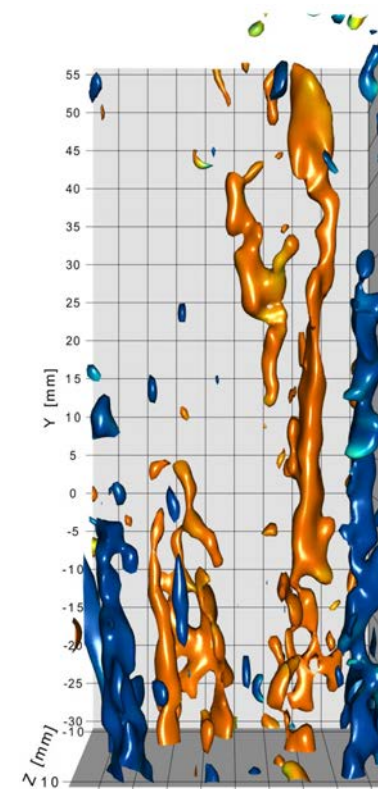

125837

780

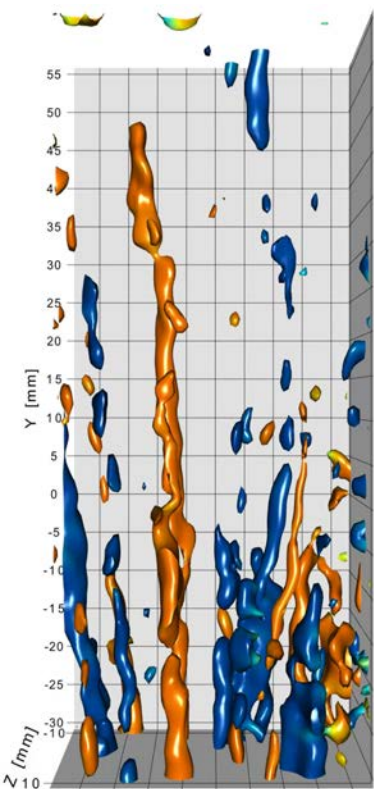

126645

781

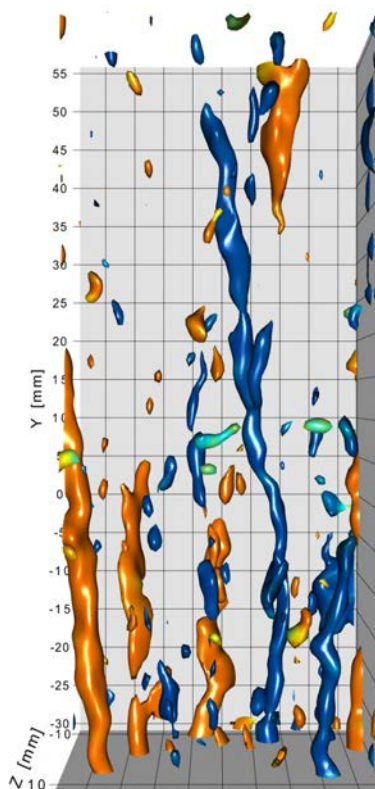

127121

782

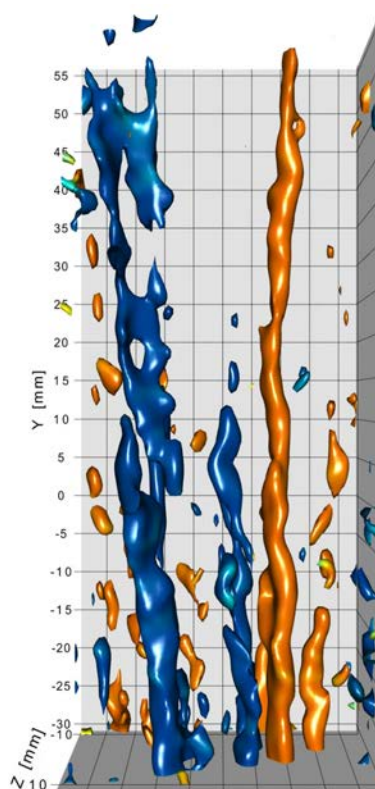

127545

783

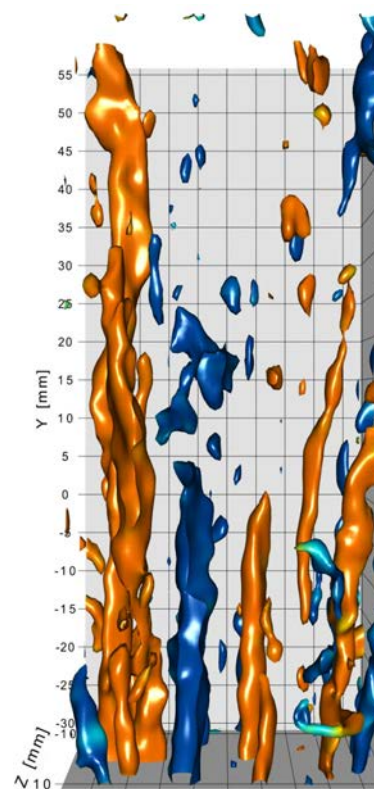

127926

784

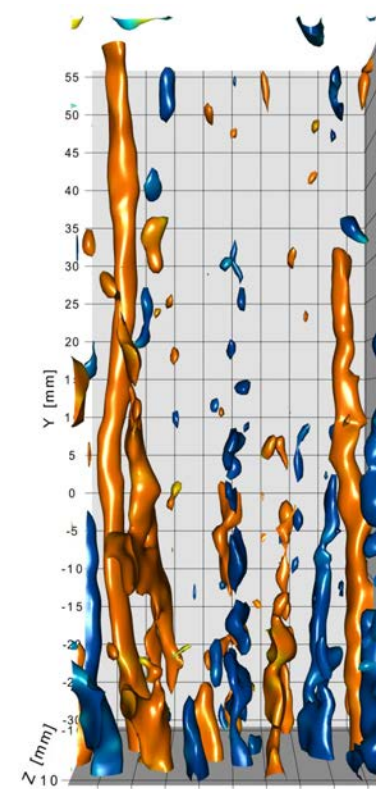

128280

785



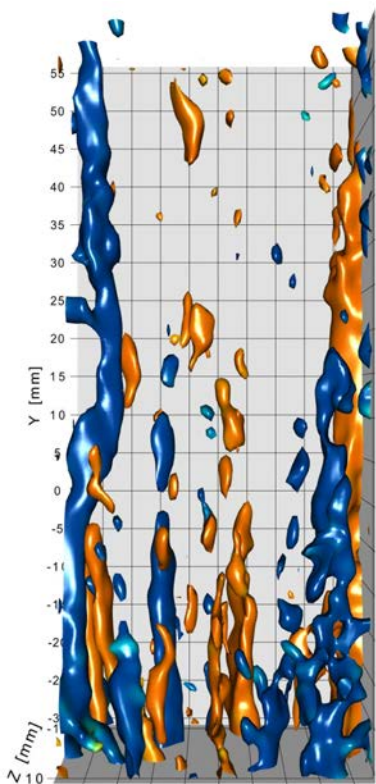

128556

786

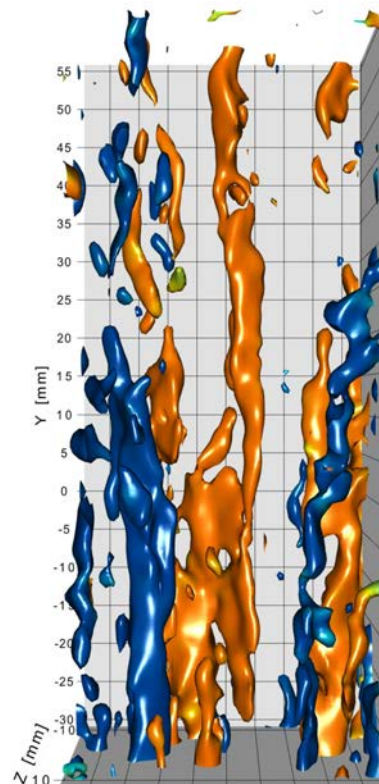

128737

787

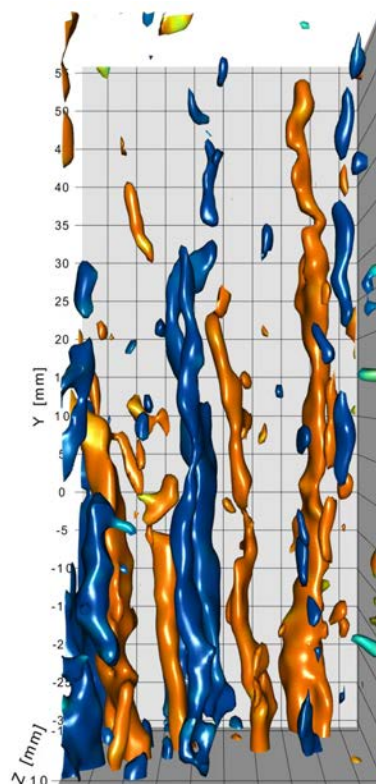

129083

788

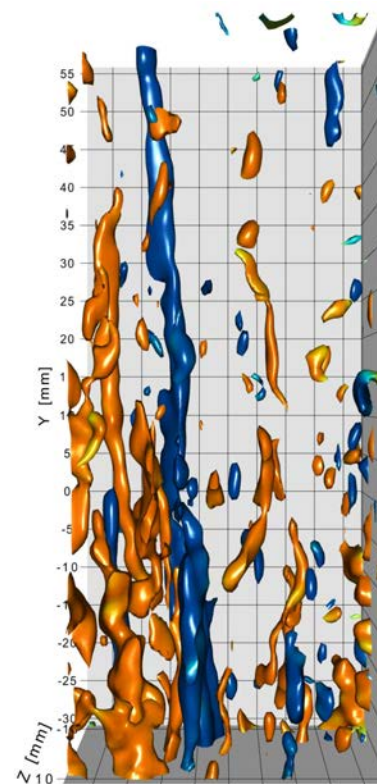

129586

789

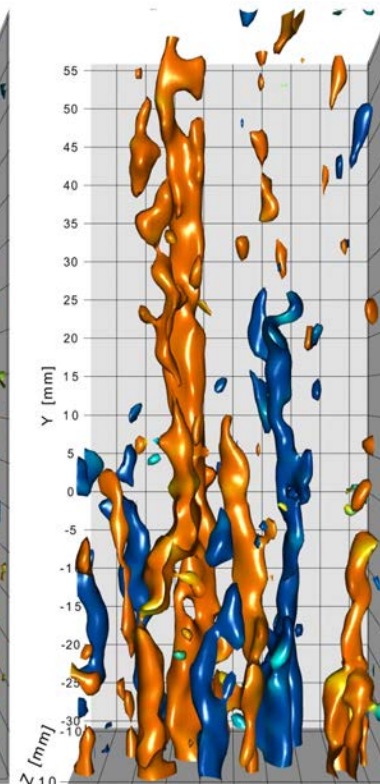

129880

790



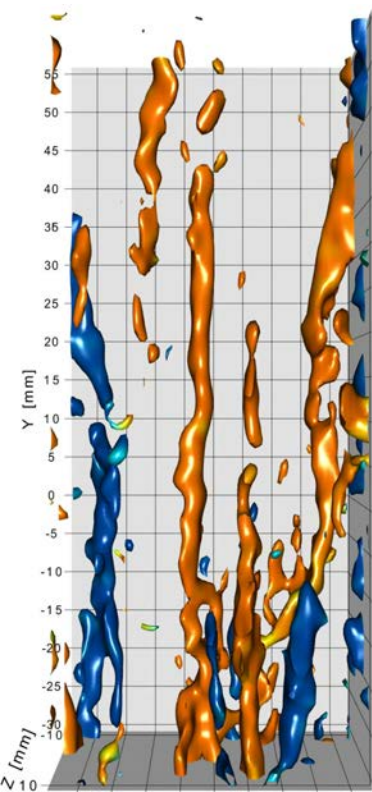

130201

791

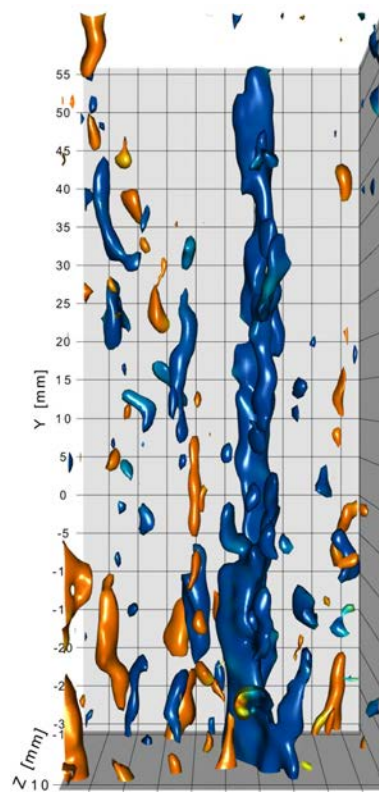

131020

792

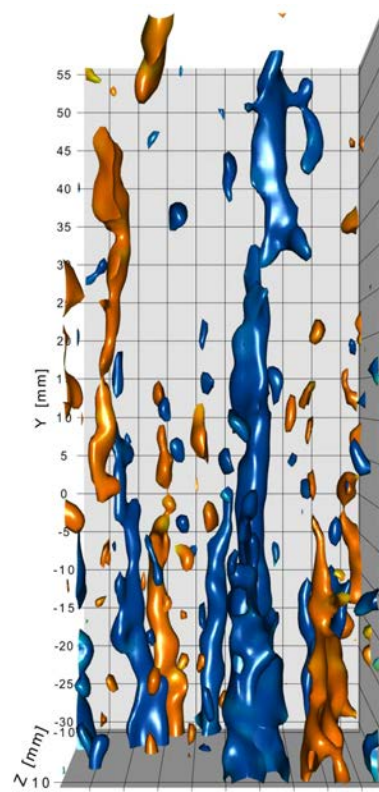

131176

793

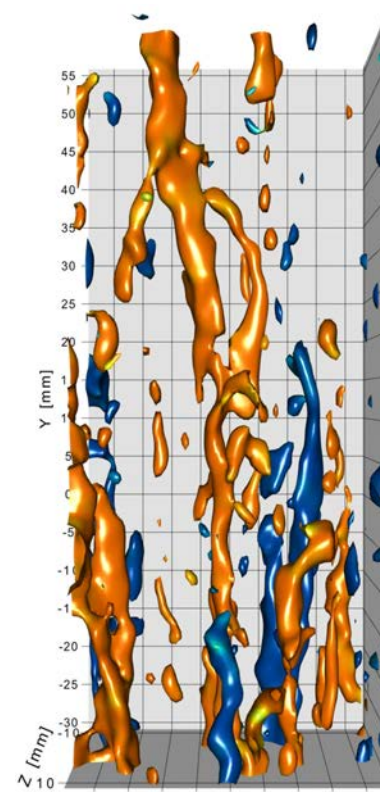

131827

794

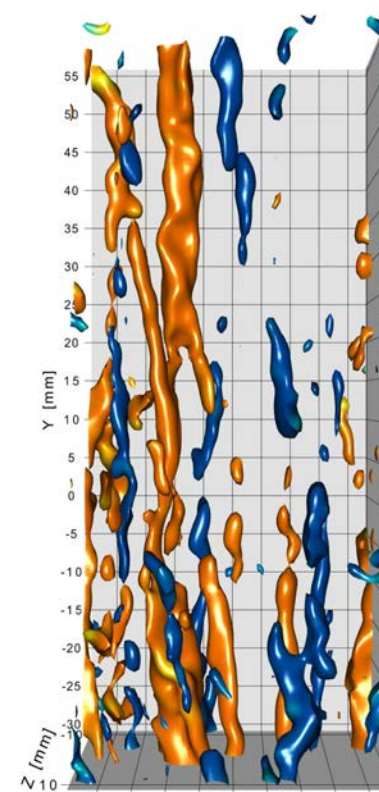

132212

795
